# Supplementary material for: Refined^2 Environment Classifiers
Source: arXiv:2608.07888 source file (2026-08-08)
Supplement: Supplementary file 1 [file supplementary_material.tex]

\documentclass{article}

% \newif\ifdraft
% \draftfalse

\newif\ifanonymous
\anonymousfalse

\usepackage[margin=2cm,bottom=3cm,footskip=1.5cm]{geometry}
\usepackage{amsthm}
\usepackage{amssymb}
\usepackage{hyperref}
\usepackage{mathpartir}
\usepackage{longtable}
\usepackage{mathtools}
\usepackage{thmtools}
\usepackage[svgnames]{xcolor}
\usepackage{zref}
\usepackage{zref-clever}
\usepackage{xspace}

% allow page breaks in math environments
\allowdisplaybreaks

% zcref
\zcsetup{capfirst,noabbrevfirst}

% new theorems
\declaretheorem[name=Definition]{definition}
\declaretheorem[name=Lemma]{lemma}
\declaretheorem[name=Theorem]{theorem}
\declaretheorem[name=Corollary]{corollary}
\declaretheorem[name=Notation]{notation}
\declaretheorem[name=Convention]{convention}

% hyperref
\hypersetup{hidelinks}

\input{macros}
\input{refenv}

\ifanonymous
\author{Anonymous Author(s)}
\else
\author{Yuito Murase and Atsushi Igarashi}
\fi

\title{Supplementary Material for ``Refined\textsuperscript{2} Environment Classifiers''}
\date{}

\begin{document}

\maketitle

\tableofcontents

\listoftheorems

\section{Outline}
This is the supplementary material of the paper titled ``Refined\textsuperscript{2} Environment Classifiers''.

\section{Definitions}
\subsection{Surface Language}
\begin{tabular}{cllcl}
  Integer          & $\refenvnt{n}$          & $\in  \token{Int} $                                         &             &                                                                                                                                                             \\
  Variable         & $\refenvmv{x}, \refenvmv{y}$ & $\in  \token{Var} $                                         &             &                                                                                                                                                             \\
  Expression       & $ \refenvnt{e} ^{ \refenvnt{k}  } $ & $\in  \token{Exp}^{ \refenvnt{k} } $    & $\Coloneqq$ & $ \refenvnt{n} \mid \refenvmv{x} \mid   \lambda \binder{ \refenvmv{x} }.\  \refenvnt{e}  ^{ \refenvnt{k}  }  \mid    \refenvnt{e_{{\mathrm{1}}}} ^{ \refenvnt{k}  }     \refenvnt{e_{{\mathrm{2}}}} ^{ \refenvnt{k}  }    \mid  \langle   \refenvnt{e} ^{  \refenvnt{k}  \refenvsym{+}  1   }   \rangle  \mid  { \mathdollar }_{ \refenvnt{k'} }\lbrace  \refenvnt{e} ^{ \refenvnt{k}  \refenvsym{-}  \refenvnt{k'}  }  \rbrace  \text{\ (where $\refenvnt{k} \ge \refenvnt{k'}$)}$ \\
                   &               &                    & $\mid$      & $  \token{rec}\ \binder{ \refenvmv{f} }(\binder{ \refenvmv{x} }).\  \refenvnt{e}  ^{ \refenvnt{k}  }  \mid \token{ref} \, \refenvsym{(}   \refenvnt{e} ^{ \refenvnt{k}  }   \refenvsym{)} \mid   \refenvnt{e_{{\mathrm{1}}}} ^{ \refenvnt{k}  }  \coloneqq  \refenvnt{e_{{\mathrm{2}}}} ^{ \refenvnt{k}  }   \mid  \token{deref}(  \refenvnt{e} ^{ \refenvnt{k}  }  ) $
  \\
\end{tabular}

\subsection{Surface Type System}
\subsubsection{Objects for the Type System}
\begin{tabular}{cllcl}
  Classifier Stack   &               & $ \overrightarrow{ \gamma } $      & $\Coloneqq$ & $ \varepsilon  \mid  \overrightarrow{ \gamma }   \refenvsym{,}  \delta$                                                                                                                           \\
  Polymorphic Classifier Declaration &               & $\varrho$ & $\Coloneqq$ & $ \varepsilon  \mid \varrho  \refenvsym{,}   \binder{ \gamma_{{\mathrm{1}}} }  \mathbin{:\succeq}   \gamma_{{\mathrm{2}}} $ \\
  Base Type          &               & $\iota$   & $\Coloneqq$ & $ \texttt{int}  \mid \ldots$                                                                                                                                     \\
  Type               &               & $\refenvnt{A}, \refenvnt{B}$ & $\Coloneqq$ & $\iota \mid \refenvnt{A}  \rightarrow  \refenvnt{B} \mid  \langle \refenvnt{A} \rangle^{ \gamma } \mid  \refenvnt{A} \/\ \token{ref}  \mid  \forall  \varrho . \refenvnt{A} $                                                                                                           \\
  Typing Context     &               & $\Gamma$          & $\Coloneqq$ & $ \varepsilon  \mid \Gamma  \refenvsym{,}   \binder{ \refenvmv{x} }\mathord{:^{\binder{ \gamma } } } \refenvnt{A}  \mid \Gamma  \refenvsym{,}   \blacktriangleright ^{ \gamma }  \mid \Gamma  \refenvsym{,}   \blacktriangleleft _{ \refenvnt{k} }^{\binder{ \gamma } }  \mid \Gamma  \refenvsym{,}   [  \varrho  ]^{\binder{ \gamma } } $ \\
  Introduction Forms &               & $ {e_{I} } ^{ \refenvnt{k}  } $       & $\Coloneqq$ & $  \lambda \binder{ \refenvmv{x} }.\  \refenvnt{e}  ^{ \refenvnt{k}  }  \mid   \token{rec}\ \binder{ \refenvmv{f} }(\binder{ \refenvmv{x} }).\  \refenvnt{e}  ^{ \refenvnt{k}  }   \mid  \langle   \refenvnt{e} ^{  \refenvnt{k}  \refenvsym{+}  1   }   \rangle $
\end{tabular}

\begin{definition}[Free Occurrences of Classifiers]
  $ \token{FC}( \refenvnt{A} ) $, $ \token{FC}( \varrho ) $, $ \token{FC}( \Gamma ) $ return the set of classifiers that occur freely in $\refenvnt{A}$, $\varrho$ and $\Gamma$, respectively. They are defined as follows.
  \begin{align*}
     \token{FC}( \iota )  & =  \emptyset           \\
     \token{FC}( \refenvnt{A_{{\mathrm{1}}}}  \rightarrow  \refenvnt{A_{{\mathrm{2}}}} )  & =  \token{FC}( \refenvnt{A_{{\mathrm{1}}}} )  \, \cup \,  \token{FC}( \refenvnt{A_{{\mathrm{2}}}} )  \\
     \token{FC}(  \langle \refenvnt{A} \rangle^{ \gamma }  )     & =  \token{FC}( \refenvnt{A} )  \, \cup \, \refenvsym{\{}  \gamma  \refenvsym{\}} \\
     \token{FC}(  \refenvnt{A} \/\ \token{ref}  )     & =  \token{FC}( \refenvnt{A} )  \\
     \token{FC}(  \forall  \varrho . \refenvnt{A}  )  &= \refenvsym{(}   \token{FC}( \refenvnt{A} )   \refenvsym{-}   \token{Dom}_{C}( \varrho )   \refenvsym{)} \, \cup \,  \token{FC}( \varrho )  \\
    \\
     \token{FC}( \varepsilon )  & =  \emptyset           \\
     \token{FC}( \varrho  \refenvsym{,}   \binder{ \gamma_{{\mathrm{1}}} }  \mathbin{:\succeq}   \gamma_{{\mathrm{2}}}  )  & =  \token{FC}( \varrho )  \, \cup \, \refenvsym{\{}  \gamma_{{\mathrm{2}}}  \refenvsym{\}}\\
    \\
     \token{FC}( \varepsilon )  & =  \emptyset           \\
     \token{FC}(  \binder{ \refenvmv{x} }\mathord{:^{\binder{ \gamma } } } \refenvnt{A}   \refenvsym{,}  \Gamma )  & =  \token{FC}( \Gamma )   \refenvsym{-}  \refenvsym{\{}  \gamma  \refenvsym{\}} \\
     \token{FC}(  \blacktriangleright ^{ \gamma }   \refenvsym{,}  \Gamma )  & =  \token{FC}( \Gamma )  \, \cup \, \refenvsym{\{}  \gamma  \refenvsym{\}} \\
     \token{FC}(  \blacktriangleleft _{ \refenvnt{k} }^{\binder{ \gamma } }   \refenvsym{,}  \Gamma )  & =  \token{FC}( \Gamma )   \refenvsym{-}  \refenvsym{\{}  \gamma  \refenvsym{\}} \\
     \token{FC}(  [  \varrho  ]^{\binder{ \gamma } }   \refenvsym{,}  \Gamma )  & =  \token{FC}( \Gamma )   \refenvsym{-}  \refenvsym{(}  \refenvsym{\{}  \gamma  \refenvsym{\}} \, \cup \,  \token{Dom}_{C}( \varrho )   \refenvsym{)} \, \cup \,  \token{FC}( \varrho ) 
  \end{align*}
\end{definition}

\begin{definition}[Classifier Domain of Contexts]
  $ \token{Dom}_{C}( \Gamma ) $ and $ \token{Dom}_{C}( \varrho ) $ return the set of classifiers declared in $\Gamma$ and $\varrho$, respectively. They are defined as follows.
  \begin{align*}
     \token{Dom}_{C}( \varepsilon )     & =  \emptyset               \\
     \token{Dom}_{C}( \Gamma  \refenvsym{,}   \binder{ \refenvmv{x} }\mathord{:^{\binder{ \gamma } } } \refenvnt{A}  )  & =  \token{Dom}_{C}( \Gamma )  \, \cup \, \refenvsym{\{}  \gamma  \refenvsym{\}} \\
     \token{Dom}_{C}( \Gamma  \refenvsym{,}   \blacktriangleright ^{ \gamma }  )    & =  \token{Dom}_{C}( \Gamma )              \\
     \token{Dom}_{C}( \Gamma  \refenvsym{,}   \blacktriangleleft _{ \refenvnt{k} }^{\binder{ \gamma } }  )  & =  \token{Dom}_{C}( \Gamma )  \, \cup \, \refenvsym{\{}  \gamma  \refenvsym{\}} \\
     \token{Dom}_{C}( \Gamma  \refenvsym{,}   [  \varrho  ]^{\binder{ \gamma } }  )  & =  \token{Dom}_{C}( \Gamma )  \, \cup \,  \token{Dom}_{C}( \varrho )  \, \cup \, \refenvsym{\{}  \gamma  \refenvsym{\}} \\
    \\
     \token{Dom}_{C}( \varepsilon )  & =  \emptyset               \\
     \token{Dom}_{C}( \varrho  \refenvsym{,}   \binder{ \gamma_{{\mathrm{1}}} }  \mathbin{:\succeq}   \gamma_{{\mathrm{2}}}  )  & =  \token{Dom}_{C}( \varrho )  \, \cup \, \refenvsym{\{}  \gamma_{{\mathrm{1}}}  \refenvsym{\}}
  \end{align*}
\end{definition}

\begin{definition}[Classifier Substitution Mapping]
  A classifier substitution mapping, ranged over by $\sigma$, is a
  finite mapping from classifiers to classifiers.  We write it as
  $  \gamma _{ 1 }  \coloneqq  \gamma' _{ 1 }  ,\dotsc,  \gamma _{ \refenvnt{k} }  \coloneqq  \gamma' _{ \refenvnt{k} }  $, assuming that the classifiers
  $ \gamma _{ 1 } $ to $ \gamma _{ \refenvnt{k} } $ are pairwise distinct.
  Its domain and range are defined as follows:
  \begin{align*}
     \token{Dom}_{C}(   \gamma _{ 1 }  \coloneqq  \gamma' _{ 1 }  ,\dotsc,  \gamma _{ \refenvnt{k} }  \coloneqq  \gamma' _{ \refenvnt{k} }   )  &= \refenvsym{\{}    \gamma _{ 1 }  ,\dotsc,  \gamma _{ \refenvnt{k} }    \refenvsym{\}} \\
     \token{Reg}_{C}(   \gamma _{ 1 }  \coloneqq  \gamma' _{ 1 }  ,\dotsc,  \gamma _{ \refenvnt{k} }  \coloneqq  \gamma' _{ \refenvnt{k} }   )  &= \refenvsym{\{}    \gamma' _{ 1 }  ,\dotsc,  \gamma' _{ \refenvnt{k} }    \refenvsym{\}}
  \end{align*}
\end{definition}

\begin{definition}[Classifier Substitution]
  Classifier substitution is the capture-avoiding operation induced by a
  classifier substitution mapping.  For
  $\sigma =   \gamma _{ 1 }  \coloneqq  \gamma' _{ 1 }  ,\dotsc,  \gamma _{ \refenvnt{k} }  \coloneqq  \gamma' _{ \refenvnt{k} }  $, we write
  $\delta  \refenvsym{[}  \sigma  \refenvsym{]}$ for the classifier obtained by replacing $\delta$
  with $ \gamma' _{ \refenvnt{i} } $ when $\delta =  \gamma _{ \refenvnt{i} } $, and leaving $\delta$
  unchanged otherwise.

  It extends to classifier sequences, types, polymorphic classifier
  declarations, and contexts as follows:
  \begin{align*}
    \varepsilon  \refenvsym{[}  \sigma  \refenvsym{]} &=  \varepsilon  \\
    \refenvsym{(}   \overrightarrow{ \gamma }   \refenvsym{,}  \delta  \refenvsym{)}  \refenvsym{[}  \sigma  \refenvsym{]} &= \refenvsym{(}   \overrightarrow{ \gamma }   \refenvsym{)}  \refenvsym{[}  \sigma  \refenvsym{]}  \refenvsym{,}  \delta  \refenvsym{[}  \sigma  \refenvsym{]} \\
    \\
    \iota  \refenvsym{[}  \sigma  \refenvsym{]} &= \iota \\
    \refenvsym{(}  \refenvnt{A_{{\mathrm{1}}}}  \rightarrow  \refenvnt{A_{{\mathrm{2}}}}  \refenvsym{)}  \refenvsym{[}  \sigma  \refenvsym{]} &= \refenvnt{A_{{\mathrm{1}}}}  \refenvsym{[}  \sigma  \refenvsym{]}  \rightarrow  \refenvnt{A_{{\mathrm{2}}}}  \refenvsym{[}  \sigma  \refenvsym{]} \\
     \langle \refenvnt{A} \rangle^{ \gamma }   \refenvsym{[}  \sigma  \refenvsym{]} &=  \langle \refenvnt{A}  \refenvsym{[}  \sigma  \refenvsym{]} \rangle^{ \gamma  \refenvsym{[}  \sigma  \refenvsym{]} }  \\
    \refenvsym{(}   \refenvnt{A} \/\ \token{ref}   \refenvsym{)}  \refenvsym{[}  \sigma  \refenvsym{]} &=  \refenvnt{A}  \refenvsym{[}  \sigma  \refenvsym{]} \/\ \token{ref}  \\
    \refenvsym{(}   \forall  \varrho . \refenvnt{A}   \refenvsym{)}  \refenvsym{[}  \sigma  \refenvsym{]} &=
       \forall  \varrho  \refenvsym{[}  \sigma  \refenvsym{]} . \refenvnt{A}  \refenvsym{[}  \sigma  \refenvsym{]} \\
      &\qquad \text{if\/ $ \token{Dom}_{C}( \varrho )  \, \cap \, \refenvsym{(}   \token{Dom}_{C}( \sigma )  \, \cup \,  \token{Reg}_{C}( \sigma )   \refenvsym{)} = \emptyset$} \\
    \\
    \varepsilon  \refenvsym{[}  \sigma  \refenvsym{]} &=  \varepsilon  \\
    \refenvsym{(}  \varrho  \refenvsym{,}   \binder{ \gamma_{{\mathrm{1}}} }  \mathbin{:\succeq}   \gamma_{{\mathrm{2}}}   \refenvsym{)}  \refenvsym{[}  \sigma  \refenvsym{]} &=
      \varrho  \refenvsym{[}  \sigma  \refenvsym{]}  \refenvsym{,}   \binder{ \gamma_{{\mathrm{1}}} }  \mathbin{:\succeq}   \gamma_{{\mathrm{2}}}   \refenvsym{[}  \sigma  \refenvsym{]} \\
    \\
    \varepsilon  \refenvsym{[}  \sigma  \refenvsym{]} &=  \varepsilon  \\
    \refenvsym{(}  \Gamma  \refenvsym{,}   \binder{ \refenvmv{x} }\mathord{:^{\binder{ \gamma } } } \refenvnt{A}   \refenvsym{)}  \refenvsym{[}  \sigma  \refenvsym{]} &= \Gamma  \refenvsym{[}  \sigma  \refenvsym{]}  \refenvsym{,}   \binder{ \refenvmv{x} }\mathord{:^{\binder{ \gamma } } } \refenvnt{A}  \refenvsym{[}  \sigma  \refenvsym{]}  \\
    \refenvsym{(}  \Gamma  \refenvsym{,}   \blacktriangleright ^{ \gamma }   \refenvsym{)}  \refenvsym{[}  \sigma  \refenvsym{]} &= \Gamma  \refenvsym{[}  \sigma  \refenvsym{]}  \refenvsym{,}   \blacktriangleright ^{  \gamma  \refenvsym{[}  \sigma  \refenvsym{]}  }  \\
    \refenvsym{(}  \Gamma  \refenvsym{,}   \blacktriangleleft _{ \refenvnt{k} }^{\binder{ \gamma } }   \refenvsym{)}  \refenvsym{[}  \sigma  \refenvsym{]} &= \Gamma  \refenvsym{[}  \sigma  \refenvsym{]}  \refenvsym{,}   \blacktriangleleft _{ \refenvnt{k} }^{\binder{ \gamma } }  \\
    \refenvsym{(}  \Gamma  \refenvsym{,}   [  \varrho  ]^{\binder{ \gamma } }   \refenvsym{)}  \refenvsym{[}  \sigma  \refenvsym{]} &=
      \Gamma  \refenvsym{[}  \sigma  \refenvsym{]}  \refenvsym{,}   [  \varrho  \refenvsym{[}  \sigma  \refenvsym{]}  ]^{\binder{ \gamma } } 
  \end{align*}
  The side condition in the clause for polymorphic classifier types ensures
  that the substitution does not capture the classifiers bound by
  $\varrho$.
\end{definition}


\subsubsection{Judgments and Derivation Rules}
\vspace{1em}
\fbox{$ \Gamma \vdash^{  \overrightarrow{ \gamma }^{+}  }\token{wf} $}
\begin{mathparpagebreakable}
  \myinferrule[WF-Ctx-Emp]
  {
  }
  {
     \varepsilon \vdash^{  \exclam  }\token{wf} 
  }
  \and
  \myinferrule[WF-Ctx-Var]
  { \Gamma \vdash^{  \overrightarrow{ \gamma_{{\mathrm{1}}} }   \refenvsym{,}  \gamma_{{\mathrm{2}}} }\token{wf}  \\
   \Gamma \vdash^{  \overrightarrow{ \gamma_{{\mathrm{1}}} }   \refenvsym{,}  \gamma_{{\mathrm{2}}} } \refenvnt{A} \ \token{wf}  \\
  \gamma_{{\mathrm{3}}} \, \not\in \,  \token{Dom}_{C}( \Gamma ) }
  {
     \Gamma  \refenvsym{,}   \binder{ \refenvmv{x} }\mathord{:^{\binder{ \gamma_{{\mathrm{3}}} } } } \refenvnt{A}  \vdash^{  \overrightarrow{ \gamma_{{\mathrm{1}}} }   \refenvsym{,}  \gamma_{{\mathrm{3}}} }\token{wf} 
  }
  \\
  \myinferrule[WF-Ctx-Open]
  { \Gamma \vdash^{  \overrightarrow{ \gamma_{{\mathrm{1}}} }   \refenvsym{,}  \gamma_{{\mathrm{2}}} }\token{wf}  \\
   \Gamma \vdash \gamma_{{\mathrm{3}}} \subseteq \gamma_{{\mathrm{2}}} }
  {
     \Gamma  \refenvsym{,}   \blacktriangleright ^{ \gamma_{{\mathrm{3}}} }  \vdash^{  \overrightarrow{ \gamma_{{\mathrm{1}}} }   \refenvsym{,}  \gamma_{{\mathrm{2}}}  \refenvsym{,}  \gamma_{{\mathrm{3}}} }\token{wf} 
  }
  \and
  \myinferrule[WF-Ctx-Shut]
  { \Gamma \vdash^{  \overrightarrow{ \gamma_{{\mathrm{1}}} }   \refenvsym{,}    \delta _{ 0 }  ,\dotsc,  \delta _{ \refenvnt{k} }   }\token{wf}  \\
  \gamma_{{\mathrm{2}}} \, \not\in \,  \token{Dom}_{C}( \Gamma ) }
  {
     \Gamma  \refenvsym{,}   \blacktriangleleft _{ \refenvnt{k} }^{\binder{ \gamma_{{\mathrm{2}}} } }  \vdash^{  \overrightarrow{ \gamma_{{\mathrm{1}}} }   \refenvsym{,}  \gamma_{{\mathrm{2}}} }\token{wf} 
  }
  \and
  \myinferrule[WF-Ctx-Polycls]
  { \Gamma \vdash^{  \overrightarrow{ \delta }   \refenvsym{,}   \gamma' _{ 0 }  }\token{wf}  \\
    \gamma _{ 0 }  ,\dotsc,  \gamma _{ \refenvnt{k} }   \text{\ are pairwise distinct } \\
   \gamma _{ \refenvnt{i} }  \, \not\in \,  \token{Dom}_{C}( \Gamma )  \text{\ for\ } 0 \le \refenvnt{i} \le \refenvnt{k} \\
   \gamma _{ 0 }  \, \not\in \,  \token{Dom}_{C}( \refenvsym{(}   \binder{  \gamma _{ 1 }  }  \mathbin{:\succeq}    \gamma' _{ 1 }  ,\dotsc,\binder{  \gamma _{ \refenvnt{k} }  }  \mathbin{:\succeq}    \gamma' _{ \refenvnt{k} }    \refenvsym{)} )  \\
   \Gamma \vdash  \gamma' _{ \refenvnt{i}  \refenvsym{+}  1 }  \subseteq  \gamma' _{ \refenvnt{i} }   \text{\ for \ } 0 \le \refenvnt{i} < \refenvnt{k}}
  { \Gamma  \refenvsym{,}   [    \binder{  \gamma _{ 1 }  }  \mathbin{:\succeq}    \gamma' _{ 1 }  ,\dotsc,\binder{  \gamma _{ \refenvnt{k} }  }  \mathbin{:\succeq}   \gamma'  _{ \refenvnt{k} }   ]^{\binder{  \gamma _{ 0 }  } }  \vdash^{  \overrightarrow{ \delta }   \refenvsym{,}   \gamma _{ 0 }  }\token{wf} }
  \label{rule:surface-wf-ctx-polycls}
\end{mathparpagebreakable}

\noindent\fbox{$ \Gamma \vdash^{  \overrightarrow{ \gamma }^{+}  } \refenvnt{A} \ \token{wf} $}
\begin{mathparpagebreakable}
  \myinferrule[WF-T-Base]
  { \Gamma \vdash^{  \overrightarrow{ \gamma }^{+}  }\token{wf} }
  { \Gamma \vdash^{  \overrightarrow{ \gamma }^{+}  } \iota \ \token{wf} }
  \label{rule:surface-wf-t-base}
  \and
  \myinferrule[WF-T-Func]
  { \Gamma \vdash^{  \overrightarrow{ \gamma }^{+}  } \refenvnt{A_{{\mathrm{1}}}} \ \token{wf}  \\
   \Gamma \vdash^{  \overrightarrow{ \gamma }^{+}  } \refenvnt{A_{{\mathrm{2}}}} \ \token{wf} }
  { \Gamma \vdash^{  \overrightarrow{ \gamma }^{+}  } \refenvnt{A_{{\mathrm{1}}}}  \rightarrow  \refenvnt{A_{{\mathrm{2}}}} \ \token{wf} }
  \label{rule:surface-wf-t-func}
  \and
  \myinferrule[WF-T-$\langle\rangle$]
  { \Gamma  \refenvsym{,}   \blacktriangleright ^{ \gamma_{{\mathrm{1}}} }  \vdash^{  \overrightarrow{ \gamma_{{\mathrm{2}}} }^{+}   \refenvsym{,}  \gamma_{{\mathrm{1}}} } \refenvnt{A} \ \token{wf} }
  { \Gamma \vdash^{  \overrightarrow{ \gamma_{{\mathrm{2}}} }^{+}  }  \langle \refenvnt{A} \rangle^{ \gamma_{{\mathrm{1}}} }  \ \token{wf} }
  \label{rule:surface-wf-t-code}
  \and
  \myinferrule[WF-T-Ref]
  { \Gamma \vdash^{  \overrightarrow{ \gamma }^{+}  } \refenvnt{A} \ \token{wf} }
  { \Gamma \vdash^{  \overrightarrow{ \gamma }^{+}  }  \refenvnt{A} \/\ \token{ref}  \ \token{wf} }
  \label{rule:surface-wf-t-ref}
  \and
  \myinferrule[WF-T-Polycls]
  { \Gamma  \refenvsym{,}   [  \varrho  ]^{\binder{ \gamma_{{\mathrm{1}}} } }  \vdash^{  \overrightarrow{ \delta }   \refenvsym{,}  \gamma_{{\mathrm{1}}} } \refenvnt{A} \ \token{wf}  \\
   \token{Dom}_{C}( \varrho )  \, \cap \,  \token{FC}( \refenvnt{A} )  = \emptyset \\
  \gamma_{{\mathrm{1}}} \, \not\in \,  \token{FC}( \refenvnt{A} )  \\
   \Gamma \vdash^{  \overrightarrow{ \delta }   \refenvsym{,}  \gamma_{{\mathrm{2}}} }\token{wf} }
  { \Gamma \vdash^{  \overrightarrow{ \delta }   \refenvsym{,}  \gamma_{{\mathrm{2}}} }  \forall  \varrho . \refenvnt{A}  \ \token{wf} }
  \label{rule:surface-wf-t-polycls}
\end{mathparpagebreakable}

\noindent\fbox{$ \Gamma \vdash \gamma_{{\mathrm{1}}} \preceq \gamma_{{\mathrm{2}}} $} \fbox{$ \Gamma \vdash \gamma_{{\mathrm{1}}} \subseteq \gamma_{{\mathrm{2}}} $}\quad Assuming that $ \Gamma \vdash^{  \overrightarrow{ \delta }^{+}  }\token{wf} $ for some $ \overrightarrow{ \delta }^{+} $.
\begin{mathparpagebreakable}
  \myinferrule[$ \preceq $-Refl]
  {\gamma \, \in \,  \token{Dom}_{C}( \Gamma )  \, \cup \, \refenvsym{\{}   \exclam   \refenvsym{\}}}
  { \Gamma \vdash \gamma \preceq \gamma }
  \label{rule:surface-ltrans-refl}
  \and
  \myinferrule[$ \preceq $-Trans]
  { \Gamma \vdash \gamma_{{\mathrm{1}}} \preceq \gamma_{{\mathrm{2}}}  \\
   \Gamma \vdash \gamma_{{\mathrm{2}}} \preceq \gamma_{{\mathrm{3}}} }
  { \Gamma \vdash \gamma_{{\mathrm{1}}} \preceq \gamma_{{\mathrm{3}}} }
  \label{rule:surface-ltrans-trans}
  \and
  \myinferrule[$ \preceq $-Var]
  { \Gamma_{{\mathrm{1}}} \vdash^{  \overrightarrow{ \gamma_{{\mathrm{1}}} }   \refenvsym{,}  \gamma_{{\mathrm{2}}} }\token{wf} }
  { \Gamma_{{\mathrm{1}}}  \refenvsym{,}   \binder{ \refenvmv{x} }\mathord{:^{\binder{ \gamma_{{\mathrm{3}}} } } } \refenvnt{A}   \refenvsym{,}  \Gamma_{{\mathrm{2}}} \vdash \gamma_{{\mathrm{2}}} \preceq \gamma_{{\mathrm{3}}} }
  \label{rule:surface-ltrans-var}
  \and
  \myinferrule[$ \preceq $-$ \blacktriangleleft $]
  { \Gamma_{{\mathrm{1}}} \vdash^{  \overrightarrow{ \gamma_{{\mathrm{1}}} }   \refenvsym{,}   \delta _{ 0 }   \refenvsym{,}    \delta _{ 1 }  ,\dotsc,  \delta _{ \refenvnt{k} }   }\token{wf}  \\
  \refenvnt{k} \ge 0}
  { \Gamma_{{\mathrm{1}}}  \refenvsym{,}   \blacktriangleleft _{ \refenvnt{k} }^{\binder{ \gamma_{{\mathrm{2}}} } }   \refenvsym{,}  \Gamma_{{\mathrm{2}}} \vdash  \delta _{ 0 }  \preceq \gamma_{{\mathrm{2}}} }
  \label{rule:surface-ltrans-shut}
  \and
  \myinferrule[$ \subseteq $-Lift]
  { \Gamma \vdash \gamma_{{\mathrm{1}}} \preceq \gamma_{{\mathrm{2}}} }
  { \Gamma \vdash \gamma_{{\mathrm{1}}} \subseteq \gamma_{{\mathrm{2}}} }
  \label{rule:surface-gtrans-lift}
  \and
  \myinferrule[$ \subseteq $-Trans]
  { \Gamma \vdash \gamma_{{\mathrm{1}}} \subseteq \gamma_{{\mathrm{2}}}  \\
   \Gamma \vdash \gamma_{{\mathrm{2}}} \subseteq \gamma_{{\mathrm{3}}} }
  { \Gamma \vdash \gamma_{{\mathrm{1}}} \subseteq \gamma_{{\mathrm{3}}} }
  \label{rule:surface-gtrans-trans}
  \and
  \myinferrule[$ \subseteq $-$ \blacktriangleleft $]
  { \Gamma_{{\mathrm{1}}} \vdash^{  \overrightarrow{ \gamma_{{\mathrm{1}}} }   \refenvsym{,}  \gamma_{{\mathrm{2}}} }\token{wf} }
  { \Gamma_{{\mathrm{1}}}  \refenvsym{,}   \blacktriangleleft _{ \refenvnt{k} }^{\binder{ \gamma_{{\mathrm{3}}} } }   \refenvsym{,}  \Gamma_{{\mathrm{2}}} \vdash \gamma_{{\mathrm{2}}} \subseteq \gamma_{{\mathrm{3}}} }
  \label{rule:surface-gtrans-shut}
  \and
  \myinferrule[$ \preceq $-Polycls]
  { \Gamma_{{\mathrm{1}}} \vdash^{  \overrightarrow{ \delta }   \refenvsym{,}   \gamma' _{ 0 }  }\token{wf}  \\
  0 \le \refenvnt{i} \le \refenvnt{k}}
  { \Gamma_{{\mathrm{1}}}  \refenvsym{,}   [    \binder{  \gamma _{ 1 }  }  \mathbin{:\succeq}    \gamma' _{ 1 }  ,\dotsc,\binder{  \gamma _{ \refenvnt{k} }  }  \mathbin{:\succeq}   \gamma'  _{ \refenvnt{k} }   ]^{\binder{  \gamma _{ 0 }  } }   \refenvsym{,}  \Gamma_{{\mathrm{2}}} \vdash  \gamma' _{ \refenvnt{i} }  \preceq  \gamma _{ \refenvnt{i} }  }
  \label{rule:surface-ltrans-polycls}
  \and
  \myinferrule[$ \subseteq $-Polycls]
  {0 \le \refenvnt{i} < \refenvnt{k}}
  { \Gamma_{{\mathrm{1}}}  \refenvsym{,}   [    \binder{  \gamma _{ 1 }  }  \mathbin{:\succeq}    \gamma' _{ 1 }  ,\dotsc,\binder{  \gamma _{ \refenvnt{k} }  }  \mathbin{:\succeq}   \gamma'  _{ \refenvnt{k} }   ]^{\binder{  \gamma _{ 0 }  } }   \refenvsym{,}  \Gamma_{{\mathrm{2}}} \vdash  \gamma _{ \refenvnt{i}  \refenvsym{+}  1 }  \subseteq  \gamma _{ \refenvnt{i} }  }
  \label{rule:surface-gtrans-polycls}
    \vspace{0.5em}
\end{mathparpagebreakable}

\noindent\fbox{$ \Gamma \vdash^{  \overrightarrow{ \gamma }^{+}  } \refenvnt{e} : \refenvnt{A} $}
\begin{mathparpagebreakable}
  \myinferrule[T-Int]
  { \Gamma \vdash^{  \overrightarrow{ \gamma }^{+}  }\token{wf} }
  { \Gamma \vdash^{  \overrightarrow{ \gamma }^{+}  } \refenvnt{n} :  \texttt{int}  }
  \label{rule:surface-type-int}
  \and
  \myinferrule[T-Var]
  { \Gamma \vdash^{  \overrightarrow{ \gamma_{{\mathrm{1}}} }   \refenvsym{,}  \gamma_{{\mathrm{2}}} }\token{wf}  \\
  \token{lookup} \, \refenvsym{(}  \Gamma  \refenvsym{,}  \refenvmv{x}  \refenvsym{)} = \token{Done} \, \refenvsym{(}  \refenvnt{A}  \refenvsym{,}  \gamma_{{\mathrm{3}}}  \refenvsym{)} \\
   \Gamma \vdash \gamma_{{\mathrm{3}}} \preceq \gamma_{{\mathrm{2}}} }
  { \Gamma \vdash^{  \overrightarrow{ \gamma_{{\mathrm{1}}} }   \refenvsym{,}  \gamma_{{\mathrm{2}}} } \refenvmv{x} : \refenvnt{A} }
  \label{rule:surface-type-var}
  \and
  \myinferrule[T-Rec]
  { \Gamma  \refenvsym{,}   \binder{ \refenvmv{f} }\mathord{:^{\binder{ \gamma_{{\mathrm{1}}} } } } \refenvnt{A_{{\mathrm{1}}}}  \rightarrow  \refenvnt{A_{{\mathrm{2}}}}   \refenvsym{,}   \binder{ \refenvmv{x} }\mathord{:^{\binder{ \gamma_{{\mathrm{2}}} } } } \refenvnt{A_{{\mathrm{1}}}}  \vdash^{  \overrightarrow{ \gamma_{{\mathrm{3}}} }   \refenvsym{,}  \gamma_{{\mathrm{2}}} } \refenvnt{e} : \refenvnt{A_{{\mathrm{2}}}}  \\
   \Gamma \vdash^{  \overrightarrow{ \gamma_{{\mathrm{3}}} }   \refenvsym{,}  \gamma_{{\mathrm{4}}} }\token{wf} }
  { \Gamma \vdash^{  \overrightarrow{ \gamma_{{\mathrm{3}}} }   \refenvsym{,}  \gamma_{{\mathrm{4}}} }  \token{rec}\ \binder{ \refenvmv{f} }(\binder{ \refenvmv{x} }).\  \refenvnt{e}  : \refenvnt{A_{{\mathrm{1}}}}  \rightarrow  \refenvnt{A_{{\mathrm{2}}}} }
  \label{rule:surface-type-rec}
  \and
  \myinferrule[T-Func]
  { \Gamma  \refenvsym{,}   \binder{ \refenvmv{x} }\mathord{:^{\binder{ \gamma_{{\mathrm{1}}} } } } \refenvnt{A_{{\mathrm{1}}}}  \vdash^{  \overrightarrow{ \gamma_{{\mathrm{2}}} }   \refenvsym{,}  \gamma_{{\mathrm{1}}} } \refenvnt{e} : \refenvnt{A_{{\mathrm{2}}}}  \\
  \gamma_{{\mathrm{1}}} \, \not\in \,  \token{FC}( \refenvnt{A_{{\mathrm{2}}}} )  \\
   \Gamma \vdash^{  \overrightarrow{ \gamma_{{\mathrm{2}}} }   \refenvsym{,}  \gamma_{{\mathrm{3}}} }\token{wf} }
  { \Gamma \vdash^{  \overrightarrow{ \gamma_{{\mathrm{2}}} }   \refenvsym{,}  \gamma_{{\mathrm{3}}} }  \lambda \binder{ \refenvmv{x} }.\  \refenvnt{e}  : \refenvnt{A_{{\mathrm{1}}}}  \rightarrow  \refenvnt{A_{{\mathrm{2}}}} }
  \label{rule:surface-type-func}
  \and
  \myinferrule[T-App]
  { \Gamma \vdash^{  \overrightarrow{ \gamma }^{+}  } \refenvnt{e_{{\mathrm{1}}}} : \refenvnt{A_{{\mathrm{1}}}}  \rightarrow  \refenvnt{A_{{\mathrm{2}}}}  \\
   \Gamma \vdash^{  \overrightarrow{ \gamma }^{+}  } \refenvnt{e_{{\mathrm{2}}}} : \refenvnt{A_{{\mathrm{1}}}} }
  { \Gamma \vdash^{  \overrightarrow{ \gamma }^{+}  }  \refenvnt{e_{{\mathrm{1}}}} \refenvnt{e_{{\mathrm{2}}}}  : \refenvnt{A_{{\mathrm{2}}}} }
  \label{rule:surface-type-app}
  \\
  \myinferrule[T-Quo]
  { \Gamma  \refenvsym{,}   \blacktriangleright ^{ \gamma_{{\mathrm{1}}} }  \vdash^{  \overrightarrow{ \gamma_{{\mathrm{2}}} }^{+}   \refenvsym{,}  \gamma_{{\mathrm{1}}} } \refenvnt{e} : \refenvnt{A} }
  { \Gamma \vdash^{  \overrightarrow{ \gamma_{{\mathrm{2}}} }^{+}  }  \langle  \refenvnt{e}  \rangle  :  \langle \refenvnt{A} \rangle^{ \gamma_{{\mathrm{1}}} }  }
  \label{rule:surface-type-quo}
  \and
  \myinferrule[T-Splice]
  { \Gamma \vdash^{  \overrightarrow{ \gamma_{{\mathrm{3}}} }   \refenvsym{,}    \delta _{ 0 }  ,\dotsc,  \delta _{ \refenvnt{k} }   }\token{wf}  \\
  \gamma_{{\mathrm{1}}} \, \not\in \,  \token{FC}( \refenvnt{A} ) \\
   \Gamma  \refenvsym{,}   \blacktriangleleft _{ \refenvnt{k} }^{\binder{ \gamma_{{\mathrm{1}}} } }  \vdash^{  \overrightarrow{ \gamma_{{\mathrm{3}}} }   \refenvsym{,}  \gamma_{{\mathrm{1}}} } \refenvnt{e} :  \langle \refenvnt{A} \rangle^{ \gamma_{{\mathrm{2}}} }   \\
   \Gamma \vdash \gamma_{{\mathrm{2}}} \preceq  \delta _{ \refenvnt{k} }   \\
  \gamma_{{\mathrm{1}}} \neq \gamma_{{\mathrm{2}}}}
  { \Gamma \vdash^{  \overrightarrow{ \gamma_{{\mathrm{3}}} }   \refenvsym{,}    \delta _{ 0 }  ,\dotsc,  \delta _{ \refenvnt{k} }   }  { \mathdollar }_{ \refenvnt{k} }\lbrace \refenvnt{e} \rbrace  : \refenvnt{A} }
  \label{rule:surface-type-splice}
  \\
  \myinferrule[T-Ref]
  { \Gamma \vdash^{  \overrightarrow{ \gamma }^{+}  } \refenvnt{e} : \refenvnt{A} }
  { \Gamma \vdash^{  \overrightarrow{ \gamma }^{+}  } \token{ref} \, \refenvsym{(}  \refenvnt{e}  \refenvsym{)} :  \refenvnt{A} \/\ \token{ref}  }
  \label{rule:surface-type-ref}
  \and
  \myinferrule[T-Set]
  { \Gamma \vdash^{  \overrightarrow{ \gamma }^{+}  } \refenvnt{e_{{\mathrm{1}}}} :  \refenvnt{A} \/\ \token{ref}   \\
   \Gamma \vdash^{  \overrightarrow{ \gamma }^{+}  } \refenvnt{e_{{\mathrm{2}}}} : \refenvnt{A} }
  { \Gamma \vdash^{  \overrightarrow{ \gamma }^{+}  }  \refenvnt{e_{{\mathrm{1}}}} \coloneqq \refenvnt{e_{{\mathrm{2}}}}  : \refenvnt{A} }
  \label{rule:surface-type-assign}
  \and
  \myinferrule[T-Get]
  { \Gamma \vdash^{  \overrightarrow{ \gamma }^{+}  } \refenvnt{e} :  \refenvnt{A} \/\ \token{ref}  }
  { \Gamma \vdash^{  \overrightarrow{ \gamma }^{+}  }  \token{deref}( \refenvnt{e} )  : \refenvnt{A} }
  \label{rule:surface-type-deref}
  \and
  \myinferrule[T-Polycls]
  { \Gamma  \refenvsym{,}   [  \varrho  ]^{\binder{ \gamma_{{\mathrm{1}}} } }  \vdash^{  \overrightarrow{ \delta }   \refenvsym{,}  \gamma_{{\mathrm{1}}} } {e_{I} } : \refenvnt{A}  \\
   \token{Dom}_{C}( \varrho )  \, \cap \,  \token{FC}( \refenvnt{A} )  = \emptyset \\
  \gamma_{{\mathrm{1}}} \, \not\in \,  \token{FC}( \refenvnt{A} )  \\
   \Gamma \vdash^{  \overrightarrow{ \delta }   \refenvsym{,}  \gamma_{{\mathrm{2}}} }\token{wf} }
  { \Gamma \vdash^{  \overrightarrow{ \delta }   \refenvsym{,}  \gamma_{{\mathrm{2}}} } {e_{I} } :  \forall  \varrho . \refenvnt{A}  }
  \label{rule:surface-type-polycls}
  \and
  \myinferrule[T-Appcls]
  { \Gamma \vdash^{  \overrightarrow{ \delta' }   \refenvsym{,}   \delta _{ 0 }  } \refenvnt{e} :  \forall    \binder{  \gamma _{ 1 }  }  \mathbin{:\succeq}    \gamma' _{ 1 }  ,\dotsc,\binder{  \gamma _{ \refenvnt{k} }  }  \mathbin{:\succeq}   \gamma'  _{ \refenvnt{k} }  . \refenvnt{A}   \\
   \Gamma \vdash  \gamma' _{ \refenvnt{i} }  \preceq  \delta _{ \refenvnt{i} }   \text{\ for\ }  1 \le \refenvnt{i} \le \refenvnt{k} \\
   \Gamma \vdash  \delta _{ \refenvnt{i}  \refenvsym{+}  1 }  \subseteq  \delta _{ \refenvnt{i} }   \text{\ for\ }  0 \le \refenvnt{i} < \refenvnt{k}}
  { \Gamma \vdash^{  \overrightarrow{ \delta' }   \refenvsym{,}   \delta _{ 0 }  } \refenvnt{e} : \refenvnt{A}  \refenvsym{[}    \gamma _{ 1 }  \coloneqq  \delta _{ 1 }  ,\dotsc,  \gamma _{ \refenvnt{k} }  \coloneqq  \delta _{ \refenvnt{k} }    \refenvsym{]} }
  \label{rule:surface-type-appcls}
\end{mathparpagebreakable}

Here, the auxiliary function $\token{lookup} \, \refenvsym{(}  \Gamma  \refenvsym{,}  \refenvmv{x}  \refenvsym{)}$ is defined as follows:
\begin{align*}
  \token{lookup} \, \refenvsym{(}  \varepsilon  \refenvsym{,}  \refenvmv{x}  \refenvsym{)} & =  \token{Fail}  \\
  \token{lookup} \, \refenvsym{(}  \refenvsym{(}  \Gamma  \refenvsym{,}   \binder{ \refenvmv{x} }\mathord{:^{\binder{ \gamma } } } \refenvnt{A}   \refenvsym{)}  \refenvsym{,}  \refenvmv{x}  \refenvsym{)} & = \token{Done} \, \refenvsym{(}  \refenvnt{A}  \refenvsym{,}  \gamma  \refenvsym{)} \\
  \token{lookup} \, \refenvsym{(}  \refenvsym{(}  \Gamma  \refenvsym{,}   \binder{ \refenvmv{y} }\mathord{:^{\binder{ \gamma } } } \refenvnt{A}   \refenvsym{)}  \refenvsym{,}  \refenvmv{x}  \refenvsym{)} & = \token{lookup} \, \refenvsym{(}  \Gamma  \refenvsym{,}  \refenvmv{x}  \refenvsym{)} \quad\text{ if } \refenvmv{x}\neq\refenvmv{y} \\
  \token{lookup} \, \refenvsym{(}  \refenvsym{(}  \Gamma  \refenvsym{,}   \blacktriangleright ^{ \gamma }   \refenvsym{)}  \refenvsym{,}  \refenvmv{x}  \refenvsym{)} & = \token{lookup} \, \refenvsym{(}  \Gamma  \refenvsym{,}  \refenvmv{x}  \refenvsym{)} \\
  \token{lookup} \, \refenvsym{(}  \refenvsym{(}  \Gamma  \refenvsym{,}   \blacktriangleleft _{ \refenvnt{k} }^{\binder{ \gamma } }   \refenvsym{)}  \refenvsym{,}  \refenvmv{x}  \refenvsym{)} & = \token{lookup} \, \refenvsym{(}  \Gamma  \refenvsym{,}  \refenvmv{x}  \refenvsym{)} \\
  \token{lookup} \, \refenvsym{(}  \refenvsym{(}  \Gamma  \refenvsym{,}   [  \varrho  ]^{\binder{ \gamma } }   \refenvsym{)}  \refenvsym{,}  \refenvmv{x}  \refenvsym{)} & = \token{lookup} \, \refenvsym{(}  \Gamma  \refenvsym{,}  \refenvmv{x}  \refenvsym{)}
\end{align*}

\subsection{Operational Semantics}
\subsubsection{Runtime Objects}
\begin{tabular}{cllcl}
  Value          & $\refenvnt{v}$     & $\in  \token{Val} $ & $\Coloneqq$ & $\refenvnt{n} \mid \token{clos} \, \refenvsym{(}  E  \refenvsym{,}  R  \refenvsym{,}    \lambda \binder{ \refenvmv{x} }.\  \refenvnt{e}  ^{ 0  }   \refenvsym{)} \mid \token{clos} \, \refenvsym{(}  E  \refenvsym{,}  R  \refenvsym{,}    \token{rec}\ \binder{ \refenvmv{f} }(\binder{ \refenvmv{x} }).\  \refenvnt{e}  ^{ 0  }   \refenvsym{)} \mid  \langle   \refenvnt{e} ^{ 0  }   \rangle  \mid \refenvmv{l}$ \\
  Reserved Names & $N$    & $\in  \token{RN} $    & $\Coloneqq$ & $ \varepsilon  \mid N  \refenvsym{,}  \refenvmv{x}$                                                                                   \\
  Value Environment     & $E$  & $\in  \token{VEnv} $  & $\Coloneqq$ & $ \varepsilon  \mid E  \refenvsym{,}  \refenvmv{x}  \coloneqq  \refenvnt{v}$                                                                              \\
  Renaming Environment  & $R$  & $\in  \token{REnv} $  & $\Coloneqq$ & $ \token{id}  \mid R  \refenvsym{,}  \refenvmv{x}  \coloneqq  \refenvmv{y}$                                                                            \\
  Store          & $S$ & $\in  \token{Store} $ & $\Coloneqq$ & $ \varepsilon  \mid S  \refenvsym{,}  \refenvmv{l}  \coloneqq  \refenvnt{v}$
\end{tabular}

\subsubsection{Notations for the Meta Language}
For the following definitions, we briefly introduce definitions and notations for the meta language. The meta language is a simple functional language with pattern matching.

We have the type $ \token{Result}( \tau ) $ with the following definition:
\[
  \token{type}\  \token{Result}( \tau ) \ \Coloneqq  \token{Timeout}  \mid  \token{Fail}  \mid  \token{Done} (\tau)
\]

Then, we introduce monadic notations for the type $ \token{Result}( \tau ) $ as follows:
\begin{align*}
   \token{return}  (M) \equiv\        &  \token{Done}  (M)                                                \\
  X \leftarrow M_1;\ M_2 \equiv\  & \token{match}\ M_1\ \token{with}                              \\
                                  & \token{case}\  \token{Timeout}  \Rightarrow  \token{Timeout}          \\
                                  & \token{case}\   \token{Fail}  \Rightarrow  \token{Fail}               \\
                                  & \token{case}\   \token{Done}  (R) \Rightarrow [ X \coloneq R ]M_2
\end{align*}

\subsubsection{Auxiliary Functions}
\begin{align*}
  \token{lookup} \, \refenvsym{(}  \varepsilon  \refenvsym{,}  \refenvmv{x}  \refenvsym{)}                & =  \token{Fail}                                                                      \\
  \token{lookup} \, \refenvsym{(}  \refenvsym{(}  E  \refenvsym{,}  \refenvmv{x}  \coloneqq  \refenvnt{v}  \refenvsym{)}  \refenvsym{,}  \refenvmv{x}  \refenvsym{)}         & = \token{Done} \, \refenvsym{(}  \refenvnt{v}  \refenvsym{)}                                                                  \\
  \token{lookup} \, \refenvsym{(}  \refenvsym{(}  E  \refenvsym{,}  \refenvmv{y}  \coloneqq  \refenvnt{v}  \refenvsym{)}  \refenvsym{,}  \refenvmv{x}  \refenvsym{)}         & = \token{lookup} \, \refenvsym{(}  E  \refenvsym{,}  \refenvmv{x}  \refenvsym{)} \quad\text{ if } \refenvmv{x}\neq\refenvmv{y}                             \\
                                        &                                                                                  \\
  \token{gensym} \, \refenvsym{(}  N  \refenvsym{)}                      & = \token{return} \, \refenvsym{(}  \refenvmv{x}  \refenvsym{)} \quad\text{ for some $\refenvmv{x}$ such that $\refenvmv{x} \, \not\in \, N$}         \\
                                        &                                                                                  \\
  \token{rename} \, \refenvsym{(}   \token{id}   \refenvsym{,}  \refenvmv{x}  \refenvsym{)}              & = \refenvmv{x}                                                                        \\
  \token{rename} \, \refenvsym{(}  \refenvsym{(}  R  \refenvsym{,}  \refenvmv{x}  \coloneqq  \refenvmv{y}  \refenvsym{)}  \refenvsym{,}  \refenvmv{x}  \refenvsym{)}          & = \refenvmv{y}                                                                        \\
  \token{rename} \, \refenvsym{(}  \refenvsym{(}  R  \refenvsym{,}  \refenvmv{x}  \coloneqq  \refenvmv{y}  \refenvsym{)}  \refenvsym{,}  \refenvmv{z}  \refenvsym{)}          & = \token{rename} \, \refenvsym{(}  R  \refenvsym{,}  \refenvmv{z}  \refenvsym{)} \quad\text{ if } \refenvmv{x}\neq\refenvmv{z}                           \\
                                        &                                                                                  \\
  \token{alloc} \, \refenvsym{(}  S  \refenvsym{)}                    & = \token{return} \, \refenvsym{(}  \refenvmv{l}  \refenvsym{)} \quad\text{ for some $\refenvmv{l}$ such that $\refenvmv{l} \, \not\in \,  \token{Dom}_{L}( S ) $} \\
                                        &                                                                                  \\
  \token{lookupStore}  \refenvsym{(}  \varepsilon  \refenvsym{,}  \refenvmv{l}  \refenvsym{)}           & =  \token{Fail}                                                                      \\
  \token{lookupStore}  \refenvsym{(}  \refenvsym{(}  S  \refenvsym{,}  \refenvmv{l}  \coloneqq  \refenvnt{v}  \refenvsym{)}  \refenvsym{,}  \refenvmv{l}  \refenvsym{)}   & = \token{Done} \, \refenvsym{(}  \refenvnt{v}  \refenvsym{)}                                                                  \\
  \token{lookupStore}  \refenvsym{(}  \refenvsym{(}  S  \refenvsym{,}  \refenvmv{l_{{\mathrm{1}}}}  \coloneqq  \refenvnt{v}  \refenvsym{)}  \refenvsym{,}  \refenvmv{l_{{\mathrm{2}}}}  \refenvsym{)} & = \token{lookupStore}  \refenvsym{(}  S  \refenvsym{,}  \refenvmv{l_{{\mathrm{2}}}}  \refenvsym{)} \quad\text{ if } \refenvmv{l_{{\mathrm{1}}}}\neq\refenvmv{l_{{\mathrm{2}}}}                 \\
                                        &                                                                                  \\
  \token{updateStore} \, \refenvsym{(}  \varepsilon  \refenvsym{,}  \refenvmv{l}  \refenvsym{,}  \refenvnt{v}  \refenvsym{)}             & =  \token{Fail}                                                                      \\
  \token{updateStore} \, \refenvsym{(}  \refenvsym{(}  S  \refenvsym{,}  \refenvmv{l}  \coloneqq  \refenvnt{v_{{\mathrm{1}}}}  \refenvsym{)}  \refenvsym{,}  \refenvmv{l}  \refenvsym{,}  \refenvnt{v_{{\mathrm{2}}}}  \refenvsym{)}   & = \token{return} \, \refenvsym{(}  S  \refenvsym{,}  \refenvmv{l}  \coloneqq  \refenvnt{v_{{\mathrm{2}}}}  \refenvsym{)}                                                     \\
  \token{updateStore} \, \refenvsym{(}  \refenvsym{(}  S  \refenvsym{,}  \refenvmv{l_{{\mathrm{1}}}}  \coloneqq  \refenvnt{v_{{\mathrm{1}}}}  \refenvsym{)}  \refenvsym{,}  \refenvmv{l_{{\mathrm{2}}}}  \refenvsym{,}  \refenvnt{v_{{\mathrm{2}}}}  \refenvsym{)} & = S_{{\mathrm{1}}}  \leftarrow \, \token{updateStore} \, \refenvsym{(}  S  \refenvsym{,}  \refenvmv{l_{{\mathrm{2}}}}  \refenvsym{,}  \refenvnt{v_{{\mathrm{2}}}}  \refenvsym{)}                                          \\
                                        & \quad \token{return} \, \refenvsym{(}  S_{{\mathrm{1}}}  \refenvsym{,}  \refenvmv{l_{{\mathrm{1}}}}  \coloneqq  \refenvnt{v_{{\mathrm{1}}}}  \refenvsym{)} \quad\text{if } \refenvmv{l_{{\mathrm{1}}}}\neq\refenvmv{l_{{\mathrm{2}}}}            \\
                                        &                                                                                  \\
  \token{toQuote} \, \refenvsym{(}   \langle   \refenvnt{e} ^{ 0  }   \rangle   \refenvsym{)}               & = \token{Done} \, \refenvsym{(}   \refenvnt{e} ^{ 0  }   \refenvsym{)}                                                                \\
  \token{toQuote} \, \refenvsym{(}  \refenvnt{v}  \refenvsym{)}                      & =  \token{Fail}  \text{ otherwise }                                                  \\
                                        &                                                                                  \\
  \token{toLocation} \, \refenvsym{(}  \refenvmv{l}  \refenvsym{)}                   & = \token{Done} \, \refenvsym{(}  \refenvmv{l}  \refenvsym{)}                                                                  \\
  \token{toLocation} \, \refenvsym{(}  \refenvnt{v}  \refenvsym{)}                   & =  \token{Fail}  \text{ otherwise }                                                  \\
\end{align*}



\subsubsection{Evaluator Functions}
{\small
  \begin{align*}
    \mathcal{V}^{\mathrm{rt} }  \refenvsym{(}   \refenvnt{e} ^{ 0  }   \refenvsym{,}  E  \refenvsym{,}  R  \refenvsym{,}  N  \refenvsym{,}  S  \refenvsym{,}  0  \refenvsym{)}             & =  \token{Timeout}                                                                                          \\
    \mathcal{V}^{\mathrm{rt} }  \refenvsym{(}  \refenvnt{n}  \refenvsym{,}  E  \refenvsym{,}  R  \refenvsym{,}  N  \refenvsym{,}  S  \refenvsym{,}   \refenvnt{k} ^{+}   \refenvsym{)}              & = \token{return} \, \refenvsym{(}  \refenvnt{n}  \refenvsym{,}  N  \refenvsym{,}  S  \refenvsym{)}                                                                           \\
    \mathcal{V}^{\mathrm{rt} }  \refenvsym{(}  \refenvmv{x}  \refenvsym{,}  E  \refenvsym{,}  R  \refenvsym{,}  N  \refenvsym{,}  S  \refenvsym{,}   \refenvnt{k} ^{+}   \refenvsym{)}              & = \refenvnt{v}  \leftarrow \, \token{lookup} \, \refenvsym{(}  E  \refenvsym{,}  \token{rename} \, \refenvsym{(}  R  \refenvsym{,}  \refenvmv{x}  \refenvsym{)}  \refenvsym{)};                                                              \\
                                                            & \quad \token{return} \, \refenvsym{(}  \refenvnt{v}  \refenvsym{,}  N  \refenvsym{,}  S  \refenvsym{)}                                                                       \\
    \mathcal{V}^{\mathrm{rt} }  \refenvsym{(}    \lambda \binder{ \refenvmv{x} }.\  \refenvnt{e}  ^{ 0  }   \refenvsym{,}  E  \refenvsym{,}  R  \refenvsym{,}  N  \refenvsym{,}  S  \refenvsym{,}   \refenvnt{k} ^{+}   \refenvsym{)}    & = \token{return} \, \refenvsym{(}  \token{clos} \, \refenvsym{(}  E  \refenvsym{,}  R  \refenvsym{,}    \lambda \binder{ \refenvmv{x} }.\  \refenvnt{e}  ^{ 0  }   \refenvsym{)}  \refenvsym{,}  N  \refenvsym{,}  S  \refenvsym{)}                                                   \\
    \mathcal{V}^{\mathrm{rt} }  \refenvsym{(}    \token{rec}\ \binder{ \refenvmv{f} }(\binder{ \refenvmv{x} }).\  \refenvnt{e}  ^{ 0  }   \refenvsym{,}  E  \refenvsym{,}  R  \refenvsym{,}  N  \refenvsym{,}  S  \refenvsym{,}   \refenvnt{k} ^{+}   \refenvsym{)} & = \token{return} \, \refenvsym{(}  \token{clos} \, \refenvsym{(}  E  \refenvsym{,}  R  \refenvsym{,}    \token{rec}\ \binder{ \refenvmv{f} }(\binder{ \refenvmv{x} }).\  \refenvnt{e}  ^{ 0  }   \refenvsym{)}  \refenvsym{,}  N  \refenvsym{,}  S  \refenvsym{)}                                                \\
    \mathcal{V}^{\mathrm{rt} }  \refenvsym{(}     \refenvnt{e_{{\mathrm{1}}}} ^{ 0  }  \refenvnt{e_{{\mathrm{2}}}}  ^{ 0  }   \refenvsym{,}  E  \refenvsym{,}  R  \refenvsym{,}  N  \refenvsym{,}  S  \refenvsym{,}   \refenvnt{k} ^{+}   \refenvsym{)}    & = \refenvsym{(}  \refenvnt{v_{{\mathrm{1}}}}  \refenvsym{,}  N_{{\mathrm{1}}}  \refenvsym{,}  S_{{\mathrm{1}}}  \refenvsym{)}  \leftarrow  \mathcal{V}^{\mathrm{rt} }  \refenvsym{(}   \refenvnt{e_{{\mathrm{1}}}} ^{ 0  }   \refenvsym{,}  E  \refenvsym{,}  R  \refenvsym{,}  N  \refenvsym{,}  S  \refenvsym{,}  \refenvnt{k}  \refenvsym{)};                                  \\
                                                            & \quad \refenvsym{(}  \refenvnt{v_{{\mathrm{2}}}}  \refenvsym{,}  N_{{\mathrm{2}}}  \refenvsym{,}  S_{{\mathrm{2}}}  \refenvsym{)}  \leftarrow  \mathcal{V}^{\mathrm{rt} }  \refenvsym{(}   \refenvnt{e_{{\mathrm{2}}}} ^{ 0  }   \refenvsym{,}  E  \refenvsym{,}  R  \refenvsym{,}  N_{{\mathrm{1}}}  \refenvsym{,}  S_{{\mathrm{1}}}  \refenvsym{,}  \refenvnt{k}  \refenvsym{)};                            \\
                                                            & \quad  \token{match}\  \refenvnt{v_{{\mathrm{1}}}} \ \token{with}                                                                                 \\
                                                            & \quad  \token{case}\  \token{clos} \, \refenvsym{(}  E'  \refenvsym{,}  R'  \refenvsym{,}    \lambda \binder{ \refenvmv{x} }.\  \refenvnt{e_{{\mathrm{3}}}}  ^{ 0  }   \refenvsym{)} \ \Rightarrow                                                      \\
                                                            & \qquad \refenvmv{y}  \leftarrow \, \token{gensym} \, \refenvsym{(}  N_{{\mathrm{2}}}  \refenvsym{)};                                                                           \\
                                                            & \qquad \mathcal{V}^{\mathrm{rt} }  \refenvsym{(}   \refenvnt{e_{{\mathrm{3}}}} ^{ 0  }   \refenvsym{,}  \refenvsym{(}  E'  \refenvsym{,}  \refenvmv{y}  \coloneqq  \refenvnt{v_{{\mathrm{2}}}}  \refenvsym{)}  \refenvsym{,}  \refenvsym{(}  R'  \refenvsym{,}  \refenvmv{x}  \coloneqq  \refenvmv{y}  \refenvsym{)}  \refenvsym{,}  \refenvsym{(}  N_{{\mathrm{2}}}  \refenvsym{,}  \refenvmv{y}  \refenvsym{)}  \refenvsym{,}  S_{{\mathrm{2}}}  \refenvsym{,}  \refenvnt{k}  \refenvsym{)}                          \\
                                                            & \quad  \token{case}\  \token{clos} \, \refenvsym{(}  E'  \refenvsym{,}  R'  \refenvsym{,}    \token{rec}\ \binder{ \refenvmv{f} }(\binder{ \refenvmv{x} }).\  \refenvnt{e_{{\mathrm{3}}}}  ^{ 0  }   \refenvsym{)} \ \Rightarrow                                                   \\
                                                            & \qquad g  \leftarrow \, \token{gensym} \, \refenvsym{(}  N_{{\mathrm{2}}}  \refenvsym{)};                                                                        \\
                                                            & \qquad \refenvmv{y}  \leftarrow \, \token{gensym} \, \refenvsym{(}  N_{{\mathrm{2}}}  \refenvsym{,}  g  \refenvsym{)};                                                                      \\
                                                            & \qquad \mathcal{V}^{\mathrm{rt} }  \refenvsym{(}   \refenvnt{e_{{\mathrm{3}}}} ^{ 0  }   \refenvsym{,}  \refenvsym{(}  E'  \refenvsym{,}  g  \coloneqq  \refenvnt{v_{{\mathrm{1}}}}  \refenvsym{,}  \refenvmv{y}  \coloneqq  \refenvnt{v_{{\mathrm{2}}}}  \refenvsym{)}  \refenvsym{,}  \refenvsym{(}  R'  \refenvsym{,}  \refenvmv{f}  \coloneqq  g  \refenvsym{,}  \refenvmv{x}  \coloneqq  \refenvmv{y}  \refenvsym{)}  \refenvsym{,}  \refenvsym{(}  N_{{\mathrm{2}}}  \refenvsym{,}  g  \refenvsym{,}  \refenvmv{y}  \refenvsym{)}  \refenvsym{,}  S_{{\mathrm{2}}}  \refenvsym{,}  \refenvnt{k}  \refenvsym{)} \\
                                                            & \quad  \token{case}\ \_ \Rightarrow \token{Fail}                                                                                 \\
                                                            & \quad  \token{end}                                                                                            \\
    \mathcal{V}^{\mathrm{rt} }  \refenvsym{(}   \langle   \refenvnt{e_{{\mathrm{1}}}} ^{ 1  }   \rangle   \refenvsym{,}  E  \refenvsym{,}  R  \refenvsym{,}  N  \refenvsym{,}  S  \refenvsym{,}   \refenvnt{k} ^{+}   \refenvsym{)}   & = \refenvsym{(}  \refenvnt{v_{{\mathrm{1}}}}  \refenvsym{,}  N_{{\mathrm{1}}}  \refenvsym{,}  S_{{\mathrm{1}}}  \refenvsym{)}  \leftarrow  \mathcal{V}^{\mathrm{fut} }  \refenvsym{(}  0  \refenvsym{,}   \refenvnt{e_{{\mathrm{1}}}} ^{ 1  }   \refenvsym{,}  E  \refenvsym{,}  R  \refenvsym{,}  N  \refenvsym{,}  S  \refenvsym{,}  \refenvnt{k}  \refenvsym{)};                                \\
                                                            & \quad \token{return} \, \refenvsym{(}   \langle  \refenvnt{v_{{\mathrm{1}}}}  \rangle   \refenvsym{,}  N_{{\mathrm{1}}}  \refenvsym{,}  S_{{\mathrm{1}}}  \refenvsym{)}                                                                   \\
    \mathcal{V}^{\mathrm{rt} }  \refenvsym{(}   { \mathdollar }_{ 0 }\lbrace  \refenvnt{e_{{\mathrm{1}}}} ^{ 0  }  \rbrace   \refenvsym{,}  E  \refenvsym{,}  R  \refenvsym{,}  N  \refenvsym{,}  S  \refenvsym{,}   \refenvnt{k} ^{+}   \refenvsym{)}
                                                            & = \refenvsym{(}  \refenvnt{v_{{\mathrm{1}}}}  \refenvsym{,}  N_{{\mathrm{1}}}  \refenvsym{,}  S_{{\mathrm{1}}}  \refenvsym{)}  \leftarrow  \mathcal{V}^{\mathrm{rt} }  \refenvsym{(}   \refenvnt{e_{{\mathrm{1}}}} ^{ 0  }   \refenvsym{,}  E  \refenvsym{,}  R  \refenvsym{,}  N  \refenvsym{,}  S  \refenvsym{,}  \refenvnt{k}  \refenvsym{)};                                 \\
                                                            & \quad  \refenvnt{e_{{\mathrm{2}}}} ^{ 0  }   \leftarrow \, \token{toQuote} \, \refenvsym{(}  \refenvnt{v_{{\mathrm{1}}}}  \refenvsym{)};                                                                        \\
                                                            & \quad \mathcal{V}^{\mathrm{rt} }  \refenvsym{(}   \refenvnt{e_{{\mathrm{2}}}} ^{ 0  }   \refenvsym{,}  E  \refenvsym{,}   \token{id}   \refenvsym{,}  N_{{\mathrm{1}}}  \refenvsym{,}  S_{{\mathrm{1}}}  \refenvsym{,}  \refenvnt{k}  \refenvsym{)}                                              \\
    \mathcal{V}^{\mathrm{rt} }  \refenvsym{(}  \token{ref} \, \refenvsym{(}   \refenvnt{e} ^{ 0  }   \refenvsym{)}  \refenvsym{,}  E  \refenvsym{,}  R  \refenvsym{,}  N  \refenvsym{,}  S  \refenvsym{,}   \refenvnt{k} ^{+}   \refenvsym{)}
                                                            & = \refenvsym{(}  \refenvnt{v_{{\mathrm{1}}}}  \refenvsym{,}  N_{{\mathrm{1}}}  \refenvsym{,}  S_{{\mathrm{1}}}  \refenvsym{)}  \leftarrow  \mathcal{V}^{\mathrm{rt} }  \refenvsym{(}   \refenvnt{e} ^{ 0  }   \refenvsym{,}  E  \refenvsym{,}  R  \refenvsym{,}  N  \refenvsym{,}  S  \refenvsym{,}  \refenvnt{k}  \refenvsym{)};                                  \\
                                                            & \quad \refenvmv{l}  \leftarrow \, \token{alloc} \, \refenvsym{(}  S_{{\mathrm{1}}}  \refenvsym{)};                                                                         \\
                                                            & \quad \token{return} \, \refenvsym{(}  \refenvmv{l}  \refenvsym{,}  N_{{\mathrm{1}}}  \refenvsym{,}  \refenvsym{(}  S_{{\mathrm{1}}}  \refenvsym{,}  \refenvmv{l}  \coloneqq  \refenvnt{v_{{\mathrm{1}}}}  \refenvsym{)}  \refenvsym{)};                                                           \\
    \mathcal{V}^{\mathrm{rt} }  \refenvsym{(}    \refenvnt{e_{{\mathrm{1}}}} ^{ 0  }  \coloneqq  \refenvnt{e_{{\mathrm{2}}}} ^{ 0  }    \refenvsym{,}  E  \refenvsym{,}  R  \refenvsym{,}  N  \refenvsym{,}  S  \refenvsym{,}   \refenvnt{k} ^{+}   \refenvsym{)}
                                                            & = \refenvsym{(}  \refenvnt{v_{{\mathrm{1}}}}  \refenvsym{,}  N_{{\mathrm{1}}}  \refenvsym{,}  S_{{\mathrm{1}}}  \refenvsym{)}  \leftarrow  \mathcal{V}^{\mathrm{rt} }  \refenvsym{(}   \refenvnt{e_{{\mathrm{1}}}} ^{ 0  }   \refenvsym{,}  E  \refenvsym{,}  R  \refenvsym{,}  N  \refenvsym{,}  S  \refenvsym{,}  \refenvnt{k}  \refenvsym{)};                                 \\
                                                            & \quad \refenvsym{(}  \refenvnt{v_{{\mathrm{2}}}}  \refenvsym{,}  N_{{\mathrm{2}}}  \refenvsym{,}  S_{{\mathrm{2}}}  \refenvsym{)}  \leftarrow  \mathcal{V}^{\mathrm{rt} }  \refenvsym{(}   \refenvnt{e_{{\mathrm{2}}}} ^{ 0  }   \refenvsym{,}  E  \refenvsym{,}  R  \refenvsym{,}  N_{{\mathrm{1}}}  \refenvsym{,}  S_{{\mathrm{1}}}  \refenvsym{,}  \refenvnt{k}  \refenvsym{)};                           \\
                                                            & \quad \refenvmv{l}  \leftarrow \, \token{toLocation} \, \refenvsym{(}  \refenvnt{v_{{\mathrm{1}}}}  \refenvsym{)};                                                                        \\
                                                            & \quad S_{{\mathrm{3}}}  \leftarrow \, \token{updateStore} \, \refenvsym{(}  S_{{\mathrm{2}}}  \refenvsym{,}  \refenvmv{l}  \refenvsym{,}  \refenvnt{v_{{\mathrm{2}}}}  \refenvsym{)};                                                            \\
                                                            & \quad \token{return} \, \refenvsym{(}  \refenvnt{v_{{\mathrm{2}}}}  \refenvsym{,}  N_{{\mathrm{2}}}  \refenvsym{,}  S_{{\mathrm{3}}}  \refenvsym{)}                                                                    \\
    \mathcal{V}^{\mathrm{rt} }  \refenvsym{(}   \token{deref}(  \refenvnt{e} ^{ 0  }  )   \refenvsym{,}  E  \refenvsym{,}  R  \refenvsym{,}  N  \refenvsym{,}  S  \refenvsym{,}   \refenvnt{k} ^{+}   \refenvsym{)}
                                                            & = \refenvsym{(}  \refenvnt{v_{{\mathrm{1}}}}  \refenvsym{,}  N_{{\mathrm{1}}}  \refenvsym{,}  S_{{\mathrm{1}}}  \refenvsym{)}  \leftarrow  \mathcal{V}^{\mathrm{rt} }  \refenvsym{(}   \refenvnt{e} ^{ 0  }   \refenvsym{,}  E  \refenvsym{,}  R  \refenvsym{,}  N  \refenvsym{,}  S  \refenvsym{,}  \refenvnt{k}  \refenvsym{)};                                  \\
                                                            & \quad \refenvmv{l}  \leftarrow \, \token{toLocation} \, \refenvsym{(}  \refenvnt{v_{{\mathrm{1}}}}  \refenvsym{)};                                                                        \\
                                                            & \quad \refenvnt{v_{{\mathrm{2}}}}  \leftarrow  \token{lookupStore}  \refenvsym{(}  S_{{\mathrm{1}}}  \refenvsym{,}  \refenvmv{l}  \refenvsym{)};                                                              \\
                                                            & \quad \token{return} \, \refenvsym{(}  \refenvnt{v_{{\mathrm{2}}}}  \refenvsym{,}  N_{{\mathrm{1}}}  \refenvsym{,}  S_{{\mathrm{1}}}  \refenvsym{)}
  \end{align*}

  \begin{align*}
    \mathcal{V}^{\mathrm{fut} }  \refenvsym{(}  \refenvnt{k_{{\mathrm{1}}}}  \refenvsym{,}   \refenvnt{e} ^{  \refenvnt{k_{{\mathrm{1}}}} ^{+}   }   \refenvsym{,}  E  \refenvsym{,}  R  \refenvsym{,}  N  \refenvsym{,}  S  \refenvsym{,}  0  \refenvsym{)}                   & =  \token{Timeout}                                                                                                    \\
    \mathcal{V}^{\mathrm{fut} }  \refenvsym{(}  \refenvnt{k_{{\mathrm{1}}}}  \refenvsym{,}  \refenvnt{n}  \refenvsym{,}  E  \refenvsym{,}  R  \refenvsym{,}  N  \refenvsym{,}  S  \refenvsym{,}   \refenvnt{k_{{\mathrm{2}}}} ^{+}   \refenvsym{)}                     & = \token{return} \, \refenvsym{(}  \refenvnt{n}  \refenvsym{,}  N  \refenvsym{,}  S  \refenvsym{)}                                                                                      \\
    \mathcal{V}^{\mathrm{fut} }  \refenvsym{(}  \refenvnt{k_{{\mathrm{1}}}}  \refenvsym{,}  \refenvmv{x}  \refenvsym{,}  E  \refenvsym{,}  R  \refenvsym{,}  N  \refenvsym{,}  S  \refenvsym{,}   \refenvnt{k_{{\mathrm{2}}}} ^{+}   \refenvsym{)}                     & = \token{return} \, \refenvsym{(}  \token{rename} \, \refenvsym{(}  R  \refenvsym{,}  \refenvmv{x}  \refenvsym{)}  \refenvsym{,}  N  \refenvsym{,}  S  \refenvsym{)}                                                                         \\
    \mathcal{V}^{\mathrm{fut} }  \refenvsym{(}  \refenvnt{k_{{\mathrm{1}}}}  \refenvsym{,}    \lambda \binder{ \refenvmv{x} }.\  \refenvnt{e_{{\mathrm{1}}}}  ^{  \refenvnt{k_{{\mathrm{1}}}} ^{+}   }   \refenvsym{,}  E  \refenvsym{,}  R  \refenvsym{,}  N  \refenvsym{,}  S  \refenvsym{,}   \refenvnt{k_{{\mathrm{2}}}} ^{+}   \refenvsym{)}        & = \refenvmv{y}  \leftarrow \, \token{gensym} \, \refenvsym{(}  N  \refenvsym{)};                                                                                          \\
                                                                        & \quad \refenvsym{(}   \refenvnt{e_{{\mathrm{2}}}} ^{ \refenvnt{k_{{\mathrm{1}}}}  }   \refenvsym{,}  N_{{\mathrm{1}}}  \refenvsym{,}  S_{{\mathrm{1}}}  \refenvsym{)}  \leftarrow  \mathcal{V}^{\mathrm{fut} }  \refenvsym{(}  \refenvnt{k_{{\mathrm{1}}}}  \refenvsym{,}   \refenvnt{e_{{\mathrm{1}}}} ^{  \refenvnt{k_{{\mathrm{1}}}} ^{+}   }   \refenvsym{,}  E  \refenvsym{,}  \refenvsym{(}  R  \refenvsym{,}  \refenvmv{x}  \coloneqq  \refenvmv{y}  \refenvsym{)}  \refenvsym{,}  \refenvsym{(}  N  \refenvsym{,}  \refenvmv{y}  \refenvsym{)}  \refenvsym{,}  S  \refenvsym{,}  \refenvnt{k_{{\mathrm{2}}}}  \refenvsym{)};                \\
                                                                        & \quad \token{return} \, \refenvsym{(}    \lambda \binder{ \refenvmv{y} }.\  \refenvnt{e_{{\mathrm{2}}}}  ^{ \refenvnt{k_{{\mathrm{1}}}}  }   \refenvsym{,}  N_{{\mathrm{1}}}  \refenvsym{,}  S_{{\mathrm{1}}}  \refenvsym{)}                                                                      \\
    \mathcal{V}^{\mathrm{fut} }  \refenvsym{(}  \refenvnt{k_{{\mathrm{1}}}}  \refenvsym{,}    \token{rec}\ \binder{ \refenvmv{f} }(\binder{ \refenvmv{x} }).\  \refenvnt{e_{{\mathrm{1}}}}  ^{  \refenvnt{k_{{\mathrm{1}}}} ^{+}   }   \refenvsym{,}  E  \refenvsym{,}  R  \refenvsym{,}  N  \refenvsym{,}  S  \refenvsym{,}   \refenvnt{k_{{\mathrm{2}}}} ^{+}   \refenvsym{)}     & = g  \leftarrow \, \token{gensym} \, \refenvsym{(}  N  \refenvsym{)};                                                                                       \\
                                                                        & \quad \refenvmv{y}  \leftarrow \, \token{gensym} \, \refenvsym{(}  N  \refenvsym{,}  g  \refenvsym{)};                                                                                 \\
                                                                        & \quad \refenvsym{(}   \refenvnt{e_{{\mathrm{2}}}} ^{ \refenvnt{k_{{\mathrm{1}}}}  }   \refenvsym{,}  N_{{\mathrm{1}}}  \refenvsym{,}  S_{{\mathrm{1}}}  \refenvsym{)}  \leftarrow  \mathcal{V}^{\mathrm{fut} }  \refenvsym{(}  \refenvnt{k_{{\mathrm{1}}}}  \refenvsym{,}   \refenvnt{e_{{\mathrm{1}}}} ^{  \refenvnt{k_{{\mathrm{1}}}} ^{+}   }   \refenvsym{,}  E  \refenvsym{,}  \refenvsym{(}  R  \refenvsym{,}  \refenvmv{f}  \coloneqq  g  \refenvsym{,}  \refenvmv{x}  \coloneqq  \refenvmv{y}  \refenvsym{)}  \refenvsym{,}  \refenvsym{(}  N  \refenvsym{,}  g  \refenvsym{,}  \refenvmv{y}  \refenvsym{)}  \refenvsym{,}  S  \refenvsym{,}  \refenvnt{k_{{\mathrm{2}}}}  \refenvsym{)}; \\
                                                                        & \quad \token{return} \, \refenvsym{(}    \token{rec}\ \binder{ g }(\binder{ \refenvmv{y} }).\  \refenvnt{e_{{\mathrm{2}}}}  ^{ \refenvnt{k_{{\mathrm{1}}}}  }   \refenvsym{,}  N_{{\mathrm{1}}}  \refenvsym{,}  S_{{\mathrm{1}}}  \refenvsym{)}                                                                \\
    \mathcal{V}^{\mathrm{fut} }  \refenvsym{(}  \refenvnt{k_{{\mathrm{1}}}}  \refenvsym{,}     \refenvnt{e_{{\mathrm{1}}}} ^{  \refenvnt{k_{{\mathrm{1}}}} ^{+}   }  \refenvnt{e_{{\mathrm{2}}}}  ^{  \refenvnt{k_{{\mathrm{1}}}} ^{+}   }   \refenvsym{,}  E  \refenvsym{,}  R  \refenvsym{,}  N  \refenvsym{,}  S  \refenvsym{,}   \refenvnt{k_{{\mathrm{2}}}} ^{+}   \refenvsym{)}       & = \refenvsym{(}   \refenvnt{e_{{\mathrm{3}}}} ^{ \refenvnt{k_{{\mathrm{1}}}}  }   \refenvsym{,}  N_{{\mathrm{1}}}  \refenvsym{,}  S_{{\mathrm{1}}}  \refenvsym{)}  \leftarrow  \mathcal{V}^{\mathrm{fut} }  \refenvsym{(}  \refenvnt{k_{{\mathrm{1}}}}  \refenvsym{,}   \refenvnt{e_{{\mathrm{1}}}} ^{  \refenvnt{k_{{\mathrm{1}}}} ^{+}   }   \refenvsym{,}  E  \refenvsym{,}  R  \refenvsym{,}  N  \refenvsym{,}  S  \refenvsym{,}  \refenvnt{k_{{\mathrm{2}}}}  \refenvsym{)};                                 \\
                                                                        & \quad \refenvsym{(}   \refenvnt{e_{{\mathrm{4}}}} ^{ \refenvnt{k_{{\mathrm{1}}}}  }   \refenvsym{,}  N_{{\mathrm{2}}}  \refenvsym{,}  S_{{\mathrm{2}}}  \refenvsym{)}  \leftarrow  \mathcal{V}^{\mathrm{fut} }  \refenvsym{(}  \refenvnt{k_{{\mathrm{1}}}}  \refenvsym{,}   \refenvnt{e_{{\mathrm{2}}}} ^{  \refenvnt{k_{{\mathrm{1}}}} ^{+}   }   \refenvsym{,}  E  \refenvsym{,}  R  \refenvsym{,}  N_{{\mathrm{1}}}  \refenvsym{,}  S_{{\mathrm{1}}}  \refenvsym{,}  \refenvnt{k_{{\mathrm{2}}}}  \refenvsym{)};                           \\
                                                                        & \quad \token{return} \, \refenvsym{(}     \refenvnt{e_{{\mathrm{3}}}} ^{ \refenvnt{k_{{\mathrm{1}}}}  }  \refenvnt{e_{{\mathrm{4}}}}  ^{ \refenvnt{k_{{\mathrm{1}}}}  }   \refenvsym{,}  N_{{\mathrm{2}}}  \refenvsym{,}  S_{{\mathrm{2}}}  \refenvsym{)}                                                                      \\
    \mathcal{V}^{\mathrm{fut} }  \refenvsym{(}  \refenvnt{k_{{\mathrm{1}}}}  \refenvsym{,}   \langle   \refenvnt{e_{{\mathrm{1}}}} ^{  \refenvnt{k_{{\mathrm{1}}}}  \refenvsym{+}  2   }   \rangle   \refenvsym{,}  E  \refenvsym{,}  R  \refenvsym{,}  N  \refenvsym{,}  S  \refenvsym{,}   \refenvnt{k_{{\mathrm{2}}}} ^{+}   \refenvsym{)}    & = \refenvsym{(}   \refenvnt{e_{{\mathrm{2}}}} ^{  \refenvnt{k_{{\mathrm{1}}}} ^{+}   }   \refenvsym{,}  N_{{\mathrm{1}}}  \refenvsym{,}  S_{{\mathrm{1}}}  \refenvsym{)}  \leftarrow  \mathcal{V}^{\mathrm{fut} }  \refenvsym{(}   \refenvnt{k_{{\mathrm{1}}}} ^{+}   \refenvsym{,}   \refenvnt{e_{{\mathrm{1}}}} ^{  \refenvnt{k_{{\mathrm{1}}}}  \refenvsym{+}  2   }   \refenvsym{,}  E  \refenvsym{,}  R  \refenvsym{,}  N  \refenvsym{,}  S  \refenvsym{,}  \refenvnt{k_{{\mathrm{2}}}}  \refenvsym{)};                          \\
                                                                        & \quad \token{return} \, \refenvsym{(}   \langle   \refenvnt{e_{{\mathrm{2}}}} ^{  \refenvnt{k_{{\mathrm{1}}}} ^{+}   }   \rangle   \refenvsym{,}  N_{{\mathrm{1}}}  \refenvsym{,}  S_{{\mathrm{1}}}  \refenvsym{)}                                                                       \\
    \mathcal{V}^{\mathrm{fut} }  \refenvsym{(}  \refenvnt{k_{{\mathrm{1}}}}  \refenvsym{,}   { \mathdollar }_{  \refenvnt{k_{{\mathrm{1}}}} ^{+}  }\lbrace  \refenvnt{e_{{\mathrm{1}}}} ^{ 0  }  \rbrace   \refenvsym{,}  E  \refenvsym{,}  R  \refenvsym{,}  N  \refenvsym{,}  S  \refenvsym{,}   \refenvnt{k_{{\mathrm{2}}}} ^{+}   \refenvsym{)}
                                                                        & = \refenvsym{(}  \refenvnt{v_{{\mathrm{1}}}}  \refenvsym{,}  N_{{\mathrm{1}}}  \refenvsym{,}  S_{{\mathrm{1}}}  \refenvsym{)}  \leftarrow  \mathcal{V}^{\mathrm{rt} }  \refenvsym{(}   \refenvnt{e_{{\mathrm{1}}}} ^{ 0  }   \refenvsym{,}  E  \refenvsym{,}  R  \refenvsym{,}  N  \refenvsym{,}  S  \refenvsym{,}  \refenvnt{k_{{\mathrm{2}}}}  \refenvsym{)};                                        \\
                                                                        & \quad  \refenvnt{e_{{\mathrm{2}}}} ^{ 0  }   \leftarrow \, \token{toQuote} \, \refenvsym{(}  \refenvnt{v_{{\mathrm{1}}}}  \refenvsym{)};                                                                                \\
                                                                        & \quad \token{return} \, \refenvsym{(}   \refenvnt{e_{{\mathrm{2}}}} ^{ 0  }   \refenvsym{,}  N_{{\mathrm{1}}}  \refenvsym{,}  S_{{\mathrm{1}}}  \refenvsym{)}; \quad\text{(Note that $ \refenvnt{e_{{\mathrm{2}}}} ^{ 0  }  \, \in \,  \token{Exp}^{ \refenvnt{k_{{\mathrm{1}}}} } $)}                          \\
    \mathcal{V}^{\mathrm{fut} }  \refenvsym{(}  \refenvnt{k_{{\mathrm{1}}}}  \refenvsym{,}   { \mathdollar }_{ \refenvnt{k_{{\mathrm{2}}}} }\lbrace  \refenvnt{e_{{\mathrm{1}}}} ^{  \refenvnt{k_{{\mathrm{1}}}} ^{+}   \refenvsym{-}  \refenvnt{k_{{\mathrm{2}}}}  }  \rbrace   \refenvsym{,}  E  \refenvsym{,}  R  \refenvsym{,}  N  \refenvsym{,}  S  \refenvsym{,}   \refenvnt{k_{{\mathrm{3}}}} ^{+}   \refenvsym{)}
                                                                        & \text{ (where $\refenvnt{k_{{\mathrm{1}}}} \ge \refenvnt{k_{{\mathrm{2}}}}$ ) }                                                                       \\
                                                                        & = \refenvsym{(}   \refenvnt{e_{{\mathrm{2}}}} ^{ \refenvnt{k_{{\mathrm{1}}}}  \refenvsym{-}  \refenvnt{k_{{\mathrm{2}}}}  }   \refenvsym{,}  N_{{\mathrm{1}}}  \refenvsym{,}  S_{{\mathrm{1}}}  \refenvsym{)}  \leftarrow  \mathcal{V}^{\mathrm{fut} }  \refenvsym{(}  \refenvnt{k_{{\mathrm{1}}}}  \refenvsym{-}  \refenvnt{k_{{\mathrm{2}}}}  \refenvsym{,}   \refenvnt{e_{{\mathrm{1}}}} ^{  \refenvnt{k_{{\mathrm{1}}}} ^{+}   \refenvsym{-}  \refenvnt{k_{{\mathrm{2}}}}  }   \refenvsym{,}  E  \refenvsym{,}  R  \refenvsym{,}  N  \refenvsym{,}  S  \refenvsym{,}  \refenvnt{k_{{\mathrm{3}}}}  \refenvsym{)};                       \\
                                                                        & \quad \token{return} \, \refenvsym{(}   { \mathdollar }_{ \refenvnt{k_{{\mathrm{2}}}} }\lbrace  \refenvnt{e_{{\mathrm{2}}}} ^{ \refenvnt{k_{{\mathrm{1}}}}  \refenvsym{-}  \refenvnt{k_{{\mathrm{2}}}}  }  \rbrace   \refenvsym{,}  N_{{\mathrm{1}}}  \refenvsym{,}  S_{{\mathrm{1}}}  \refenvsym{)}                                                               \\
    \mathcal{V}^{\mathrm{fut} }  \refenvsym{(}  \refenvnt{k_{{\mathrm{1}}}}  \refenvsym{,}  \token{ref} \, \refenvsym{(}   \refenvnt{e_{{\mathrm{1}}}} ^{  \refenvnt{k_{{\mathrm{1}}}} ^{+}   }   \refenvsym{)}  \refenvsym{,}  E  \refenvsym{,}  R  \refenvsym{,}  N  \refenvsym{,}  S  \refenvsym{,}   \refenvnt{k_{{\mathrm{2}}}} ^{+}   \refenvsym{)}         & = \refenvsym{(}   \refenvnt{e_{{\mathrm{2}}}} ^{ \refenvnt{k_{{\mathrm{1}}}}  }   \refenvsym{,}  N_{{\mathrm{1}}}  \refenvsym{,}  S_{{\mathrm{1}}}  \refenvsym{)}  \leftarrow  \mathcal{V}^{\mathrm{fut} }  \refenvsym{(}  \refenvnt{k_{{\mathrm{1}}}}  \refenvsym{,}   \refenvnt{e} ^{  \refenvnt{k_{{\mathrm{1}}}} ^{+}   }   \refenvsym{,}  E  \refenvsym{,}  R  \refenvsym{,}  N  \refenvsym{,}  S  \refenvsym{,}  \refenvnt{k_{{\mathrm{2}}}}  \refenvsym{)};                                \\
                                                                        & \quad \token{return} \, \refenvsym{(}  \token{ref} \, \refenvsym{(}   \refenvnt{e_{{\mathrm{2}}}} ^{ \refenvnt{k_{{\mathrm{1}}}}  }   \refenvsym{)}  \refenvsym{,}  N_{{\mathrm{1}}}  \refenvsym{,}  S_{{\mathrm{1}}}  \refenvsym{)}                                                                    \\
    \mathcal{V}^{\mathrm{fut} }  \refenvsym{(}  \refenvnt{k_{{\mathrm{1}}}}  \refenvsym{,}    \refenvnt{e_{{\mathrm{1}}}} ^{  \refenvnt{k_{{\mathrm{1}}}} ^{+}   }  \coloneqq  \refenvnt{e_{{\mathrm{2}}}} ^{  \refenvnt{k_{{\mathrm{1}}}} ^{+}   }    \refenvsym{,}  E  \refenvsym{,}  R  \refenvsym{,}  N  \refenvsym{,}  S  \refenvsym{,}   \refenvnt{k_{{\mathrm{2}}}} ^{+}   \refenvsym{)} & = \refenvsym{(}   \refenvnt{e_{{\mathrm{3}}}} ^{ \refenvnt{k_{{\mathrm{1}}}}  }   \refenvsym{,}  N_{{\mathrm{1}}}  \refenvsym{,}  S_{{\mathrm{1}}}  \refenvsym{)}  \leftarrow  \mathcal{V}^{\mathrm{fut} }  \refenvsym{(}  \refenvnt{k_{{\mathrm{1}}}}  \refenvsym{,}   \refenvnt{e_{{\mathrm{1}}}} ^{  \refenvnt{k_{{\mathrm{1}}}} ^{+}   }   \refenvsym{,}  E  \refenvsym{,}  R  \refenvsym{,}  N  \refenvsym{,}  S  \refenvsym{,}  \refenvnt{k_{{\mathrm{2}}}}  \refenvsym{)};                              \\
                                                                        & \quad \refenvsym{(}   \refenvnt{e_{{\mathrm{4}}}} ^{ \refenvnt{k_{{\mathrm{1}}}}  }   \refenvsym{,}  N_{{\mathrm{2}}}  \refenvsym{,}  S_{{\mathrm{2}}}  \refenvsym{)}  \leftarrow  \mathcal{V}^{\mathrm{fut} }  \refenvsym{(}  \refenvnt{k_{{\mathrm{1}}}}  \refenvsym{,}   \refenvnt{e_{{\mathrm{2}}}} ^{  \refenvnt{k_{{\mathrm{1}}}} ^{+}   }   \refenvsym{,}  E  \refenvsym{,}  R  \refenvsym{,}  N_{{\mathrm{1}}}  \refenvsym{,}  S_{{\mathrm{1}}}  \refenvsym{,}  \refenvnt{k_{{\mathrm{2}}}}  \refenvsym{)};                         \\
                                                                        & \quad \token{return} \, \refenvsym{(}    \refenvnt{e_{{\mathrm{3}}}} ^{ \refenvnt{k_{{\mathrm{1}}}}  }  \coloneqq  \refenvnt{e_{{\mathrm{4}}}} ^{ \refenvnt{k_{{\mathrm{1}}}}  }    \refenvsym{,}  N_{{\mathrm{2}}}  \refenvsym{,}  S_{{\mathrm{2}}}  \refenvsym{)}                                                              \\
    \mathcal{V}^{\mathrm{fut} }  \refenvsym{(}  \refenvnt{k_{{\mathrm{1}}}}  \refenvsym{,}   \token{deref}(  \refenvnt{e_{{\mathrm{1}}}} ^{  \refenvnt{k_{{\mathrm{1}}}} ^{+}   }  )   \refenvsym{,}  E  \refenvsym{,}  R  \refenvsym{,}  N  \refenvsym{,}  S  \refenvsym{,}   \refenvnt{k_{{\mathrm{2}}}} ^{+}   \refenvsym{)}        & = \refenvsym{(}   \refenvnt{e_{{\mathrm{2}}}} ^{ \refenvnt{k_{{\mathrm{1}}}}  }   \refenvsym{,}  N_{{\mathrm{1}}}  \refenvsym{,}  S_{{\mathrm{1}}}  \refenvsym{)}  \leftarrow  \mathcal{V}^{\mathrm{fut} }  \refenvsym{(}  \refenvnt{k_{{\mathrm{1}}}}  \refenvsym{,}   \refenvnt{e_{{\mathrm{1}}}} ^{  \refenvnt{k_{{\mathrm{1}}}} ^{+}   }   \refenvsym{,}  E  \refenvsym{,}  R  \refenvsym{,}  N  \refenvsym{,}  S  \refenvsym{,}  \refenvnt{k_{{\mathrm{2}}}}  \refenvsym{)};                              \\
                                                                        & \quad \token{return} \, \refenvsym{(}   \token{deref}(  \refenvnt{e_{{\mathrm{2}}}} ^{ \refenvnt{k_{{\mathrm{1}}}}  }  )   \refenvsym{,}  N_{{\mathrm{1}}}  \refenvsym{,}  S_{{\mathrm{1}}}  \refenvsym{)}                                                                    \\
  \end{align*}
}

\subsection{Runtime Typing}
\subsubsection{Objects for Runtime Typing}
\begin{tabular}{clcl}
  \textbf{Reserved Names Typing} & $\Psi$ & $\Coloneqq$ & $ \varepsilon  \mid \Psi  \refenvsym{,}   \binder{ \refenvmv{x} }: \refenvnt{A} \mathrel{@}\binder{ \gamma_{{\mathrm{1}}} } \mathbin{:\succeq} \gamma_{{\mathrm{2}}}  \mid \Psi  \refenvsym{,}   \binder{ \gamma_{{\mathrm{1}}} }( \mathbin{:\succeq} \; \gamma_{{\mathrm{2}}}  /  \mathbin{:\supseteq} \; \gamma_{{\mathrm{3}}} )  \mid \Psi  \refenvsym{,}   [    \binder{  \gamma _{ 0 }  }  \mathbin{:\succeq}    \delta _{ 0 }  ,\dotsc,\binder{  \gamma _{ \refenvnt{k} }  }  \mathbin{:\succeq}   \delta  _{ \refenvnt{k} }   ] $ \\
  \textbf{Location Typing}       & $\Theta$  & $\Coloneqq$ & $ \varepsilon  \mid \Theta  \refenvsym{,}   \refenvmv{l} : \refenvnt{A} $
\end{tabular}

\begin{definition}
  \begin{enumerate}
    \item We write $ \Psi_{{\mathrm{1}}} \subseteq \Psi_{{\mathrm{2}}} $ if there exists $\Psi_{{\mathrm{3}}}$ such that $\Psi_{{\mathrm{1}}}  \refenvsym{,}  \Psi_{{\mathrm{3}}} = \Psi_{{\mathrm{2}}}$.
    \item We write $ \Theta_{{\mathrm{1}}} \subseteq \Theta_{{\mathrm{2}}} $ if there exists $\Theta_{{\mathrm{3}}}$ such that $\Theta_{{\mathrm{1}}}  \refenvsym{,}  \Theta_{{\mathrm{3}}} = \Theta_{{\mathrm{2}}}$.
  \end{enumerate}
\end{definition}

\begin{definition}[Classifier Domain of Reserved Names Typing]
  $ \token{Dom}_{C}( \Psi ) $ returns the set of classifiers declared in $\Psi$, and is defined as follows.
  \begin{align*}
     \token{Dom}_{C}( \varepsilon )                 & = \refenvsym{\{}   \exclam   \refenvsym{\}}                 \\
     \token{Dom}_{C}( \Psi  \refenvsym{,}   \binder{ \gamma_{{\mathrm{1}}} }( \mathbin{:\succeq} \; \gamma_{{\mathrm{2}}}  /  \mathbin{:\supseteq} \; \gamma_{{\mathrm{3}}} )  )  & =  \token{Dom}_{C}( \Psi )  \, \cup \, \refenvsym{\{}  \gamma_{{\mathrm{1}}}  \refenvsym{\}} \\
     \token{Dom}_{C}( \Psi  \refenvsym{,}   \binder{ \refenvmv{x} }: \refenvnt{A} \mathrel{@}\binder{ \gamma_{{\mathrm{1}}} } \mathbin{:\succeq} \gamma_{{\mathrm{2}}}  )       & =  \token{Dom}_{C}( \Psi )  \, \cup \, \refenvsym{\{}  \gamma_{{\mathrm{1}}}  \refenvsym{\}} \\
     \token{Dom}_{C}( \Psi  \refenvsym{,}   [    \binder{  \gamma _{ 0 }  }  \mathbin{:\succeq}    \delta _{ 0 }  ,\dotsc,\binder{  \gamma _{ \refenvnt{k} }  }  \mathbin{:\succeq}   \delta  _{ \refenvnt{k} }   ]  )  & =  \token{Dom}_{C}( \Psi )  \, \cup \, \refenvsym{\{}    \gamma _{ 0 }  ,\dotsc,  \gamma _{ \refenvnt{k} }    \refenvsym{\}}
  \end{align*}
\end{definition}

\begin{definition}[Variable Domain of Reserved Names Typing]
  $ \token{Dom}_{V}( \Psi ) $ returns the set of variables declared in $\Psi$, and is defined as follows.
  \begin{align*}
     \token{Dom}_{V}( \varepsilon )                 & =  \emptyset                 \\
     \token{Dom}_{V}( \Psi  \refenvsym{,}   \binder{ \gamma_{{\mathrm{1}}} }( \mathbin{:\succeq} \; \gamma_{{\mathrm{2}}}  /  \mathbin{:\supseteq} \; \gamma_{{\mathrm{3}}} )  )  & =  \token{Dom}_{V}( \Psi )              \\
     \token{Dom}_{V}( \Psi  \refenvsym{,}   \binder{ \refenvmv{x} }: \refenvnt{A} \mathrel{@}\binder{ \gamma_{{\mathrm{1}}} } \mathbin{:\succeq} \gamma_{{\mathrm{2}}}  )       & =  \token{Dom}_{V}( \Psi )  \, \cup \, \refenvsym{\{}  \refenvmv{x}  \refenvsym{\}} \\
     \token{Dom}_{V}( \Psi  \refenvsym{,}   [    \binder{  \gamma _{ 0 }  }  \mathbin{:\succeq}    \delta _{ 0 }  ,\dotsc,\binder{  \gamma _{ \refenvnt{k} }  }  \mathbin{:\succeq}   \delta  _{ \refenvnt{k} }   ]  )  & =  \token{Dom}_{V}( \Psi ) 
  \end{align*}
\end{definition}

\begin{definition}[Location Domain of Store Typing and Store]
  $ \token{Dom}_{L}( \Theta ) $ and $ \token{Dom}_{L}( S ) $ return the set of locations declared in $\Theta$ and $S$, respectively.
  \begin{align*}
     \token{Dom}_{L}( \varepsilon )           & =  \emptyset                   \\
     \token{Dom}_{L}( \Theta  \refenvsym{,}   \refenvmv{l} : \refenvnt{A}  )      & =  \token{Dom}_{L}( \Theta )  \, \cup \, \refenvsym{\{}  \refenvmv{l}  \refenvsym{\}}    \\
    & \\
     \token{Dom}_{L}( \varepsilon )        & =  \emptyset                   \\
     \token{Dom}_{L}( S  \refenvsym{,}  \refenvmv{l}  \coloneqq  \refenvnt{v} )  & =  \token{Dom}_{L}( S )  \, \cup \, \refenvsym{\{}  \refenvmv{l}  \refenvsym{\}}
  \end{align*}
\end{definition}

\subsubsection{Judgments and Derivation Rules}

\vspace{1em}
\fbox{$ \vdash  \Psi \ \token{wf} $}
\begin{mathparpagebreakable}
  \myinferrule[R-WF-NHT-Emp]
  {}
  { \vdash  \varepsilon \ \token{wf} }
  \label{rule:runtime-wf-nht-empty}
  \and
  \myinferrule[R-WF-NHT-CLS]
  { \vdash  \Psi \ \token{wf}  \\
  \gamma_{{\mathrm{1}}} \, \not\in \,  \token{Dom}_{C}( \Psi )  \\
  \gamma_{{\mathrm{2}}} \, \in \,  \token{Dom}_{C}( \Psi )  \\
  \gamma_{{\mathrm{3}}} \, \in \,  \token{Dom}_{C}( \Psi ) }
  { \vdash  \Psi  \refenvsym{,}   \binder{ \gamma_{{\mathrm{1}}} }( \mathbin{:\succeq} \; \gamma_{{\mathrm{2}}}  /  \mathbin{:\supseteq} \; \gamma_{{\mathrm{3}}} )  \ \token{wf} }
  \label{rule:runtime-wf-nht-cls}
  \and
  \myinferrule[R-WF-NHT-Name]
  { \vdash  \Psi \ \token{wf}  \\
  \refenvmv{x} \, \not\in \,  \token{Dom}_{V}( \Psi )  \\
  \gamma_{{\mathrm{1}}} \, \in \,  \token{Dom}_{C}( \Psi )  \\
  \gamma_{{\mathrm{2}}} \, \not\in \,  \token{Dom}_{C}( \Psi )  \\
   \Psi  \vdash^{ \gamma_{{\mathrm{1}}} }  \refenvnt{A} \ \token{wf} }
  { \vdash  \Psi  \refenvsym{,}   \binder{ \refenvmv{x} }: \refenvnt{A} \mathrel{@}\binder{ \gamma_{{\mathrm{2}}} } \mathbin{:\succeq} \gamma_{{\mathrm{1}}}  \ \token{wf} }
  \label{rule:runtime-wf-nht-name}
  \and
  \myinferrule[R-WF-NHT-Polycls]
  { \vdash  \Psi \ \token{wf}  \\
    \gamma _{ 0 }  ,\dotsc,  \gamma _{ \refenvnt{k} }   \text{\ are pairwise distinct } \\
  \Psi  \vdash   \delta _{ \refenvnt{i}  \refenvsym{+}  1 }   \subseteq   \delta _{ \refenvnt{i} }  \text{\ for\ } 0\le\refenvnt{i}<\refenvnt{k} \\
   \delta _{ \refenvnt{i} }  \, \in \,  \token{Dom}_{C}( \Psi )  \text{\ for\ } 0\le\refenvnt{i}\le\refenvnt{k} \\
   \gamma _{ \refenvnt{i} }  \, \not\in \,  \token{Dom}_{C}( \Psi )  \text{\ for\ } 0\le\refenvnt{i}\le\refenvnt{k} \\
   }
  { \vdash  \Psi  \refenvsym{,}   [    \binder{  \gamma _{ 0 }  }  \mathbin{:\succeq}    \delta _{ 0 }  ,\dotsc,\binder{  \gamma _{ \refenvnt{k} }  }  \mathbin{:\succeq}   \delta  _{ \refenvnt{k} }   ]  \ \token{wf} }
  \label{rule:runtime-wf-nht-polycls}
\end{mathparpagebreakable}

\noindent\fbox{$\Psi  \vdash   \overrightarrow{ \gamma }^{+}  \, \token{wf}$}
\begin{mathparpagebreakable}
  \myinferrule[R-WF-CSeq-Init]
  {\gamma \, \in \,  \token{Dom}_{C}( \Psi )  \\
    \vdash  \Psi \ \token{wf} }
  {\Psi  \vdash  \gamma \, \token{wf}}
  \label{rule:runtime-wf-clsseq-init}
  \and
  \myinferrule[R-WF-CSeq-Succ]
  {\Psi  \vdash   \overrightarrow{ \gamma_{{\mathrm{1}}} }^{+}  \, \token{wf} \\
  \gamma_{{\mathrm{2}}} \, \in \,  \token{Dom}_{C}( \Psi ) }
  {\Psi  \vdash   \overrightarrow{ \gamma_{{\mathrm{1}}} }^{+}   \refenvsym{,}  \gamma_{{\mathrm{2}}} \, \token{wf}}
  \label{rule:runtime-wf-clsseq-succ}
\end{mathparpagebreakable}

\noindent\fbox{$ \Psi \mid^{  \overrightarrow{ \gamma_{{\mathrm{1}}} }^{+}  } \Gamma \vdash^{  \overrightarrow{ \gamma_{{\mathrm{2}}} }^{+}  }\token{wf} $}
\begin{mathparpagebreakable}
  \myinferrule[R-WF-Ctx-Var]
  { \Psi \mid^{  \overrightarrow{ \gamma_{{\mathrm{1}}} }^{+}  } \Gamma \vdash^{  \overrightarrow{ \gamma_{{\mathrm{2}}} }   \refenvsym{,}  \gamma_{{\mathrm{3}}} }\token{wf}  \\
   \Psi \mid^{  \overrightarrow{ \gamma_{{\mathrm{1}}} }^{+}  }  \Gamma \vdash ^{  \overrightarrow{ \gamma_{{\mathrm{2}}} }   \refenvsym{,}  \gamma_{{\mathrm{3}}} } \refenvnt{A} \ \token{wf}  \\
  \gamma_{{\mathrm{4}}} \, \not\in \,  \token{Dom}_{C}( \Psi )  \, \cup \,  \token{Dom}_{C}( \Gamma ) }
  { \Psi \mid^{  \overrightarrow{ \gamma_{{\mathrm{1}}} }^{+}  } \Gamma  \refenvsym{,}   \binder{ \refenvmv{x} }\mathord{:^{\binder{ \gamma_{{\mathrm{4}}} } } } \refenvnt{A}  \vdash^{  \overrightarrow{ \gamma_{{\mathrm{2}}} }   \refenvsym{,}  \gamma_{{\mathrm{4}}} }\token{wf} }
  \label{rule:runtime-wf-ctx-var}
  \and
  \myinferrule[R-WF-Ctx-Nil]
  {\Psi  \vdash   \overrightarrow{ \gamma }^{+}  \, \token{wf}}
  { \Psi \mid^{  \overrightarrow{ \gamma }^{+}  } \varepsilon \vdash^{  \overrightarrow{ \gamma }^{+}  }\token{wf} }
  \label{rule:runtime-wf-ctx-nil}
  \and
  \myinferrule[R-WF-Ctx-$ \blacktriangleright $]
  { \Psi \mid^{  \overrightarrow{ \gamma_{{\mathrm{1}}} }^{+}  } \Gamma \vdash^{  \overrightarrow{ \gamma_{{\mathrm{2}}} }   \refenvsym{,}  \gamma_{{\mathrm{3}}} }\token{wf}  \\
   \Psi \mid^{  \overrightarrow{ \gamma_{{\mathrm{1}}} }^{+}  } \Gamma \vdash \gamma_{{\mathrm{4}}} \subseteq \gamma_{{\mathrm{3}}} }
  { \Psi \mid^{  \overrightarrow{ \gamma_{{\mathrm{1}}} }^{+}  } \Gamma  \refenvsym{,}   \blacktriangleright ^{ \gamma_{{\mathrm{4}}} }  \vdash^{  \overrightarrow{ \gamma_{{\mathrm{2}}} }   \refenvsym{,}  \gamma_{{\mathrm{3}}}  \refenvsym{,}  \gamma_{{\mathrm{4}}} }\token{wf} }
  \label{rule:runtime-wf-ctx-open}
  \and
  \myinferrule[R-WF-Ctx-$ \blacktriangleleft $]
  { \Psi \mid^{  \overrightarrow{ \gamma_{{\mathrm{1}}} }^{+}  } \Gamma \vdash^{  \overrightarrow{ \gamma_{{\mathrm{2}}} }^{+}   \refenvsym{,}    \delta _{ 0 }  ,\dotsc,  \delta _{ \refenvnt{k} }   }\token{wf}  \\
    \gamma_{{\mathrm{3}}} \, \not\in \,  \token{Dom}_{C}( \Psi )  \, \cup \,  \token{Dom}_{C}( \Gamma ) }
  { \Psi \mid^{  \overrightarrow{ \gamma_{{\mathrm{1}}} }^{+}  } \Gamma  \refenvsym{,}   \blacktriangleleft _{ \refenvnt{k} }^{\binder{ \gamma_{{\mathrm{3}}} } }  \vdash^{  \overrightarrow{ \gamma_{{\mathrm{2}}} }   \refenvsym{,}  \gamma_{{\mathrm{3}}} }\token{wf} }
  \label{rule:runtime-wf-ctx-shut}
  \and
  \myinferrule[R-WF-Ctx-Polycls]
  { \Psi \mid^{  \overrightarrow{ \delta_{{\mathrm{1}}} }^{+}  } \Gamma \vdash^{  \overrightarrow{ \delta_{{\mathrm{2}}} }   \refenvsym{,}   \gamma' _{ 0 }  }\token{wf} \\
    \gamma _{ 0 }  ,\dotsc,  \gamma _{ \refenvnt{k} }   \text{\ are pairwise distinct } \\
   \gamma _{ \refenvnt{i} }  \, \not\in \,  \token{Dom}_{C}( \Psi )  \text{\ for\ } 0 \le \refenvnt{i} \le \refenvnt{k}\\
   \gamma _{ \refenvnt{i} }  \, \not\in \,  \token{Dom}_{C}( \Gamma )  \text{\ for\ } 0 \le \refenvnt{i} \le \refenvnt{k}\\
   \gamma _{ 0 }  \, \not\in \,  \token{Dom}_{C}( \refenvsym{(}   \binder{  \gamma _{ 1 }  }  \mathbin{:\succeq}    \gamma' _{ 1 }  ,\dotsc,\binder{  \gamma _{ \refenvnt{k} }  }  \mathbin{:\succeq}    \gamma' _{ \refenvnt{k} }    \refenvsym{)} ) \\
   \Psi \mid^{  \overrightarrow{ \delta_{{\mathrm{1}}} }^{+}  } \Gamma \vdash  \gamma' _{ \refenvnt{i}  \refenvsym{+}  1 }  \subseteq  \gamma' _{ \refenvnt{i} }   \text{\ for \ } 0 \le \refenvnt{i} < \refenvnt{k}
  }
  { \Psi \mid^{  \overrightarrow{ \delta_{{\mathrm{1}}} }^{+}  } \Gamma  \refenvsym{,}   [    \binder{  \gamma _{ 1 }  }  \mathbin{:\succeq}    \gamma' _{ 1 }  ,\dotsc,\binder{  \gamma _{ \refenvnt{k} }  }  \mathbin{:\succeq}   \gamma'  _{ \refenvnt{k} }   ]^{\binder{  \gamma _{ 0 }  } }  \vdash^{  \overrightarrow{ \delta_{{\mathrm{2}}} }   \refenvsym{,}   \gamma _{ 0 }  }\token{wf} }
  \label{rule:runtime-wf-ctx-polycls}
\end{mathparpagebreakable}

\noindent\fbox{$ \Psi \mid^{  \overrightarrow{ \gamma_{{\mathrm{1}}} }^{+}  }  \Gamma \vdash ^{  \overrightarrow{ \gamma_{{\mathrm{2}}} }^{+}  } \refenvnt{A} \ \token{wf} $}
\begin{itemize}
  \item $ \Psi  \vdash^{  \overrightarrow{ \gamma }^{+}  }  \refenvnt{A} \ \token{wf} $ is a shorthand for $ \Psi \mid^{  \overrightarrow{ \gamma }^{+}  }  \varepsilon \vdash ^{  \overrightarrow{ \gamma }^{+}  } \refenvnt{A} \ \token{wf} $.
\end{itemize}
\begin{mathparpagebreakable}
  \myinferrule[R-WF-T-Base]
  { \vdash  \Psi \ \token{wf}  \\
   \Psi \mid^{  \overrightarrow{ \gamma_{{\mathrm{1}}} }^{+}  } \Gamma \vdash^{  \overrightarrow{ \gamma_{{\mathrm{2}}} }^{+}  }\token{wf} }
  { \Psi \mid^{  \overrightarrow{ \gamma_{{\mathrm{1}}} }^{+}  }  \Gamma \vdash ^{  \overrightarrow{ \gamma_{{\mathrm{2}}} }^{+}  } \iota \ \token{wf} }
  \label{rule:runtime-wf-t-base}
  \and
  \myinferrule[R-WF-T-Func]
  { \Psi \mid^{  \overrightarrow{ \gamma_{{\mathrm{1}}} }^{+}  }  \Gamma \vdash ^{  \overrightarrow{ \gamma_{{\mathrm{2}}} }^{+}  } \refenvnt{A_{{\mathrm{1}}}} \ \token{wf}  \\
   \Psi \mid^{  \overrightarrow{ \gamma_{{\mathrm{1}}} }^{+}  }  \Gamma \vdash ^{  \overrightarrow{ \gamma_{{\mathrm{2}}} }^{+}  } \refenvnt{A_{{\mathrm{2}}}} \ \token{wf} }
  { \Psi \mid^{  \overrightarrow{ \gamma_{{\mathrm{1}}} }^{+}  }  \Gamma \vdash ^{  \overrightarrow{ \gamma_{{\mathrm{2}}} }^{+}  } \refenvnt{A_{{\mathrm{1}}}}  \rightarrow  \refenvnt{A_{{\mathrm{2}}}} \ \token{wf} }
  \label{rule:runtime-wf-t-func}
  \and
  \myinferrule[R-WF-T-$\langle\rangle$]
  { \Psi \mid^{  \overrightarrow{ \gamma_{{\mathrm{1}}} }^{+}  }  \Gamma  \refenvsym{,}   \blacktriangleright ^{ \gamma_{{\mathrm{2}}} }  \vdash ^{  \overrightarrow{ \gamma_{{\mathrm{3}}} }^{+}   \refenvsym{,}  \gamma_{{\mathrm{2}}} } \refenvnt{A} \ \token{wf} }
  { \Psi \mid^{  \overrightarrow{ \gamma_{{\mathrm{1}}} }^{+}  }  \Gamma \vdash ^{  \overrightarrow{ \gamma_{{\mathrm{3}}} }^{+}  }  \langle \refenvnt{A} \rangle^{ \gamma_{{\mathrm{2}}} }  \ \token{wf} }
  \label{rule:runtime-wf-t-code}
  \and
  \myinferrule[R-WF-T-Ref]
  { \Psi \mid^{  \overrightarrow{ \gamma_{{\mathrm{1}}} }^{+}  }  \Gamma \vdash ^{  \overrightarrow{ \gamma_{{\mathrm{2}}} }^{+}  } \refenvnt{A} \ \token{wf} }
  { \Psi \mid^{  \overrightarrow{ \gamma_{{\mathrm{1}}} }^{+}  }  \Gamma \vdash ^{  \overrightarrow{ \gamma_{{\mathrm{2}}} }^{+}  }  \refenvnt{A} \/\ \token{ref}  \ \token{wf} }
  \label{rule:runtime-wf-t-ref}
  \and
  \myinferrule[R-WF-T-Polycls]
    { \Psi \mid^{  \overrightarrow{ \delta_{{\mathrm{1}}} }^{+}  }  \Gamma  \refenvsym{,}   [    \binder{  \gamma _{ 1 }  }  \mathbin{:\succeq}    \gamma' _{ 1 }  ,\dotsc,\binder{  \gamma _{ \refenvnt{k} }  }  \mathbin{:\succeq}   \gamma'  _{ \refenvnt{k} }   ]^{\binder{  \gamma _{ 0 }  } }  \vdash ^{  \overrightarrow{ \delta_{{\mathrm{2}}} }   \refenvsym{,}   \gamma _{ 0 }  } \refenvnt{A} \ \token{wf} \\
       \gamma _{ \refenvnt{i} }  \, \not\in \,  \token{FC}( \refenvnt{A} )  \text{\ for\ } 1 \le \refenvnt{i} \le \refenvnt{k}\\
       \gamma _{ 0 }  \, \not\in \,  \token{FC}( \refenvnt{A} ) \\
       \Psi \mid^{  \overrightarrow{ \delta_{{\mathrm{1}}} }^{+}  } \Gamma \vdash^{  \overrightarrow{ \delta_{{\mathrm{1}}} }   \refenvsym{,}   \gamma' _{ 0 }  }\token{wf} 
    }{
       \Psi \mid^{  \overrightarrow{ \delta_{{\mathrm{1}}} }^{+}  }  \Gamma \vdash ^{  \overrightarrow{ \delta_{{\mathrm{2}}} }   \refenvsym{,}   \gamma' _{ 0 }  }  \forall    \binder{  \gamma _{ 1 }  }  \mathbin{:\succeq}    \gamma' _{ 1 }  ,\dotsc,\binder{  \gamma _{ \refenvnt{k} }  }  \mathbin{:\succeq}   \gamma'  _{ \refenvnt{k} }  . \refenvnt{A}  \ \token{wf} 
    }
    \label{rule:runtime-wf-t-polycls}
\end{mathparpagebreakable}

\noindent\fbox{$ \Psi \mid^{  \overrightarrow{ \gamma_{{\mathrm{1}}} }^{+}  } \Gamma \vdash \gamma_{{\mathrm{2}}} \preceq \gamma_{{\mathrm{3}}} $} \noindent\fbox{$ \Psi \mid^{  \overrightarrow{ \gamma_{{\mathrm{1}}} }^{+}  } \Gamma \vdash \gamma_{{\mathrm{2}}} \subseteq \gamma_{{\mathrm{3}}} $}
\begin{itemize}
  \item These judgments assume that $ \Psi \mid^{  \overrightarrow{ \gamma_{{\mathrm{1}}} }^{+}  } \Gamma \vdash^{  \overrightarrow{ \gamma_{{\mathrm{2}}} }^{+}  }\token{wf} $ for some $ \overrightarrow{ \gamma_{{\mathrm{2}}} }^{+} $.
  \item $\Psi  \vdash  \gamma_{{\mathrm{2}}}  \preceq  \gamma_{{\mathrm{3}}}$ and $\Psi  \vdash  \gamma_{{\mathrm{2}}}  \subseteq  \gamma_{{\mathrm{3}}}$ are shorthands for $ \Psi \mid^{  \exclam  } \varepsilon \vdash \gamma_{{\mathrm{2}}} \preceq \gamma_{{\mathrm{3}}} $ and $ \Psi \mid^{  \exclam  } \varepsilon \vdash \gamma_{{\mathrm{2}}} \subseteq \gamma_{{\mathrm{3}}} $, respectively.
\end{itemize}
\begin{mathparpagebreakable}
  \myinferrule[R-$ \preceq $-NHT-Name]
  { \binder{ \refenvmv{x} }: \refenvnt{A} \mathrel{@}\binder{ \gamma_{{\mathrm{1}}} } \mathbin{:\succeq} \gamma_{{\mathrm{2}}}  \, \in \, \Psi}
  { \Psi \mid^{  \overrightarrow{ \gamma_{{\mathrm{3}}} }^{+}  } \Gamma \vdash \gamma_{{\mathrm{2}}} \preceq \gamma_{{\mathrm{1}}} }
  \label{rule:runtime-ltrans-nht1}
  \and
  \myinferrule[R-$ \preceq $-NHT-$ \blacktriangleleft $]
  { \binder{ \gamma_{{\mathrm{1}}} }( \mathbin{:\succeq} \; \gamma_{{\mathrm{2}}}  /  \mathbin{:\supseteq} \; \gamma_{{\mathrm{3}}} )  \, \in \, \Psi}
  { \Psi \mid^{  \overrightarrow{ \gamma_{{\mathrm{4}}} }^{+}  } \Gamma \vdash \gamma_{{\mathrm{2}}} \preceq \gamma_{{\mathrm{1}}} }
  \label{rule:runtime-ltrans-nht2}
  \and
  \myinferrule[R-$ \preceq $-NHT-Polycls]
  { [    \binder{  \gamma _{ 0 }  }  \mathbin{:\succeq}    \gamma' _{ 0 }  ,\dotsc,\binder{  \gamma _{ \refenvnt{k} }  }  \mathbin{:\succeq}   \gamma'  _{ \refenvnt{k} }   ]  \, \in \, \Psi\\
    0 \le \refenvnt{i} \le \refenvnt{k}
  }
  { \Psi \mid^{  \overrightarrow{ \delta }^{+}  } \Gamma \vdash  \gamma' _{ \refenvnt{i} }  \preceq  \gamma _{ \refenvnt{i} }  }
  \label{rule:runtime-ltrans-nht3}
  \and
  \myinferrule[R-$ \preceq $-Var]
  { \Psi \mid^{  \overrightarrow{ \gamma_{{\mathrm{1}}} }  } \Gamma_{{\mathrm{1}}} \vdash^{  \overrightarrow{ \gamma_{{\mathrm{2}}} }   \refenvsym{,}  \gamma_{{\mathrm{3}}} }\token{wf} }
  { \Psi \mid^{  \overrightarrow{ \gamma_{{\mathrm{1}}} }  } \Gamma_{{\mathrm{1}}}  \refenvsym{,}   \binder{ \refenvmv{x} }\mathord{:^{\binder{ \gamma_{{\mathrm{4}}} } } } \refenvnt{A}   \refenvsym{,}  \Gamma_{{\mathrm{2}}} \vdash \gamma_{{\mathrm{3}}} \preceq \gamma_{{\mathrm{4}}} }
  \label{rule:runtime-ltrans-var}
  \and
  \myinferrule[R-$ \preceq $-$ \blacktriangleleft $-Ctx]
  { \Psi \mid^{  \overrightarrow{ \gamma_{{\mathrm{1}}} }  } \Gamma_{{\mathrm{1}}} \vdash^{  \overrightarrow{ \gamma_{{\mathrm{2}}} }   \refenvsym{,}    \delta _{ 0 }  ,\dotsc,  \delta _{ \refenvnt{k} }   }\token{wf} }
  { \Psi \mid^{  \overrightarrow{ \gamma_{{\mathrm{1}}} }  } \Gamma_{{\mathrm{1}}}  \refenvsym{,}   \blacktriangleleft _{ \refenvnt{k} }^{\binder{ \gamma_{{\mathrm{3}}} } }   \refenvsym{,}  \Gamma_{{\mathrm{2}}} \vdash  \delta _{ 0 }  \preceq \gamma_{{\mathrm{3}}} }
  \label{rule:runtime-ltrans-shut}
  \and
  \myinferrule[R-$ \preceq $-Polycls-Ctx]
  { \Psi \mid^{  \overrightarrow{ \delta }^{+}  } \Gamma_{{\mathrm{1}}} \vdash^{  \overrightarrow{ \delta_{{\mathrm{1}}} }   \refenvsym{,}   \gamma' _{ 0 }  }\token{wf}  \\
  0 \le \refenvnt{i} \le \refenvnt{k}}
  { \Psi \mid^{  \overrightarrow{ \delta }^{+}  } \Gamma_{{\mathrm{1}}}  \refenvsym{,}   [    \binder{  \gamma _{ 1 }  }  \mathbin{:\succeq}    \gamma' _{ 1 }  ,\dotsc,\binder{  \gamma _{ \refenvnt{k} }  }  \mathbin{:\succeq}   \gamma'  _{ \refenvnt{k} }   ]^{\binder{  \gamma _{ 0 }  } }   \refenvsym{,}  \Gamma_{{\mathrm{2}}} \vdash  \gamma' _{ \refenvnt{i} }  \preceq  \gamma _{ \refenvnt{i} }  }
  \label{rule:runtime-ltrans-polycls-ctx}
  \and
  \myinferrule[R-$ \preceq $-Refl]
  {\gamma_{{\mathrm{1}}} \, \in \,  \token{Dom}_{C}( \Psi )  \, \cup \,  \token{Dom}_{C}( \Gamma ) }
  { \Psi \mid^{  \overrightarrow{ \gamma_{{\mathrm{2}}} }  } \Gamma \vdash \gamma_{{\mathrm{1}}} \preceq \gamma_{{\mathrm{1}}} }
  \label{rule:runtime-ltrans-refl}
  \and
  \myinferrule[R-$ \preceq $-Trans]
  { \Psi \mid^{  \overrightarrow{ \gamma_{{\mathrm{1}}} }^{+}  } \Gamma \vdash \gamma_{{\mathrm{2}}} \preceq \gamma_{{\mathrm{3}}}  \\
   \Psi \mid^{  \overrightarrow{ \gamma_{{\mathrm{1}}} }^{+}  } \Gamma \vdash \gamma_{{\mathrm{3}}} \preceq \gamma_{{\mathrm{4}}} }
  { \Psi \mid^{  \overrightarrow{ \gamma_{{\mathrm{1}}} }^{+}  } \Gamma \vdash \gamma_{{\mathrm{2}}} \preceq \gamma_{{\mathrm{4}}} }
  \label{rule:runtime-ltrans-trans}
  \and
  \myinferrule[R-$ \subseteq $-Lift]
  { \Psi \mid^{  \overrightarrow{ \gamma_{{\mathrm{1}}} }^{+}  } \Gamma \vdash \gamma_{{\mathrm{1}}} \preceq \gamma_{{\mathrm{2}}} }
  { \Psi \mid^{  \overrightarrow{ \gamma_{{\mathrm{1}}} }^{+}  } \Gamma \vdash \gamma_{{\mathrm{1}}} \subseteq \gamma_{{\mathrm{2}}} }
  \label{rule:runtime-gtrans-lift}
  \and
  \myinferrule[R-$ \subseteq $-Trans]
  { \Psi \mid^{  \overrightarrow{ \gamma_{{\mathrm{1}}} }^{+}  } \Gamma \vdash \gamma_{{\mathrm{2}}} \subseteq \gamma_{{\mathrm{3}}}  \\
   \Psi \mid^{  \overrightarrow{ \gamma_{{\mathrm{1}}} }^{+}  } \Gamma \vdash \gamma_{{\mathrm{3}}} \subseteq \gamma_{{\mathrm{4}}} }
  { \Psi \mid^{  \overrightarrow{ \gamma_{{\mathrm{1}}} }^{+}  } \Gamma \vdash \gamma_{{\mathrm{2}}} \subseteq \gamma_{{\mathrm{4}}} }
  \label{rule:runtime-gtrans-trans}
  \and
  \myinferrule[R-$ \subseteq $-NHT-$ \blacktriangleleft $]
  { \binder{ \gamma_{{\mathrm{1}}} }( \mathbin{:\succeq} \; \gamma_{{\mathrm{2}}}  /  \mathbin{:\supseteq} \; \gamma_{{\mathrm{3}}} )  \, \in \, \Psi}
  { \Psi \mid^{  \overrightarrow{ \gamma_{{\mathrm{4}}} }^{+}  } \Gamma \vdash \gamma_{{\mathrm{3}}} \subseteq \gamma_{{\mathrm{1}}} }
  \label{rule:runtime-gtrans-shut-nht}
  \and
  \myinferrule[R-$ \subseteq $-NHT-Polycls]
  { [    \binder{  \gamma _{ 0 }  }  \mathbin{:\succeq}    \gamma' _{ 0 }  ,\dotsc,\binder{  \gamma _{ \refenvnt{k} }  }  \mathbin{:\succeq}   \gamma'  _{ \refenvnt{k} }   ]  \, \in \, \Psi\\
    0 \le \refenvnt{i} < \refenvnt{k}
  }
  { \Psi \mid^{  \overrightarrow{ \delta }^{+}  } \Gamma \vdash  \gamma _{ \refenvnt{i}  \refenvsym{+}  1 }  \subseteq  \gamma _{ \refenvnt{i} }  }
  \label{rule:runtime-gtrans-nht-polycls}
  \and
  \myinferrule[R-$ \subseteq $-$ \blacktriangleleft $-Ctx]
  { \Psi \mid^{  \overrightarrow{ \gamma_{{\mathrm{1}}} }  } \Gamma_{{\mathrm{1}}} \vdash^{  \overrightarrow{ \gamma_{{\mathrm{2}}} }   \refenvsym{,}    \delta _{ 0 }  ,\dotsc,  \delta _{ \refenvnt{k} }   }\token{wf} }
  { \Psi \mid^{  \overrightarrow{ \gamma_{{\mathrm{1}}} }  } \Gamma_{{\mathrm{1}}}  \refenvsym{,}   \blacktriangleleft _{ \refenvnt{k} }^{\binder{ \gamma_{{\mathrm{3}}} } }   \refenvsym{,}  \Gamma_{{\mathrm{2}}} \vdash  \delta _{ \refenvnt{k} }  \subseteq \gamma_{{\mathrm{3}}} }
  \label{rule:runtime-gtrans-shut-ctx}
  \and
  \myinferrule[R-$ \subseteq $-Polycls-Ctx]
  {0 \le \refenvnt{i} < \refenvnt{k}}
  { \Psi \mid^{  \overrightarrow{ \delta }^{+}  } \Gamma_{{\mathrm{1}}}  \refenvsym{,}   [    \binder{  \gamma _{ 1 }  }  \mathbin{:\succeq}    \gamma' _{ 1 }  ,\dotsc,\binder{  \gamma _{ \refenvnt{k} }  }  \mathbin{:\succeq}   \gamma'  _{ \refenvnt{k} }   ]^{\binder{  \gamma _{ 0 }  } }   \refenvsym{,}  \Gamma_{{\mathrm{2}}} \vdash  \gamma _{ \refenvnt{i}  \refenvsym{+}  1 }  \subseteq  \gamma _{ \refenvnt{i} }  }
  \label{rule:runtime-gtrans-polycls-ctx}
\end{mathparpagebreakable}

\noindent\fbox{$ \Psi \mid^{  \overrightarrow{ \gamma_{{\mathrm{1}}} }^{+}  }  \Gamma \vdash^{  \overrightarrow{ \gamma_{{\mathrm{2}}} }^{+}  }_{ R }  \refenvnt{e} : \refenvnt{A} $}

\begin{mathparpagebreakable}
  \myinferrule[R-T-Int]
  { \Psi \mid^{  \overrightarrow{ \gamma_{{\mathrm{1}}} }^{+}  } \Gamma \vdash^{  \overrightarrow{ \gamma_{{\mathrm{2}}} }^{+}  }\token{wf} }
  { \Psi \mid^{  \overrightarrow{ \gamma_{{\mathrm{1}}} }^{+}  }  \Gamma \vdash^{  \overrightarrow{ \gamma_{{\mathrm{2}}} }^{+}  }_{ R }  \refenvnt{n} :  \texttt{int}  }
  \label{rule:runtime-type-int}
  \and
  \myinferrule[R-T-Var]
  {\token{lookup} \, \refenvsym{(}  \Gamma  \refenvsym{,}  \refenvmv{x}  \refenvsym{)} = \token{Done} \, \refenvsym{(}  \refenvnt{A}  \refenvsym{,}  \gamma_{{\mathrm{1}}}  \refenvsym{)} \\
   \Psi \mid^{  \overrightarrow{ \gamma_{{\mathrm{2}}} }^{+}  } \Gamma \vdash^{  \overrightarrow{ \gamma_{{\mathrm{3}}} }   \refenvsym{,}  \gamma_{{\mathrm{4}}} }\token{wf}  \\
   \Psi \mid^{  \overrightarrow{ \gamma_{{\mathrm{2}}} }^{+}  } \Gamma \vdash \gamma_{{\mathrm{1}}} \preceq \gamma_{{\mathrm{4}}} }
  { \Psi \mid^{  \overrightarrow{ \gamma_{{\mathrm{2}}} }^{+}  }  \Gamma \vdash^{  \overrightarrow{ \gamma_{{\mathrm{3}}} }   \refenvsym{,}  \gamma_{{\mathrm{4}}} }_{ R }  \refenvmv{x} : \refenvnt{A} }
  \label{rule:runtime-type-var}
  \and
  \myinferrule[R-T-Name]
  {\token{lookup} \, \refenvsym{(}  \Gamma  \refenvsym{,}  \refenvmv{x}  \refenvsym{)} =  \token{Fail}  \\
   \binder{ \refenvmv{y} }: \refenvnt{A} \mathrel{@}\binder{ \gamma_{{\mathrm{1}}} } \mathbin{:\succeq} \gamma_{{\mathrm{2}}}  \, \in \, \Psi \\
   \Psi \mid^{  \overrightarrow{ \gamma_{{\mathrm{3}}} }^{+}  } \Gamma \vdash^{  \overrightarrow{ \gamma_{{\mathrm{4}}} }   \refenvsym{,}  \gamma_{{\mathrm{5}}} }\token{wf}  \\
   \Psi \mid^{  \overrightarrow{ \gamma_{{\mathrm{3}}} }^{+}  } \Gamma \vdash \gamma_{{\mathrm{1}}} \preceq \gamma_{{\mathrm{5}}}  \\
  \token{rename} \, \refenvsym{(}  R  \refenvsym{,}  \refenvmv{x}  \refenvsym{)}  \refenvsym{=}  \refenvmv{y}}
  { \Psi \mid^{  \overrightarrow{ \gamma_{{\mathrm{3}}} }^{+}  }  \Gamma \vdash^{  \overrightarrow{ \gamma_{{\mathrm{4}}} }   \refenvsym{,}  \gamma_{{\mathrm{5}}} }_{ R }  \refenvmv{x} : \refenvnt{A} }
  \label{rule:runtime-type-reserved-var}
  \and
  \myinferrule[R-T-Func]
  { \Psi \mid^{  \overrightarrow{ \gamma_{{\mathrm{1}}} }^{+}  }  \Gamma  \refenvsym{,}   \binder{ \refenvmv{x} }\mathord{:^{\binder{ \gamma_{{\mathrm{2}}} } } } \refenvnt{A_{{\mathrm{1}}}}  \vdash^{  \overrightarrow{ \gamma_{{\mathrm{3}}} }   \refenvsym{,}  \gamma_{{\mathrm{2}}} }_{ R }  \refenvnt{e} : \refenvnt{A_{{\mathrm{2}}}}  \\
  \gamma_{{\mathrm{2}}} \, \not\in \,  \token{FC}( \refenvnt{A_{{\mathrm{2}}}} )  \\
   \Psi \mid^{  \overrightarrow{ \gamma_{{\mathrm{1}}} }^{+}  } \Gamma \vdash^{  \overrightarrow{ \gamma_{{\mathrm{3}}} }   \refenvsym{,}  \gamma_{{\mathrm{4}}} }\token{wf} }
  { \Psi \mid^{  \overrightarrow{ \gamma_{{\mathrm{1}}} }^{+}  }  \Gamma \vdash^{  \overrightarrow{ \gamma_{{\mathrm{3}}} }   \refenvsym{,}  \gamma_{{\mathrm{4}}} }_{ R }   \lambda \binder{ \refenvmv{x} }.\  \refenvnt{e}  : \refenvnt{A_{{\mathrm{1}}}}  \rightarrow  \refenvnt{A_{{\mathrm{2}}}} }
  \label{rule:runtime-type-func}
  \and
  \myinferrule[R-T-Rec]
  { \Psi \mid^{  \overrightarrow{ \gamma_{{\mathrm{1}}} }^{+}  }  \Gamma  \refenvsym{,}   \binder{ \refenvmv{f} }\mathord{:^{\binder{ \gamma_{{\mathrm{2}}} } } } \refenvnt{A_{{\mathrm{1}}}}  \rightarrow  \refenvnt{A_{{\mathrm{2}}}}   \refenvsym{,}   \binder{ \refenvmv{x} }\mathord{:^{\binder{ \gamma_{{\mathrm{3}}} } } } \refenvnt{A_{{\mathrm{1}}}}  \vdash^{  \overrightarrow{ \gamma_{{\mathrm{4}}} }   \refenvsym{,}  \gamma_{{\mathrm{3}}} }_{ R }  \refenvnt{e} : \refenvnt{A_{{\mathrm{2}}}}  \\
   \Psi \mid^{  \overrightarrow{ \gamma_{{\mathrm{1}}} }^{+}  } \Gamma \vdash^{  \overrightarrow{ \gamma_{{\mathrm{4}}} }   \refenvsym{,}  \gamma_{{\mathrm{5}}} }\token{wf} }
  { \Psi \mid^{  \overrightarrow{ \gamma_{{\mathrm{1}}} }^{+}  }  \Gamma \vdash^{  \overrightarrow{ \gamma_{{\mathrm{4}}} }   \refenvsym{,}  \gamma_{{\mathrm{5}}} }_{ R }   \token{rec}\ \binder{ \refenvmv{f} }(\binder{ \refenvmv{x} }).\  \refenvnt{e}  : \refenvnt{A_{{\mathrm{1}}}}  \rightarrow  \refenvnt{A_{{\mathrm{2}}}} }
  \label{rule:runtime-type-rec}
  \and
  \myinferrule[R-T-App]
  { \Psi \mid^{  \overrightarrow{ \gamma_{{\mathrm{1}}} }^{+}  }  \Gamma \vdash^{  \overrightarrow{ \gamma_{{\mathrm{2}}} }^{+}  }_{ R }  \refenvnt{e_{{\mathrm{1}}}} : \refenvnt{A_{{\mathrm{1}}}}  \rightarrow  \refenvnt{A_{{\mathrm{2}}}}  \\
   \Psi \mid^{  \overrightarrow{ \gamma_{{\mathrm{1}}} }^{+}  }  \Gamma \vdash^{  \overrightarrow{ \gamma_{{\mathrm{2}}} }^{+}  }_{ R }  \refenvnt{e_{{\mathrm{2}}}} : \refenvnt{A_{{\mathrm{1}}}} }
  { \Psi \mid^{  \overrightarrow{ \gamma_{{\mathrm{1}}} }^{+}  }  \Gamma \vdash^{  \overrightarrow{ \gamma_{{\mathrm{2}}} }^{+}  }_{ R }   \refenvnt{e_{{\mathrm{1}}}} \refenvnt{e_{{\mathrm{2}}}}  : \refenvnt{A_{{\mathrm{2}}}} }
  \label{rule:runtime-type-app}
  \and
  \myinferrule[R-T-Quote]
  { \Psi \mid^{  \overrightarrow{ \gamma_{{\mathrm{1}}} }^{+}  }  \Gamma  \refenvsym{,}   \blacktriangleright ^{ \gamma_{{\mathrm{2}}} }  \vdash^{  \overrightarrow{ \gamma_{{\mathrm{3}}} }^{+}   \refenvsym{,}  \gamma_{{\mathrm{2}}} }_{ R }  \refenvnt{e_{{\mathrm{1}}}} : \refenvnt{A} }
  { \Psi \mid^{  \overrightarrow{ \gamma_{{\mathrm{1}}} }^{+}  }  \Gamma \vdash^{  \overrightarrow{ \gamma_{{\mathrm{3}}} }^{+}  }_{ R }   \langle  \refenvnt{e_{{\mathrm{1}}}}  \rangle  :  \langle \refenvnt{A} \rangle^{ \gamma_{{\mathrm{2}}} }  }
  \label{rule:runtime-type-quote}
  \and
  \myinferrule[R-T-Splice]
  { \Psi \mid^{  \overrightarrow{ \gamma_{{\mathrm{1}}} }^{+}  } \Gamma \vdash^{  \overrightarrow{ \gamma_{{\mathrm{4}}} }   \refenvsym{,}    \delta _{ 0 }  ,\dotsc,  \delta _{ \refenvnt{k} }   }\token{wf}  \\
  \gamma_{{\mathrm{2}}} \, \not\in \,  \token{FC}( \refenvnt{A} )  \\
   \Psi \mid^{  \overrightarrow{ \gamma_{{\mathrm{1}}} }^{+}  }  \Gamma  \refenvsym{,}   \blacktriangleleft _{ \refenvnt{k} }^{\binder{ \gamma_{{\mathrm{2}}} } }  \vdash^{  \overrightarrow{ \gamma_{{\mathrm{4}}} }   \refenvsym{,}  \gamma_{{\mathrm{2}}} }_{ R }  \refenvnt{e} :  \langle \refenvnt{A} \rangle^{ \gamma_{{\mathrm{3}}} }   \\
   \Psi \mid^{  \overrightarrow{ \gamma_{{\mathrm{1}}} }^{+}  } \Gamma \vdash \gamma_{{\mathrm{3}}} \preceq  \delta _{ \refenvnt{k} }   \\
  \gamma_{{\mathrm{2}}} \neq \gamma_{{\mathrm{3}}}}
  { \Psi \mid^{  \overrightarrow{ \gamma_{{\mathrm{1}}} }^{+}  }  \Gamma \vdash^{  \overrightarrow{ \gamma_{{\mathrm{4}}} }   \refenvsym{,}    \delta _{ 0 }  ,\dotsc,  \delta _{ \refenvnt{k} }   }_{ R }   { \mathdollar }_{ \refenvnt{k} }\lbrace \refenvnt{e} \rbrace  : \refenvnt{A} }
  \label{rule:runtime-type-splice}
  \and
  \myinferrule[R-T-Ref]
  { \Psi \mid^{  \overrightarrow{ \gamma_{{\mathrm{1}}} }^{+}  }  \Gamma \vdash^{  \overrightarrow{ \gamma_{{\mathrm{2}}} }^{+}  }_{ R }  \refenvnt{e} : \refenvnt{A} }
  { \Psi \mid^{  \overrightarrow{ \gamma_{{\mathrm{1}}} }^{+}  }  \Gamma \vdash^{  \overrightarrow{ \gamma_{{\mathrm{2}}} }^{+}  }_{ R }  \token{ref} \, \refenvsym{(}  \refenvnt{e}  \refenvsym{)} :  \refenvnt{A} \/\ \token{ref}  }
  \label{rule:runtime-type-ref}
  \and
  \myinferrule[R-T-Deref]
  { \Psi \mid^{  \overrightarrow{ \gamma_{{\mathrm{1}}} }^{+}  }  \Gamma \vdash^{  \overrightarrow{ \gamma_{{\mathrm{2}}} }^{+}  }_{ R }  \refenvnt{e} :  \refenvnt{A} \/\ \token{ref}  }
  { \Psi \mid^{  \overrightarrow{ \gamma_{{\mathrm{1}}} }^{+}  }  \Gamma \vdash^{  \overrightarrow{ \gamma_{{\mathrm{2}}} }^{+}  }_{ R }   \token{deref}( \refenvnt{e} )  : \refenvnt{A} }
  \label{rule:runtime-type-get}
  \and
  \myinferrule[R-T-Assign]
  { \Psi \mid^{  \overrightarrow{ \gamma_{{\mathrm{1}}} }^{+}  }  \Gamma \vdash^{  \overrightarrow{ \gamma_{{\mathrm{2}}} }^{+}  }_{ R }  \refenvnt{e_{{\mathrm{1}}}} :  \refenvnt{A} \/\ \token{ref}   \\
   \Psi \mid^{  \overrightarrow{ \gamma_{{\mathrm{1}}} }^{+}  }  \Gamma \vdash^{  \overrightarrow{ \gamma_{{\mathrm{2}}} }^{+}  }_{ R }  \refenvnt{e_{{\mathrm{2}}}} : \refenvnt{A} }
  { \Psi \mid^{  \overrightarrow{ \gamma_{{\mathrm{1}}} }^{+}  }  \Gamma \vdash^{  \overrightarrow{ \gamma_{{\mathrm{2}}} }^{+}  }_{ R }   \refenvnt{e_{{\mathrm{1}}}} \coloneqq \refenvnt{e_{{\mathrm{2}}}}  : \refenvnt{A} }
  \label{rule:runtime-type-set}
  \and
    \myinferrule[R-T-Polycls]
  { \Psi \mid^{  \overrightarrow{ \delta_{{\mathrm{1}}} }^{+}  }  \Gamma  \refenvsym{,}   [    \binder{  \gamma _{ 1 }  }  \mathbin{:\succeq}    \gamma' _{ 1 }  ,\dotsc,\binder{  \gamma _{ \refenvnt{k} }  }  \mathbin{:\succeq}   \gamma'  _{ \refenvnt{k} }   ]^{\binder{  \gamma _{ 0 }  } }  \vdash^{  \overrightarrow{ \delta_{{\mathrm{2}}} }   \refenvsym{,}   \gamma _{ 0 }  }_{ R }  {e_{I} } : \refenvnt{A}  \\
   \gamma _{ \refenvnt{i} }  \, \not\in \,  \token{FC}( \refenvnt{A} )  \text{\ for\ } 1 \le \refenvnt{i} \le \refenvnt{k} \\
   \gamma _{ 0 }  \, \not\in \,  \token{FC}( \refenvnt{A} )  \\
   \Psi \mid^{  \overrightarrow{ \delta_{{\mathrm{1}}} }^{+}  } \Gamma \vdash^{  \overrightarrow{ \delta_{{\mathrm{2}}} }   \refenvsym{,}   \gamma' _{ 0 }  }\token{wf} }
  { \Psi \mid^{  \overrightarrow{ \delta_{{\mathrm{1}}} }^{+}  }  \Gamma \vdash^{  \overrightarrow{ \delta_{{\mathrm{2}}} }   \refenvsym{,}   \gamma' _{ 0 }  }_{ R }  {e_{I} } :  \forall    \binder{  \gamma _{ 1 }  }  \mathbin{:\succeq}    \gamma' _{ 1 }  ,\dotsc,\binder{  \gamma _{ \refenvnt{k} }  }  \mathbin{:\succeq}   \gamma'  _{ \refenvnt{k} }  . \refenvnt{A}  }
  \label{rule:runtime-type-polycls}
  \and
  \myinferrule[R-T-Appcls]
  { \Psi \mid^{  \overrightarrow{ \delta'_{{\mathrm{1}}} }^{+}  }  \Gamma \vdash^{  \overrightarrow{ \delta'_{{\mathrm{2}}} }   \refenvsym{,}   \delta _{ 0 }  }_{ R }  \refenvnt{e} :  \forall    \binder{  \gamma _{ 1 }  }  \mathbin{:\succeq}    \gamma' _{ 1 }  ,\dotsc,\binder{  \gamma _{ \refenvnt{k} }  }  \mathbin{:\succeq}   \gamma'  _{ \refenvnt{k} }  . \refenvnt{A}   \\
   \Psi \mid^{  \overrightarrow{ \delta'_{{\mathrm{1}}} }^{+}  } \Gamma \vdash  \gamma' _{ \refenvnt{i} }  \preceq  \delta _{ \refenvnt{i} }   \text{\ for\ }  1 \le \refenvnt{i} \le \refenvnt{k} \\
   \Psi \mid^{  \overrightarrow{ \delta'_{{\mathrm{1}}} }^{+}  } \Gamma \vdash  \delta _{ \refenvnt{i}  \refenvsym{+}  1 }  \subseteq  \delta _{ \refenvnt{i} }   \text{\ for\ }  0 \le \refenvnt{i} < \refenvnt{k}}
  { \Psi \mid^{  \overrightarrow{ \delta'_{{\mathrm{1}}} }^{+}  }  \Gamma \vdash^{  \overrightarrow{ \delta'_{{\mathrm{2}}} }   \refenvsym{,}   \delta _{ 0 }  }_{ R }  \refenvnt{e} : \refenvnt{A}  \refenvsym{[}    \gamma _{ 1 }  \coloneqq  \delta _{ 1 }  ,\dotsc,  \gamma _{ \refenvnt{k} }  \coloneqq  \delta _{ \refenvnt{k} }    \refenvsym{]} }
  \label{rule:runtime-type-appcls}
\end{mathparpagebreakable}

\noindent\fbox{$ \Psi  \vdash  \Theta \ \token{wf} $}
\begin{mathparpagebreakable}
  \myinferrule[WF-ST-Nil]
  {}
  {\Psi  \vdash  \varepsilon \, \token{wf}}
  \label{rule:wf-store-typ-nil}
  \and
  \myinferrule[WF-ST-Cons]
  { \Psi  \vdash  \Theta \ \token{wf}  \\
  \refenvmv{l} \, \not\in \,  \token{Dom}_{L}( \Theta )  \\
   \Psi  \vdash^{ \gamma }  \refenvnt{A} \ \token{wf} \ \text{for some $\gamma$}}
  { \Psi  \vdash  \refenvsym{(}  \Theta  \refenvsym{,}   \refenvmv{l} : \refenvnt{A}   \refenvsym{)} \ \token{wf} }
  \label{rule:wf-store-typ-cons}
\end{mathparpagebreakable}

\noindent\fbox{$\Psi  \vdash  S  \colon  \Theta$}
\begin{mathparpagebreakable}
  \myinferrule[T-Store]
  {S = \refenvsym{(}    { \refenvmv{l} _{ 1 } }  \coloneqq  { \refenvnt{v} _{ 1 } }  ,\dotsc,  { \refenvmv{l} _{ \refenvnt{k} } }  \coloneqq  { \refenvnt{v} _{ \refenvnt{k} } }    \refenvsym{)} \\
  \Theta = \refenvsym{(}    { \refenvmv{l} _{ 1 } }  :  { \refenvnt{A} _{ 1 } }  ,\dotsc,  { \refenvmv{l} _{ \refenvnt{k} } }  :  { \refenvnt{A} _{ \refenvnt{k} } }    \refenvsym{)} \\
   \Psi  \vdash  \Theta \ \token{wf}  \\
   \Psi \mid \Theta \vdash^{  \gamma _{ \refenvnt{i} }  }  { \refenvnt{v} _{ \refenvnt{i} } }  :  { \refenvnt{A} _{ \refenvnt{i} } }  \ \token{val} \ \text{with some $ \gamma _{ \refenvnt{i} } $ for}\ 1 \le \refenvnt{i} \le \refenvnt{k}}
  {\Psi  \vdash  S  \colon  \Theta}
  \label{rule:type-store}
\end{mathparpagebreakable}

\noindent\fbox{$ \Psi \mid \Theta \vdash^{ \gamma } \refenvnt{v} : \refenvnt{A} \ \token{val} $}

\begin{mathparpagebreakable}
  \myinferrule[VT-Int]
  { \Psi  \vdash  \Theta \ \token{wf}  \\
   \Psi  \vdash  \gamma \, \token{wf}}
  { \Psi \mid \Theta \vdash^{ \gamma } \refenvnt{n} :  \texttt{int}  \ \token{val} }
  \label{rule:value-type-int}
  \and
  \myinferrule[VT-Clos-Func]{
   \Psi \mid^{ \gamma_{{\mathrm{1}}} }  \varepsilon \vdash^{ \gamma_{{\mathrm{1}}} }_{ R }    \lambda \binder{ \refenvmv{x} }.\  \refenvnt{e}  ^{ 0  }  : \refenvnt{A}  \\
   \Psi \mid \Theta \vdash^{ \gamma_{{\mathrm{1}}} } E \ \token{wf}  \\
   \Psi  \vdash^{ \delta }  \refenvnt{A} \ \token{wf} 
  }
  { \Psi \mid \Theta \vdash^{ \delta } \token{clos} \, \refenvsym{(}  E  \refenvsym{,}  R  \refenvsym{,}    \lambda \binder{ \refenvmv{x} }.\  \refenvnt{e}  ^{ 0  }   \refenvsym{)} : \refenvnt{A} \ \token{val} }
  \label{rule:value-type-clos-func}
  \and
  \myinferrule[VT-Clos-Rec]
  { \Psi \mid^{ \gamma_{{\mathrm{1}}} }  \varepsilon \vdash^{ \gamma_{{\mathrm{1}}} }_{ R }    \token{rec}\ \binder{ \refenvmv{f} }(\binder{ \refenvmv{x} }).\  \refenvnt{e}  ^{ 0  }  : \refenvnt{A}  \\
   \Psi \mid \Theta \vdash^{ \gamma_{{\mathrm{1}}} } E \ \token{wf}  \\
   \Psi  \vdash^{ \delta }  \refenvnt{A} \ \token{wf} 
  }
  { \Psi \mid \Theta \vdash^{ \delta } \token{clos} \, \refenvsym{(}  E  \refenvsym{,}  R  \refenvsym{,}    \token{rec}\ \binder{ \refenvmv{f} }(\binder{ \refenvmv{x} }).\  \refenvnt{e}  ^{ 0  }   \refenvsym{)} : \refenvnt{A} \ \token{val} }
  \label{rule:value-type-clos-rec}
  \and
  \myinferrule[VT-Code]
  { \Psi \mid^{ \gamma_{{\mathrm{1}}} }  \varepsilon \vdash^{ \gamma_{{\mathrm{1}}} }_{  \token{id}  }   \langle   \refenvnt{e} ^{ 0  }   \rangle  : \refenvnt{A}  \\
   \Psi  \vdash  \Theta \ \token{wf} \\
  }
  { \Psi \mid \Theta \vdash^{ \gamma_{{\mathrm{1}}} }  \langle   \refenvnt{e} ^{ 0  }   \rangle  : \refenvnt{A} \ \token{val} }
  \label{rule:value-type-code}
  \and
  \myinferrule[VT-Loc]
  { \Psi  \vdash  \Theta \ \token{wf}  \\
  \token{lookupStore}  \refenvsym{(}  \Theta  \refenvsym{,}  \refenvmv{l}  \refenvsym{)} = \token{Done} \, \refenvsym{(}  \refenvnt{A}  \refenvsym{)} \\
   \Psi  \vdash^{ \gamma }  \refenvnt{A} \ \token{wf} }
  { \Psi \mid \Theta \vdash^{ \gamma } \refenvmv{l} :  \refenvnt{A} \/\ \token{ref}  \ \token{val} }
  \label{rule:value-type-loc}
\end{mathparpagebreakable}

\noindent\fbox{$ \Psi \mid \Theta \vdash^{ \gamma } E \ \token{wf} $}
\begin{mathparpagebreakable}
  \myinferrule[WF-VEnv-Empty]
  { \Psi  \vdash  \Theta \ \token{wf} }
  { \Psi \mid \Theta \vdash^{  \exclam  } \varepsilon \ \token{wf} }
  \label{rule:runtime-wf-venv-empty}
  \and
  \myinferrule[WF-VEnv-Shut]
  { \Psi \mid \Theta \vdash^{ \gamma_{{\mathrm{1}}} } E \ \token{wf}  \\
   \binder{ \gamma_{{\mathrm{2}}} }( \mathbin{:\succeq} \; \gamma_{{\mathrm{1}}}  /  \mathbin{:\supseteq} \; \gamma_{{\mathrm{3}}} )  \, \in \, \Psi}
  { \Psi \mid \Theta \vdash^{ \gamma_{{\mathrm{2}}} } E \ \token{wf} }
  \label{rule:runtime-wf-venv-name-cls}
  \and
  \myinferrule[WF-VEnv-Var]
  { \Psi \mid \Theta \vdash^{ \gamma_{{\mathrm{1}}} } E \ \token{wf}  \\
   \Psi \mid \Theta \vdash^{ \gamma_{{\mathrm{1}}} } \refenvnt{v} : \refenvnt{A} \ \token{val}  \\
   \binder{ \refenvmv{x} }: \refenvnt{A} \mathrel{@}\binder{ \gamma_{{\mathrm{2}}} } \mathbin{:\succeq} \gamma_{{\mathrm{1}}}  \, \in \, \Psi}
  { \Psi \mid \Theta \vdash^{ \gamma_{{\mathrm{2}}} } E  \refenvsym{,}  \refenvmv{x}  \coloneqq  \refenvnt{v} \ \token{wf} }
  \label{rule:runtime-wf-venv-var}
  \and
  \myinferrule[WF-VEnv-Polycls]
  { \Psi \mid \Theta \vdash^{  \delta _{ 0 }  } E \ \token{wf}  \\
   [    \binder{  \gamma _{ 0 }  }  \mathbin{:\succeq}    \delta _{ 0 }  ,\dotsc,\binder{  \gamma _{ \refenvnt{k} }  }  \mathbin{:\succeq}   \delta  _{ \refenvnt{k} }   ]  \, \in \, \Psi}
  { \Psi \mid \Theta \vdash^{  \gamma _{ 0 }  } E \ \token{wf} }
  \label{rule:runtime-wf-venv-polycls}
\end{mathparpagebreakable}

Here, $\token{lookupStore}  \refenvsym{(}  \Theta  \refenvsym{,}  \refenvmv{l}  \refenvsym{)}$ returns the type of location $\refenvmv{l}$ in $\Theta$ if it exists, and $ \token{Fail} $ otherwise.
\begin{align*}
  \token{lookupStore}  \refenvsym{(}  \varepsilon  \refenvsym{,}  \refenvmv{l}  \refenvsym{)} & =  \token{Fail}  \\
  \token{lookupStore}  \refenvsym{(}  \Theta  \refenvsym{,}  \refenvmv{l}  \refenvsym{)} & = \token{Done} \, \refenvsym{(}  \refenvnt{A}  \refenvsym{)}\text{\ if $\Theta = \refenvsym{(}  \Theta'  \refenvsym{,}   \refenvmv{l} : \refenvnt{A}   \refenvsym{)}$} \\
  \token{lookupStore}  \refenvsym{(}  \Theta  \refenvsym{,}  \refenvmv{l}  \refenvsym{)} & = \token{lookupStore}  \refenvsym{(}  \Theta'  \refenvsym{,}  \refenvmv{l}  \refenvsym{)}\text{\ if $\Theta = \refenvsym{(}  \Theta'  \refenvsym{,}   \refenvmv{l'} : \refenvnt{A'}   \refenvsym{)}$ and $\refenvmv{l'} \neq \refenvmv{l}$}
\end{align*}

\section{Proofs}

\subsection{Basic Properties of Judgments}
\begin{lemma}[Regularity of Runtime Judgments]\label{claim:regularity-runtime-judgments}
  \begin{enumerate}
    %% nht well-formedness
    \item If\/ $ \vdash  \Psi_{{\mathrm{1}}}  \refenvsym{,}  \Psi_{{\mathrm{2}}} \ \token{wf} $,
          then $ \vdash  \Psi_{{\mathrm{1}}} \ \token{wf} $.
    \item If\/ $ \vdash  \Psi_{{\mathrm{1}}}  \refenvsym{,}   \binder{ \refenvmv{x} }: \refenvnt{A} \mathrel{@}\binder{ \gamma_{{\mathrm{1}}} } \mathbin{:\succeq} \gamma_{{\mathrm{2}}}   \refenvsym{,}  \Psi_{{\mathrm{2}}} \ \token{wf} $,
          then $ \Psi_{{\mathrm{1}}}  \vdash^{ \gamma_{{\mathrm{2}}} }  \refenvnt{A} \ \token{wf} $.
    \item[] We also use the following entry-wise consequences of reserved names typing well-formedness:
      \begin{enumerate}
        \item If\/ $ \vdash  \Psi_{{\mathrm{1}}}  \refenvsym{,}   \binder{ \refenvmv{x} }: \refenvnt{A} \mathrel{@}\binder{ \gamma_{{\mathrm{2}}} } \mathbin{:\succeq} \gamma_{{\mathrm{1}}}   \refenvsym{,}  \Psi_{{\mathrm{2}}} \ \token{wf} $,
              then $\gamma_{{\mathrm{1}}} \, \in \,  \token{Dom}_{C}( \Psi_{{\mathrm{1}}} ) $.
        \item If\/ $ \vdash  \Psi_{{\mathrm{1}}}  \refenvsym{,}   \binder{ \gamma_{{\mathrm{1}}} }( \mathbin{:\succeq} \; \gamma_{{\mathrm{2}}}  /  \mathbin{:\supseteq} \; \gamma_{{\mathrm{3}}} )   \refenvsym{,}  \Psi_{{\mathrm{2}}} \ \token{wf} $,
              then $\gamma_{{\mathrm{2}}} \, \in \,  \token{Dom}_{C}( \Psi_{{\mathrm{1}}} ) $ and $\gamma_{{\mathrm{3}}} \, \in \,  \token{Dom}_{C}( \Psi_{{\mathrm{1}}} ) $.
        \item If\/ $ \vdash  \Psi_{{\mathrm{1}}}  \refenvsym{,}   [    \binder{  \gamma _{ 0 }  }  \mathbin{:\succeq}    \delta _{ 0 }  ,\dotsc,\binder{  \gamma _{ \refenvnt{k} }  }  \mathbin{:\succeq}   \delta  _{ \refenvnt{k} }   ]   \refenvsym{,}  \Psi_{{\mathrm{2}}} \ \token{wf} $,
              then $ \delta _{ \refenvnt{i} }  \, \in \,  \token{Dom}_{C}( \Psi_{{\mathrm{1}}} ) $ for any $0\le\refenvnt{i}\le\refenvnt{k}$.
      \end{enumerate}
    %% classifier sequence well-formedness
    \item If\/ $\Psi  \vdash   \overrightarrow{ \gamma_{{\mathrm{1}}} }^{+}  \, \token{wf}$,
          then $\gamma_{{\mathrm{2}}} \, \in \,  \token{Dom}_{C}( \Psi ) $ for any $\gamma_{{\mathrm{2}}} \, \in \, \refenvsym{\{}   \overrightarrow{ \gamma_{{\mathrm{1}}} }^{+}   \refenvsym{\}}$.
    %% context well-formedness
    \item If\/ $ \Psi \mid^{  \overrightarrow{ \gamma_{{\mathrm{1}}} }^{+}  } \Gamma_{{\mathrm{1}}} \vdash^{  \overrightarrow{ \gamma_{{\mathrm{2}}} }^{+}  }\token{wf} $,
          then $ \vdash  \Psi \ \token{wf} $ and $\Psi  \vdash   \overrightarrow{ \gamma_{{\mathrm{1}}} }^{+}  \, \token{wf}$.
    \item If\/ $ \Psi \mid^{  \overrightarrow{ \gamma_{{\mathrm{1}}} }^{+}  } \Gamma_{{\mathrm{1}}}  \refenvsym{,}  \Gamma_{{\mathrm{2}}} \vdash^{  \overrightarrow{ \gamma_{{\mathrm{2}}} }^{+}  }\token{wf} $,
          then $ \Psi \mid^{  \overrightarrow{ \gamma_{{\mathrm{1}}} }^{+}  } \Gamma_{{\mathrm{1}}} \vdash^{  \overrightarrow{ \gamma_{{\mathrm{3}}} }^{+}  }\token{wf} $ for some $ \overrightarrow{ \gamma_{{\mathrm{3}}} }^{+} $.
    \item If\/ $ \Psi \mid^{  \overrightarrow{ \gamma_{{\mathrm{1}}} }^{+}  } \Gamma_{{\mathrm{1}}} \vdash^{  \overrightarrow{ \gamma_{{\mathrm{2}}} }^{+}   \refenvsym{,}   \overrightarrow{ \gamma_{{\mathrm{3}}} }  }\token{wf} $ and\ $\Gamma_{{\mathrm{1}}} = \Gamma_{{\mathrm{2}}}  \refenvsym{,}  \Gamma_{{\mathrm{3}}}$,
          then
          $ \Psi \mid^{  \overrightarrow{ \gamma_{{\mathrm{1}}} }^{+}  } \Gamma_{{\mathrm{2}}} \vdash^{  \overrightarrow{ \gamma_{{\mathrm{2}}} }^{+}  }\token{wf} $.
    \item If\/ $ \Psi \mid^{  \overrightarrow{ \gamma_{{\mathrm{1}}} }^{+}  } \Gamma_{{\mathrm{1}}}  \refenvsym{,}   \binder{ \refenvmv{x} }\mathord{:^{\binder{ \gamma_{{\mathrm{1}}} } } } \refenvnt{A}   \refenvsym{,}  \Gamma_{{\mathrm{3}}} \vdash^{  \overrightarrow{ \gamma_{{\mathrm{2}}} }^{+}  }\token{wf} $,
          then $ \Psi \mid^{  \overrightarrow{ \gamma_{{\mathrm{1}}} }^{+}  }  \Gamma_{{\mathrm{1}}} \vdash ^{  \overrightarrow{ \gamma_{{\mathrm{3}}} }^{+}  } \refenvnt{A} \ \token{wf} $
          for some $ \overrightarrow{ \gamma_{{\mathrm{3}}} }^{+} $.
    \item If\/ $ \Psi \mid^{  \overrightarrow{ \gamma_{{\mathrm{1}}} }^{+}  } \Gamma \vdash^{  \overrightarrow{ \gamma_{{\mathrm{2}}} }^{+}  }\token{wf} $ and $\delta \, \in \, \refenvsym{\{}   \overrightarrow{ \gamma_{{\mathrm{2}}} }^{+}   \refenvsym{\}}$,
          then $\delta \, \in \,  \token{Dom}_{C}( \Psi )  \, \cup \,  \token{Dom}_{C}( \Gamma ) $.
    \item If\/ $ \Psi \mid^{  \overrightarrow{ \gamma_{{\mathrm{1}}} }^{+}  } \Gamma \vdash^{  \overrightarrow{ \gamma_{{\mathrm{2}}} }^{+}  }\token{wf} $,
          then $ \token{FC}( \Gamma )  \subseteq  \token{Dom}_{C}( \Psi ) $.
    %% type well-formedness
    \item If\/ $ \Psi \mid^{  \overrightarrow{ \gamma_{{\mathrm{1}}} }^{+}  }  \Gamma \vdash ^{  \overrightarrow{ \gamma_{{\mathrm{2}}} }^{+}  } \refenvnt{A} \ \token{wf} $,
          then $ \Psi \mid^{  \overrightarrow{ \gamma_{{\mathrm{1}}} }^{+}  } \Gamma \vdash^{  \overrightarrow{ \gamma_{{\mathrm{2}}} }^{+}  }\token{wf} $.
    %% ltrans and gtrans
    \item If\/ $ \Psi \mid^{  \overrightarrow{ \gamma_{{\mathrm{1}}} }^{+}  } \Gamma \vdash \gamma_{{\mathrm{2}}} \preceq \gamma_{{\mathrm{3}}} $ or $ \Psi \mid^{  \overrightarrow{ \gamma_{{\mathrm{1}}} }^{+}  } \Gamma \vdash \gamma_{{\mathrm{2}}} \subseteq \gamma_{{\mathrm{3}}} $,
          then $ \Psi \mid^{  \overrightarrow{ \gamma_{{\mathrm{1}}} }^{+}  } \Gamma \vdash^{  \overrightarrow{ \gamma_{{\mathrm{4}}} }^{+}  }\token{wf} $ for some $ \overrightarrow{ \gamma_{{\mathrm{4}}} }^{+} $.
    \item If\/ $ \Psi \mid^{  \overrightarrow{ \gamma_{{\mathrm{1}}} }^{+}  } \Gamma \vdash \gamma_{{\mathrm{2}}} \preceq \gamma_{{\mathrm{3}}} $ or $ \Psi \mid^{  \overrightarrow{ \gamma_{{\mathrm{1}}} }^{+}  } \Gamma \vdash \gamma_{{\mathrm{2}}} \subseteq \gamma_{{\mathrm{3}}} $,
          then $\gamma_{{\mathrm{2}}} \, \in \,  \token{Dom}_{C}( \Psi )  \, \cup \,  \token{Dom}_{C}( \Gamma ) $ and $\gamma_{{\mathrm{3}}} \, \in \,  \token{Dom}_{C}( \Psi )  \, \cup \,  \token{Dom}_{C}( \Gamma ) $.
    %% Expression typing
    \item \label{claim:regularity-runtime-judgments-exp-typing}
          If\/ $ \Psi \mid^{  \overrightarrow{ \gamma_{{\mathrm{1}}} }^{+}  }  \Gamma \vdash^{  \overrightarrow{ \gamma_{{\mathrm{2}}} }^{+}  }_{ R }  \refenvnt{e} : \refenvnt{A} $,
          then $ \Psi \mid^{  \overrightarrow{ \gamma_{{\mathrm{1}}} }^{+}  }  \Gamma \vdash ^{  \overrightarrow{ \gamma_{{\mathrm{2}}} }^{+}  } \refenvnt{A} \ \token{wf} $.
    %% Store typing well-formedness
    \item If\/ $ \Psi  \vdash  \Theta \ \token{wf} $,
          then $ \vdash  \Psi \ \token{wf} $.
    \item If\/ $ \Psi  \vdash  \Theta_{{\mathrm{1}}}  \refenvsym{,}  \Theta_{{\mathrm{2}}} \ \token{wf} $,
          then $ \Psi  \vdash  \Theta_{{\mathrm{1}}} \ \token{wf} $.
    \item If\/ $ \Psi  \vdash  \Theta_{{\mathrm{1}}}  \refenvsym{,}   \refenvmv{l} : \refenvnt{A}   \refenvsym{,}  \Theta_{{\mathrm{2}}} \ \token{wf} $,
          then $ \Psi  \vdash^{ \gamma }  \refenvnt{A} \ \token{wf} $ for some $\gamma$.
    %% Store typing
    \item If\/ $\Psi  \vdash  S  \colon  \Theta$,
          then $ \Psi  \vdash  \Theta \ \token{wf} $.
    %% Value typing
    \item If\/ $ \Psi \mid \Theta \vdash^{ \gamma } \refenvnt{v} : \refenvnt{A} \ \token{val} $,
          then $ \Psi  \vdash^{ \gamma }  \refenvnt{A} \ \token{wf} $ and $ \Psi  \vdash  \Theta \ \token{wf} $.
    %% Value Environment well-formedness
    \item If\/ $ \Psi \mid \Theta \vdash^{ \gamma } E \ \token{wf} $,
          then $\Psi  \vdash  \gamma \, \token{wf}$ and $ \Psi  \vdash  \Theta \ \token{wf} $.
    \item If\/ $ \Psi \mid \Theta \vdash^{ \gamma_{{\mathrm{1}}} } E_{{\mathrm{1}}}  \refenvsym{,}  E_{{\mathrm{2}}} \ \token{wf} $,
          then $ \Psi \mid \Theta \vdash^{ \gamma_{{\mathrm{2}}} } E_{{\mathrm{1}}} \ \token{wf} $ for some $\gamma_{{\mathrm{2}}}$.
    \item If\/ $ \Psi \mid \Theta \vdash^{ \gamma_{{\mathrm{1}}} } E_{{\mathrm{1}}}  \refenvsym{,}  \refenvmv{x}  \coloneqq  \refenvnt{v}  \refenvsym{,}  E_{{\mathrm{2}}} \ \token{wf} $,
          then $\refenvmv{x} \, \in \,  \token{Dom}_{V}( \Psi ) $ and $ \Psi \mid \Theta \vdash^{ \gamma_{{\mathrm{2}}} } \refenvnt{v} : \refenvnt{A} \ \token{val} $ for some $\refenvnt{A}$ and $\gamma_{{\mathrm{2}}}$.
  \end{enumerate}
\end{lemma}

\begin{proof}
  By induction on the derivation of each judgment.
  The entry-wise consequences for reserved names typing well-formedness follow by inversion of the corresponding reserved names typing well-formedness rule, after peeling any suffix of the reserved names typing with the first item.
  The classifier-stack containment fact and the reachability/visibility endpoint fact are proved simultaneously: the context-variable and context-shut cases use classifier-stack containment for the relevant prefix, while the open-context case uses the visibility endpoint fact.
  The reserved names typing cases of reachability and visibility use the entry-wise consequences above.
  For \zcref{claim:regularity-runtime-judgments-exp-typing},
  we use \zcref{claim:runtime-monotonicity-type-wellformedness}.
\end{proof}

\begin{definition}[Stratified Contexts]
  For any $\refenvnt{k_{{\mathrm{1}}}}, \refenvnt{k_{{\mathrm{2}}}}$ such that $0 \le \refenvnt{k_{{\mathrm{1}}}} \le \refenvnt{k_{{\mathrm{2}}}}$, $ \token{Ctx}^{ \refenvnt{k_{{\mathrm{1}}}} , \refenvnt{k_{{\mathrm{2}}}} } $ is the set of contexts.
  We annotate a context like $ \Gamma ^{ \refenvnt{k_{{\mathrm{1}}}} , \refenvnt{k_{{\mathrm{2}}}} } $ to clarify that it is a member of $ \token{Ctx}^{ \refenvnt{k_{{\mathrm{1}}}} , \refenvnt{k_{{\mathrm{2}}}} } $.
  They are defined mutually recursively as follows.
  \[
       \Gamma ^{ \refenvnt{k_{{\mathrm{1}}}} , \refenvnt{k_{{\mathrm{2}}}} }  \in  \token{Ctx}^{ \refenvnt{k_{{\mathrm{1}}}} , \refenvnt{k_{{\mathrm{2}}}} }  \Coloneqq  \varepsilon  \text{(where $\refenvnt{k_{{\mathrm{1}}}} = \refenvnt{k_{{\mathrm{2}}}}$ )}  \mid   \binder{ \refenvmv{x} }\mathord{:^{\binder{ \gamma } } } \refenvnt{A}   \refenvsym{,}  \Gamma ^{ \refenvnt{k_{{\mathrm{1}}}} , \refenvnt{k_{{\mathrm{2}}}} }  \mid   \blacktriangleright ^{ \delta }   \refenvsym{,}  \Gamma ^{ \refenvnt{k_{{\mathrm{1}}}}  \refenvsym{+}  1 , \refenvnt{k_{{\mathrm{2}}}} }  \mid   \blacktriangleleft _{ \refenvnt{k_{{\mathrm{3}}}} }^{\binder{ \gamma } }   \refenvsym{,}  \Gamma ^{ \refenvnt{k_{{\mathrm{1}}}}  \refenvsym{-}  \refenvnt{k_{{\mathrm{3}}}} , \refenvnt{k_{{\mathrm{2}}}} }  \text{(where $\refenvnt{k_{{\mathrm{1}}}} \ge \refenvnt{k_{{\mathrm{3}}}}$ )}  \mid   [  \varrho  ]^{\binder{ \gamma } }   \refenvsym{,}  \Gamma ^{ \refenvnt{k_{{\mathrm{1}}}} , \refenvnt{k_{{\mathrm{2}}}} } 
  \]
\end{definition}

\begin{lemma}[Monotonicity for Runtime Reachability, Visibility, and Type Well-formedness]
  \label{claim:runtime-monotonicity-type-wellformedness}
  \begin{enumerate}
    \item If\/
          $ \Psi \mid^{  \overrightarrow{ \gamma_{{\mathrm{1}}} }   \refenvsym{,}  \gamma_{{\mathrm{2}}} }  \Gamma_{{\mathrm{1}}}  \refenvsym{,}  \Gamma_{{\mathrm{2}}} ^{ 0 , \refenvnt{k} }  \vdash \delta_{{\mathrm{1}}} \preceq \delta_{{\mathrm{2}}} $,
          $ \Psi \mid^{  \overrightarrow{ \gamma_{{\mathrm{1}}} }   \refenvsym{,}  \gamma_{{\mathrm{2}}} } \Gamma_{{\mathrm{1}}} \vdash^{  \dotsc   \refenvsym{,}  \gamma_{{\mathrm{4}}} }\token{wf} $,
          $ \Psi \mid^{  \overrightarrow{ \gamma_{{\mathrm{1}}} }   \refenvsym{,}  \gamma_{{\mathrm{2}}} } \Gamma_{{\mathrm{1}}}  \refenvsym{,}  \Gamma_{{\mathrm{3}}} \vdash^{  \dotsc   \refenvsym{,}  \gamma_{{\mathrm{5}}} }\token{wf} $,
          $ \Psi \mid^{  \overrightarrow{ \gamma_{{\mathrm{1}}} }   \refenvsym{,}  \gamma_{{\mathrm{2}}} }  \Gamma_{{\mathrm{1}}}  \refenvsym{,}  \Gamma_{{\mathrm{3}}}  \refenvsym{,}  \Gamma_{{\mathrm{2}}} ^{ 0 , \refenvnt{k} }  \vdash^{  \dotsc  }\token{wf} $, and
          $ \Psi \mid^{  \overrightarrow{ \gamma_{{\mathrm{1}}} }   \refenvsym{,}  \gamma_{{\mathrm{2}}} } \Gamma_{{\mathrm{1}}}  \refenvsym{,}  \Gamma_{{\mathrm{3}}} \vdash \gamma_{{\mathrm{4}}} \preceq \gamma_{{\mathrm{5}}} $,
          then
          $ \Psi \mid^{  \overrightarrow{ \gamma_{{\mathrm{1}}} }   \refenvsym{,}  \gamma_{{\mathrm{2}}} }  \Gamma_{{\mathrm{1}}}  \refenvsym{,}  \Gamma_{{\mathrm{3}}}  \refenvsym{,}  \Gamma_{{\mathrm{2}}} ^{ 0 , \refenvnt{k} }  \vdash \delta_{{\mathrm{1}}} \preceq \delta_{{\mathrm{2}}} $.
    \item If\/
          $ \Psi \mid^{  \overrightarrow{ \gamma_{{\mathrm{1}}} }   \refenvsym{,}  \gamma_{{\mathrm{2}}} }  \Gamma_{{\mathrm{1}}}  \refenvsym{,}  \Gamma_{{\mathrm{2}}} ^{ 0 , \refenvnt{k} }  \vdash \delta_{{\mathrm{1}}} \subseteq \delta_{{\mathrm{2}}} $,
          $ \Psi \mid^{  \overrightarrow{ \gamma_{{\mathrm{1}}} }   \refenvsym{,}  \gamma_{{\mathrm{2}}} } \Gamma_{{\mathrm{1}}} \vdash^{  \dotsc   \refenvsym{,}  \gamma_{{\mathrm{4}}} }\token{wf} $,
          $ \Psi \mid^{  \overrightarrow{ \gamma_{{\mathrm{1}}} }   \refenvsym{,}  \gamma_{{\mathrm{2}}} } \Gamma_{{\mathrm{1}}}  \refenvsym{,}  \Gamma_{{\mathrm{3}}} \vdash^{  \dotsc   \refenvsym{,}  \gamma_{{\mathrm{5}}} }\token{wf} $,
          $ \Psi \mid^{  \overrightarrow{ \gamma_{{\mathrm{1}}} }   \refenvsym{,}  \gamma_{{\mathrm{2}}} }  \Gamma_{{\mathrm{1}}}  \refenvsym{,}  \Gamma_{{\mathrm{3}}}  \refenvsym{,}  \Gamma_{{\mathrm{2}}} ^{ 0 , \refenvnt{k} }  \vdash^{  \dotsc  }\token{wf} $, and
          $ \Psi \mid^{  \overrightarrow{ \gamma_{{\mathrm{1}}} }   \refenvsym{,}  \gamma_{{\mathrm{2}}} } \Gamma_{{\mathrm{1}}}  \refenvsym{,}  \Gamma_{{\mathrm{3}}} \vdash \gamma_{{\mathrm{4}}} \preceq \gamma_{{\mathrm{5}}} $,
          then
          $ \Psi \mid^{  \overrightarrow{ \gamma_{{\mathrm{1}}} }   \refenvsym{,}  \gamma_{{\mathrm{2}}} }  \Gamma_{{\mathrm{1}}}  \refenvsym{,}  \Gamma_{{\mathrm{3}}}  \refenvsym{,}  \Gamma_{{\mathrm{2}}} ^{ 0 , \refenvnt{k} }  \vdash \delta_{{\mathrm{1}}} \subseteq \delta_{{\mathrm{2}}} $.
    \item If\/
          $ \Psi \mid^{  \overrightarrow{ \gamma_{{\mathrm{1}}} }   \refenvsym{,}  \gamma_{{\mathrm{2}}} }   \Gamma_{{\mathrm{1}}}  \refenvsym{,}  \Gamma_{{\mathrm{2}}} ^{ 0 , \refenvnt{k} }  \vdash ^{  \overrightarrow{ \gamma_{{\mathrm{3}}} }^{+}  } \refenvnt{A} \ \token{wf} $,
          $ \Psi \mid^{  \overrightarrow{ \gamma_{{\mathrm{1}}} }   \refenvsym{,}  \gamma_{{\mathrm{2}}} } \Gamma_{{\mathrm{1}}} \vdash^{  \dotsc   \refenvsym{,}  \gamma_{{\mathrm{4}}} }\token{wf} $,
          $ \Psi \mid^{  \overrightarrow{ \gamma_{{\mathrm{1}}} }   \refenvsym{,}  \gamma_{{\mathrm{2}}} } \Gamma_{{\mathrm{1}}}  \refenvsym{,}  \Gamma_{{\mathrm{3}}} \vdash^{  \dotsc   \refenvsym{,}  \gamma_{{\mathrm{5}}} }\token{wf} $,
          $ \Psi \mid^{  \overrightarrow{ \gamma_{{\mathrm{1}}} }   \refenvsym{,}  \gamma_{{\mathrm{2}}} }  \Gamma_{{\mathrm{1}}}  \refenvsym{,}  \Gamma_{{\mathrm{3}}}  \refenvsym{,}  \Gamma_{{\mathrm{2}}} ^{ 0 , \refenvnt{k} }  \vdash^{  \dotsc  }\token{wf} $, and
          $ \Psi \mid^{  \overrightarrow{ \gamma_{{\mathrm{1}}} }   \refenvsym{,}  \gamma_{{\mathrm{2}}} } \Gamma_{{\mathrm{1}}}  \refenvsym{,}  \Gamma_{{\mathrm{3}}} \vdash \gamma_{{\mathrm{4}}} \preceq \gamma_{{\mathrm{5}}} $,
          then
          $ \Psi \mid^{  \overrightarrow{ \gamma_{{\mathrm{1}}} }   \refenvsym{,}  \gamma_{{\mathrm{2}}} }   \Gamma_{{\mathrm{1}}}  \refenvsym{,}  \Gamma_{{\mathrm{3}}}  \refenvsym{,}  \Gamma_{{\mathrm{2}}} ^{ 0 , \refenvnt{k} }  \vdash ^{  \overrightarrow{ \gamma_{{\mathrm{6}}} }^{+}  } \refenvnt{A} \ \token{wf} $
          for some $ \overrightarrow{ \gamma_{{\mathrm{6}}} }^{+} $.
  \end{enumerate}
\end{lemma}

\begin{proof}
  By induction on the derivation of each judgment.
\end{proof}


\subsection{Properties on Reachability/Visibility Judgments}
% \begin{notation}
%   We write $ \Gamma ^{\pos{ \gamma } } $ if a classifier $\gamma$ is declared at the rightmost element of a context $\Gamma$.
%   More concretely, $ \Gamma ^{\pos{ \gamma } } $ indicates one of the following situations:
%   \begin{enumerate}
%     \item $\Gamma = \Gamma'  \refenvsym{,}   \binder{ \refenvmv{x} }\mathord{:^{\binder{ \gamma } } } \refenvnt{A} $
%     \item $\Gamma = \Gamma'  \refenvsym{,}   \blacktriangleleft _{ \refenvnt{k} }^{\binder{ \gamma } } $
%     \item $\Gamma = \Gamma'  \refenvsym{,}   [  \varrho  ]^{\binder{ \gamma } } $
%     \item $\Gamma = \Gamma'  \refenvsym{,}   [  \varrho  ]^{\binder{ \gamma' } } $ where $\gamma \, \in \,  \token{Dom}_{C}( \varrho ) $
%   \end{enumerate}
% \end{notation}

\begin{definition}
  Given $ \Psi \mid^{ \delta_{{\mathrm{1}}} } \Gamma \vdash^{  \overrightarrow{ \delta_{{\mathrm{2}}} }  }\token{wf} $ and $\gamma \, \in \,  \token{Dom}_{C}( \Psi )  \, \cup \,  \token{Dom}_{C}( \Gamma ) $, $ \token{len} ( \Psi , \Gamma ) $ returns the number of classifiers declared in $\Psi$ and $\Gamma$.
  \begin{align*}
     \token{len} ( \varepsilon , \varepsilon )  &= 0 \\
     \token{len} ( \refenvsym{(}  \Psi  \refenvsym{,}   \binder{ \refenvmv{x} }: \refenvnt{A} \mathrel{@}\binder{ \gamma_{{\mathrm{1}}} } \mathbin{:\succeq} \gamma_{{\mathrm{2}}}   \refenvsym{)} , \varepsilon )  &=  \token{len} ( \Psi , \varepsilon )   \refenvsym{+}  1 \\
     \token{len} ( \refenvsym{(}  \Psi  \refenvsym{,}   \binder{ \gamma_{{\mathrm{1}}} }( \mathbin{:\succeq} \; \gamma_{{\mathrm{2}}}  /  \mathbin{:\supseteq} \; \gamma_{{\mathrm{3}}} )   \refenvsym{)} , \varepsilon )  &=  \token{len} ( \Psi , \varepsilon )   \refenvsym{+}  1 \\
     \token{len} ( \refenvsym{(}  \Psi  \refenvsym{,}   [    \binder{  \gamma _{ 1 }  }  \mathbin{:\succeq}    \delta _{ 1 }  ,\dotsc,\binder{  \gamma _{ \refenvnt{k} }  }  \mathbin{:\succeq}   \delta  _{ \refenvnt{k} }   ]   \refenvsym{)} , \varepsilon )  &=  \token{len} ( \Psi , \varepsilon )   \refenvsym{+}  \refenvnt{k} \\
     \token{len} ( \Psi , \refenvsym{(}  \Gamma  \refenvsym{,}   \binder{ \refenvmv{x} }\mathord{:^{\binder{ \gamma } } } \refenvnt{A}   \refenvsym{)} )  & =  \token{len} ( \Psi , \Gamma )   \refenvsym{+}  1 \\
     \token{len} ( \Psi , \refenvsym{(}  \Gamma  \refenvsym{,}   \blacktriangleright ^{ \gamma }   \refenvsym{)} )  &=  \token{len} ( \Psi , \Gamma )  \\
     \token{len} ( \Psi , \refenvsym{(}  \Gamma  \refenvsym{,}   \blacktriangleleft _{ \refenvnt{k} }^{\binder{ \gamma } }   \refenvsym{)} )  & =  \token{len} ( \Psi , \Gamma )   \refenvsym{+}  1 \\
     \token{len} ( \Psi , \refenvsym{(}  \Gamma  \refenvsym{,}   [    \binder{  \gamma _{ 1 }  }  \mathbin{:\succeq}    \gamma' _{ 1 }  ,\dotsc,\binder{  \gamma _{ \refenvnt{k} }  }  \mathbin{:\succeq}   \gamma'  _{ \refenvnt{k} }   ]^{\binder{  \gamma _{ 0 }  } }   \refenvsym{)} )  & =  \token{len} ( \Psi , \Gamma )   \refenvsym{+}  \refenvnt{k}  \refenvsym{+}  1
  \end{align*}

  We also define $ \token{deg} ( \Psi , \Gamma , \gamma ) $ as the position at which $\gamma$ occurs among the classifiers declared in $\Psi$ and $\Gamma$.
  \begin{align*}
     \token{deg} ( \Psi , \Gamma ,  \exclam  )  & = 0 \\
     \token{deg} ( \refenvsym{(}  \Psi_{{\mathrm{1}}}  \refenvsym{,}   \binder{ \refenvmv{x} }: \refenvnt{A} \mathrel{@}\binder{ \gamma_{{\mathrm{1}}} } \mathbin{:\succeq} \gamma_{{\mathrm{2}}}   \refenvsym{,}  \Psi_{{\mathrm{2}}}  \refenvsym{)} , \Gamma , \gamma_{{\mathrm{1}}} )  & =  \token{len} ( \Psi_{{\mathrm{1}}} , \varepsilon )   \refenvsym{+}  1 \\
     \token{deg} ( \refenvsym{(}  \Psi_{{\mathrm{1}}}  \refenvsym{,}   \binder{ \gamma_{{\mathrm{1}}} }( \mathbin{:\succeq} \; \gamma_{{\mathrm{2}}}  /  \mathbin{:\supseteq} \; \gamma_{{\mathrm{3}}} )   \refenvsym{,}  \Psi_{{\mathrm{2}}}  \refenvsym{)} , \Gamma , \gamma_{{\mathrm{1}}} )  & =  \token{len} ( \Psi_{{\mathrm{1}}} , \varepsilon )   \refenvsym{+}  1 \\
     \token{deg} ( \refenvsym{(}  \Psi_{{\mathrm{1}}}  \refenvsym{,}   [    \binder{  \gamma _{ 1 }  }  \mathbin{:\succeq}    \delta _{ 1 }  ,\dotsc,\binder{  \gamma _{ \refenvnt{k} }  }  \mathbin{:\succeq}   \delta  _{ \refenvnt{k} }   ]   \refenvsym{,}  \Psi_{{\mathrm{2}}}  \refenvsym{)} , \Gamma ,  \gamma _{ \refenvnt{i} }  )  & =  \token{len} ( \Psi_{{\mathrm{1}}} , \varepsilon )   \refenvsym{+}  \refenvnt{k}  \refenvsym{-}  \refenvnt{i}  \refenvsym{+}  1 \\
     \token{deg} ( \Psi , \refenvsym{(}  \Gamma_{{\mathrm{1}}}  \refenvsym{,}   \binder{ \refenvmv{x} }\mathord{:^{\binder{ \gamma } } } \refenvnt{A}   \refenvsym{,}  \Gamma_{{\mathrm{2}}}  \refenvsym{)} , \gamma )  &=  \token{len} ( \Psi , \Gamma_{{\mathrm{1}}} )   \refenvsym{+}  1 \\
     \token{deg} ( \Psi , \refenvsym{(}  \Gamma_{{\mathrm{1}}}  \refenvsym{,}   \blacktriangleleft _{ \refenvnt{k} }^{\binder{ \gamma } }   \refenvsym{,}  \Gamma_{{\mathrm{2}}}  \refenvsym{)} , \gamma )  & =  \token{len} ( \Psi , \Gamma_{{\mathrm{1}}} )   \refenvsym{+}  1 \\
     \token{deg} ( \Psi , \refenvsym{(}  \Gamma_{{\mathrm{1}}}  \refenvsym{,}   [    \binder{  \gamma _{ 1 }  }  \mathbin{:\succeq}    \gamma' _{ 1 }  ,\dotsc,\binder{  \gamma _{ \refenvnt{k} }  }  \mathbin{:\succeq}   \gamma'  _{ \refenvnt{k} }   ]^{\binder{  \gamma _{ 0 }  } }   \refenvsym{,}  \Gamma_{{\mathrm{2}}}  \refenvsym{)} ,  \gamma _{ \refenvnt{i} }  )  & =  \token{len} ( \Psi , \Gamma_{{\mathrm{1}}} )   \refenvsym{+}  \refenvnt{k}  \refenvsym{-}  \refenvnt{i}  \refenvsym{+}  1
  \end{align*}
\end{definition}

\begin{lemma}\label{claim:deg-preserves-trans-order}
  If either $ \Psi \mid^{ \gamma_{{\mathrm{1}}} } \Gamma \vdash \gamma_{{\mathrm{2}}} \preceq \gamma_{{\mathrm{3}}} $ or $ \Psi \mid^{ \gamma_{{\mathrm{1}}} } \Gamma \vdash \gamma_{{\mathrm{2}}} \subseteq \gamma_{{\mathrm{3}}} $ holds,
  then $ \token{deg} ( \Psi , \Gamma , \gamma_{{\mathrm{2}}} )  \le  \token{deg} ( \Psi , \Gamma , \gamma_{{\mathrm{3}}} ) $.
  Moreover, the inequality is strict whenever $\gamma_{{\mathrm{2}}} \neq \gamma_{{\mathrm{3}}}$.
\end{lemma}

\begin{proof}
  By induction on the derivation of $ \Psi \mid^{ \gamma_{{\mathrm{1}}} } \Gamma_{{\mathrm{2}}} \vdash \gamma_{{\mathrm{2}}} \preceq \gamma_{{\mathrm{3}}} $ or $ \Psi \mid^{ \gamma_{{\mathrm{1}}} } \Gamma_{{\mathrm{2}}} \vdash \gamma_{{\mathrm{2}}} \subseteq \gamma_{{\mathrm{3}}} $.
\end{proof}

\begin{lemma}[Antisymmetry of $ \preceq $ and $ \subseteq $]\label{claim:trans-antisymmetry}
  If\/ $ \Psi \mid^{ \gamma_{{\mathrm{1}}} } \Gamma \vdash \gamma_{{\mathrm{2}}} \preceq \gamma_{{\mathrm{3}}} $ and\/ $ \Psi \mid^{ \gamma_{{\mathrm{1}}} } \Gamma \vdash \gamma_{{\mathrm{3}}} \preceq \gamma_{{\mathrm{2}}} $, then $\gamma_{{\mathrm{2}}}  \refenvsym{=}  \gamma_{{\mathrm{3}}}$.
  Similarly, If\/ $ \Psi \mid^{ \gamma_{{\mathrm{1}}} } \Gamma \vdash \gamma_{{\mathrm{2}}} \subseteq \gamma_{{\mathrm{3}}} $ and\/ $ \Psi \mid^{ \gamma_{{\mathrm{1}}} } \Gamma \vdash \gamma_{{\mathrm{3}}} \subseteq \gamma_{{\mathrm{2}}} $, then $\gamma_{{\mathrm{2}}}  \refenvsym{=}  \gamma_{{\mathrm{3}}}$.
\end{lemma}

\begin{proof}
  We show the first statement; the second is analogous.
  Suppose, for contradiction, that $\gamma_{{\mathrm{2}}} \neq \gamma_{{\mathrm{3}}}$.
  By \zcref{claim:deg-preserves-trans-order} applied to
  $ \Psi \mid^{ \gamma_{{\mathrm{1}}} } \Gamma \vdash \gamma_{{\mathrm{2}}} \preceq \gamma_{{\mathrm{3}}} $, we have
  $ \token{deg} ( \Psi , \Gamma , \gamma_{{\mathrm{2}}} )  <  \token{deg} ( \Psi , \Gamma , \gamma_{{\mathrm{3}}} ) $.
  Applying the same lemma to $ \Psi \mid^{ \gamma_{{\mathrm{1}}} } \Gamma \vdash \gamma_{{\mathrm{3}}} \preceq \gamma_{{\mathrm{2}}} $ gives
  $ \token{deg} ( \Psi , \Gamma , \gamma_{{\mathrm{3}}} )  <  \token{deg} ( \Psi , \Gamma , \gamma_{{\mathrm{2}}} ) $.
  This is impossible.  Hence $\gamma_{{\mathrm{2}}}  \refenvsym{=}  \gamma_{{\mathrm{3}}}$.
\end{proof}

\begin{lemma}\label{claim:local-to-global-trans}
  \begin{enumerate}
    \item If\/ $ \Psi \mid^{ \delta_{{\mathrm{1}}} } \Gamma \vdash \gamma_{{\mathrm{1}}} \preceq \gamma_{{\mathrm{2}}} $ and $\gamma_{{\mathrm{2}}} \, \in \,  \token{Dom}_{C}( \Psi ) $,
          then $\Psi  \vdash  \gamma_{{\mathrm{1}}}  \preceq  \gamma_{{\mathrm{2}}}$.
    \item If\/ $ \Psi \mid^{ \delta_{{\mathrm{1}}} } \Gamma \vdash \gamma_{{\mathrm{1}}} \subseteq \gamma_{{\mathrm{2}}} $ and $\gamma_{{\mathrm{2}}} \, \in \,  \token{Dom}_{C}( \Psi ) $,
          then $\Psi  \vdash  \gamma_{{\mathrm{1}}}  \subseteq  \gamma_{{\mathrm{2}}}$.
  \end{enumerate}
\end{lemma}

\begin{proof}
We prove both statements by induction on the given derivation.
Since $\gamma_{{\mathrm{2}}} \, \in \,  \token{Dom}_{C}( \Psi ) $,
\zcref{claim:deg-preserves-trans-order} implies $\gamma_{{\mathrm{1}}} \, \in \,  \token{Dom}_{C}( \Psi ) $; the remaining argument is straightforward.
\end{proof}

\begin{lemma}\label{claim:global-to-local-trans}
  \begin{enumerate}
    \item If\/ $\Psi  \vdash  \gamma_{{\mathrm{1}}}  \preceq  \gamma_{{\mathrm{2}}}$ and $ \Psi \mid^{ \delta } \Gamma \vdash^{  \dotsc  }\token{wf} $,
          then $ \Psi \mid^{ \delta } \Gamma \vdash \gamma_{{\mathrm{1}}} \preceq \gamma_{{\mathrm{2}}} $.
    \item If\/ $\Psi  \vdash  \gamma_{{\mathrm{1}}}  \subseteq  \gamma_{{\mathrm{2}}}$ and $ \Psi \mid^{ \delta } \Gamma \vdash^{  \dotsc  }\token{wf} $,
          then $ \Psi \mid^{ \delta } \Gamma \vdash \gamma_{{\mathrm{1}}} \subseteq \gamma_{{\mathrm{2}}} $.
  \end{enumerate}
\end{lemma}

\begin{proof}
  By induction on the given derivation.
\end{proof}

\begin{lemma}[Inversion for $ \preceq $ w.r.t. Reserved Names Typing]
  \label{claim:inversion-runtime-ltrans-nht}
  If\/ $\Psi  \vdash  \gamma_{{\mathrm{1}}}  \preceq  \gamma_{{\mathrm{2}}}$ and $\gamma_{{\mathrm{1}}} \neq \gamma_{{\mathrm{2}}}$, then the following hold:
  \begin{enumerate}
    \item If\/ $ \binder{ \refenvmv{x} }: \refenvnt{A} \mathrel{@}\binder{ \gamma_{{\mathrm{2}}} } \mathbin{:\succeq} \delta_{{\mathrm{1}}}  \, \in \, \Psi$,
          then $\Psi  \vdash  \gamma_{{\mathrm{1}}}  \preceq  \delta_{{\mathrm{1}}}$.
    \item If\/ $ \binder{ \gamma_{{\mathrm{2}}} }( \mathbin{:\succeq} \; \delta_{{\mathrm{1}}}  /  \mathbin{:\supseteq} \; \delta_{{\mathrm{2}}} )  \, \in \, \Psi$,
          then $\Psi  \vdash  \gamma_{{\mathrm{1}}}  \preceq  \delta_{{\mathrm{1}}}$.
    \item If\/ $ [    \binder{  \gamma _{ 0 }  }  \mathbin{:\succeq}    \gamma' _{ 0 }  ,\dotsc,\binder{  \gamma _{ \refenvnt{k} }  }  \mathbin{:\succeq}   \gamma'  _{ \refenvnt{k} }   ]  \, \in \, \Psi$
          and $\gamma_{{\mathrm{2}}}  \refenvsym{=}   \gamma _{ \refenvnt{i} } $ for some $\refenvnt{i}$ with $0 \le \refenvnt{i} \le \refenvnt{k}$,
          then $\Psi  \vdash  \gamma_{{\mathrm{1}}}  \preceq   \gamma' _{ \refenvnt{i} } $.
  \end{enumerate}
\end{lemma}

\begin{proof}
  By induction on the given derivation.
\end{proof}

\begin{lemma}[Inversion for $ \preceq $ w.r.t. Context]
  \label{claim:inversion-runtime-ltrans-ctx}
  If\/ $ \Psi \mid^{ \delta_{{\mathrm{1}}} } \Gamma \vdash \gamma_{{\mathrm{1}}} \preceq \gamma_{{\mathrm{2}}} $,  $\gamma_{{\mathrm{1}}} \neq \gamma_{{\mathrm{2}}}$ and $\gamma_{{\mathrm{2}}} \, \in \,  \token{Dom}_{C}( \Gamma ) $, then the following hold:
  \begin{enumerate}
    \item If\/ $\Gamma = \Gamma_{{\mathrm{1}}}  \refenvsym{,}   \binder{ \refenvmv{x} }\mathord{:^{\binder{ \gamma_{{\mathrm{2}}} } } } \refenvnt{A}   \refenvsym{,}  \Gamma_{{\mathrm{2}}}$
          and $ \Psi \mid^{ \delta_{{\mathrm{1}}} } \Gamma_{{\mathrm{1}}} \vdash^{  \dotsc   \refenvsym{,}  \delta_{{\mathrm{2}}} }\token{wf} $,
          then $ \Psi \mid^{ \delta_{{\mathrm{1}}} } \Gamma \vdash \gamma_{{\mathrm{1}}} \preceq \delta_{{\mathrm{2}}} $.
    \item If\/ $\Gamma = \Gamma_{{\mathrm{1}}}  \refenvsym{,}   \blacktriangleleft _{ \refenvnt{k} }^{\binder{ \gamma_{{\mathrm{2}}} } }   \refenvsym{,}  \Gamma_{{\mathrm{2}}}$
          and $ \Psi \mid^{ \delta_{{\mathrm{1}}} } \Gamma_{{\mathrm{1}}} \vdash^{  \dotsc   \refenvsym{,}  \delta_{{\mathrm{2}}} }\token{wf} $,
          then $ \Psi \mid^{ \delta_{{\mathrm{1}}} } \Gamma \vdash \gamma_{{\mathrm{1}}} \preceq \delta_{{\mathrm{2}}} $.
    \item If\/ $\Gamma = \Gamma_{{\mathrm{1}}}  \refenvsym{,}   [    \binder{  \gamma' _{ 1 }  }  \mathbin{:\succeq}    \gamma'' _{ 1 }  ,\dotsc,\binder{  \gamma' _{ \refenvnt{k} }  }  \mathbin{:\succeq}   \gamma''  _{ \refenvnt{k} }   ]^{\binder{ \gamma_{{\mathrm{2}}} } }   \refenvsym{,}  \Gamma_{{\mathrm{2}}}$
          and $ \Psi \mid^{ \delta_{{\mathrm{1}}} } \Gamma_{{\mathrm{1}}} \vdash^{  \dotsc   \refenvsym{,}  \delta_{{\mathrm{2}}} }\token{wf} $,
          then $ \Psi \mid^{ \delta_{{\mathrm{1}}} } \Gamma \vdash \gamma_{{\mathrm{1}}} \preceq \delta_{{\mathrm{2}}} $.
    \item If\/ $\Gamma = \Gamma_{{\mathrm{1}}}  \refenvsym{,}   [    \binder{  \gamma' _{ 1 }  }  \mathbin{:\succeq}    \gamma'' _{ 1 }  ,\dotsc,\binder{  \gamma' _{ \refenvnt{k} }  }  \mathbin{:\succeq}   \gamma''  _{ \refenvnt{k} }   ]^{\binder{  \gamma' _{ 0 }  } }   \refenvsym{,}  \Gamma_{{\mathrm{2}}}$
          and $ \gamma' _{ \refenvnt{i} }  = \gamma_{{\mathrm{2}}}$ for some $\refenvnt{i}$ with $1 \le \refenvnt{i} \le \refenvnt{k}$,
          then $ \Psi \mid^{ \delta_{{\mathrm{1}}} } \Gamma \vdash \gamma_{{\mathrm{1}}} \preceq  \gamma'' _{ \refenvnt{i} }  $.
  \end{enumerate}
\end{lemma}

\begin{proof}
  By induction on the given derivation.
\end{proof}

\begin{lemma}[Inversion for $ \subseteq $ w.r.t. Reserved Names Typing]
  \label{claim:inversion-runtime-gtrans-nht}
  If\/ $\Psi  \vdash  \gamma_{{\mathrm{1}}}  \subseteq  \gamma_{{\mathrm{2}}}$ and $\gamma_{{\mathrm{1}}} \neq \gamma_{{\mathrm{2}}}$, then the following hold:
  \begin{enumerate}
    \item If\/ $ \binder{ \refenvmv{x} }: \refenvnt{A} \mathrel{@}\binder{ \gamma_{{\mathrm{2}}} } \mathbin{:\succeq} \delta_{{\mathrm{1}}}  \, \in \, \Psi$,
          then $\Psi  \vdash  \gamma_{{\mathrm{1}}}  \subseteq  \delta_{{\mathrm{1}}}$.
    \item If\/ $ \binder{ \gamma_{{\mathrm{2}}} }( \mathbin{:\succeq} \; \delta_{{\mathrm{1}}}  /  \mathbin{:\supseteq} \; \delta_{{\mathrm{2}}} )  \, \in \, \Psi$,
          then $\Psi  \vdash  \gamma_{{\mathrm{1}}}  \subseteq  \delta_{{\mathrm{1}}}$ or $\Psi  \vdash  \gamma_{{\mathrm{1}}}  \subseteq  \delta_{{\mathrm{2}}}$.
    \item If\/ $ [    \binder{  \delta _{ 0 }  }  \mathbin{:\succeq}    \delta' _{ 0 }  ,\dotsc,\binder{  \delta _{ \refenvnt{k} }  }  \mathbin{:\succeq}   \delta'  _{ \refenvnt{k} }   ]  \, \in \, \Psi$
          and $\gamma_{{\mathrm{2}}}  \refenvsym{=}   \delta _{ \refenvnt{i} } $ for some $\refenvnt{i}$ with $0 \le \refenvnt{i} < \refenvnt{k}$,
          then $\Psi  \vdash  \gamma_{{\mathrm{1}}}  \subseteq   \delta' _{ \refenvnt{i} } $ or $\Psi  \vdash  \gamma_{{\mathrm{1}}}  \subseteq   \delta _{ \refenvnt{i}  \refenvsym{+}  1 } $.
    \item If\/ $ [    \binder{  \delta _{ 0 }  }  \mathbin{:\succeq}    \delta' _{ 0 }  ,\dotsc,\binder{  \delta _{ \refenvnt{k} }  }  \mathbin{:\succeq}   \delta'  _{ \refenvnt{k} }   ]  \, \in \, \Psi$
          and $\gamma_{{\mathrm{2}}}  \refenvsym{=}   \delta _{ \refenvnt{k} } $,
          then $\Psi  \vdash  \gamma_{{\mathrm{1}}}  \subseteq   \delta' _{ \refenvnt{k} } $.
  \end{enumerate}
\end{lemma}

\begin{proof}
  By induction on the given derivation.
\end{proof}

\begin{lemma}[Inversion for $ \subseteq $ w.r.t. Context]
  \label{claim:inversion-runtime-gtrans-ctx}
  If\/ $ \Psi \mid^{ \delta_{{\mathrm{1}}} } \Gamma \vdash \gamma_{{\mathrm{1}}} \subseteq \gamma_{{\mathrm{2}}} $, $\gamma_{{\mathrm{1}}} \neq \gamma_{{\mathrm{2}}}$ and $\gamma_{{\mathrm{2}}} \, \in \,  \token{Dom}_{C}( \Gamma ) $, then the following hold:
  \begin{enumerate}
    \item If\/ $\Gamma = \Gamma_{{\mathrm{1}}}  \refenvsym{,}   \binder{ \refenvmv{x} }\mathord{:^{\binder{ \gamma_{{\mathrm{2}}} } } } \refenvnt{A}   \refenvsym{,}  \Gamma_{{\mathrm{2}}}$
          and $ \Psi \mid^{ \delta_{{\mathrm{1}}} } \Gamma_{{\mathrm{1}}} \vdash^{  \dotsc   \refenvsym{,}  \delta_{{\mathrm{2}}} }\token{wf} $,
          then $ \Psi \mid^{ \delta_{{\mathrm{1}}} } \Gamma \vdash \gamma_{{\mathrm{1}}} \subseteq \delta_{{\mathrm{2}}} $.
    \item If\/ $\Gamma = \Gamma_{{\mathrm{1}}}  \refenvsym{,}   \blacktriangleleft _{ \refenvnt{k_{{\mathrm{1}}}} }^{\binder{ \gamma_{{\mathrm{2}}} } }   \refenvsym{,}  \Gamma_{{\mathrm{2}}}$
          and $ \Psi \mid^{ \delta_{{\mathrm{1}}} } \Gamma_{{\mathrm{1}}} \vdash^{   \delta' _{ 1 }  ,\dotsc,  \delta' _{ \refenvnt{k_{{\mathrm{2}}}} }   }\token{wf} $,
          then $ \Psi \mid^{ \delta_{{\mathrm{1}}} } \Gamma \vdash \gamma_{{\mathrm{1}}} \subseteq  \delta' _{ \refenvnt{k_{{\mathrm{2}}}} }  $
          or $ \Psi \mid^{ \delta_{{\mathrm{1}}} } \Gamma \vdash \gamma_{{\mathrm{1}}} \subseteq  \delta' _{ \refenvnt{k_{{\mathrm{2}}}}  \refenvsym{-}  \refenvnt{k_{{\mathrm{1}}}} }  $.
    \item If\/ $\Gamma = \Gamma_{{\mathrm{1}}}  \refenvsym{,}   [    \binder{  \gamma' _{ 1 }  }  \mathbin{:\succeq}    \gamma'' _{ 1 }  ,\dotsc,\binder{  \gamma' _{ \refenvnt{k} }  }  \mathbin{:\succeq}   \gamma''  _{ \refenvnt{k} }   ]^{\binder{ \gamma_{{\mathrm{2}}} } }   \refenvsym{,}  \Gamma_{{\mathrm{2}}}$
          and $ \Psi \mid^{ \delta_{{\mathrm{1}}} } \Gamma_{{\mathrm{1}}} \vdash^{  \dotsc   \refenvsym{,}  \delta_{{\mathrm{2}}} }\token{wf} $,
          then $ \Psi \mid^{ \delta_{{\mathrm{1}}} } \Gamma \vdash \gamma_{{\mathrm{1}}} \subseteq \delta_{{\mathrm{2}}} $.
    \item If\/ $\Gamma = \Gamma_{{\mathrm{1}}}  \refenvsym{,}   [    \binder{  \gamma' _{ 1 }  }  \mathbin{:\succeq}    \gamma'' _{ 1 }  ,\dotsc,\binder{  \gamma' _{ \refenvnt{k} }  }  \mathbin{:\succeq}   \gamma''  _{ \refenvnt{k} }   ]^{\binder{  \gamma' _{ 0 }  } }   \refenvsym{,}  \Gamma_{{\mathrm{2}}}$
          and $ \gamma' _{ \refenvnt{i} }  = \gamma_{{\mathrm{2}}}$ for some $\refenvnt{i}$ with $1 \le \refenvnt{i} < \refenvnt{k}$,
          then $ \Psi \mid^{ \delta_{{\mathrm{1}}} } \Gamma \vdash \gamma_{{\mathrm{1}}} \subseteq  \gamma'' _{ \refenvnt{i} }  $ or $ \Psi \mid^{ \delta_{{\mathrm{1}}} } \Gamma \vdash \gamma_{{\mathrm{1}}} \subseteq  \gamma' _{ \refenvnt{i}  \refenvsym{+}  1 }  $.
    \item If\/ $\Gamma = \Gamma_{{\mathrm{1}}}  \refenvsym{,}   [    \binder{  \gamma' _{ 1 }  }  \mathbin{:\succeq}    \gamma'' _{ 1 }  ,\dotsc,\binder{  \gamma' _{ \refenvnt{k} }  }  \mathbin{:\succeq}   \gamma''  _{ \refenvnt{k} }   ]^{\binder{  \gamma' _{ 0 }  } }   \refenvsym{,}  \Gamma_{{\mathrm{2}}}$
          and $ \gamma' _{ \refenvnt{i} }  = \gamma_{{\mathrm{2}}}$ for some $\refenvnt{i}$ with $1 \le \refenvnt{i} \le \refenvnt{k}$,
          then $ \Psi \mid^{ \delta_{{\mathrm{1}}} } \Gamma \vdash \gamma_{{\mathrm{1}}} \subseteq  \gamma'' _{ \refenvnt{i} }  $.
  \end{enumerate}
\end{lemma}

\begin{proof}
  By induction on the given derivation.
\end{proof}

\subsection{Structural Properties}

\begin{lemma}[Weakening with regard to Reserved Names Typing]
  \label{claim:nht-weakening}
  Suppose $ \Psi_{{\mathrm{1}}} \subseteq \Psi_{{\mathrm{2}}} $ and $ \vdash  \Psi_{{\mathrm{2}}} \ \token{wf} $.  Then the following hold:
  \begin{enumerate}
    \item If\/ $\Psi_{{\mathrm{1}}}  \vdash   \overrightarrow{ \gamma }^{+}  \, \token{wf}$ and\/ $ \vdash  \Psi_{{\mathrm{2}}} \ \token{wf} $,
          then $\Psi_{{\mathrm{2}}}  \vdash   \overrightarrow{ \gamma }^{+}  \, \token{wf}$.
    % \item If\/ $ \Psi_{{\mathrm{1}}} \mid^{  \overrightarrow{ \gamma_{{\mathrm{1}}} }^{+}  } \Gamma \vdash^{  \overrightarrow{ \gamma_{{\mathrm{2}}} }^{+}  }\token{wf} $,
    %       then $ \Psi_{{\mathrm{2}}} \mid^{  \overrightarrow{ \gamma_{{\mathrm{1}}} }^{+}  } \Gamma \vdash^{  \overrightarrow{ \gamma_{{\mathrm{2}}} }^{+}  }\token{wf} $.
    \item If\/ $ \Psi_{{\mathrm{1}}} \mid^{  \overrightarrow{ \gamma_{{\mathrm{1}}} }^{+}  }  \Gamma \vdash ^{  \overrightarrow{ \gamma_{{\mathrm{2}}} }^{+}  } \refenvnt{A} \ \token{wf} $ and\/ $ \Psi_{{\mathrm{2}}} \mid^{  \overrightarrow{ \gamma_{{\mathrm{1}}} }^{+}  } \Gamma \vdash^{  \overrightarrow{ \gamma_{{\mathrm{2}}} }^{+}  }\token{wf} $,
          then $ \Psi_{{\mathrm{2}}} \mid^{  \overrightarrow{ \gamma_{{\mathrm{1}}} }^{+}  }  \Gamma \vdash ^{  \overrightarrow{ \gamma_{{\mathrm{2}}} }^{+}  } \refenvnt{A} \ \token{wf} $.
    \item If\/ $ \Psi_{{\mathrm{1}}} \mid^{  \overrightarrow{ \gamma_{{\mathrm{1}}} }^{+}  } \Gamma \vdash \gamma_{{\mathrm{2}}} \preceq \gamma_{{\mathrm{3}}} $ and\/ $ \Psi_{{\mathrm{2}}} \mid^{  \overrightarrow{ \gamma_{{\mathrm{1}}} }^{+}  } \Gamma \vdash^{  \overrightarrow{ \gamma_{{\mathrm{2}}} }^{+}  }\token{wf} $,
          then $ \Psi_{{\mathrm{2}}} \mid^{  \overrightarrow{ \gamma_{{\mathrm{1}}} }^{+}  } \Gamma \vdash \gamma_{{\mathrm{2}}} \preceq \gamma_{{\mathrm{3}}} $.
    \item If\/ $ \Psi_{{\mathrm{1}}} \mid^{  \overrightarrow{ \gamma_{{\mathrm{1}}} }^{+}  } \Gamma \vdash \gamma_{{\mathrm{2}}} \subseteq \gamma_{{\mathrm{3}}} $ and\/ $ \Psi_{{\mathrm{2}}} \mid^{  \overrightarrow{ \gamma_{{\mathrm{1}}} }^{+}  } \Gamma \vdash^{  \overrightarrow{ \gamma_{{\mathrm{2}}} }^{+}  }\token{wf} $,
          then $ \Psi_{{\mathrm{2}}} \mid^{  \overrightarrow{ \gamma_{{\mathrm{1}}} }^{+}  } \Gamma \vdash \gamma_{{\mathrm{2}}} \subseteq \gamma_{{\mathrm{3}}} $.
    \item If\/ $ \Psi_{{\mathrm{1}}} \mid^{  \overrightarrow{ \gamma_{{\mathrm{1}}} }^{+}  }  \Gamma \vdash^{  \overrightarrow{ \gamma_{{\mathrm{2}}} }^{+}  }_{ R }  \refenvnt{e} : \refenvnt{A} $  and\/ $ \Psi_{{\mathrm{2}}} \mid^{  \overrightarrow{ \gamma_{{\mathrm{1}}} }^{+}  } \Gamma \vdash^{  \overrightarrow{ \gamma_{{\mathrm{2}}} }^{+}  }\token{wf} $,
          then $ \Psi_{{\mathrm{2}}} \mid^{  \overrightarrow{ \gamma_{{\mathrm{1}}} }^{+}  }  \Gamma \vdash^{  \overrightarrow{ \gamma_{{\mathrm{2}}} }^{+}  }_{ R }  \refenvnt{e} : \refenvnt{A} $.
    \item If\/ $ \Psi_{{\mathrm{1}}}  \vdash  \Theta \ \token{wf} $,
          then $ \Psi_{{\mathrm{2}}}  \vdash  \Theta \ \token{wf} $.
    \item If\/ $\Psi_{{\mathrm{1}}}  \vdash  S  \colon  \Theta$,
          then $\Psi_{{\mathrm{2}}}  \vdash  S  \colon  \Theta$.
    \item If\/ $ \Psi_{{\mathrm{1}}} \mid \Theta \vdash^{ \gamma } \refenvnt{v} : \refenvnt{A} \ \token{val} $,
          then $ \Psi_{{\mathrm{2}}} \mid \Theta \vdash^{ \gamma } \refenvnt{v} : \refenvnt{A} \ \token{val} $.
    \item If\/ $ \Psi_{{\mathrm{1}}} \mid \Theta \vdash^{ \gamma } E \ \token{wf} $,
          then $ \Psi_{{\mathrm{2}}} \mid \Theta \vdash^{ \gamma } E \ \token{wf} $.
  \end{enumerate}
\end{lemma}

\begin{proof}
  By mutual induction on the given derivation.
\end{proof}

\begin{lemma}[Weakening with regard to Store Typing]
  \label{claim:store-typing-weakening}
  Suppose $ \Psi  \vdash  \Theta_{{\mathrm{2}}} \ \token{wf} $ and $ \Theta_{{\mathrm{1}}} \subseteq \Theta_{{\mathrm{2}}} $.
  Then the following hold:
  \begin{enumerate}
    \item If\/ $ \Psi \mid \Theta_{{\mathrm{1}}} \vdash^{ \gamma } \refenvnt{v} : \refenvnt{A} \ \token{val} $,
          then $ \Psi \mid \Theta_{{\mathrm{2}}} \vdash^{ \gamma } \refenvnt{v} : \refenvnt{A} \ \token{val} $.
    \item If\/ $ \Psi \mid \Theta_{{\mathrm{1}}} \vdash^{ \gamma } E \ \token{wf} $,
          then $ \Psi \mid \Theta_{{\mathrm{2}}} \vdash^{ \gamma } E \ \token{wf} $.
  \end{enumerate}
\end{lemma}

\begin{proof}
  By mutual induction on the given derivation.
\end{proof}

\begin{lemma}[Monotonicity with regard to Reserved Names Typing]
  \label{claim:nht-monotonicity}
  Suppose $\Psi  \vdash   \overrightarrow{ \delta_{{\mathrm{1}}} }^{+}   \refenvsym{,}  \delta_{{\mathrm{2}}} \, \token{wf}$ and $\Psi  \vdash  \gamma_{{\mathrm{0}}}  \preceq  \delta_{{\mathrm{2}}}$.
  If\/ $ \Psi \mid^{ \gamma_{{\mathrm{0}}} } \Gamma \vdash^{  \overrightarrow{ \gamma_{{\mathrm{1}}} }^{+}  }\token{wf} $, then there exists
  $ \overrightarrow{ \delta_{{\mathrm{3}}} }^{+} $ such that
  $ \Psi \mid^{  \overrightarrow{ \delta_{{\mathrm{1}}} }^{+}   \refenvsym{,}  \delta_{{\mathrm{2}}} } \Gamma \vdash^{  \overrightarrow{ \delta_{{\mathrm{3}}} }^{+}  }\token{wf} $.
  For such $ \overrightarrow{ \delta_{{\mathrm{3}}} }^{+} $, the following hold:
  \begin{enumerate}
    \item If\/ $ \Psi \mid^{ \gamma_{{\mathrm{0}}} }  \Gamma \vdash ^{  \overrightarrow{ \gamma_{{\mathrm{1}}} }^{+}  } \refenvnt{A} \ \token{wf} $,
          then $ \Psi \mid^{  \overrightarrow{ \delta_{{\mathrm{1}}} }^{+}   \refenvsym{,}  \delta_{{\mathrm{2}}} }  \Gamma \vdash ^{  \overrightarrow{ \delta_{{\mathrm{3}}} }^{+}  } \refenvnt{A} \ \token{wf} $.
    \item If\/ $ \Psi \mid^{ \gamma_{{\mathrm{0}}} } \Gamma \vdash \gamma_{{\mathrm{1}}} \preceq \gamma_{{\mathrm{2}}} $,
          then $ \Psi \mid^{  \overrightarrow{ \delta_{{\mathrm{1}}} }^{+}   \refenvsym{,}  \delta_{{\mathrm{2}}} } \Gamma \vdash \gamma_{{\mathrm{1}}} \preceq \gamma_{{\mathrm{2}}} $.
    \item If\/ $ \Psi \mid^{ \gamma_{{\mathrm{0}}} } \Gamma \vdash \gamma_{{\mathrm{1}}} \subseteq \gamma_{{\mathrm{2}}} $,
          then $ \Psi \mid^{  \overrightarrow{ \delta_{{\mathrm{1}}} }^{+}   \refenvsym{,}  \delta_{{\mathrm{2}}} } \Gamma \vdash \gamma_{{\mathrm{1}}} \subseteq \gamma_{{\mathrm{2}}} $.
    \item If\/ $ \Psi \mid^{ \gamma_{{\mathrm{0}}} }  \Gamma \vdash^{  \overrightarrow{ \gamma_{{\mathrm{1}}} }^{+}  }_{ R }  \refenvnt{e} : \refenvnt{A} $,
          then $ \Psi \mid^{  \overrightarrow{ \delta_{{\mathrm{1}}} }^{+}   \refenvsym{,}  \delta_{{\mathrm{2}}} }  \Gamma \vdash^{  \overrightarrow{ \delta_{{\mathrm{3}}} }^{+}  }_{ R }  \refenvnt{e} : \refenvnt{A} $.
  \end{enumerate}
\end{lemma}

\begin{proof}
  By mutual induction on the given derivation.
\end{proof}

\begin{lemma}[Weakening with regard to Context]\label{claim:ctx-weakening}
  \begin{enumerate}
    \item If\/ $ \Psi \mid^{  \overrightarrow{ \gamma_{{\mathrm{1}}} }^{+}  } \Gamma_{{\mathrm{1}}} \vdash \delta_{{\mathrm{1}}} \preceq \delta_{{\mathrm{2}}} $
          and $ \Psi \mid^{  \overrightarrow{ \gamma_{{\mathrm{1}}} }^{+}  } \Gamma_{{\mathrm{1}}}  \refenvsym{,}  \Gamma_{{\mathrm{2}}} \vdash^{  \dotsc  }\token{wf} $,
          then $ \Psi \mid^{  \overrightarrow{ \gamma_{{\mathrm{1}}} }^{+}  } \Gamma_{{\mathrm{1}}}  \refenvsym{,}  \Gamma_{{\mathrm{2}}} \vdash \delta_{{\mathrm{1}}} \preceq \delta_{{\mathrm{2}}} $.
    \item If\/ $ \Psi \mid^{  \overrightarrow{ \gamma_{{\mathrm{1}}} }^{+}  } \Gamma_{{\mathrm{1}}} \vdash \delta_{{\mathrm{1}}} \subseteq \delta_{{\mathrm{2}}} $
          and $ \Psi \mid^{  \overrightarrow{ \gamma_{{\mathrm{1}}} }^{+}  } \Gamma_{{\mathrm{1}}}  \refenvsym{,}  \Gamma_{{\mathrm{2}}} \vdash^{  \dotsc  }\token{wf} $,
          then $ \Psi \mid^{  \overrightarrow{ \gamma_{{\mathrm{1}}} }^{+}  } \Gamma_{{\mathrm{1}}}  \refenvsym{,}  \Gamma_{{\mathrm{2}}} \vdash \delta_{{\mathrm{1}}} \subseteq \delta_{{\mathrm{2}}} $.
  \end{enumerate}
\end{lemma}

\begin{proof}
  By mutual induction on the given derivation.
\end{proof}

\begin{lemma}[Strengthening with regard to Context]\label{claim:ctx-strengthening}
  \begin{enumerate}
    \item If\/ $ \Psi \mid^{  \overrightarrow{ \gamma_{{\mathrm{1}}} }^{+}  } \Gamma_{{\mathrm{1}}}  \refenvsym{,}  \Gamma_{{\mathrm{2}}} \vdash \delta_{{\mathrm{1}}} \preceq \delta_{{\mathrm{2}}} $
          and $\delta_{{\mathrm{2}}} \, \not\in \,  \token{Dom}_{C}( \Gamma_{{\mathrm{2}}} ) $,
          then $ \Psi \mid^{  \overrightarrow{ \gamma_{{\mathrm{1}}} }^{+}  } \Gamma_{{\mathrm{1}}} \vdash \delta_{{\mathrm{1}}} \preceq \delta_{{\mathrm{2}}} $.
    \item If\/ $ \Psi \mid^{  \overrightarrow{ \gamma_{{\mathrm{1}}} }^{+}  } \Gamma_{{\mathrm{1}}}  \refenvsym{,}  \Gamma_{{\mathrm{2}}} \vdash \delta_{{\mathrm{1}}} \subseteq \delta_{{\mathrm{2}}} $
          and $\delta_{{\mathrm{2}}} \, \not\in \,  \token{Dom}_{C}( \Gamma_{{\mathrm{2}}} ) $,
          then $ \Psi \mid^{  \overrightarrow{ \gamma_{{\mathrm{1}}} }^{+}  } \Gamma_{{\mathrm{1}}} \vdash \delta_{{\mathrm{1}}} \subseteq \delta_{{\mathrm{2}}} $.
  \end{enumerate}
\end{lemma}

\begin{proof}
  By mutual induction on the given derivation.
\end{proof}

\begin{lemma}[Classifier Substitution Lemma for Polymorphic Classifier Declarations]
  \label{claim:polyclsdecl-substitution}
  Let $\Gamma_{{\mathrm{0}}} =  [    \binder{  \gamma _{ 1 }  }  \mathbin{:\succeq}    \gamma' _{ 1 }  ,\dotsc,\binder{  \gamma _{ \refenvnt{k} }  }  \mathbin{:\succeq}   \gamma'  _{ \refenvnt{k} }   ]^{\binder{  \gamma _{ 0 }  } } $ and
  $\sigma =   \gamma _{ 0 }  \coloneqq  \delta' _{ 0 }  ,\dotsc,  \gamma _{ \refenvnt{k} }  \coloneqq  \delta' _{ \refenvnt{k} }  $.
  Suppose
  $ \Psi \mid^{  \overrightarrow{ \delta_{{\mathrm{1}}} }^{+}  } \Gamma_{{\mathrm{1}}} \vdash^{  \overrightarrow{ \delta_{{\mathrm{3}}} }   \refenvsym{,}   \delta' _{ 0 }  }\token{wf} $,
  $ \Psi \mid^{  \overrightarrow{ \delta_{{\mathrm{1}}} }^{+}  } \Gamma_{{\mathrm{1}}} \vdash  \gamma' _{ \refenvnt{i} }  \preceq  \delta' _{ \refenvnt{i} }  $ for $1 \le \refenvnt{i} \le \refenvnt{k}$,
  and
  $ \Psi \mid^{  \overrightarrow{ \delta_{{\mathrm{1}}} }^{+}  } \Gamma_{{\mathrm{1}}} \vdash  \delta' _{ \refenvnt{i}  \refenvsym{+}  1 }  \subseteq  \delta' _{ \refenvnt{i} }  $ for $0 \le \refenvnt{i} < \refenvnt{k}$.
  Then the following hold:
  \begin{enumerate}
    \item If\/ $ \Psi \mid^{  \overrightarrow{ \delta_{{\mathrm{1}}} }^{+}  } \Gamma_{{\mathrm{1}}}  \refenvsym{,}  \Gamma_{{\mathrm{0}}}  \refenvsym{,}  \Gamma_{{\mathrm{2}}} \vdash^{  \overrightarrow{ \delta_{{\mathrm{2}}} }^{+}  }\token{wf} $,
          then
          $ \Psi \mid^{  \overrightarrow{ \delta_{{\mathrm{1}}} }^{+}  } \Gamma_{{\mathrm{1}}}  \refenvsym{,}  \Gamma_{{\mathrm{2}}}  \refenvsym{[}  \sigma  \refenvsym{]} \vdash^{   \overrightarrow{ \delta_{{\mathrm{2}}} }^{+}    \refenvsym{[}  \sigma  \refenvsym{]} }\token{wf} $.
    \item If\/ $ \Psi \mid^{  \overrightarrow{ \delta_{{\mathrm{1}}} }^{+}  }  \Gamma_{{\mathrm{1}}}  \refenvsym{,}  \Gamma_{{\mathrm{0}}}  \refenvsym{,}  \Gamma_{{\mathrm{2}}} \vdash ^{  \overrightarrow{ \delta_{{\mathrm{2}}} }^{+}  } \refenvnt{A} \ \token{wf} $,
          then
          $ \Psi \mid^{  \overrightarrow{ \delta_{{\mathrm{1}}} }^{+}  }  \Gamma_{{\mathrm{1}}}  \refenvsym{,}  \Gamma_{{\mathrm{2}}}  \refenvsym{[}  \sigma  \refenvsym{]} \vdash ^{   \overrightarrow{ \delta_{{\mathrm{2}}} }^{+}    \refenvsym{[}  \sigma  \refenvsym{]} } \refenvnt{A}  \refenvsym{[}  \sigma  \refenvsym{]} \ \token{wf} $.
    \item If\/ $ \Psi \mid^{  \overrightarrow{ \delta_{{\mathrm{1}}} }^{+}  } \Gamma_{{\mathrm{1}}}  \refenvsym{,}  \Gamma_{{\mathrm{0}}}  \refenvsym{,}  \Gamma_{{\mathrm{2}}} \vdash \delta''_{{\mathrm{1}}} \preceq \delta''_{{\mathrm{2}}} $,
          then
          $ \Psi \mid^{  \overrightarrow{ \delta_{{\mathrm{1}}} }^{+}  } \Gamma_{{\mathrm{1}}}  \refenvsym{,}  \Gamma_{{\mathrm{2}}}  \refenvsym{[}  \sigma  \refenvsym{]} \vdash \delta''_{{\mathrm{1}}}  \refenvsym{[}  \sigma  \refenvsym{]} \preceq \delta''_{{\mathrm{2}}}  \refenvsym{[}  \sigma  \refenvsym{]} $.
    \item If\/ $ \Psi \mid^{  \overrightarrow{ \delta_{{\mathrm{1}}} }^{+}  } \Gamma_{{\mathrm{1}}}  \refenvsym{,}  \Gamma_{{\mathrm{0}}}  \refenvsym{,}  \Gamma_{{\mathrm{2}}} \vdash \delta''_{{\mathrm{1}}} \subseteq \delta''_{{\mathrm{2}}} $,
          then
          $ \Psi \mid^{  \overrightarrow{ \delta_{{\mathrm{1}}} }^{+}  } \Gamma_{{\mathrm{1}}}  \refenvsym{,}  \Gamma_{{\mathrm{2}}}  \refenvsym{[}  \sigma  \refenvsym{]} \vdash \delta''_{{\mathrm{1}}}  \refenvsym{[}  \sigma  \refenvsym{]} \subseteq \delta''_{{\mathrm{2}}}  \refenvsym{[}  \sigma  \refenvsym{]} $.
    \item If\/ $ \Psi \mid^{  \overrightarrow{ \delta_{{\mathrm{1}}} }^{+}  }  \Gamma_{{\mathrm{1}}}  \refenvsym{,}  \Gamma_{{\mathrm{0}}}  \refenvsym{,}  \Gamma_{{\mathrm{2}}} \vdash^{  \overrightarrow{ \delta_{{\mathrm{2}}} }^{+}  }_{ R }  \refenvnt{e} : \refenvnt{A} $,
          then
          $ \Psi \mid^{  \overrightarrow{ \delta_{{\mathrm{1}}} }^{+}  }  \Gamma_{{\mathrm{1}}}  \refenvsym{,}  \Gamma_{{\mathrm{2}}}  \refenvsym{[}  \sigma  \refenvsym{]} \vdash^{   \overrightarrow{ \delta_{{\mathrm{2}}} }^{+}    \refenvsym{[}  \sigma  \refenvsym{]} }_{ R }  \refenvnt{e} : \refenvnt{A}  \refenvsym{[}  \sigma  \refenvsym{]} $.
  \end{enumerate}
\end{lemma}

\begin{proof}
  By mutual induction on the given derivation.
\end{proof}

\begin{lemma}\label{claim:unlift-quote-body}
  If\/ $ \Psi \mid^{ \gamma_{{\mathrm{1}}} }   \blacktriangleright ^{ \gamma_{{\mathrm{2}}} }  \vdash^{ \gamma_{{\mathrm{1}}}  \refenvsym{,}  \gamma_{{\mathrm{2}}} }_{  \token{id}  }   \refenvnt{e} ^{ 0  }  : \refenvnt{A} $,
  then $ \Psi \mid^{ \gamma_{{\mathrm{2}}} }  \varepsilon \vdash^{ \gamma_{{\mathrm{2}}} }_{  \token{id}  }   \refenvnt{e} ^{ 0  }  : \refenvnt{A} $.
\end{lemma}

\begin{proof}
  By induction on the given derivation.
\end{proof}

\subsection{Normal Form of Expression Typing Derivations}
\begin{definition}
  We define an additional rule \ref{rule:runtime-type-appcls-nonintro} for expression typing.

  \begin{mathpar}
  \myinferrule[R-T-Appcls-NonIntro]
  { \Psi \mid^{  \overrightarrow{ \delta'_{{\mathrm{1}}} }^{+}  }  \Gamma \vdash^{  \overrightarrow{ \delta'_{{\mathrm{2}}} }   \refenvsym{,}   \delta _{ 0 }  }_{ R }  \refenvnt{e} :  \forall    \binder{  \gamma _{ 1 }  }  \mathbin{:\succeq}    \gamma' _{ 1 }  ,\dotsc,\binder{  \gamma _{ \refenvnt{k} }  }  \mathbin{:\succeq}   \gamma'  _{ \refenvnt{k} }  . \refenvnt{A}   \\
   \Psi \mid^{  \overrightarrow{ \delta'_{{\mathrm{1}}} }^{+}  } \Gamma \vdash  \gamma' _{ \refenvnt{i} }  \preceq  \delta _{ \refenvnt{i} }   \text{\ for\ }  1 \le \refenvnt{i} \le \refenvnt{k} \\
   \Psi \mid^{  \overrightarrow{ \delta'_{{\mathrm{1}}} }^{+}  } \Gamma \vdash  \delta _{ \refenvnt{i}  \refenvsym{+}  1 }  \subseteq  \delta _{ \refenvnt{i} }   \text{\ for\ }  0 \le \refenvnt{i} < \refenvnt{k} \\
  \text{$\refenvnt{e}$ is not an introduction form} }
  { \Psi \mid^{  \overrightarrow{ \delta'_{{\mathrm{1}}} }^{+}  }  \Gamma \vdash^{  \overrightarrow{ \delta'_{{\mathrm{2}}} }   \refenvsym{,}   \delta _{ 0 }  }_{ R }  \refenvnt{e} : \refenvnt{A}  \refenvsym{[}    \gamma _{ 1 }  \coloneqq  \delta _{ 1 }  ,\dotsc,  \gamma _{ \refenvnt{k} }  \coloneqq  \delta _{ \refenvnt{k} }    \refenvsym{]} }
  \label{rule:runtime-type-appcls-nonintro}
  \end{mathpar}

  If an expression typing derivation contains no use of \ref{rule:runtime-type-appcls},
  then we say it is in \emph{normal form}.
\end{definition}

\begin{lemma}[Classifier Substitution Lemma for Polymorphic Classifier Declarations]
  \label{claim:polyclsdecl-substitution-exp-normal}
  Let $\Gamma_{{\mathrm{0}}} =  [    \binder{  \gamma _{ 1 }  }  \mathbin{:\succeq}    \gamma' _{ 1 }  ,\dotsc,\binder{  \gamma _{ \refenvnt{k} }  }  \mathbin{:\succeq}   \gamma'  _{ \refenvnt{k} }   ]^{\binder{  \gamma _{ 0 }  } } $ and
  $\sigma =   \gamma _{ 0 }  \coloneqq  \delta' _{ 0 }  ,\dotsc,  \gamma _{ \refenvnt{k} }  \coloneqq  \delta' _{ \refenvnt{k} }  $.
  Suppose
  $ \Psi \mid^{  \overrightarrow{ \delta_{{\mathrm{1}}} }^{+}  } \Gamma_{{\mathrm{1}}} \vdash^{  \overrightarrow{ \delta_{{\mathrm{3}}} }   \refenvsym{,}   \delta' _{ 0 }  }\token{wf} $,
  $ \Psi \mid^{  \overrightarrow{ \delta_{{\mathrm{1}}} }^{+}  } \Gamma_{{\mathrm{1}}} \vdash  \gamma' _{ \refenvnt{i} }  \preceq  \delta' _{ \refenvnt{i} }  $ for $1 \le \refenvnt{i} \le \refenvnt{k}$,
  and
  $ \Psi \mid^{  \overrightarrow{ \delta_{{\mathrm{1}}} }^{+}  } \Gamma_{{\mathrm{1}}} \vdash  \delta' _{ \refenvnt{i}  \refenvsym{+}  1 }  \subseteq  \delta' _{ \refenvnt{i} }  $ for $0 \le \refenvnt{i} < \refenvnt{k}$.
  If\/ there is a normal derivation for
  $ \Psi \mid^{  \overrightarrow{ \delta_{{\mathrm{1}}} }^{+}  }  \Gamma_{{\mathrm{1}}}  \refenvsym{,}  \Gamma_{{\mathrm{0}}}  \refenvsym{,}  \Gamma_{{\mathrm{2}}} \vdash^{  \overrightarrow{ \delta_{{\mathrm{2}}} }^{+}  }_{ R }  \refenvnt{e} : \refenvnt{A} $,
  then there is also a normal derivation for
  $ \Psi \mid^{  \overrightarrow{ \delta_{{\mathrm{1}}} }^{+}  }  \Gamma_{{\mathrm{1}}}  \refenvsym{,}  \Gamma_{{\mathrm{2}}}  \refenvsym{[}  \sigma  \refenvsym{]} \vdash^{   \overrightarrow{ \delta_{{\mathrm{2}}} }^{+}    \refenvsym{[}  \sigma  \refenvsym{]} }_{ R }  \refenvnt{e} : \refenvnt{A}  \refenvsym{[}  \sigma  \refenvsym{]} $.
\end{lemma}

\begin{proof}
  By induction on the given derivation, as done in \zcref{claim:polyclsdecl-substitution}.
\end{proof}

\begin{lemma}[Normal Form of Expression Typing Derivations]\label{claim:runtime-typing-normal-form}
  If an expression typing judgment is derivable, then it is derivable with a normal form derivation.
  Namely, \ref{rule:runtime-type-appcls} can be safely restricted to \ref{rule:runtime-type-appcls-nonintro}.
\end{lemma}

\begin{proof}
  By induction on the given derivation. The only non-trivial case is when the last rule is \ref{rule:runtime-type-appcls} and the expression is an introduction form. By the induction hypothesis, the derivation of the first premise of \ref{rule:runtime-type-appcls} can be taken to be in normal form. Since the expression is an introduction form, this normal-form derivation must end with \ref{rule:runtime-type-polycls}. We can therefore apply \zcref{claim:polyclsdecl-substitution-exp-normal} to obtain a normal-form derivation of the same typing judgment.
\end{proof}

\begin{convention}
  In the rest of this note, we assume that all expression typing derivations
  are in normal form. Accordingly, we use
  \ref{rule:runtime-type-appcls} to refer to
  \ref{rule:runtime-type-appcls-nonintro}, unless stated otherwise.
\end{convention}

\subsection{Upper Bound of Classifiers}
\begin{lemma}
  $ \token{Ctx}^{ \refenvnt{k_{{\mathrm{1}}}} , \refenvnt{k_{{\mathrm{2}}}} }  \subseteq  \token{Ctx}^{ \refenvnt{k_{{\mathrm{1}}}}  \refenvsym{+}  \refenvnt{k_{{\mathrm{3}}}} , \refenvnt{k_{{\mathrm{2}}}}  \refenvsym{+}  \refenvnt{k_{{\mathrm{3}}}} } $ for any $\refenvnt{k_{{\mathrm{3}}}} > 0$.
\end{lemma}

\begin{proof}
  By induction on the structure of contexts.
\end{proof}

\begin{lemma}
  $  \Gamma_{{\mathrm{1}}} ^{ \refenvnt{k_{{\mathrm{1}}}} , \refenvnt{k_{{\mathrm{2}}}} }   \refenvsym{,}  \Gamma_{{\mathrm{2}}} ^{ \refenvnt{k_{{\mathrm{2}}}} , \refenvnt{k_{{\mathrm{3}}}} }  \, \in \,  \token{Ctx}^{ \refenvnt{k_{{\mathrm{1}}}} , \refenvnt{k_{{\mathrm{3}}}} } $.
\end{lemma}

\begin{proof}
  By induction on the structure of $ \Gamma_{{\mathrm{1}}} ^{ \refenvnt{k_{{\mathrm{1}}}} , \refenvnt{k_{{\mathrm{2}}}} } $.
\end{proof}

\begin{lemma}[Origins of Output Classifiers]
  \label{claim:ctx-output-classifier-origin}
  If
  \begin{itemize}
    \item $ \Psi \mid^{  \overrightarrow{ \gamma_{{\mathrm{1}}} }^{+}  } \Gamma_{{\mathrm{1}}} \vdash^{  \overrightarrow{ \gamma_{{\mathrm{2}}} }   \refenvsym{,}    \delta _{ 0 }  ,\dotsc,  \delta _{ \refenvnt{k_{{\mathrm{1}}}} }   }\token{wf} $,
    \item $ \Psi \mid^{  \overrightarrow{ \gamma_{{\mathrm{1}}} }^{+}  }  \Gamma_{{\mathrm{1}}}  \refenvsym{,}  \Gamma_{{\mathrm{2}}} ^{ \refenvnt{k_{{\mathrm{1}}}} , \refenvnt{k_{{\mathrm{2}}}} }  \vdash^{  \overrightarrow{ \gamma_{{\mathrm{2}}} }   \refenvsym{,}   \overrightarrow{ \gamma_{{\mathrm{3}}} }^{+}  }\token{wf} $, and
    \item $\gamma_{{\mathrm{4}}} \, \in \, \refenvsym{\{}   \overrightarrow{ \gamma_{{\mathrm{3}}} }^{+}   \refenvsym{\}}$,
  \end{itemize}
  then $\gamma_{{\mathrm{4}}} \, \in \, \refenvsym{\{}    \delta _{ 0 }  ,\dotsc,  \delta _{ \refenvnt{k_{{\mathrm{1}}}} }    \refenvsym{\}} \, \cup \,  \token{Dom}_{C}(  \Gamma_{{\mathrm{2}}} ^{ \refenvnt{k_{{\mathrm{1}}}} , \refenvnt{k_{{\mathrm{2}}}} }  )  \, \cup \,  \token{FC}(  \Gamma_{{\mathrm{2}}} ^{ \refenvnt{k_{{\mathrm{1}}}} , \refenvnt{k_{{\mathrm{2}}}} }  ) $.
\end{lemma}

\begin{proof}
  Straightforward.
\end{proof}

\begin{lemma}\label{claim:cls-upper-bound-aux}
  If
  \begin{itemize}
    \item $ \Psi \mid^{  \overrightarrow{ \gamma_{{\mathrm{1}}} }^{+}  } \Gamma_{{\mathrm{1}}} \vdash^{  \overrightarrow{ \gamma_{{\mathrm{2}}} }   \refenvsym{,}    \delta _{ 0 }  ,\dotsc,  \delta _{ \refenvnt{k_{{\mathrm{1}}}} }   }\token{wf} $,
    \item $ \Psi \mid^{  \overrightarrow{ \gamma_{{\mathrm{1}}} }^{+}  }  \Gamma_{{\mathrm{1}}}  \refenvsym{,}  \Gamma_{{\mathrm{2}}} ^{ \refenvnt{k_{{\mathrm{1}}}} , \refenvnt{k_{{\mathrm{2}}}} }  \vdash \gamma_{{\mathrm{3}}} \subseteq \gamma_{{\mathrm{4}}} $,
    \item $\gamma_{{\mathrm{3}}} \, \in \,  \token{Dom}_{C}( \Psi )  \, \cup \,  \token{Dom}_{C}( \Gamma_{{\mathrm{1}}} ) $, and
    \item $\gamma_{{\mathrm{4}}} \, \in \, \refenvsym{\{}    \delta _{ 0 }  ,\dotsc,  \delta _{ \refenvnt{k_{{\mathrm{1}}}} }    \refenvsym{\}} \, \cup \,  \token{Dom}_{C}(  \Gamma_{{\mathrm{2}}} ^{ \refenvnt{k_{{\mathrm{1}}}} , \refenvnt{k_{{\mathrm{2}}}} }  )  \, \cup \,  \token{FC}(  \Gamma_{{\mathrm{2}}} ^{ \refenvnt{k_{{\mathrm{1}}}} , \refenvnt{k_{{\mathrm{2}}}} }  ) $,
  \end{itemize}
  then there exists $\gamma_{{\mathrm{5}}}$ such that
  \begin{itemize}
    \item $\gamma_{{\mathrm{5}}} \, \in \, \refenvsym{\{}    \delta _{ 0 }  ,\dotsc,  \delta _{ \refenvnt{k_{{\mathrm{1}}}} }    \refenvsym{\}} \, \cup \,  \token{FC}(  \Gamma_{{\mathrm{2}}} ^{ \refenvnt{k_{{\mathrm{1}}}} , \refenvnt{k_{{\mathrm{2}}}} }  ) $,
    \item $ \Psi \mid^{  \overrightarrow{ \gamma_{{\mathrm{1}}} }^{+}  }  \Gamma_{{\mathrm{1}}}  \refenvsym{,}  \Gamma_{{\mathrm{2}}} ^{ \refenvnt{k_{{\mathrm{1}}}} , \refenvnt{k_{{\mathrm{2}}}} }  \vdash \gamma_{{\mathrm{5}}} \subseteq \gamma_{{\mathrm{4}}} $ and
    \item $ \Psi \mid^{  \overrightarrow{ \gamma_{{\mathrm{1}}} }^{+}  }  \Gamma_{{\mathrm{1}}}  \refenvsym{,}  \Gamma_{{\mathrm{2}}} ^{ \refenvnt{k_{{\mathrm{1}}}} , \refenvnt{k_{{\mathrm{2}}}} }  \vdash \gamma_{{\mathrm{3}}} \subseteq \gamma_{{\mathrm{5}}} $
  \end{itemize}
\end{lemma}

\begin{proof}
  By induction with respect to
  $ \token{deg} ( \Psi , \refenvsym{(}   \Gamma_{{\mathrm{1}}}  \refenvsym{,}  \Gamma_{{\mathrm{2}}} ^{ \refenvnt{k_{{\mathrm{1}}}} , \refenvnt{k_{{\mathrm{2}}}} }   \refenvsym{)} , \gamma_{{\mathrm{4}}} ) $.

  If $\gamma_{{\mathrm{4}}} \, \in \, \refenvsym{\{}    \delta _{ 0 }  ,\dotsc,  \delta _{ \refenvnt{k_{{\mathrm{1}}}} }    \refenvsym{\}} \, \cup \,  \token{FC}(  \Gamma_{{\mathrm{2}}} ^{ \refenvnt{k_{{\mathrm{1}}}} , \refenvnt{k_{{\mathrm{2}}}} }  ) $, then take
  $\gamma_{{\mathrm{5}}} = \gamma_{{\mathrm{4}}}$.  The two required visibility judgments follow by
  reflexivity and the given derivation.

  We consider the remaining case where $\gamma_{{\mathrm{4}}} \, \in \,  \token{Dom}_{C}(  \Gamma_{{\mathrm{2}}} ^{ \refenvnt{k_{{\mathrm{1}}}} , \refenvnt{k_{{\mathrm{2}}}} }  ) $.  If
  $\gamma_{{\mathrm{3}}} = \gamma_{{\mathrm{4}}}$, then this contradicts the freshness/disjointness
  guaranteed by context well-formedness, because
  $\gamma_{{\mathrm{3}}} \, \in \,  \token{Dom}_{C}( \Psi )  \, \cup \,  \token{Dom}_{C}( \Gamma_{{\mathrm{1}}} ) $.  Hence, we assume
  $\gamma_{{\mathrm{3}}} \neq \gamma_{{\mathrm{4}}}$ and perform case analysis on how $\gamma_{{\mathrm{4}}}$ is
  introduced in $ \Gamma_{{\mathrm{2}}} ^{ \refenvnt{k_{{\mathrm{1}}}} , \refenvnt{k_{{\mathrm{2}}}} } $.
  \begin{description}
    \item[Case \textmd{$ \Gamma_{{\mathrm{2}}} ^{ \refenvnt{k_{{\mathrm{1}}}} , \refenvnt{k_{{\mathrm{2}}}} }  =
           \Gamma_{{\mathrm{3}}} ^{ \refenvnt{k_{{\mathrm{1}}}} , \refenvnt{k_{{\mathrm{3}}}} }   \refenvsym{,}   \binder{ \refenvmv{x} }\mathord{:^{\binder{ \gamma_{{\mathrm{4}}} } } } \refenvnt{A}   \refenvsym{,}  \Gamma_{{\mathrm{4}}}$}:]
      By regularity, we have
      $ \Psi \mid^{  \overrightarrow{ \gamma_{{\mathrm{1}}} }^{+}  }  \Gamma_{{\mathrm{1}}}  \refenvsym{,}  \Gamma_{{\mathrm{3}}} ^{ \refenvnt{k_{{\mathrm{1}}}} , \refenvnt{k_{{\mathrm{3}}}} }  \vdash^{  \dotsc   \refenvsym{,}  \delta'' }\token{wf} $
      for some $\delta''$.
      By \zcref{claim:inversion-runtime-gtrans-ctx},
      $ \Psi \mid^{  \overrightarrow{ \gamma_{{\mathrm{1}}} }^{+}  }  \Gamma_{{\mathrm{1}}}  \refenvsym{,}  \Gamma_{{\mathrm{2}}} ^{ \refenvnt{k_{{\mathrm{1}}}} , \refenvnt{k_{{\mathrm{2}}}} }  \vdash \gamma_{{\mathrm{3}}} \subseteq \delta'' $.  Moreover, by
      \zcref{claim:ctx-output-classifier-origin},
      $\delta'' \, \in \, \refenvsym{\{}    \delta _{ 0 }  ,\dotsc,  \delta _{ \refenvnt{k_{{\mathrm{1}}}} }    \refenvsym{\}} \, \cup \,  \token{Dom}_{C}(  \Gamma_{{\mathrm{2}}} ^{ \refenvnt{k_{{\mathrm{1}}}} , \refenvnt{k_{{\mathrm{2}}}} }  )  \, \cup \,  \token{FC}(  \Gamma_{{\mathrm{2}}} ^{ \refenvnt{k_{{\mathrm{1}}}} , \refenvnt{k_{{\mathrm{2}}}} }  ) $.  Since
      $ \token{deg} ( \Psi , \refenvsym{(}   \Gamma_{{\mathrm{1}}}  \refenvsym{,}  \Gamma_{{\mathrm{2}}} ^{ \refenvnt{k_{{\mathrm{1}}}} , \refenvnt{k_{{\mathrm{2}}}} }   \refenvsym{)} , \delta'' )  <
       \token{deg} ( \Psi , \refenvsym{(}   \Gamma_{{\mathrm{1}}}  \refenvsym{,}  \Gamma_{{\mathrm{2}}} ^{ \refenvnt{k_{{\mathrm{1}}}} , \refenvnt{k_{{\mathrm{2}}}} }   \refenvsym{)} , \gamma_{{\mathrm{4}}} ) $, the induction hypothesis gives
      some $\gamma_{{\mathrm{5}}}$ such that
      \[
        \gamma_{{\mathrm{5}}} \, \in \, \refenvsym{\{}    \delta _{ 0 }  ,\dotsc,  \delta _{ \refenvnt{k_{{\mathrm{1}}}} }    \refenvsym{\}} \, \cup \,  \token{FC}(  \Gamma_{{\mathrm{2}}} ^{ \refenvnt{k_{{\mathrm{1}}}} , \refenvnt{k_{{\mathrm{2}}}} }  ) ,\qquad
         \Psi \mid^{  \overrightarrow{ \gamma_{{\mathrm{1}}} }^{+}  }  \Gamma_{{\mathrm{1}}}  \refenvsym{,}  \Gamma_{{\mathrm{2}}} ^{ \refenvnt{k_{{\mathrm{1}}}} , \refenvnt{k_{{\mathrm{2}}}} }  \vdash \gamma_{{\mathrm{5}}} \subseteq \delta'' ,
        \quad\text{and}\quad
         \Psi \mid^{  \overrightarrow{ \gamma_{{\mathrm{1}}} }^{+}  }  \Gamma_{{\mathrm{1}}}  \refenvsym{,}  \Gamma_{{\mathrm{2}}} ^{ \refenvnt{k_{{\mathrm{1}}}} , \refenvnt{k_{{\mathrm{2}}}} }  \vdash \gamma_{{\mathrm{3}}} \subseteq \gamma_{{\mathrm{5}}} .
      \]
      Reapplying the variable context rule gives
      $ \Psi \mid^{  \overrightarrow{ \gamma_{{\mathrm{1}}} }^{+}  }  \Gamma_{{\mathrm{1}}}  \refenvsym{,}  \Gamma_{{\mathrm{2}}} ^{ \refenvnt{k_{{\mathrm{1}}}} , \refenvnt{k_{{\mathrm{2}}}} }  \vdash \delta'' \subseteq \gamma_{{\mathrm{4}}} $.  Thus
      $ \Psi \mid^{  \overrightarrow{ \gamma_{{\mathrm{1}}} }^{+}  }  \Gamma_{{\mathrm{1}}}  \refenvsym{,}  \Gamma_{{\mathrm{2}}} ^{ \refenvnt{k_{{\mathrm{1}}}} , \refenvnt{k_{{\mathrm{2}}}} }  \vdash \gamma_{{\mathrm{5}}} \subseteq \gamma_{{\mathrm{4}}} $ by
      \ref{rule:runtime-gtrans-trans}.

    \item[Case \textmd{$ \Gamma_{{\mathrm{2}}} ^{ \refenvnt{k_{{\mathrm{1}}}} , \refenvnt{k_{{\mathrm{2}}}} }  =
           \Gamma_{{\mathrm{3}}} ^{ \refenvnt{k_{{\mathrm{1}}}} , \refenvnt{k_{{\mathrm{3}}}} }   \refenvsym{,}   \blacktriangleleft _{ \refenvnt{k_{{\mathrm{4}}}} }^{\binder{ \gamma_{{\mathrm{4}}} } }   \refenvsym{,}  \Gamma_{{\mathrm{4}}}$}:]
      By regularity, we have
      $ \Psi \mid^{  \overrightarrow{ \gamma_{{\mathrm{1}}} }^{+}  }  \Gamma_{{\mathrm{1}}}  \refenvsym{,}  \Gamma_{{\mathrm{3}}} ^{ \refenvnt{k_{{\mathrm{1}}}} , \refenvnt{k_{{\mathrm{3}}}} }  \vdash^{  \dotsc   \refenvsym{,}    \delta' _{ 0 }  ,\dotsc,  \delta' _{ \refenvnt{k_{{\mathrm{4}}}} }   }\token{wf} $.
      By \zcref{claim:inversion-runtime-gtrans-ctx}, either
      $ \Psi \mid^{  \overrightarrow{ \gamma_{{\mathrm{1}}} }^{+}  }  \Gamma_{{\mathrm{1}}}  \refenvsym{,}  \Gamma_{{\mathrm{2}}} ^{ \refenvnt{k_{{\mathrm{1}}}} , \refenvnt{k_{{\mathrm{2}}}} }  \vdash \gamma_{{\mathrm{3}}} \subseteq  \delta' _{ 0 }  $ or
      $ \Psi \mid^{  \overrightarrow{ \gamma_{{\mathrm{1}}} }^{+}  }  \Gamma_{{\mathrm{1}}}  \refenvsym{,}  \Gamma_{{\mathrm{2}}} ^{ \refenvnt{k_{{\mathrm{1}}}} , \refenvnt{k_{{\mathrm{2}}}} }  \vdash \gamma_{{\mathrm{3}}} \subseteq  \delta' _{ \refenvnt{k_{{\mathrm{4}}}} }  $.  Let $\delta''$ be the
      right-hand classifier obtained in this way.  By
      \zcref{claim:ctx-output-classifier-origin},
      $\delta'' \, \in \, \refenvsym{\{}    \delta _{ 0 }  ,\dotsc,  \delta _{ \refenvnt{k_{{\mathrm{1}}}} }    \refenvsym{\}} \, \cup \,  \token{Dom}_{C}(  \Gamma_{{\mathrm{2}}} ^{ \refenvnt{k_{{\mathrm{1}}}} , \refenvnt{k_{{\mathrm{2}}}} }  )  \, \cup \,  \token{FC}(  \Gamma_{{\mathrm{2}}} ^{ \refenvnt{k_{{\mathrm{1}}}} , \refenvnt{k_{{\mathrm{2}}}} }  ) $.  Since
      $ \token{deg} ( \Psi , \refenvsym{(}   \Gamma_{{\mathrm{1}}}  \refenvsym{,}  \Gamma_{{\mathrm{2}}} ^{ \refenvnt{k_{{\mathrm{1}}}} , \refenvnt{k_{{\mathrm{2}}}} }   \refenvsym{)} , \delta'' )  <
       \token{deg} ( \Psi , \refenvsym{(}   \Gamma_{{\mathrm{1}}}  \refenvsym{,}  \Gamma_{{\mathrm{2}}} ^{ \refenvnt{k_{{\mathrm{1}}}} , \refenvnt{k_{{\mathrm{2}}}} }   \refenvsym{)} , \gamma_{{\mathrm{4}}} ) $, the induction hypothesis gives
      some $\gamma_{{\mathrm{5}}}$ such that
      \[
        \gamma_{{\mathrm{5}}} \, \in \, \refenvsym{\{}    \delta _{ 0 }  ,\dotsc,  \delta _{ \refenvnt{k_{{\mathrm{1}}}} }    \refenvsym{\}} \, \cup \,  \token{FC}(  \Gamma_{{\mathrm{2}}} ^{ \refenvnt{k_{{\mathrm{1}}}} , \refenvnt{k_{{\mathrm{2}}}} }  ) ,\qquad
         \Psi \mid^{  \overrightarrow{ \gamma_{{\mathrm{1}}} }^{+}  }  \Gamma_{{\mathrm{1}}}  \refenvsym{,}  \Gamma_{{\mathrm{2}}} ^{ \refenvnt{k_{{\mathrm{1}}}} , \refenvnt{k_{{\mathrm{2}}}} }  \vdash \gamma_{{\mathrm{5}}} \subseteq \delta'' ,
        \quad\text{and}\quad
         \Psi \mid^{  \overrightarrow{ \gamma_{{\mathrm{1}}} }^{+}  }  \Gamma_{{\mathrm{1}}}  \refenvsym{,}  \Gamma_{{\mathrm{2}}} ^{ \refenvnt{k_{{\mathrm{1}}}} , \refenvnt{k_{{\mathrm{2}}}} }  \vdash \gamma_{{\mathrm{3}}} \subseteq \gamma_{{\mathrm{5}}} .
      \]
      Reapplying the corresponding $ \blacktriangleleft $ context rule gives
      $ \Psi \mid^{  \overrightarrow{ \gamma_{{\mathrm{1}}} }^{+}  }  \Gamma_{{\mathrm{1}}}  \refenvsym{,}  \Gamma_{{\mathrm{2}}} ^{ \refenvnt{k_{{\mathrm{1}}}} , \refenvnt{k_{{\mathrm{2}}}} }  \vdash \delta'' \subseteq \gamma_{{\mathrm{4}}} $.  Thus
      $ \Psi \mid^{  \overrightarrow{ \gamma_{{\mathrm{1}}} }^{+}  }  \Gamma_{{\mathrm{1}}}  \refenvsym{,}  \Gamma_{{\mathrm{2}}} ^{ \refenvnt{k_{{\mathrm{1}}}} , \refenvnt{k_{{\mathrm{2}}}} }  \vdash \gamma_{{\mathrm{5}}} \subseteq \gamma_{{\mathrm{4}}} $ by
      \ref{rule:runtime-gtrans-trans}.

    \item[Case \textmd{$ \Gamma_{{\mathrm{2}}} ^{ \refenvnt{k_{{\mathrm{1}}}} , \refenvnt{k_{{\mathrm{2}}}} }  =
           \Gamma_{{\mathrm{3}}} ^{ \refenvnt{k_{{\mathrm{1}}}} , \refenvnt{k_{{\mathrm{3}}}} }   \refenvsym{,}   [    \binder{  \gamma' _{ 1 }  }  \mathbin{:\succeq}    \gamma'' _{ 1 }  ,\dotsc,\binder{  \gamma' _{ \refenvnt{k} }  }  \mathbin{:\succeq}   \gamma''  _{ \refenvnt{k} }   ]^{\binder{ \gamma_{{\mathrm{4}}} } }   \refenvsym{,}  \Gamma_{{\mathrm{4}}}$}:]
      By regularity, we have
      $ \Psi \mid^{  \overrightarrow{ \gamma_{{\mathrm{1}}} }^{+}  }  \Gamma_{{\mathrm{1}}}  \refenvsym{,}  \Gamma_{{\mathrm{3}}} ^{ \refenvnt{k_{{\mathrm{1}}}} , \refenvnt{k_{{\mathrm{3}}}} }  \vdash^{  \dotsc   \refenvsym{,}  \delta'' }\token{wf} $
      for some $\delta''$.
      By \zcref{claim:inversion-runtime-gtrans-ctx}, the derivation factors
      through the output classifier $\delta''$.  By
      \zcref{claim:ctx-output-classifier-origin},
      $\delta'' \, \in \, \refenvsym{\{}    \delta _{ 0 }  ,\dotsc,  \delta _{ \refenvnt{k_{{\mathrm{1}}}} }    \refenvsym{\}} \, \cup \,  \token{Dom}_{C}(  \Gamma_{{\mathrm{2}}} ^{ \refenvnt{k_{{\mathrm{1}}}} , \refenvnt{k_{{\mathrm{2}}}} }  )  \, \cup \,  \token{FC}(  \Gamma_{{\mathrm{2}}} ^{ \refenvnt{k_{{\mathrm{1}}}} , \refenvnt{k_{{\mathrm{2}}}} }  ) $.  Since
      $ \token{deg} ( \Psi , \refenvsym{(}   \Gamma_{{\mathrm{1}}}  \refenvsym{,}  \Gamma_{{\mathrm{2}}} ^{ \refenvnt{k_{{\mathrm{1}}}} , \refenvnt{k_{{\mathrm{2}}}} }   \refenvsym{)} , \delta'' )  <
       \token{deg} ( \Psi , \refenvsym{(}   \Gamma_{{\mathrm{1}}}  \refenvsym{,}  \Gamma_{{\mathrm{2}}} ^{ \refenvnt{k_{{\mathrm{1}}}} , \refenvnt{k_{{\mathrm{2}}}} }   \refenvsym{)} , \gamma_{{\mathrm{4}}} ) $, the induction hypothesis
      gives some $\gamma_{{\mathrm{5}}}$ such that
      \[
        \gamma_{{\mathrm{5}}} \, \in \, \refenvsym{\{}    \delta _{ 0 }  ,\dotsc,  \delta _{ \refenvnt{k_{{\mathrm{1}}}} }    \refenvsym{\}} \, \cup \,  \token{FC}(  \Gamma_{{\mathrm{2}}} ^{ \refenvnt{k_{{\mathrm{1}}}} , \refenvnt{k_{{\mathrm{2}}}} }  ) ,\qquad
         \Psi \mid^{  \overrightarrow{ \gamma_{{\mathrm{1}}} }^{+}  }  \Gamma_{{\mathrm{1}}}  \refenvsym{,}  \Gamma_{{\mathrm{2}}} ^{ \refenvnt{k_{{\mathrm{1}}}} , \refenvnt{k_{{\mathrm{2}}}} }  \vdash \gamma_{{\mathrm{5}}} \subseteq \delta'' ,
        \quad\text{and}\quad
         \Psi \mid^{  \overrightarrow{ \gamma_{{\mathrm{1}}} }^{+}  }  \Gamma_{{\mathrm{1}}}  \refenvsym{,}  \Gamma_{{\mathrm{2}}} ^{ \refenvnt{k_{{\mathrm{1}}}} , \refenvnt{k_{{\mathrm{2}}}} }  \vdash \gamma_{{\mathrm{3}}} \subseteq \gamma_{{\mathrm{5}}} .
      \]
      Reapplying the corresponding polymorphic-classifier context rule gives
      $ \Psi \mid^{  \overrightarrow{ \gamma_{{\mathrm{1}}} }^{+}  }  \Gamma_{{\mathrm{1}}}  \refenvsym{,}  \Gamma_{{\mathrm{2}}} ^{ \refenvnt{k_{{\mathrm{1}}}} , \refenvnt{k_{{\mathrm{2}}}} }  \vdash \delta'' \subseteq \gamma_{{\mathrm{4}}} $.  Thus
      $ \Psi \mid^{  \overrightarrow{ \gamma_{{\mathrm{1}}} }^{+}  }  \Gamma_{{\mathrm{1}}}  \refenvsym{,}  \Gamma_{{\mathrm{2}}} ^{ \refenvnt{k_{{\mathrm{1}}}} , \refenvnt{k_{{\mathrm{2}}}} }  \vdash \gamma_{{\mathrm{5}}} \subseteq \gamma_{{\mathrm{4}}} $ by
      \ref{rule:runtime-gtrans-trans}.

    \item[Case \textmd{$ \Gamma_{{\mathrm{2}}} ^{ \refenvnt{k_{{\mathrm{1}}}} , \refenvnt{k_{{\mathrm{2}}}} }  =
           \Gamma_{{\mathrm{3}}} ^{ \refenvnt{k_{{\mathrm{1}}}} , \refenvnt{k_{{\mathrm{3}}}} }   \refenvsym{,}   [    \binder{  \gamma' _{ 1 }  }  \mathbin{:\succeq}    \gamma'' _{ 1 }  ,\dotsc,\binder{  \gamma' _{ \refenvnt{k} }  }  \mathbin{:\succeq}   \gamma''  _{ \refenvnt{k} }   ]^{\binder{  \gamma' _{ 0 }  } }   \refenvsym{,}  \Gamma_{{\mathrm{4}}}$ and
          $\gamma_{{\mathrm{4}}} =  \gamma' _{ \refenvnt{i} } $ for some $\refenvnt{i}$ with $1 \le \refenvnt{i} \le \refenvnt{k}$}:]
      By \zcref{claim:inversion-runtime-gtrans-ctx}, the derivation factors
      through either $ \gamma'' _{ \refenvnt{i} } $ or, when $\refenvnt{i} < \refenvnt{k}$,
      $ \gamma' _{ \refenvnt{i}  \refenvsym{+}  1 } $.  Let $\delta''$ be the right-hand classifier obtained
      in this way.  The membership condition
      $\delta'' \, \in \, \refenvsym{\{}    \delta _{ 0 }  ,\dotsc,  \delta _{ \refenvnt{k_{{\mathrm{1}}}} }    \refenvsym{\}} \, \cup \,  \token{Dom}_{C}(  \Gamma_{{\mathrm{2}}} ^{ \refenvnt{k_{{\mathrm{1}}}} , \refenvnt{k_{{\mathrm{2}}}} }  )  \, \cup \,  \token{FC}(  \Gamma_{{\mathrm{2}}} ^{ \refenvnt{k_{{\mathrm{1}}}} , \refenvnt{k_{{\mathrm{2}}}} }  ) $
      follows from the definitions of $ \token{Dom}_{C}(  \Gamma_{{\mathrm{2}}} ^{ \refenvnt{k_{{\mathrm{1}}}} , \refenvnt{k_{{\mathrm{2}}}} }  ) $ and
      $ \token{FC}(  \Gamma_{{\mathrm{2}}} ^{ \refenvnt{k_{{\mathrm{1}}}} , \refenvnt{k_{{\mathrm{2}}}} }  ) $.  Since
      $ \token{deg} ( \Psi , \refenvsym{(}   \Gamma_{{\mathrm{1}}}  \refenvsym{,}  \Gamma_{{\mathrm{2}}} ^{ \refenvnt{k_{{\mathrm{1}}}} , \refenvnt{k_{{\mathrm{2}}}} }   \refenvsym{)} , \delta'' )  <
       \token{deg} ( \Psi , \refenvsym{(}   \Gamma_{{\mathrm{1}}}  \refenvsym{,}  \Gamma_{{\mathrm{2}}} ^{ \refenvnt{k_{{\mathrm{1}}}} , \refenvnt{k_{{\mathrm{2}}}} }   \refenvsym{)} , \gamma_{{\mathrm{4}}} ) $, the induction hypothesis
      gives some $\gamma_{{\mathrm{5}}}$ such that
      \[
        \gamma_{{\mathrm{5}}} \, \in \, \refenvsym{\{}    \delta _{ 0 }  ,\dotsc,  \delta _{ \refenvnt{k_{{\mathrm{1}}}} }    \refenvsym{\}} \, \cup \,  \token{FC}(  \Gamma_{{\mathrm{2}}} ^{ \refenvnt{k_{{\mathrm{1}}}} , \refenvnt{k_{{\mathrm{2}}}} }  ) ,\qquad
         \Psi \mid^{  \overrightarrow{ \gamma_{{\mathrm{1}}} }^{+}  }  \Gamma_{{\mathrm{1}}}  \refenvsym{,}  \Gamma_{{\mathrm{2}}} ^{ \refenvnt{k_{{\mathrm{1}}}} , \refenvnt{k_{{\mathrm{2}}}} }  \vdash \gamma_{{\mathrm{5}}} \subseteq \delta'' ,
        \quad\text{and}\quad
         \Psi \mid^{  \overrightarrow{ \gamma_{{\mathrm{1}}} }^{+}  }  \Gamma_{{\mathrm{1}}}  \refenvsym{,}  \Gamma_{{\mathrm{2}}} ^{ \refenvnt{k_{{\mathrm{1}}}} , \refenvnt{k_{{\mathrm{2}}}} }  \vdash \gamma_{{\mathrm{3}}} \subseteq \gamma_{{\mathrm{5}}} .
      \]
      Reapplying the corresponding polymorphic-classifier context rule gives
      $ \Psi \mid^{  \overrightarrow{ \gamma_{{\mathrm{1}}} }^{+}  }  \Gamma_{{\mathrm{1}}}  \refenvsym{,}  \Gamma_{{\mathrm{2}}} ^{ \refenvnt{k_{{\mathrm{1}}}} , \refenvnt{k_{{\mathrm{2}}}} }  \vdash \delta'' \subseteq \gamma_{{\mathrm{4}}} $.  Thus
      $ \Psi \mid^{  \overrightarrow{ \gamma_{{\mathrm{1}}} }^{+}  }  \Gamma_{{\mathrm{1}}}  \refenvsym{,}  \Gamma_{{\mathrm{2}}} ^{ \refenvnt{k_{{\mathrm{1}}}} , \refenvnt{k_{{\mathrm{2}}}} }  \vdash \gamma_{{\mathrm{5}}} \subseteq \gamma_{{\mathrm{4}}} $ by
      \ref{rule:runtime-gtrans-trans}.
  \end{description}
\end{proof}


\begin{lemma}[Upper Bound of Classifiers]
  \label{claim:cls-upper-bound-wrt-gtrans-common}
  Suppose
  \begin{itemize}
    \item $ \Psi \mid^{  \overrightarrow{ \gamma_{{\mathrm{1}}} }^{+}  } \Gamma_{{\mathrm{1}}} \vdash^{  \overrightarrow{ \gamma_{{\mathrm{2}}} }   \refenvsym{,}    \delta _{ 0 }  ,\dotsc,  \delta _{ \refenvnt{k_{{\mathrm{1}}}} }   }\token{wf} $ and
    \item $ \Psi \mid^{  \overrightarrow{ \gamma_{{\mathrm{1}}} }^{+}  }  \Gamma_{{\mathrm{1}}}  \refenvsym{,}  \Gamma_{{\mathrm{2}}} ^{ \refenvnt{k_{{\mathrm{1}}}} , \refenvnt{k_{{\mathrm{2}}}} }  \vdash^{  \overrightarrow{ \gamma_{{\mathrm{4}}} }^{+}  }\token{wf} $.
  \end{itemize}
  If\/ $\gamma_{{\mathrm{5}}} \, \in \,  \token{FC}(  \Gamma_{{\mathrm{2}}} ^{ \refenvnt{k_{{\mathrm{1}}}} , \refenvnt{k_{{\mathrm{2}}}} }  ) $,
  then $ \Psi \mid^{  \overrightarrow{ \gamma_{{\mathrm{1}}} }^{+}  } \Gamma_{{\mathrm{1}}} \vdash \gamma_{{\mathrm{5}}} \subseteq  \delta _{ \refenvnt{i} }  $
  for some $\refenvnt{i}$ such that $0 \le \refenvnt{i} \le \refenvnt{k_{{\mathrm{1}}}}$.
\end{lemma}

\begin{proof}
  By induction with respect to the size of $ \Gamma_{{\mathrm{2}}} ^{ \refenvnt{k_{{\mathrm{1}}}} , \refenvnt{k_{{\mathrm{2}}}} } $.
  By the definition of $ \token{FC}(  \Gamma_{{\mathrm{2}}} ^{ \refenvnt{k_{{\mathrm{1}}}} , \refenvnt{k_{{\mathrm{2}}}} }  ) $, it suffices to consider the cases
  in which the occurrence of $\gamma_{{\mathrm{5}}}$ is introduced by the last context
  constructor of $ \Gamma_{{\mathrm{2}}} ^{ \refenvnt{k_{{\mathrm{1}}}} , \refenvnt{k_{{\mathrm{2}}}} } $.  If the occurrence comes from a proper
  subcontext, the result follows from the induction hypothesis and
  \zcref{claim:ctx-weakening}.

  \begin{description}
    \item[Case \textmd{$ \Gamma_{{\mathrm{2}}} ^{ \refenvnt{k_{{\mathrm{1}}}} , \refenvnt{k_{{\mathrm{2}}}} }  =  \Gamma_{{\mathrm{3}}} ^{ \refenvnt{k_{{\mathrm{1}}}} , \refenvnt{k_{{\mathrm{2}}}}  \refenvsym{-}  1 }   \refenvsym{,}   \blacktriangleright ^{ \gamma_{{\mathrm{5}}} } $}:]
      By regularity, we have
      $ \Psi \mid^{  \overrightarrow{ \gamma_{{\mathrm{1}}} }^{+}  }  \Gamma_{{\mathrm{1}}}  \refenvsym{,}  \Gamma_{{\mathrm{3}}} ^{ \refenvnt{k_{{\mathrm{1}}}} , \refenvnt{k_{{\mathrm{2}}}}  \refenvsym{-}  1 }  \vdash^{  \dotsc   \refenvsym{,}  \gamma_{{\mathrm{6}}} }\token{wf} $ for some $\gamma_{{\mathrm{6}}}$.
      The well-formedness of $ \Gamma_{{\mathrm{1}}}  \refenvsym{,}  \Gamma_{{\mathrm{2}}} ^{ \refenvnt{k_{{\mathrm{1}}}} , \refenvnt{k_{{\mathrm{2}}}} } $ gives
      $ \Psi \mid^{  \overrightarrow{ \gamma_{{\mathrm{1}}} }^{+}  }  \Gamma_{{\mathrm{1}}}  \refenvsym{,}  \Gamma_{{\mathrm{3}}} ^{ \refenvnt{k_{{\mathrm{1}}}} , \refenvnt{k_{{\mathrm{2}}}}  \refenvsym{-}  1 }  \vdash \gamma_{{\mathrm{5}}} \subseteq \gamma_{{\mathrm{6}}} $.
      By \zcref{claim:ctx-output-classifier-origin},
      $\gamma_{{\mathrm{6}}} \, \in \, \refenvsym{\{}    \delta _{ 0 }  ,\dotsc,  \delta _{ \refenvnt{k_{{\mathrm{1}}}} }    \refenvsym{\}} \, \cup \,  \token{Dom}_{C}(  \Gamma_{{\mathrm{3}}} ^{ \refenvnt{k_{{\mathrm{1}}}} , \refenvnt{k_{{\mathrm{2}}}}  \refenvsym{-}  1 }  )  \, \cup \,  \token{FC}(  \Gamma_{{\mathrm{3}}} ^{ \refenvnt{k_{{\mathrm{1}}}} , \refenvnt{k_{{\mathrm{2}}}}  \refenvsym{-}  1 }  ) $.
      Also $\gamma_{{\mathrm{5}}} \, \in \,  \token{Dom}_{C}( \Psi )  \, \cup \,  \token{Dom}_{C}( \Gamma_{{\mathrm{1}}} ) $ from $\gamma_{{\mathrm{5}}} \, \in \,  \token{FC}(  \Gamma_{{\mathrm{2}}} ^{ \refenvnt{k_{{\mathrm{1}}}} , \refenvnt{k_{{\mathrm{2}}}} }  ) $.
      Hence
      \zcref{claim:cls-upper-bound-aux} gives some $\gamma_{{\mathrm{7}}}$ such that
      \[
        \gamma_{{\mathrm{7}}} \, \in \, \refenvsym{\{}    \delta _{ 0 }  ,\dotsc,  \delta _{ \refenvnt{k_{{\mathrm{1}}}} }    \refenvsym{\}} \, \cup \,  \token{FC}(  \Gamma_{{\mathrm{3}}} ^{ \refenvnt{k_{{\mathrm{1}}}} , \refenvnt{k_{{\mathrm{2}}}}  \refenvsym{-}  1 }  ) ,\qquad
         \Psi \mid^{  \overrightarrow{ \gamma_{{\mathrm{1}}} }^{+}  }  \Gamma_{{\mathrm{1}}}  \refenvsym{,}  \Gamma_{{\mathrm{3}}} ^{ \refenvnt{k_{{\mathrm{1}}}} , \refenvnt{k_{{\mathrm{2}}}}  \refenvsym{-}  1 }  \vdash \gamma_{{\mathrm{7}}} \subseteq \gamma_{{\mathrm{6}}} ,
        \quad\text{and}\quad
         \Psi \mid^{  \overrightarrow{ \gamma_{{\mathrm{1}}} }^{+}  }  \Gamma_{{\mathrm{1}}}  \refenvsym{,}  \Gamma_{{\mathrm{3}}} ^{ \refenvnt{k_{{\mathrm{1}}}} , \refenvnt{k_{{\mathrm{2}}}}  \refenvsym{-}  1 }  \vdash \gamma_{{\mathrm{5}}} \subseteq \gamma_{{\mathrm{7}}} .
      \]
      If $\gamma_{{\mathrm{7}}} \, \in \, \refenvsym{\{}    \delta _{ 0 }  ,\dotsc,  \delta _{ \refenvnt{k_{{\mathrm{1}}}} }    \refenvsym{\}}$, choose $\refenvnt{i}$ such that $ \delta _{ \refenvnt{i} }  = \gamma_{{\mathrm{7}}}$.
      By \zcref{claim:ctx-weakening}, the judgment
      $ \Psi \mid^{  \overrightarrow{ \gamma_{{\mathrm{1}}} }^{+}  }  \Gamma_{{\mathrm{1}}}  \refenvsym{,}  \Gamma_{{\mathrm{2}}} ^{ \refenvnt{k_{{\mathrm{1}}}} , \refenvnt{k_{{\mathrm{2}}}} }  \vdash \gamma_{{\mathrm{5}}} \subseteq  \delta _{ \refenvnt{i} }  $ gives the desired judgment for $ \delta _{ \refenvnt{i} } $.

      Otherwise, $\gamma_{{\mathrm{7}}} \, \in \,  \token{FC}(  \Gamma_{{\mathrm{3}}} ^{ \refenvnt{k_{{\mathrm{1}}}} , \refenvnt{k_{{\mathrm{2}}}}  \refenvsym{-}  1 }  ) $. By the induction hypothesis, there exists
      some $\refenvnt{j}$ with $0 \le \refenvnt{j} \le \refenvnt{k_{{\mathrm{1}}}}$ such that
      $ \Psi \mid^{  \overrightarrow{ \gamma_{{\mathrm{1}}} }^{+}  }  \Gamma_{{\mathrm{1}}}  \refenvsym{,}  \Gamma_{{\mathrm{3}}} ^{ \refenvnt{k_{{\mathrm{1}}}} , \refenvnt{k_{{\mathrm{2}}}}  \refenvsym{-}  1 }  \vdash \gamma_{{\mathrm{7}}} \subseteq  \delta _{ \refenvnt{j} }  $.
      By transitivity, we obtain
      $ \Psi \mid^{  \overrightarrow{ \gamma_{{\mathrm{1}}} }^{+}  }  \Gamma_{{\mathrm{1}}}  \refenvsym{,}  \Gamma_{{\mathrm{3}}} ^{ \refenvnt{k_{{\mathrm{1}}}} , \refenvnt{k_{{\mathrm{2}}}}  \refenvsym{-}  1 }  \vdash \gamma_{{\mathrm{5}}} \subseteq  \delta _{ \refenvnt{j} }  $.
      Then, by \zcref{claim:ctx-weakening},
      $ \Psi \mid^{  \overrightarrow{ \gamma_{{\mathrm{1}}} }^{+}  }  \Gamma_{{\mathrm{1}}}  \refenvsym{,}  \Gamma_{{\mathrm{2}}} ^{ \refenvnt{k_{{\mathrm{1}}}} , \refenvnt{k_{{\mathrm{2}}}} }  \vdash \gamma_{{\mathrm{5}}} \subseteq  \delta _{ \refenvnt{j} }  $.
      Since $ \delta _{ \refenvnt{j} }  \, \in \,  \token{Dom}_{C}( \Psi )  \, \cup \,  \token{Dom}_{C}( \Gamma_{{\mathrm{1}}} ) $, applying \zcref{claim:ctx-strengthening} yields
      $ \Psi \mid^{  \overrightarrow{ \gamma_{{\mathrm{1}}} }^{+}  } \Gamma_{{\mathrm{1}}} \vdash \gamma_{{\mathrm{5}}} \subseteq  \delta _{ \refenvnt{j} }  $.
      Hence, we may take $\refenvnt{i} = \refenvnt{j}$.

    \item[Case \textmd{$ \Gamma_{{\mathrm{2}}} ^{ \refenvnt{k_{{\mathrm{1}}}} , \refenvnt{k_{{\mathrm{2}}}} }  =
           \Gamma_{{\mathrm{3}}} ^{ \refenvnt{k_{{\mathrm{1}}}} , \refenvnt{k_{{\mathrm{2}}}} }   \refenvsym{,}   [    \binder{  \delta' _{ 1 }  }  \mathbin{:\succeq}    \gamma' _{ 1 }  ,\dotsc,\binder{  \delta' _{ \refenvnt{k_{{\mathrm{3}}}} }  }  \mathbin{:\succeq}   \gamma'  _{ \refenvnt{k_{{\mathrm{3}}}} }   ]^{\binder{  \delta' _{ 0 }  } } $ and
          $\gamma_{{\mathrm{5}}} =  \gamma' _{ \refenvnt{i} } $ with $1 \le \refenvnt{i} \le \refenvnt{k_{{\mathrm{3}}}}$}:]
      By regularity, we have
      $ \Psi \mid^{  \overrightarrow{ \gamma_{{\mathrm{1}}} }^{+}  }  \Gamma_{{\mathrm{1}}}  \refenvsym{,}  \Gamma_{{\mathrm{3}}} ^{ \refenvnt{k_{{\mathrm{1}}}} , \refenvnt{k_{{\mathrm{2}}}} }  \vdash^{  \dotsc   \refenvsym{,}   \gamma' _{ 0 }  }\token{wf} $.
      The well-formedness of $ \Gamma_{{\mathrm{1}}}  \refenvsym{,}  \Gamma_{{\mathrm{2}}} ^{ \refenvnt{k_{{\mathrm{1}}}} , \refenvnt{k_{{\mathrm{2}}}} } $ gives
      $ \Psi \mid^{  \overrightarrow{ \gamma_{{\mathrm{1}}} }^{+}  }  \Gamma_{{\mathrm{1}}}  \refenvsym{,}  \Gamma_{{\mathrm{3}}} ^{ \refenvnt{k_{{\mathrm{1}}}} , \refenvnt{k_{{\mathrm{2}}}} }  \vdash  \gamma' _{ \refenvnt{i} }  \subseteq  \gamma' _{ 0 }  $.
      By \zcref{claim:ctx-output-classifier-origin},
      $ \gamma' _{ 0 }  \, \in \, \refenvsym{\{}    \delta _{ 0 }  ,\dotsc,  \delta _{ \refenvnt{k_{{\mathrm{1}}}} }    \refenvsym{\}} \, \cup \,  \token{Dom}_{C}(  \Gamma_{{\mathrm{3}}} ^{ \refenvnt{k_{{\mathrm{1}}}} , \refenvnt{k_{{\mathrm{2}}}} }  )  \, \cup \,  \token{FC}(  \Gamma_{{\mathrm{3}}} ^{ \refenvnt{k_{{\mathrm{1}}}} , \refenvnt{k_{{\mathrm{2}}}} }  ) $.
      Also $\gamma_{{\mathrm{5}}} \, \in \,  \token{Dom}_{C}( \Psi )  \, \cup \,  \token{Dom}_{C}( \Gamma_{{\mathrm{1}}} ) $ from $\gamma_{{\mathrm{5}}} \, \in \,  \token{FC}(  \Gamma_{{\mathrm{2}}} ^{ \refenvnt{k_{{\mathrm{1}}}} , \refenvnt{k_{{\mathrm{2}}}} }  ) $.
      Hence \zcref{claim:cls-upper-bound-aux} gives some $\gamma_{{\mathrm{6}}}$ such that
      \[
        \gamma_{{\mathrm{6}}} \, \in \, \refenvsym{\{}    \delta _{ 0 }  ,\dotsc,  \delta _{ \refenvnt{k_{{\mathrm{1}}}} }    \refenvsym{\}} \, \cup \,  \token{FC}(  \Gamma_{{\mathrm{3}}} ^{ \refenvnt{k_{{\mathrm{1}}}} , \refenvnt{k_{{\mathrm{2}}}} }  ) ,\qquad
         \Psi \mid^{  \overrightarrow{ \gamma_{{\mathrm{1}}} }^{+}  }  \Gamma_{{\mathrm{1}}}  \refenvsym{,}  \Gamma_{{\mathrm{3}}} ^{ \refenvnt{k_{{\mathrm{1}}}} , \refenvnt{k_{{\mathrm{2}}}} }  \vdash \gamma_{{\mathrm{6}}} \subseteq  \gamma' _{ 0 }  ,
        \quad\text{and}\quad
         \Psi \mid^{  \overrightarrow{ \gamma_{{\mathrm{1}}} }^{+}  }  \Gamma_{{\mathrm{1}}}  \refenvsym{,}  \Gamma_{{\mathrm{3}}} ^{ \refenvnt{k_{{\mathrm{1}}}} , \refenvnt{k_{{\mathrm{2}}}} }  \vdash \gamma_{{\mathrm{5}}} \subseteq \gamma_{{\mathrm{6}}} .
      \]
      If $\gamma_{{\mathrm{6}}} \, \in \, \refenvsym{\{}    \delta _{ 0 }  ,\dotsc,  \delta _{ \refenvnt{k_{{\mathrm{1}}}} }    \refenvsym{\}}$, choose $\refenvnt{i}$ such that
      $ \delta _{ \refenvnt{i} }  = \gamma_{{\mathrm{6}}}$.  By \zcref{claim:ctx-weakening}, the judgment
      $ \Psi \mid^{  \overrightarrow{ \gamma_{{\mathrm{1}}} }^{+}  }  \Gamma_{{\mathrm{1}}}  \refenvsym{,}  \Gamma_{{\mathrm{2}}} ^{ \refenvnt{k_{{\mathrm{1}}}} , \refenvnt{k_{{\mathrm{2}}}} }  \vdash \gamma_{{\mathrm{5}}} \subseteq  \delta _{ \refenvnt{i} }  $ gives the desired judgment for $ \delta _{ \refenvnt{i} } $.

      Otherwise $\gamma_{{\mathrm{6}}} \, \in \,  \token{FC}(  \Gamma_{{\mathrm{3}}} ^{ \refenvnt{k_{{\mathrm{1}}}} , \refenvnt{k_{{\mathrm{2}}}} }  ) $, and the induction hypothesis gives
      some $0 \le \refenvnt{j} \le \refenvnt{k_{{\mathrm{1}}}}$ with
      $ \Psi \mid^{  \overrightarrow{ \gamma_{{\mathrm{1}}} }^{+}  }  \Gamma_{{\mathrm{1}}}  \refenvsym{,}  \Gamma_{{\mathrm{3}}} ^{ \refenvnt{k_{{\mathrm{1}}}} , \refenvnt{k_{{\mathrm{2}}}} }  \vdash \gamma_{{\mathrm{6}}} \subseteq  \delta _{ \refenvnt{j} }  $.
      By transitivity, $ \Psi \mid^{  \overrightarrow{ \gamma_{{\mathrm{1}}} }^{+}  }  \Gamma_{{\mathrm{1}}}  \refenvsym{,}  \Gamma_{{\mathrm{3}}} ^{ \refenvnt{k_{{\mathrm{1}}}} , \refenvnt{k_{{\mathrm{2}}}} }  \vdash \gamma_{{\mathrm{5}}} \subseteq  \delta _{ \refenvnt{j} }  $.
      Then $ \Psi \mid^{  \overrightarrow{ \gamma_{{\mathrm{1}}} }^{+}  }  \Gamma_{{\mathrm{1}}}  \refenvsym{,}  \Gamma_{{\mathrm{2}}} ^{ \refenvnt{k_{{\mathrm{1}}}} , \refenvnt{k_{{\mathrm{2}}}} }  \vdash \gamma_{{\mathrm{5}}} \subseteq  \delta _{ \refenvnt{j} }  $ by
      \zcref{claim:ctx-weakening}. Thus we can take $\refenvnt{i} = \refenvnt{j}$.

      In either case, since $ \delta _{ \refenvnt{i} }  \, \in \,  \token{Dom}_{C}( \Psi )  \, \cup \,  \token{Dom}_{C}( \Gamma_{{\mathrm{1}}} ) $,
      applying \zcref{claim:ctx-strengthening} yields
      $ \Psi \mid^{  \overrightarrow{ \gamma_{{\mathrm{1}}} }^{+}  } \Gamma_{{\mathrm{1}}} \vdash \gamma_{{\mathrm{5}}} \subseteq  \delta _{ \refenvnt{i} }  $.
  \end{description}
\end{proof}

\begin{corollary}[Upper Bound of Classifiers Case 1]
  \label{claim:cls-upper-bound-wrt-gtrans-1}
  Suppose\/ $ \Psi \mid^{ \gamma_{{\mathrm{1}}} } \Gamma_{{\mathrm{1}}} \vdash^{  \overrightarrow{ \gamma_{{\mathrm{2}}} }   \refenvsym{,}  \gamma_{{\mathrm{3}}} }\token{wf} $
  and\/ $ \Psi \mid^{ \gamma_{{\mathrm{1}}} }  \Gamma_{{\mathrm{1}}}  \refenvsym{,}  \Gamma_{{\mathrm{2}}} ^{ 0 , \refenvnt{k} }  \vdash^{  \overrightarrow{ \gamma_{{\mathrm{4}}} }^{+}  }\token{wf} $.
  If $\gamma_{{\mathrm{5}}} \, \in \,  \token{FC}(  \Gamma_{{\mathrm{2}}} ^{ 0 , \refenvnt{k} }  ) $,
  then $ \Psi \mid^{ \gamma_{{\mathrm{1}}} } \Gamma_{{\mathrm{1}}} \vdash \gamma_{{\mathrm{5}}} \subseteq \gamma_{{\mathrm{3}}} $.
\end{corollary}

\begin{corollary}[Upper Bound of Classifiers Case 2]
  \label{claim:cls-upper-bound-wrt-gtrans-2}
  If\/ $ \Psi \mid^{  \overrightarrow{ \gamma_{{\mathrm{1}}} }^{+}  } \Gamma \vdash^{  \overrightarrow{ \gamma_{{\mathrm{2}}} }^{+}  }\token{wf} $,
  and $\gamma_{{\mathrm{3}}} \, \in \,  \token{FC}( \Gamma ) $,
  then $ \Psi \mid^{  \overrightarrow{ \gamma_{{\mathrm{1}}} }^{+}  } \Gamma \vdash \gamma_{{\mathrm{3}}} \subseteq \gamma_{{\mathrm{4}}} $
  for some $\gamma_{{\mathrm{4}}} \, \in \, \refenvsym{\{}   \overrightarrow{ \gamma_{{\mathrm{1}}} }^{+}   \refenvsym{\}}$.
\end{corollary}

\subsection{Properties of Value Typing}
\begin{lemma}\label{claim:value-portability-code-aux2}
  Let $\Gamma_{{\mathrm{1}}} =   [   \varrho _{ 1 }   ]^{\binder{  \gamma _{ 1 }  } }  ,\dotsc,  [   \varrho _{ \refenvnt{k_{{\mathrm{1}}}} }   ]^{\binder{  \gamma _{ \refenvnt{k_{{\mathrm{1}}}} }  } }  $
  and $ \Psi \mid^{  \gamma _{ 0 }  } \Gamma_{{\mathrm{1}}} \vdash \delta_{{\mathrm{1}}} \subseteq  \gamma _{ \refenvnt{k_{{\mathrm{1}}}} }  $
  where $\refenvnt{k_{{\mathrm{1}}}} \ge 0$.
  Suppose $ \gamma _{ \refenvnt{i} }  \, \not\in \,   \token{FC}(  \varrho _{ \refenvnt{i}  \refenvsym{+}  1 }  )  \cup\dotsb\cup  \token{FC}(  \varrho _{ \refenvnt{k_{{\mathrm{1}}}} }  )   \, \cup \, \refenvsym{\{}  \delta_{{\mathrm{1}}}  \refenvsym{\}}$
  for $1 \le \refenvnt{i} \le \refenvnt{k_{{\mathrm{1}}}}$.
  If\/ $\delta_{{\mathrm{1}}} \, \in \,  \token{Dom}_{C}( \Gamma_{{\mathrm{1}}} ) $ and $ \Psi \mid^{  \gamma _{ 0 }  } \Gamma_{{\mathrm{1}}} \vdash \delta_{{\mathrm{2}}} \subseteq \delta_{{\mathrm{1}}} $
  then $\delta_{{\mathrm{2}}} \, \not\in \, \refenvsym{\{}    \gamma _{ 1 }  ,\dotsc,  \gamma _{ \refenvnt{k_{{\mathrm{1}}}} }    \refenvsym{\}}$.
\end{lemma}

\begin{proof}
  By induction on $ \token{deg} ( \Psi , \Gamma_{{\mathrm{1}}} , \delta_{{\mathrm{1}}} ) $.
  The freshness assumption gives $\delta_{{\mathrm{1}}} \, \not\in \, \refenvsym{\{}    \gamma _{ 1 }  ,\dotsc,  \gamma _{ \refenvnt{k_{{\mathrm{1}}}} }    \refenvsym{\}}$.
  Since $\delta_{{\mathrm{1}}} \, \in \,  \token{Dom}_{C}( \Gamma_{{\mathrm{1}}} ) $,
  there exist $\refenvnt{k_{{\mathrm{2}}}}$, $\refenvnt{k_{{\mathrm{3}}}}$, and $\refenvnt{k_{{\mathrm{4}}}}$ such that
  $ \varrho _{ \refenvnt{k_{{\mathrm{2}}}} }  =
   \binder{  \gamma' _{ 1 }  }  \mathbin{:\succeq}    \gamma'' _{ 1 }  ,\dotsc,\binder{  \gamma' _{ \refenvnt{k_{{\mathrm{3}}}} }  }  \mathbin{:\succeq}    \gamma'' _{ \refenvnt{k_{{\mathrm{3}}}} }  $,
  $\delta_{{\mathrm{1}}} =  \gamma' _{ \refenvnt{k_{{\mathrm{4}}}} } $, and
  $1 \le \refenvnt{k_{{\mathrm{4}}}} \le \refenvnt{k_{{\mathrm{3}}}}$.

  First suppose $\refenvnt{k_{{\mathrm{4}}}} < \refenvnt{k_{{\mathrm{3}}}}$.  By
  \zcref{claim:inversion-runtime-gtrans-ctx}, either
  $ \Psi \mid^{  \gamma _{ 0 }  } \Gamma_{{\mathrm{1}}} \vdash \delta_{{\mathrm{2}}} \subseteq  \gamma'' _{ \refenvnt{k_{{\mathrm{4}}}} }  $ or
  $ \Psi \mid^{  \gamma _{ 0 }  } \Gamma_{{\mathrm{1}}} \vdash \delta_{{\mathrm{2}}} \subseteq  \gamma' _{ \refenvnt{k_{{\mathrm{4}}}}  \refenvsym{+}  1 }  $.
  Let $\delta_{{\mathrm{3}}}$ be the right-hand classifier obtained in this way.
  Then $\delta_{{\mathrm{3}}} \, \in \,  \token{Dom}_{C}( \Psi )  \, \cup \,  \token{Dom}_{C}( \Gamma_{{\mathrm{1}}} ) $ by \zcref{claim:regularity-runtime-judgments}.

  If\/ $\delta_{{\mathrm{3}}} \, \in \,  \token{Dom}_{C}( \Psi ) $, then $\delta_{{\mathrm{2}}} \, \in \,  \token{Dom}_{C}( \Psi ) $ follows from
  $ \Psi \mid^{  \gamma _{ 0 }  } \Gamma_{{\mathrm{1}}} \vdash \delta_{{\mathrm{2}}} \subseteq \delta_{{\mathrm{3}}} $ and
  \zcref{claim:deg-preserves-trans-order}.
  Thus $\delta_{{\mathrm{2}}} \, \not\in \, \refenvsym{\{}    \gamma _{ 1 }  ,\dotsc,  \gamma _{ \refenvnt{k_{{\mathrm{1}}}} }    \refenvsym{\}}$ by the disjointness of
  $ \token{Dom}_{C}( \Psi ) $ and $ \token{Dom}_{C}( \Gamma_{{\mathrm{1}}} ) $.

  If\/ $\delta_{{\mathrm{3}}} \, \in \,  \token{Dom}_{C}( \Gamma_{{\mathrm{1}}} ) $, then $ \varrho _{ \refenvnt{k_{{\mathrm{2}}}} } $ gives
  $ \Psi \mid^{  \gamma _{ 0 }  } \Gamma_{{\mathrm{1}}} \vdash \delta_{{\mathrm{3}}} \subseteq \delta_{{\mathrm{1}}} $. Together with
  $ \Psi \mid^{  \gamma _{ 0 }  } \Gamma_{{\mathrm{1}}} \vdash \delta_{{\mathrm{1}}} \subseteq  \gamma _{ \refenvnt{k_{{\mathrm{1}}}} }  $, transitivity yields
  $ \Psi \mid^{  \gamma _{ 0 }  } \Gamma_{{\mathrm{1}}} \vdash \delta_{{\mathrm{3}}} \subseteq  \gamma _{ \refenvnt{k_{{\mathrm{1}}}} }  $.

  Moreover, the original non-occurrence assumption implies
  \[
     \gamma _{ \refenvnt{i} }  \, \not\in \,   \token{FC}(  \varrho _{ \refenvnt{i}  \refenvsym{+}  1 }  )  \cup\dotsb\cup  \token{FC}(  \varrho _{ \refenvnt{k_{{\mathrm{1}}}} }  )   \, \cup \, \refenvsym{\{}  \delta_{{\mathrm{3}}}  \refenvsym{\}}.
  \]
  Here, we use $\delta_{{\mathrm{3}}} \, \in \,  \token{FC}(  \varrho _{ \refenvnt{k_{{\mathrm{2}}}} }  ) $ when
  $\delta_{{\mathrm{3}}} =  \gamma'' _{ \refenvnt{k_{{\mathrm{4}}}} } $, and
  $ \gamma _{ \refenvnt{i} }  \neq  \gamma' _{ \refenvnt{k_{{\mathrm{4}}}}  \refenvsym{+}  1 } $ when
  $\delta_{{\mathrm{3}}} =  \gamma' _{ \refenvnt{k_{{\mathrm{4}}}}  \refenvsym{+}  1 } $.

  Finally, by \zcref{claim:deg-preserves-trans-order},
  \[
     \token{deg} ( \Psi , \Gamma_{{\mathrm{1}}} , \delta_{{\mathrm{3}}} )  <  \token{deg} ( \Psi , \Gamma_{{\mathrm{1}}} , \delta_{{\mathrm{1}}} ) .
  \]
  Therefore, applying the induction hypothesis to $\delta_{{\mathrm{3}}}$ yields
  $\delta_{{\mathrm{2}}} \, \not\in \, \refenvsym{\{}    \gamma _{ 1 }  ,\dotsc,  \gamma _{ \refenvnt{k_{{\mathrm{1}}}} }    \refenvsym{\}}$.

  The case $\refenvnt{k_{{\mathrm{4}}}} = \refenvnt{k_{{\mathrm{3}}}}$ is analogous, using the conclusion
  $ \Psi \mid^{  \gamma _{ 0 }  } \Gamma_{{\mathrm{1}}} \vdash \delta_{{\mathrm{2}}} \subseteq  \gamma'' _{ \refenvnt{k_{{\mathrm{4}}}} }  $ obtained from
  \zcref{claim:inversion-runtime-gtrans-ctx}.
\end{proof}

\begin{lemma}\label{claim:value-portability-code-aux1}
  Let $\Gamma_{{\mathrm{1}}} =   [   \varrho _{ 1 }   ]^{\binder{  \gamma _{ 1 }  } }  ,\dotsc,  [   \varrho _{ \refenvnt{k_{{\mathrm{1}}}} }   ]^{\binder{  \gamma _{ \refenvnt{k_{{\mathrm{1}}}} }  } }    \refenvsym{,}   \blacktriangleright ^{ \delta_{{\mathrm{1}}} } $
  where $\refenvnt{k_{{\mathrm{1}}}} \ge 0$
  and\/ $ \gamma _{ \refenvnt{i} }  \, \not\in \,   \token{FC}(  \varrho _{ \refenvnt{i}  \refenvsym{+}  1 }  )  \cup\dotsb\cup  \token{FC}(  \varrho _{ \refenvnt{k_{{\mathrm{1}}}} }  )   \, \cup \, \refenvsym{\{}  \delta_{{\mathrm{1}}}  \refenvsym{\}}$ for $1 \le \refenvnt{i} \le \refenvnt{k_{{\mathrm{1}}}}$.
  If\/ $ \Psi \mid^{ \gamma' }  \Gamma_{{\mathrm{1}}}  \refenvsym{,}  \Gamma_{{\mathrm{2}}} ^{ 0 , \refenvnt{k_{{\mathrm{2}}}} }  \vdash^{  \gamma _{ \refenvnt{k_{{\mathrm{1}}}} }   \refenvsym{[}   \gamma _{ 0 }   \coloneqq  \gamma'  \refenvsym{]}  \refenvsym{,}   \overrightarrow{ \delta_{{\mathrm{2}}} }^{+}  }\token{wf} $,
  then the following hold:

  \begin{enumerate}
    \item \label{item:value-portability-code-aux1:ltrans}
          If\/ $ \Psi \mid^{  \gamma _{ 0 }  }  \Gamma_{{\mathrm{1}}}  \refenvsym{,}  \Gamma_{{\mathrm{2}}} ^{ 0 , \refenvnt{k_{{\mathrm{2}}}} }  \vdash \delta'_{{\mathrm{1}}} \preceq \delta'_{{\mathrm{2}}} $
          and either $\delta'_{{\mathrm{2}}} \, \in \,  \token{Dom}_{C}(  \Gamma_{{\mathrm{2}}} ^{ 0 , \refenvnt{k_{{\mathrm{2}}}} }  ) $ or $ \Psi \mid^{  \gamma _{ 0 }  } \Gamma_{{\mathrm{1}}} \vdash \delta'_{{\mathrm{2}}} \subseteq \delta_{{\mathrm{1}}} $,
          then $ \Psi \mid^{ \gamma' }  \Gamma_{{\mathrm{1}}}  \refenvsym{,}  \Gamma_{{\mathrm{2}}} ^{ 0 , \refenvnt{k_{{\mathrm{2}}}} }  \vdash \delta'_{{\mathrm{1}}} \preceq \delta'_{{\mathrm{2}}} $.
    \item \label{item:value-portability-code-aux1:gtrans}
          If\/ $ \Psi \mid^{  \gamma _{ 0 }  }  \Gamma_{{\mathrm{1}}}  \refenvsym{,}  \Gamma_{{\mathrm{2}}} ^{ 0 , \refenvnt{k_{{\mathrm{2}}}} }  \vdash \delta'_{{\mathrm{1}}} \subseteq \delta'_{{\mathrm{2}}} $
          and either
           $\delta'_{{\mathrm{2}}} \, \in \,  \token{Dom}_{C}(  \Gamma_{{\mathrm{2}}} ^{ 0 , \refenvnt{k_{{\mathrm{2}}}} }  ) $ or $ \Psi \mid^{  \gamma _{ 0 }  } \Gamma_{{\mathrm{1}}} \vdash \delta'_{{\mathrm{2}}} \subseteq \delta_{{\mathrm{1}}} $,
          then $ \Psi \mid^{ \gamma' }  \Gamma_{{\mathrm{1}}}  \refenvsym{,}  \Gamma_{{\mathrm{2}}} ^{ 0 , \refenvnt{k_{{\mathrm{2}}}} }  \vdash \delta'_{{\mathrm{1}}} \subseteq \delta'_{{\mathrm{2}}} $.
    % \item \label{item:value-portability-code-aux1:ctx}
    %       If\/ $ \Psi \mid^{  \gamma _{ 0 }  }  \Gamma_{{\mathrm{1}}}  \refenvsym{,}  \Gamma_{{\mathrm{2}}} ^{ 0 , \refenvnt{k_{{\mathrm{2}}}} }  \vdash^{  \gamma _{ \refenvnt{k_{{\mathrm{1}}}} }   \refenvsym{,}   \overrightarrow{ \delta_{{\mathrm{3}}} }^{+}  }\token{wf} $,
    %       then $ \overrightarrow{ \delta_{{\mathrm{2}}} }^{+}  =  \overrightarrow{ \delta_{{\mathrm{3}}} }^{+} $.
    \item \label{item:value-portability-code-aux1:type}
          If\/ $ \Psi \mid^{  \gamma _{ 0 }  }   \Gamma_{{\mathrm{1}}}  \refenvsym{,}  \Gamma_{{\mathrm{2}}} ^{ 0 , \refenvnt{k_{{\mathrm{2}}}} }  \vdash ^{  \gamma _{ \refenvnt{k_{{\mathrm{1}}}} }   \refenvsym{,}   \overrightarrow{ \delta_{{\mathrm{2}}} }^{+}  } \refenvnt{A} \ \token{wf} $,
          then $ \Psi \mid^{ \gamma' }   \Gamma_{{\mathrm{1}}}  \refenvsym{,}  \Gamma_{{\mathrm{2}}} ^{ 0 , \refenvnt{k_{{\mathrm{2}}}} }  \vdash ^{  \gamma _{ \refenvnt{k_{{\mathrm{1}}}} }   \refenvsym{[}   \gamma _{ 0 }   \coloneqq  \gamma'  \refenvsym{]}  \refenvsym{,}   \overrightarrow{ \delta_{{\mathrm{2}}} }^{+}  } \refenvnt{A} \ \token{wf} $
    \item \label{item:value-portability-code-aux1:exp}
          If\/ $ \Psi \mid^{  \gamma _{ 0 }  }   \Gamma_{{\mathrm{1}}}  \refenvsym{,}  \Gamma_{{\mathrm{2}}} ^{ 0 , \refenvnt{k_{{\mathrm{2}}}} }  \vdash^{  \gamma _{ \refenvnt{k_{{\mathrm{1}}}} }   \refenvsym{,}   \overrightarrow{ \delta_{{\mathrm{2}}} }^{+}  }_{  \token{id}  }   \refenvnt{e} ^{ \refenvnt{k_{{\mathrm{2}}}}  }  : \refenvnt{A} $,
          then $ \Psi \mid^{ \gamma' }   \Gamma_{{\mathrm{1}}}  \refenvsym{,}  \Gamma_{{\mathrm{2}}} ^{ 0 , \refenvnt{k_{{\mathrm{2}}}} }  \vdash^{  \gamma _{ \refenvnt{k_{{\mathrm{1}}}} }   \refenvsym{[}   \gamma _{ 0 }   \coloneqq  \gamma'  \refenvsym{]}  \refenvsym{,}   \overrightarrow{ \delta_{{\mathrm{2}}} }^{+}  }_{  \token{id}  }   \refenvnt{e} ^{ \refenvnt{k_{{\mathrm{2}}}}  }  : \refenvnt{A} $.
  \end{enumerate}
\end{lemma}

\begin{proof}
  Let $\Gamma =  \Gamma_{{\mathrm{1}}}  \refenvsym{,}  \Gamma_{{\mathrm{2}}} ^{ 0 , \refenvnt{k_{{\mathrm{2}}}} } $.
  We prove the four statements by mutual induction on the derivations appearing
  in their premises.

  \begin{description}
    \item[\zcref{item:value-portability-code-aux1:ltrans}.]
      The proof is analogous to that of
      \zcref{item:value-portability-code-aux1:gtrans}, using the rules and lemmas for
      $ \preceq $ in place of those for $ \subseteq $.

    \item[\zcref{item:value-portability-code-aux1:gtrans}.]
      By induction on $ \token{deg} ( \Psi , \refenvsym{(}   \Gamma_{{\mathrm{1}}}  \refenvsym{,}  \Gamma_{{\mathrm{2}}} ^{ 0 , \refenvnt{k_{{\mathrm{2}}}} }   \refenvsym{)} , \delta'_{{\mathrm{2}}} ) $.
      Since $ \Psi \mid^{  \gamma _{ 0 }  }  \Gamma_{{\mathrm{1}}}  \refenvsym{,}  \Gamma_{{\mathrm{2}}} ^{ 0 , \refenvnt{k_{{\mathrm{2}}}} }  \vdash \delta'_{{\mathrm{1}}} \subseteq \delta'_{{\mathrm{2}}} $ is derivable,
      the classifier $\delta'_{{\mathrm{2}}}$ is declared in $\Psi$, $\Gamma_{{\mathrm{1}}}$, or
      $ \Gamma_{{\mathrm{2}}} ^{ 0 , \refenvnt{k_{{\mathrm{2}}}} } $ by \zcref{claim:regularity-runtime-judgments}.
      \begin{description}
        \item[Case \textmd{$\delta'_{{\mathrm{2}}} \, \in \,  \token{Dom}_{C}(  \Gamma_{{\mathrm{2}}} ^{ 0 , \refenvnt{k_{{\mathrm{2}}}} }  ) $}:]
          We proceed by case analysis using
          \zcref{claim:inversion-runtime-gtrans-ctx}.  We spell out the case
          where $\delta'_{{\mathrm{2}}}$ is introduced by a $ \blacktriangleleft $ entry in
          $ \Gamma_{{\mathrm{2}}} ^{ 0 , \refenvnt{k_{{\mathrm{2}}}} } $.

          Suppose
          $ \Gamma_{{\mathrm{2}}} ^{ 0 , \refenvnt{k_{{\mathrm{2}}}} }  = \Gamma_{{\mathrm{3}}}  \refenvsym{,}   \blacktriangleleft _{ \refenvnt{k_{{\mathrm{3}}}} }^{\binder{ \delta'_{{\mathrm{2}}} } }   \refenvsym{,}  \Gamma_{{\mathrm{4}}}$ and
          $ \Psi \mid^{  \gamma _{ 0 }  } \Gamma_{{\mathrm{1}}}  \refenvsym{,}  \Gamma_{{\mathrm{3}}} \vdash^{  \gamma _{ \refenvnt{k_{{\mathrm{1}}}} }   \refenvsym{,}    \delta'' _{ 1 }  ,\dotsc,  \delta'' _{ \refenvnt{k_{{\mathrm{4}}}} }   }\token{wf} $.
          By \zcref{claim:inversion-runtime-gtrans-ctx}, either
          $ \Psi \mid^{  \gamma _{ 0 }  }  \Gamma_{{\mathrm{1}}}  \refenvsym{,}  \Gamma_{{\mathrm{2}}} ^{ 0 , \refenvnt{k_{{\mathrm{2}}}} }  \vdash \delta'_{{\mathrm{1}}} \subseteq  \delta'' _{ \refenvnt{k_{{\mathrm{4}}}} }  $ or
          $ \Psi \mid^{  \gamma _{ 0 }  }  \Gamma_{{\mathrm{1}}}  \refenvsym{,}  \Gamma_{{\mathrm{2}}} ^{ 0 , \refenvnt{k_{{\mathrm{2}}}} }  \vdash \delta'_{{\mathrm{1}}} \subseteq  \delta'' _{ \refenvnt{k_{{\mathrm{4}}}}  \refenvsym{-}  \refenvnt{k_{{\mathrm{3}}}} }  $.

          In the former case,
          by \zcref{claim:cls-upper-bound-wrt-gtrans-1}, either
          $ \delta'' _{ \refenvnt{k_{{\mathrm{4}}}} }  \, \in \,  \token{Dom}_{C}( \Gamma_{{\mathrm{3}}} ) $ or
          $ \Psi \mid^{  \gamma _{ 0 }  } \Gamma_{{\mathrm{1}}} \vdash  \delta'' _{ \refenvnt{k_{{\mathrm{4}}}} }  \subseteq \delta_{{\mathrm{1}}} $.
          As $ \token{deg} ( \Psi , \refenvsym{(}   \Gamma_{{\mathrm{1}}}  \refenvsym{,}  \Gamma_{{\mathrm{2}}} ^{ 0 , \refenvnt{k_{{\mathrm{2}}}} }   \refenvsym{)} ,  \delta'' _{ \refenvnt{k_{{\mathrm{4}}}} }  )  <  \token{deg} ( \Psi , \refenvsym{(}   \Gamma_{{\mathrm{1}}}  \refenvsym{,}  \Gamma_{{\mathrm{2}}} ^{ 0 , \refenvnt{k_{{\mathrm{2}}}} }   \refenvsym{)} , \delta'_{{\mathrm{2}}} ) $,
          we apply the induction hypothesis to $ \delta'' _{ \refenvnt{k_{{\mathrm{4}}}} } $
          and obtain $ \Psi \mid^{ \gamma' }  \Gamma_{{\mathrm{1}}}  \refenvsym{,}  \Gamma_{{\mathrm{2}}} ^{ 0 , \refenvnt{k_{{\mathrm{2}}}} }  \vdash \delta'_{{\mathrm{1}}} \subseteq  \delta'' _{ \refenvnt{k_{{\mathrm{4}}}} }  $.

          In the latter case,
          by \zcref{claim:regularity-runtime-judgments},
          $\Gamma_{{\mathrm{3}}} = \Gamma_{{\mathrm{5}}}  \refenvsym{,}  \Gamma_{{\mathrm{6}}}$ for some $\Gamma_{{\mathrm{5}}}$ and $\Gamma_{{\mathrm{6}}}$ such that
          $ \Psi \mid^{  \gamma _{ 0 }  } \Gamma_{{\mathrm{1}}}  \refenvsym{,}  \Gamma_{{\mathrm{5}}} \vdash^{  \gamma _{ \refenvnt{k_{{\mathrm{1}}}} }   \refenvsym{,}    \delta'' _{ 1 }  ,\dotsc,  \delta'' _{ \refenvnt{k_{{\mathrm{4}}}}  \refenvsym{-}  \refenvnt{k_{{\mathrm{3}}}} }   }\token{wf} $.
          By \zcref{claim:cls-upper-bound-wrt-gtrans-1}, either
          $ \delta'' _{ \refenvnt{k_{{\mathrm{4}}}}  \refenvsym{-}  \refenvnt{k_{{\mathrm{3}}}} }  \, \in \,  \token{Dom}_{C}( \Gamma_{{\mathrm{5}}} ) $ or
          $ \Psi \mid^{  \gamma _{ 0 }  } \Gamma_{{\mathrm{1}}} \vdash  \delta'' _{ \refenvnt{k_{{\mathrm{4}}}}  \refenvsym{-}  \refenvnt{k_{{\mathrm{3}}}} }  \subseteq \delta_{{\mathrm{1}}} $.
          $ \delta'' _{ \refenvnt{k_{{\mathrm{4}}}}  \refenvsym{-}  \refenvnt{k_{{\mathrm{3}}}} }  \, \in \,  \token{Dom}_{C}( \Gamma_{{\mathrm{5}}} ) $ implies $ \delta'' _{ \refenvnt{k_{{\mathrm{4}}}}  \refenvsym{-}  \refenvnt{k_{{\mathrm{3}}}} }  \, \in \,  \token{Dom}_{C}( \Gamma_{{\mathrm{3}}} ) $.
          As $ \token{deg} ( \Psi , \refenvsym{(}   \Gamma_{{\mathrm{1}}}  \refenvsym{,}  \Gamma_{{\mathrm{2}}} ^{ 0 , \refenvnt{k_{{\mathrm{2}}}} }   \refenvsym{)} ,  \delta'' _{ \refenvnt{k_{{\mathrm{4}}}}  \refenvsym{-}  \refenvnt{k_{{\mathrm{3}}}} }  )  <  \token{deg} ( \Psi , \refenvsym{(}   \Gamma_{{\mathrm{1}}}  \refenvsym{,}  \Gamma_{{\mathrm{2}}} ^{ 0 , \refenvnt{k_{{\mathrm{2}}}} }   \refenvsym{)} , \delta'_{{\mathrm{2}}} ) $,
          we apply the induction hypothesis to $ \delta'' _{ \refenvnt{k_{{\mathrm{4}}}}  \refenvsym{-}  \refenvnt{k_{{\mathrm{3}}}} } $
          and obtain $ \Psi \mid^{ \gamma' }  \Gamma_{{\mathrm{1}}}  \refenvsym{,}  \Gamma_{{\mathrm{2}}} ^{ 0 , \refenvnt{k_{{\mathrm{2}}}} }  \vdash \delta'_{{\mathrm{1}}} \subseteq  \delta'' _{ \refenvnt{k_{{\mathrm{4}}}}  \refenvsym{-}  \refenvnt{k_{{\mathrm{3}}}} }  $.

          Let $\delta_{{\mathrm{3}}}$ be $ \delta'' _{ \refenvnt{k_{{\mathrm{4}}}} } $ or $ \delta'' _{ \refenvnt{k_{{\mathrm{4}}}}  \refenvsym{-}  \refenvnt{k_{{\mathrm{3}}}} } $ for each case.
          Now we have $ \Psi \mid^{ \gamma' }  \Gamma_{{\mathrm{1}}}  \refenvsym{,}  \Gamma_{{\mathrm{2}}} ^{ 0 , \refenvnt{k_{{\mathrm{2}}}} }  \vdash \delta'_{{\mathrm{1}}} \subseteq \delta_{{\mathrm{3}}} $.
          By inverting the well-formedness assumption for $ \Gamma_{{\mathrm{1}}}  \refenvsym{,}  \Gamma_{{\mathrm{2}}} ^{ 0 , \refenvnt{k_{{\mathrm{2}}}} } $ and its
          subcontext with \zcref{claim:regularity-runtime-judgments},
          we have $ \Psi \mid^{ \gamma' } \Gamma_{{\mathrm{1}}}  \refenvsym{,}  \Gamma_{{\mathrm{3}}} \vdash^{  \gamma _{ \refenvnt{k_{{\mathrm{1}}}} }   \refenvsym{[}   \gamma _{ 0 }   \coloneqq  \gamma'  \refenvsym{]}  \refenvsym{,}    \delta'' _{ 1 }  ,\dotsc,  \delta'' _{ \refenvnt{k_{{\mathrm{4}}}} }   }\token{wf} $.

          If\/ $\delta_{{\mathrm{3}}} =  \delta'' _{ \refenvnt{k_{{\mathrm{4}}}} } $, reapplying
          \ref{rule:runtime-gtrans-shut-ctx} yields
          $ \Psi \mid^{ \gamma' }  \Gamma_{{\mathrm{1}}}  \refenvsym{,}  \Gamma_{{\mathrm{2}}} ^{ 0 , \refenvnt{k_{{\mathrm{2}}}} }  \vdash \delta_{{\mathrm{3}}} \subseteq \delta'_{{\mathrm{2}}} $.
          If\/ $\delta_{{\mathrm{3}}} =  \delta'' _{ \refenvnt{k_{{\mathrm{4}}}}  \refenvsym{-}  \refenvnt{k_{{\mathrm{3}}}} } $, the same judgment follows by
          \ref{rule:runtime-ltrans-shut} and \ref{rule:runtime-gtrans-lift}.
          Therefore, by \ref{rule:runtime-gtrans-trans},
          $ \Psi \mid^{ \gamma' }  \Gamma_{{\mathrm{1}}}  \refenvsym{,}  \Gamma_{{\mathrm{2}}} ^{ 0 , \refenvnt{k_{{\mathrm{2}}}} }  \vdash \delta'_{{\mathrm{1}}} \subseteq \delta'_{{\mathrm{2}}} $.

        \item[Case \textmd{$\delta'_{{\mathrm{2}}} \, \in \,  \token{Dom}_{C}( \Gamma_{{\mathrm{1}}} ) $}:]
          Since $\delta'_{{\mathrm{2}}} \, \in \,  \token{Dom}_{C}( \Gamma_{{\mathrm{1}}} ) $, the alternative
          $\delta'_{{\mathrm{2}}} \, \in \,  \token{Dom}_{C}(  \Gamma_{{\mathrm{2}}} ^{ 0 , \refenvnt{k_{{\mathrm{2}}}} }  ) $ is impossible by the disjointness of
          $ \token{Dom}_{C}( \Gamma_{{\mathrm{1}}} ) $ and $ \token{Dom}_{C}(  \Gamma_{{\mathrm{2}}} ^{ 0 , \refenvnt{k_{{\mathrm{2}}}} }  ) $.
          Hence the assumption gives $ \Psi \mid^{  \gamma _{ 0 }  } \Gamma_{{\mathrm{1}}} \vdash \delta'_{{\mathrm{2}}} \subseteq \delta_{{\mathrm{1}}} $.

          Let
          $\Gamma_{{\mathrm{0}}} =   [   \varrho _{ 1 }   ]^{\binder{  \gamma _{ 1 }  } }  ,\dotsc,  [   \varrho _{ \refenvnt{k} }   ]^{\binder{  \gamma _{ \refenvnt{k_{{\mathrm{1}}}} }  } }  $,
          so that $\Gamma_{{\mathrm{1}}} = \Gamma_{{\mathrm{0}}}  \refenvsym{,}   \blacktriangleright ^{ \delta_{{\mathrm{1}}} } $.
          We verify the premises of \zcref{claim:value-portability-code-aux2}
          for this $\Gamma_{{\mathrm{0}}}$.
          First, by construction of $\Gamma_{{\mathrm{1}}}$,
          $ \Psi \mid^{  \gamma _{ 0 }  } \Gamma_{{\mathrm{0}}} \vdash \delta_{{\mathrm{1}}} \subseteq  \gamma _{ \refenvnt{k_{{\mathrm{1}}}} }  $.
          Second, $\delta_{{\mathrm{1}}}$ must be declared in $\Psi$ or in $\Gamma_{{\mathrm{0}}}$,
          because $ \blacktriangleright ^{ \delta_{{\mathrm{1}}} } $ does not declare $\delta_{{\mathrm{1}}}$.
          The former is impossible: if\/ $\delta_{{\mathrm{1}}} \, \in \,  \token{Dom}_{C}( \Psi ) $, then
          \zcref{claim:deg-preserves-trans-order} applied to
          $ \Psi \mid^{  \gamma _{ 0 }  } \Gamma_{{\mathrm{1}}} \vdash \delta'_{{\mathrm{2}}} \subseteq \delta_{{\mathrm{1}}} $ contradicts
          $\delta'_{{\mathrm{2}}} \, \in \,  \token{Dom}_{C}( \Gamma_{{\mathrm{1}}} ) $.
          Thus $\delta_{{\mathrm{1}}} \, \in \,  \token{Dom}_{C}( \Gamma_{{\mathrm{0}}} ) $.
          Finally, the trailing $ \blacktriangleright ^{ \delta_{{\mathrm{1}}} } $ does not contribute to the
          derivation of $ \Psi \mid^{  \gamma _{ 0 }  } \Gamma_{{\mathrm{1}}} \vdash \delta'_{{\mathrm{2}}} \subseteq \delta_{{\mathrm{1}}} $, so
          $ \Psi \mid^{  \gamma _{ 0 }  } \Gamma_{{\mathrm{0}}} \vdash \delta'_{{\mathrm{2}}} \subseteq \delta_{{\mathrm{1}}} $.
          Therefore, by \zcref{claim:value-portability-code-aux2}, we have
          $\delta'_{{\mathrm{2}}} \, \not\in \, \refenvsym{\{}    \gamma _{ 1 }  ,\dotsc,  \gamma _{ \refenvnt{k_{{\mathrm{1}}}} }    \refenvsym{\}}$.

          By \zcref{claim:inversion-runtime-gtrans-ctx} and $\delta'_{{\mathrm{2}}} \, \not\in \, \refenvsym{\{}    \gamma _{ 1 }  ,\dotsc,  \gamma _{ \refenvnt{k_{{\mathrm{1}}}} }    \refenvsym{\}}$,
          we have $ \varrho _{ \refenvnt{k_{{\mathrm{3}}}} }  =  \binder{  \gamma'' _{ 1 }  }  \mathbin{:\succeq}    \delta'' _{ 1 }  ,\dotsc,\binder{  \gamma'' _{ \refenvnt{k_{{\mathrm{4}}}} }  }  \mathbin{:\succeq}    \delta'' _{ \refenvnt{k_{{\mathrm{4}}}} }  $
          and $\delta'_{{\mathrm{2}}} =  \gamma'' _{ \refenvnt{k_{{\mathrm{5}}}} } $ for some $\refenvnt{k_{{\mathrm{5}}}}$ such that $1 \le \refenvnt{k_{{\mathrm{5}}}} \le \refenvnt{k_{{\mathrm{4}}}}$.

          We consider the case $\refenvnt{k_{{\mathrm{5}}}} < \refenvnt{k_{{\mathrm{4}}}}$; the case
          $\refenvnt{k_{{\mathrm{5}}}} = \refenvnt{k_{{\mathrm{4}}}}$ is analogous.
          By \zcref{claim:inversion-runtime-gtrans-ctx}, either
          $ \Psi \mid^{  \gamma _{ 0 }  }  \Gamma_{{\mathrm{1}}}  \refenvsym{,}  \Gamma_{{\mathrm{2}}} ^{ 0 , \refenvnt{k_{{\mathrm{2}}}} }  \vdash \delta'_{{\mathrm{1}}} \subseteq  \delta'' _{ \refenvnt{k_{{\mathrm{5}}}} }  $ or
          $ \Psi \mid^{  \gamma _{ 0 }  }  \Gamma_{{\mathrm{1}}}  \refenvsym{,}  \Gamma_{{\mathrm{2}}} ^{ 0 , \refenvnt{k_{{\mathrm{2}}}} }  \vdash \delta'_{{\mathrm{1}}} \subseteq  \gamma'' _{ \refenvnt{k_{{\mathrm{5}}}}  \refenvsym{+}  1 }  $ holds.
          Let $\delta_{{\mathrm{3}}}$ be the right-hand classifier obtained in this way.
          The declaration $ \varrho _{ \refenvnt{k_{{\mathrm{3}}}} } $ gives
          $ \Psi \mid^{  \gamma _{ 0 }  }  \Gamma_{{\mathrm{1}}}  \refenvsym{,}  \Gamma_{{\mathrm{2}}} ^{ 0 , \refenvnt{k_{{\mathrm{2}}}} }  \vdash \delta_{{\mathrm{3}}} \subseteq \delta'_{{\mathrm{2}}} $.
          By \ref{rule:runtime-gtrans-trans}, combining this with
          $ \Psi \mid^{  \gamma _{ 0 }  }  \Gamma_{{\mathrm{1}}}  \refenvsym{,}  \Gamma_{{\mathrm{2}}} ^{ 0 , \refenvnt{k_{{\mathrm{2}}}} }  \vdash \delta'_{{\mathrm{2}}} \subseteq \delta_{{\mathrm{1}}} $ yields
          $ \Psi \mid^{  \gamma _{ 0 }  }  \Gamma_{{\mathrm{1}}}  \refenvsym{,}  \Gamma_{{\mathrm{2}}} ^{ 0 , \refenvnt{k_{{\mathrm{2}}}} }  \vdash \delta_{{\mathrm{3}}} \subseteq \delta_{{\mathrm{1}}} $.

          Moreover,
          $ \token{deg} ( \Psi , \refenvsym{(}   \Gamma_{{\mathrm{1}}}  \refenvsym{,}  \Gamma_{{\mathrm{2}}} ^{ 0 , \refenvnt{k_{{\mathrm{2}}}} }   \refenvsym{)} , \delta_{{\mathrm{3}}} )  <
           \token{deg} ( \Psi , \refenvsym{(}   \Gamma_{{\mathrm{1}}}  \refenvsym{,}  \Gamma_{{\mathrm{2}}} ^{ 0 , \refenvnt{k_{{\mathrm{2}}}} }   \refenvsym{)} , \delta'_{{\mathrm{2}}} ) $ by
          \zcref{claim:deg-preserves-trans-order}.
          Hence the induction hypothesis applies to $\delta_{{\mathrm{3}}}$, yielding
          $ \Psi \mid^{ \gamma' }  \Gamma_{{\mathrm{1}}}  \refenvsym{,}  \Gamma_{{\mathrm{2}}} ^{ 0 , \refenvnt{k_{{\mathrm{2}}}} }  \vdash \delta'_{{\mathrm{1}}} \subseteq \delta_{{\mathrm{3}}} $.

          By transitivity, combining
          $ \Psi \mid^{ \gamma' }  \Gamma_{{\mathrm{1}}}  \refenvsym{,}  \Gamma_{{\mathrm{2}}} ^{ 0 , \refenvnt{k_{{\mathrm{2}}}} }  \vdash \delta'_{{\mathrm{1}}} \subseteq \delta_{{\mathrm{3}}} $ with
          $ \Psi \mid^{ \gamma' }  \Gamma_{{\mathrm{1}}}  \refenvsym{,}  \Gamma_{{\mathrm{2}}} ^{ 0 , \refenvnt{k_{{\mathrm{2}}}} }  \vdash \delta_{{\mathrm{3}}} \subseteq \delta'_{{\mathrm{2}}} $
          we obtain
          $ \Psi \mid^{ \gamma' }  \Gamma_{{\mathrm{1}}}  \refenvsym{,}  \Gamma_{{\mathrm{2}}} ^{ 0 , \refenvnt{k_{{\mathrm{2}}}} }  \vdash \delta'_{{\mathrm{1}}} \subseteq \delta'_{{\mathrm{2}}} $
          as required.

        \item[Case \textmd{$\delta'_{{\mathrm{2}}} \, \in \,  \token{Dom}_{C}( \Psi ) $}:]
          By \zcref{claim:local-to-global-trans}, we have
          $\Psi  \vdash  \delta'_{{\mathrm{1}}}  \subseteq  \delta'_{{\mathrm{2}}}$.
          Moreover, the well-formedness assumption
          $ \Psi \mid^{ \gamma' }   \Gamma_{{\mathrm{1}}}  \refenvsym{,}  \Gamma_{{\mathrm{2}}} ^{ 0 , \refenvnt{k_{{\mathrm{2}}}} }  \vdash ^{  \gamma _{ \refenvnt{k_{{\mathrm{1}}}} }   \refenvsym{[}   \gamma _{ 0 }   \coloneqq  \gamma'  \refenvsym{]}  \refenvsym{,}   \overrightarrow{ \delta_{{\mathrm{2}}} }^{+}  } \refenvnt{A} \ \token{wf} $
          gives $ \Psi \mid^{ \gamma' }  \Gamma_{{\mathrm{1}}}  \refenvsym{,}  \Gamma_{{\mathrm{2}}} ^{ 0 , \refenvnt{k_{{\mathrm{2}}}} }  \vdash^{  \dotsc  }\token{wf} $.
          Hence, by \zcref{claim:global-to-local-trans}, we obtain
          $ \Psi \mid^{ \gamma' }  \Gamma_{{\mathrm{1}}}  \refenvsym{,}  \Gamma_{{\mathrm{2}}} ^{ 0 , \refenvnt{k_{{\mathrm{2}}}} }  \vdash \delta'_{{\mathrm{1}}} \subseteq \delta'_{{\mathrm{2}}} $.
      \end{description}

    % \item[\zcref{item:value-portability-code-aux1:ctx}.]
    %   By inversion on
    %   $ \Psi \mid^{  \gamma _{ 0 }  }  \Gamma_{{\mathrm{1}}}  \refenvsym{,}  \Gamma_{{\mathrm{2}}} ^{ 0 , \refenvnt{k_{{\mathrm{2}}}} }  \vdash^{  \gamma _{ \refenvnt{k_{{\mathrm{1}}}} }   \refenvsym{,}   \overrightarrow{ \delta_{{\mathrm{3}}} }^{+}  }\token{wf} $.

    \item[\zcref{item:value-portability-code-aux1:type}.]
      By induction on
      $ \Psi \mid^{  \gamma _{ 0 }  }   \Gamma_{{\mathrm{1}}}  \refenvsym{,}  \Gamma_{{\mathrm{2}}} ^{ 0 , \refenvnt{k_{{\mathrm{2}}}} }  \vdash ^{  \gamma _{ \refenvnt{k_{{\mathrm{1}}}} }   \refenvsym{,}   \overrightarrow{ \delta_{{\mathrm{2}}} }^{+}  } \refenvnt{A} \ \token{wf} $.


    \item[\zcref{item:value-portability-code-aux1:exp}.]
      By induction on
      $ \Psi \mid^{  \gamma _{ 0 }  }   \Gamma_{{\mathrm{1}}}  \refenvsym{,}  \Gamma_{{\mathrm{2}}} ^{ 0 , \refenvnt{k_{{\mathrm{2}}}} }  \vdash^{  \gamma _{ \refenvnt{k_{{\mathrm{1}}}} }   \refenvsym{,}   \overrightarrow{ \delta_{{\mathrm{2}}} }^{+}  }_{  \token{id}  }   \refenvnt{e} ^{ \refenvnt{k_{{\mathrm{2}}}}  }  : \refenvnt{A} $.
      We cover major cases.

      \begin{description}
        \item[Case \textmd{\ref{rule:runtime-type-var}}:]
          By inversion of \ref{rule:runtime-type-var}, we have
          $ \refenvnt{e} ^{ \refenvnt{k_{{\mathrm{2}}}}  }  = \refenvmv{x}$,
          $ \overrightarrow{ \delta_{{\mathrm{2}}} }^{+}  =  \overrightarrow{ \delta_{{\mathrm{3}}} }   \refenvsym{,}  \delta_{{\mathrm{4}}}$,
          $\token{lookup} \, \refenvsym{(}  \refenvsym{(}   \Gamma_{{\mathrm{1}}}  \refenvsym{,}  \Gamma_{{\mathrm{2}}} ^{ 0 , \refenvnt{k_{{\mathrm{2}}}} }   \refenvsym{)}  \refenvsym{,}  \refenvmv{x}  \refenvsym{)} = \token{Done} \, \refenvsym{(}  \refenvnt{A}  \refenvsym{,}  \delta_{{\mathrm{5}}}  \refenvsym{)}$,
          \[
             \Psi \mid^{  \gamma _{ 0 }  }  \Gamma_{{\mathrm{1}}}  \refenvsym{,}  \Gamma_{{\mathrm{2}}} ^{ 0 , \refenvnt{k_{{\mathrm{2}}}} }  \vdash^{  \gamma _{ \refenvnt{k_{{\mathrm{1}}}} }   \refenvsym{,}   \overrightarrow{ \delta_{{\mathrm{3}}} }   \refenvsym{,}  \delta_{{\mathrm{4}}} }\token{wf} 
          \]
          and
          $ \Psi \mid^{  \gamma _{ 0 }  }  \Gamma_{{\mathrm{1}}}  \refenvsym{,}  \Gamma_{{\mathrm{2}}} ^{ 0 , \refenvnt{k_{{\mathrm{2}}}} }  \vdash \delta_{{\mathrm{5}}} \preceq \delta_{{\mathrm{4}}} $.
          By \zcref{claim:cls-upper-bound-wrt-gtrans-1}, either
          $\delta_{{\mathrm{4}}} \, \in \,  \token{Dom}_{C}(  \Gamma_{{\mathrm{2}}} ^{ 0 , \refenvnt{k_{{\mathrm{2}}}} }  ) $ or
          $ \Psi \mid^{  \gamma _{ 0 }  } \Gamma_{{\mathrm{1}}} \vdash \delta_{{\mathrm{4}}} \subseteq \delta_{{\mathrm{1}}} $.
          Hence, by \zcref{item:value-portability-code-aux1:ltrans},
          $ \Psi \mid^{ \gamma' }  \Gamma_{{\mathrm{1}}}  \refenvsym{,}  \Gamma_{{\mathrm{2}}} ^{ 0 , \refenvnt{k_{{\mathrm{2}}}} }  \vdash \delta_{{\mathrm{5}}} \preceq \delta_{{\mathrm{4}}} $.
          The required context well-formedness follows from the assumption
          $ \Psi \mid^{ \gamma' }   \Gamma_{{\mathrm{1}}}  \refenvsym{,}  \Gamma_{{\mathrm{2}}} ^{ 0 , \refenvnt{k_{{\mathrm{2}}}} }  \vdash ^{  \gamma _{ \refenvnt{k_{{\mathrm{1}}}} }   \refenvsym{[}   \gamma _{ 0 }   \coloneqq  \gamma'  \refenvsym{]}  \refenvsym{,}   \overrightarrow{ \delta_{{\mathrm{3}}} }   \refenvsym{,}  \delta_{{\mathrm{4}}} } \refenvnt{A} \ \token{wf} $.
          Therefore, by \ref{rule:runtime-type-var}, we obtain
          $ \Psi \mid^{ \gamma' }   \Gamma_{{\mathrm{1}}}  \refenvsym{,}  \Gamma_{{\mathrm{2}}} ^{ 0 , \refenvnt{k_{{\mathrm{2}}}} }  \vdash^{  \gamma _{ \refenvnt{k_{{\mathrm{1}}}} }   \refenvsym{[}   \gamma _{ 0 }   \coloneqq  \gamma'  \refenvsym{]}  \refenvsym{,}   \overrightarrow{ \delta_{{\mathrm{3}}} }   \refenvsym{,}  \delta_{{\mathrm{4}}} }_{  \token{id}  }  \refenvmv{x} : \refenvnt{A} $.

        \item[Case \textmd{\ref{rule:runtime-type-func}}:]
          By inversion of \ref{rule:runtime-type-func}, we have
          $ \refenvnt{e} ^{ \refenvnt{k_{{\mathrm{2}}}}  }  =   \lambda \binder{ \refenvmv{x} }.\  \refenvnt{e_{{\mathrm{1}}}}  ^{ \refenvnt{k_{{\mathrm{2}}}}  } $,
          $\refenvnt{A} = \refenvnt{A_{{\mathrm{1}}}}  \rightarrow  \refenvnt{A_{{\mathrm{2}}}}$, and
          $ \overrightarrow{ \delta_{{\mathrm{2}}} }^{+}  =  \overrightarrow{ \delta_{{\mathrm{3}}} }   \refenvsym{,}  \delta_{{\mathrm{4}}}$.
          The derivation gives
          \[
             \Psi \mid^{  \gamma _{ 0 }  }   \Gamma_{{\mathrm{1}}}  \refenvsym{,}  \Gamma_{{\mathrm{2}}} ^{ 0 , \refenvnt{k_{{\mathrm{2}}}} }   \refenvsym{,}   \binder{ \refenvmv{x} }\mathord{:^{\binder{ \delta_{{\mathrm{5}}} } } } \refenvnt{A_{{\mathrm{1}}}}  \vdash^{  \gamma _{ \refenvnt{k_{{\mathrm{1}}}} }   \refenvsym{,}   \overrightarrow{ \delta_{{\mathrm{3}}} }   \refenvsym{,}  \delta_{{\mathrm{5}}} }_{  \token{id}  }   \refenvnt{e_{{\mathrm{1}}}} ^{ \refenvnt{k_{{\mathrm{2}}}}  }  : \refenvnt{A_{{\mathrm{2}}}} 
          \]
          together with
          $\delta_{{\mathrm{5}}} \, \not\in \,  \token{FC}( \refenvnt{A_{{\mathrm{2}}}} ) $ and
          $ \Psi \mid^{  \gamma _{ 0 }  }  \Gamma_{{\mathrm{1}}}  \refenvsym{,}  \Gamma_{{\mathrm{2}}} ^{ 0 , \refenvnt{k_{{\mathrm{2}}}} }  \vdash^{  \gamma _{ \refenvnt{k_{{\mathrm{1}}}} }   \refenvsym{,}   \overrightarrow{ \delta_{{\mathrm{3}}} }   \refenvsym{,}  \delta_{{\mathrm{4}}} }\token{wf} $.
          By the induction hypothesis applied to the body derivation, we have
          \[
             \Psi \mid^{ \gamma' }   \Gamma_{{\mathrm{1}}}  \refenvsym{,}  \Gamma_{{\mathrm{2}}} ^{ 0 , \refenvnt{k_{{\mathrm{2}}}} }   \refenvsym{,}   \binder{ \refenvmv{x} }\mathord{:^{\binder{ \delta_{{\mathrm{5}}} } } } \refenvnt{A_{{\mathrm{1}}}}  \vdash^{  \gamma _{ \refenvnt{k_{{\mathrm{1}}}} }   \refenvsym{[}   \gamma _{ 0 }   \coloneqq  \gamma'  \refenvsym{]}  \refenvsym{,}   \overrightarrow{ \delta_{{\mathrm{3}}} }   \refenvsym{,}  \delta_{{\mathrm{5}}} }_{  \token{id}  }   \refenvnt{e_{{\mathrm{1}}}} ^{ \refenvnt{k_{{\mathrm{2}}}}  }  : \refenvnt{A_{{\mathrm{2}}}} .
          \]
          From the assumption
          $ \Psi \mid^{ \gamma' }   \Gamma_{{\mathrm{1}}}  \refenvsym{,}  \Gamma_{{\mathrm{2}}} ^{ 0 , \refenvnt{k_{{\mathrm{2}}}} }  \vdash ^{  \gamma _{ \refenvnt{k_{{\mathrm{1}}}} }   \refenvsym{[}   \gamma _{ 0 }   \coloneqq  \gamma'  \refenvsym{]}  \refenvsym{,}   \overrightarrow{ \delta_{{\mathrm{3}}} }   \refenvsym{,}  \delta_{{\mathrm{4}}} } \refenvnt{A_{{\mathrm{1}}}}  \rightarrow  \refenvnt{A_{{\mathrm{2}}}} \ \token{wf} $,
          inversion gives the well-formedness premises needed for reapplying
          \ref{rule:runtime-type-func}.  The freshness premise required by
          \ref{rule:runtime-type-func} is the same as in the original
          derivation, namely $\delta_{{\mathrm{5}}} \, \not\in \,  \token{FC}( \refenvnt{A_{{\mathrm{2}}}} ) $.
          Therefore, by \ref{rule:runtime-type-func}, we obtain
          \[
             \Psi \mid^{ \gamma' }   \Gamma_{{\mathrm{1}}}  \refenvsym{,}  \Gamma_{{\mathrm{2}}} ^{ 0 , \refenvnt{k_{{\mathrm{2}}}} }  \vdash^{  \gamma _{ \refenvnt{k_{{\mathrm{1}}}} }   \refenvsym{[}   \gamma _{ 0 }   \coloneqq  \gamma'  \refenvsym{]}  \refenvsym{,}   \overrightarrow{ \delta_{{\mathrm{3}}} }   \refenvsym{,}  \delta_{{\mathrm{4}}} }_{  \token{id}  }    \lambda \binder{ \refenvmv{x} }.\  \refenvnt{e_{{\mathrm{1}}}}  ^{ \refenvnt{k_{{\mathrm{2}}}}  }  : \refenvnt{A_{{\mathrm{1}}}}  \rightarrow  \refenvnt{A_{{\mathrm{2}}}} .
          \]
      \end{description}
  \end{description}
\end{proof}

\begin{lemma}[Value Portability]\label{claim:value-portability}
  If\/ $ \Psi \mid \Theta \vdash^{ \gamma_{{\mathrm{1}}} } \refenvnt{v} : \refenvnt{A} \ \token{val} $, then for any $\gamma_{{\mathrm{2}}}$ such that $ \Psi  \vdash^{ \gamma_{{\mathrm{2}}} }  \refenvnt{A} \ \token{wf} $, we have $ \Psi \mid \Theta \vdash^{ \gamma_{{\mathrm{2}}} } \refenvnt{v} : \refenvnt{A} \ \token{val} $.
\end{lemma}

\begin{proof}
  We proceed by case analysis on the derivation of
  $ \Psi \mid \Theta \vdash^{ \gamma_{{\mathrm{1}}} } \refenvnt{v} : \refenvnt{A} \ \token{val} $.

  \begin{description}
    \item[Case \textmd{\ref{rule:value-type-int}}:] Trivial.

    \item[Case \textmd{\ref{rule:value-type-clos-func}}:]
      By inversion of \ref{rule:value-type-clos-func}, we have
      $\refenvnt{v} = \token{clos} \, \refenvsym{(}  E  \refenvsym{,}  R  \refenvsym{,}    \lambda \binder{ \refenvmv{x} }.\  \refenvnt{e}  ^{ 0  }   \refenvsym{)}$ and
      $\refenvnt{A} =  \forall   \varrho _{ 1 }  \dotsc\forall  \varrho _{ \refenvnt{k} }  . \refenvnt{A_{{\mathrm{1}}}}  \rightarrow  \refenvnt{A_{{\mathrm{2}}}} $.
      Moreover, the derivation gives
      \[
         \Psi \mid^{  \delta _{ 0 }  }  \varepsilon \vdash^{  \delta _{ 0 }  }_{ R }    \lambda \binder{ \refenvmv{x} }.\  \refenvnt{e}  ^{ 0  }  :  \forall   \varrho _{ 1 }  \dotsc\forall  \varrho _{ \refenvnt{k} }  . \refenvnt{A_{{\mathrm{1}}}}  \rightarrow  \refenvnt{A_{{\mathrm{2}}}}  
      \]
      together with $ \Psi \mid \Theta \vdash^{  \delta _{ 0 }  } E \ \token{wf} $.
      The assumption of the lemma gives
      $ \Psi  \vdash^{ \gamma_{{\mathrm{2}}} }   \forall   \varrho _{ 1 }  \dotsc\forall  \varrho _{ \refenvnt{k} }  . \refenvnt{A_{{\mathrm{1}}}}  \rightarrow  \refenvnt{A_{{\mathrm{2}}}}  \ \token{wf} $.
      Therefore, by reapplying \ref{rule:value-type-clos-func} using this
      well-formedness premise, we obtain
      $ \Psi \mid \Theta \vdash^{ \gamma_{{\mathrm{2}}} } \refenvnt{v} : \refenvnt{A} \ \token{val} $.

    \item[Case \textmd{\ref{rule:value-type-clos-rec}}:]
      This case is analogous to the previous one.

    \item[Case \textmd{\ref{rule:value-type-code}}:]
      By inversion of \ref{rule:value-type-code}, we have
      $\refenvnt{v} =  \langle   \refenvnt{e} ^{ 0  }   \rangle $ and
      $\refenvnt{A} =
       \forall   \varrho _{ 1 }  \dotsc\forall  \varrho _{ \refenvnt{k} }  .  \langle \refenvnt{A_{{\mathrm{1}}}} \rangle^{ \delta' }  $.
      Moreover, the derivation gives
      \[
         \Psi \mid^{ \gamma_{{\mathrm{1}}} }  \varepsilon \vdash^{ \gamma_{{\mathrm{1}}} }_{  \token{id}  }   \langle   \refenvnt{e} ^{ 0  }   \rangle  :  \forall   \varrho _{ 1 }  \dotsc\forall  \varrho _{ \refenvnt{k} }  .  \langle \refenvnt{A_{{\mathrm{1}}}} \rangle^{ \delta' }   
      \]
      together with $ \Psi  \vdash  \Theta \ \token{wf} $.
      By inverting this typing derivation, for some classifiers
      $ \delta _{ 0 } $ to $ \delta _{ \refenvnt{k} } $ with $ \delta _{ 0 }  = \gamma_{{\mathrm{1}}}$, we have
      \[
         \Psi \mid^{  \delta _{ 0 }  }    [   \varrho _{ 1 }   ]^{\binder{  \delta _{ 1 }  } }  ,\dotsc,  [   \varrho _{ \refenvnt{k} }   ]^{\binder{  \delta _{ \refenvnt{k} }  } }    \refenvsym{,}   \blacktriangleright ^{ \delta' }  \vdash^{  \delta _{ \refenvnt{k} }   \refenvsym{,}  \delta' }_{  \token{id}  }   \refenvnt{e} ^{ 0  }  : \refenvnt{A_{{\mathrm{1}}}} 
      \]
      and the side conditions on the classifier declarations, namely
      $ \delta _{ \refenvnt{i} }  \not\in
       \token{FC}(  \varrho _{ \refenvnt{i}  \refenvsym{+}  1 }  )  \cup \dotsb \cup  \token{FC}(  \varrho _{ \refenvnt{k} }  )  \cup
       \token{FC}( \refenvnt{A_{{\mathrm{1}}}} )  \cup \refenvsym{\{}  \delta'  \refenvsym{\}}$ for $1 \le \refenvnt{i} \le \refenvnt{k}$.
      From the assumption
      $ \Psi  \vdash^{ \gamma_{{\mathrm{2}}} }   \forall   \varrho _{ 1 }  \dotsc\forall  \varrho _{ \refenvnt{k} }  .  \langle \refenvnt{A_{{\mathrm{1}}}} \rangle^{ \delta' }   \ \token{wf} $,
      inversion gives
      $ \Psi \mid^{ \gamma_{{\mathrm{2}}} }    [   \varrho _{ 1 }   ]^{\binder{  \delta _{ 1 }  } }  ,\dotsc,  [   \varrho _{ \refenvnt{k} }   ]^{\binder{  \delta _{ \refenvnt{k} }  } }    \refenvsym{,}   \blacktriangleright ^{ \delta' }  \vdash ^{  \delta _{ \refenvnt{k} }   \refenvsym{[}   \delta _{ 0 }   \coloneqq  \gamma_{{\mathrm{2}}}  \refenvsym{]}  \refenvsym{,}  \delta' } \refenvnt{A_{{\mathrm{1}}}} \ \token{wf} $.
      Hence, by \zcref{claim:value-portability-code-aux1},
      \[
         \Psi \mid^{ \gamma_{{\mathrm{2}}} }    [   \varrho _{ 1 }   ]^{\binder{  \delta _{ 1 }  } }  ,\dotsc,  [   \varrho _{ \refenvnt{k} }   ]^{\binder{  \delta _{ \refenvnt{k} }  } }    \refenvsym{,}   \blacktriangleright ^{ \delta' }  \vdash^{  \delta _{ \refenvnt{k} }   \refenvsym{[}   \delta _{ 0 }   \coloneqq  \gamma_{{\mathrm{2}}}  \refenvsym{]}  \refenvsym{,}  \delta' }_{  \token{id}  }   \refenvnt{e} ^{ 0  }  : \refenvnt{A_{{\mathrm{1}}}} .
      \]
      By reapplying \ref{rule:runtime-type-quote} and
      \ref{rule:runtime-type-polycls}, we obtain
      \[
         \Psi \mid^{ \gamma_{{\mathrm{2}}} }  \varepsilon \vdash^{ \gamma_{{\mathrm{2}}} }_{  \token{id}  }   \langle   \refenvnt{e} ^{ 0  }   \rangle  :  \forall   \varrho _{ 1 }  \dotsc\forall  \varrho _{ \refenvnt{k} }  .  \langle \refenvnt{A_{{\mathrm{1}}}} \rangle^{ \delta' }   .
      \]
      Therefore, by reapplying \ref{rule:value-type-code}, we obtain
      $ \Psi \mid \Theta \vdash^{ \gamma_{{\mathrm{2}}} } \refenvnt{v} : \refenvnt{A} \ \token{val} $.

    \item[Case \textmd{\ref{rule:value-type-loc}}:]
      By inversion of \ref{rule:value-type-loc}, we have
      $\refenvnt{v} = \refenvmv{l}$ and $\refenvnt{A} =  \refenvnt{A_{{\mathrm{1}}}} \/\ \token{ref} $, together with
      $ \Psi  \vdash  \Theta \ \token{wf} $,
      $\token{lookupStore}  \refenvsym{(}  \Theta  \refenvsym{,}  \refenvmv{l}  \refenvsym{)} = \token{Done} \, \refenvsym{(}  \refenvnt{A_{{\mathrm{1}}}}  \refenvsym{)}$, and
      $ \Psi  \vdash^{ \gamma_{{\mathrm{1}}} }  \refenvnt{A_{{\mathrm{1}}}} \ \token{wf} $.
      From the assumption $ \Psi  \vdash^{ \gamma_{{\mathrm{2}}} }   \refenvnt{A_{{\mathrm{1}}}} \/\ \token{ref}  \ \token{wf} $, inversion of
      \ref{rule:runtime-wf-t-ref} gives $ \Psi  \vdash^{ \gamma_{{\mathrm{2}}} }  \refenvnt{A_{{\mathrm{1}}}} \ \token{wf} $.
      Therefore, by reapplying \ref{rule:value-type-loc}, we obtain
      $ \Psi \mid \Theta \vdash^{ \gamma_{{\mathrm{2}}} } \refenvmv{l} :  \refenvnt{A_{{\mathrm{1}}}} \/\ \token{ref}  \ \token{val} $.
  \end{description}
\end{proof}

\begin{lemma}[Classifier Application for Values]\label{claim:value-appcls}
  Suppose that
  \begin{enumerate}
    \item $ \Psi_{{\mathrm{1}}} \mid \Theta \vdash^{  \delta _{ 0 }  } \refenvnt{v} :  \forall    \binder{  \gamma _{ 1 }  }  \mathbin{:\succeq}    \gamma' _{ 1 }  ,\dotsc,\binder{  \gamma _{ \refenvnt{k_{{\mathrm{1}}}} }  }  \mathbin{:\succeq}   \gamma'  _{ \refenvnt{k_{{\mathrm{1}}}} }  . \refenvnt{A}  \ \token{val} $,
    \item $\Psi_{{\mathrm{1}}}  \vdash   \gamma' _{ \refenvnt{i} }   \preceq   \delta _{ \refenvnt{i} } $ for each $\refenvnt{i}$ with $1 \le \refenvnt{i} \le \refenvnt{k_{{\mathrm{1}}}}$, and
    \item $\Psi_{{\mathrm{1}}}  \vdash   \delta _{ \refenvnt{i}  \refenvsym{+}  1 }   \subseteq   \delta _{ \refenvnt{i} } $ for each $\refenvnt{i}$ with $0 \le \refenvnt{i} < \refenvnt{k_{{\mathrm{1}}}}$.
  \end{enumerate}
  Then there exists $\Psi_{{\mathrm{2}}}$ such that $ \Psi_{{\mathrm{1}}} \subseteq \Psi_{{\mathrm{2}}} $, $ \token{Dom}_{V}( \Psi_{{\mathrm{2}}} )  =  \token{Dom}_{V}( \Psi_{{\mathrm{1}}} ) $, and
  \[
     \Psi_{{\mathrm{2}}} \mid \Theta \vdash^{  \delta _{ 0 }  } \refenvnt{v} : \refenvnt{A}  \refenvsym{[}    \gamma _{ 1 }  \coloneqq  \delta _{ 1 }  ,\dotsc,  \gamma _{ \refenvnt{k_{{\mathrm{1}}}} }  \coloneqq  \delta _{ \refenvnt{k_{{\mathrm{1}}}} }    \refenvsym{]} \ \token{val} .
  \]
\end{lemma}

\begin{proof}
  We proceed by inversion on
  $ \Psi_{{\mathrm{1}}} \mid \Theta \vdash^{  \delta _{ 0 }  } \refenvnt{v} :  \forall    \binder{  \gamma _{ 1 }  }  \mathbin{:\succeq}    \gamma' _{ 1 }  ,\dotsc,\binder{  \gamma _{ \refenvnt{k_{{\mathrm{1}}}} }  }  \mathbin{:\succeq}   \gamma'  _{ \refenvnt{k_{{\mathrm{1}}}} }  . \refenvnt{A}  \ \token{val} $.
  The only possible cases are the closure cases and the code case.
  In each case, we instantiate the typing premise for the underlying
  constructor by \ref{rule:runtime-type-appcls}, and then reapply the
  corresponding value typing rule.

  \begin{description}
    \item[Case \textmd{\ref{rule:value-type-clos-func}}:]
      By inversion, we have
      $\refenvnt{v} = \token{clos} \, \refenvsym{(}  E  \refenvsym{,}  R  \refenvsym{,}    \lambda \binder{ \refenvmv{x} }.\  \refenvnt{e}  ^{ 0  }   \refenvsym{)}$ and
      $\refenvnt{A} =  \forall   \varrho _{ 1 }  \dotsc\forall  \varrho _{ \refenvnt{k_{{\mathrm{2}}}} }  . \refenvnt{A_{{\mathrm{1}}}}  \rightarrow  \refenvnt{A_{{\mathrm{2}}}} $.
      Moreover, the derivation gives
      \[
         \Psi_{{\mathrm{1}}} \mid^{  \gamma' _{ 0 }  }  \varepsilon \vdash^{  \gamma' _{ 0 }  }_{ R }    \lambda \binder{ \refenvmv{x} }.\  \refenvnt{e}  ^{ 0  }  :  \forall    \binder{  \gamma _{ 1 }  }  \mathbin{:\succeq}    \gamma' _{ 1 }  ,\dotsc,\binder{  \gamma _{ \refenvnt{k_{{\mathrm{1}}}} }  }  \mathbin{:\succeq}   \gamma'  _{ \refenvnt{k_{{\mathrm{1}}}} }  . \refenvnt{A}  ,
      \]
      together with $ \Psi_{{\mathrm{1}}} \mid \Theta \vdash^{  \gamma' _{ 0 }  } E \ \token{wf} $.

      Choose a fresh classifier $\delta''$ and let
      $\Psi_{{\mathrm{2}}} = \Psi_{{\mathrm{1}}}  \refenvsym{,}   \binder{ \delta'' }( \mathbin{:\succeq} \;  \gamma' _{ 0 }   /  \mathbin{:\supseteq} \;  \delta _{ 1 }  ) $.
      Then $ \Psi_{{\mathrm{1}}} \subseteq \Psi_{{\mathrm{2}}} $ and
      $ \token{Dom}_{V}( \Psi_{{\mathrm{2}}} )  =  \token{Dom}_{V}( \Psi_{{\mathrm{1}}} ) $.  Moreover, by
      \zcref{claim:nht-weakening} we obtain
      \[
         \Psi_{{\mathrm{2}}} \mid^{  \gamma' _{ 0 }  }  \varepsilon \vdash^{  \gamma' _{ 0 }  }_{ R }    \lambda \binder{ \refenvmv{x} }.\  \refenvnt{e}  ^{ 0  }  :  \forall    \binder{  \gamma _{ 1 }  }  \mathbin{:\succeq}    \gamma' _{ 1 }  ,\dotsc,\binder{  \gamma _{ \refenvnt{k_{{\mathrm{1}}}} }  }  \mathbin{:\succeq}   \gamma'  _{ \refenvnt{k_{{\mathrm{1}}}} }  . \refenvnt{A}  .
      \]
      Since $\Psi_{{\mathrm{2}}}  \vdash   \gamma' _{ 0 }   \preceq  \delta''$, \zcref{claim:nht-monotonicity}
      gives
      \[
         \Psi_{{\mathrm{2}}} \mid^{ \delta'' }  \varepsilon \vdash^{ \delta'' }_{ R }    \lambda \binder{ \refenvmv{x} }.\  \refenvnt{e}  ^{ 0  }  :  \forall    \binder{  \gamma _{ 1 }  }  \mathbin{:\succeq}    \gamma' _{ 1 }  ,\dotsc,\binder{  \gamma _{ \refenvnt{k_{{\mathrm{1}}}} }  }  \mathbin{:\succeq}   \gamma'  _{ \refenvnt{k_{{\mathrm{1}}}} }  . \refenvnt{A}  .
      \]
      The classifier sequence $\delta'',  \delta _{ 1 } , \dotsc,  \delta _{ \refenvnt{k_{{\mathrm{1}}}} } $
      satisfies the premises of \ref{rule:runtime-type-appcls}: the first
      reachability premise follows from the declaration of $\Psi_{{\mathrm{2}}}$, and
      the remaining premises follow by \zcref{claim:nht-weakening} from the
      assumptions of the lemma.  Hence, writing
      $\sigma =   \gamma _{ 1 }  \coloneqq  \delta _{ 1 }  ,\dotsc,  \gamma _{ \refenvnt{k_{{\mathrm{1}}}} }  \coloneqq  \delta _{ \refenvnt{k_{{\mathrm{1}}}} }  $, we obtain
      \[
         \Psi_{{\mathrm{2}}} \mid^{ \delta'' }  \varepsilon \vdash^{ \delta'' }_{ R }    \lambda \binder{ \refenvmv{x} }.\  \refenvnt{e}  ^{ 0  }  : \refenvnt{A}  \refenvsym{[}  \sigma  \refenvsym{]} .
      \]

      Moreover, $ \Psi_{{\mathrm{2}}} \mid \Theta \vdash^{ \delta'' } E \ \token{wf} $ follows by
      \ref{rule:runtime-wf-venv-name-cls}.

      By inversion of the
      well-formedness premise in the original value typing derivation, we have
      \[
         \Psi_{{\mathrm{1}}} \mid^{  \gamma' _{ 0 }  }   [    \binder{  \gamma _{ 1 }  }  \mathbin{:\succeq}    \gamma' _{ 1 }  ,\dotsc,\binder{  \gamma _{ \refenvnt{k_{{\mathrm{1}}}} }  }  \mathbin{:\succeq}   \gamma'  _{ \refenvnt{k_{{\mathrm{1}}}} }   ]^{\binder{  \gamma _{ 0 }  } }  \vdash ^{  \gamma _{ 0 }  } \refenvnt{A} \ \token{wf} .
      \]
      Weakening this judgment to $\Psi_{{\mathrm{2}}}$ and applying
      \zcref{claim:polyclsdecl-substitution} yields
      $ \Psi_{{\mathrm{2}}}  \vdash^{  \delta _{ 0 }  }  \refenvnt{A}  \refenvsym{[}  \sigma  \refenvsym{]} \ \token{wf} $.

      Therefore, by reapplying \ref{rule:value-type-clos-func},
      we obtain $ \Psi_{{\mathrm{2}}} \mid \Theta \vdash^{  \delta _{ 0 }  } \refenvnt{v} : \refenvnt{A}  \refenvsym{[}  \sigma  \refenvsym{]} \ \token{val} $.

    \item[Case \textmd{\ref{rule:value-type-clos-rec}}:]
      This case is analogous to the previous one, using
      \ref{rule:value-type-clos-rec} instead of \ref{rule:value-type-clos-func}.

    \item[Case \textmd{\ref{rule:value-type-code}}:]
      By inversion, we have
      $\refenvnt{v} =  \langle   \refenvnt{e} ^{ 0  }   \rangle $ and
      $\refenvnt{A} =  \forall   \varrho _{ 1 }  \dotsc\forall  \varrho _{ \refenvnt{k_{{\mathrm{2}}}} }  .  \langle \refenvnt{A_{{\mathrm{1}}}} \rangle^{ \delta' }  $.
      The derivation gives
      \[
         \Psi_{{\mathrm{1}}} \mid^{  \delta _{ 0 }  }  \varepsilon \vdash^{  \delta _{ 0 }  }_{  \token{id}  }   \langle   \refenvnt{e} ^{ 0  }   \rangle  :  \forall    \binder{  \gamma _{ 1 }  }  \mathbin{:\succeq}    \gamma' _{ 1 }  ,\dotsc,\binder{  \gamma _{ \refenvnt{k_{{\mathrm{1}}}} }  }  \mathbin{:\succeq}   \gamma'  _{ \refenvnt{k_{{\mathrm{1}}}} }  . \refenvnt{A}  
      \]
      together with $ \Psi_{{\mathrm{1}}}  \vdash  \Theta \ \token{wf} $.
      By \ref{rule:runtime-type-appcls} and the assumptions of the lemma, we
      obtain
      \[
         \Psi_{{\mathrm{1}}} \mid^{  \delta _{ 0 }  }  \varepsilon \vdash^{  \delta _{ 0 }  }_{  \token{id}  }   \langle   \refenvnt{e} ^{ 0  }   \rangle  : \refenvnt{A}  \refenvsym{[}    \gamma _{ 1 }  \coloneqq  \delta _{ 1 }  ,\dotsc,  \gamma _{ \refenvnt{k_{{\mathrm{1}}}} }  \coloneqq  \delta _{ \refenvnt{k_{{\mathrm{1}}}} }    \refenvsym{]} .
      \]
      Let $\Psi_{{\mathrm{2}}} = \Psi_{{\mathrm{1}}}$.
      Then $ \Psi_{{\mathrm{1}}} \subseteq \Psi_{{\mathrm{2}}} $ and
      $ \token{Dom}_{V}( \Psi_{{\mathrm{2}}} )  =  \token{Dom}_{V}( \Psi_{{\mathrm{1}}} ) $.
      Therefore, by reapplying \ref{rule:value-type-code}, we obtain
      $ \Psi_{{\mathrm{2}}} \mid \Theta \vdash^{  \delta _{ 0 }  } \refenvnt{v} : \refenvnt{A}  \refenvsym{[}    \gamma _{ 1 }  \coloneqq  \delta _{ 1 }  ,\dotsc,  \gamma _{ \refenvnt{k_{{\mathrm{1}}}} }  \coloneqq  \delta _{ \refenvnt{k_{{\mathrm{1}}}} }    \refenvsym{]} \ \token{val} $.
  \end{description}
\end{proof}


\subsection{Promotion Lemma}
\begin{lemma}[Promotion for $ \blacktriangleright $]\label{claim:promotion-open}
  \begin{enumerate}
    \item \label{item:promotion-open:ctxwf}
          If\/ $ \Psi \mid^{  \overrightarrow{ \gamma_{{\mathrm{1}}} }^{+}  }  \blacktriangleright ^{ \gamma_{{\mathrm{2}}} }   \refenvsym{,}  \Gamma \vdash^{  \overrightarrow{ \gamma_{{\mathrm{3}}} }^{+}  }\token{wf} $,
          then $ \Psi \mid^{  \overrightarrow{ \gamma_{{\mathrm{1}}} }^{+}   \refenvsym{,}  \gamma_{{\mathrm{2}}} } \Gamma \vdash^{  \overrightarrow{ \gamma_{{\mathrm{3}}} }^{+}  }\token{wf} $.
    \item \label{item:promotion-open:typwf}
          If\/ $ \Psi \mid^{  \overrightarrow{ \gamma_{{\mathrm{1}}} }^{+}  }   \blacktriangleright ^{ \gamma_{{\mathrm{2}}} }   \refenvsym{,}  \Gamma \vdash ^{  \overrightarrow{ \gamma_{{\mathrm{3}}} }^{+}  } \refenvnt{A} \ \token{wf} $,
          then $ \Psi \mid^{  \overrightarrow{ \gamma_{{\mathrm{1}}} }^{+}   \refenvsym{,}  \gamma_{{\mathrm{2}}} }  \Gamma \vdash ^{  \overrightarrow{ \gamma_{{\mathrm{3}}} }^{+}  } \refenvnt{A} \ \token{wf} $.
    \item \label{item:promotion-open:ltrans}
          If\/ $ \Psi \mid^{  \overrightarrow{ \gamma_{{\mathrm{1}}} }^{+}  }  \blacktriangleright ^{ \gamma_{{\mathrm{2}}} }   \refenvsym{,}  \Gamma \vdash \gamma_{{\mathrm{3}}} \preceq \gamma_{{\mathrm{4}}} $,
          then $ \Psi \mid^{  \overrightarrow{ \gamma_{{\mathrm{1}}} }^{+}   \refenvsym{,}  \gamma_{{\mathrm{2}}} } \Gamma \vdash \gamma_{{\mathrm{3}}} \preceq \gamma_{{\mathrm{4}}} $.
    \item \label{item:promotion-open:gtrans}
          If\/ $ \Psi \mid^{  \overrightarrow{ \gamma_{{\mathrm{1}}} }^{+}  }  \blacktriangleright ^{ \gamma_{{\mathrm{2}}} }   \refenvsym{,}  \Gamma \vdash \gamma_{{\mathrm{3}}} \subseteq \gamma_{{\mathrm{4}}} $,
          then $ \Psi \mid^{  \overrightarrow{ \gamma_{{\mathrm{1}}} }^{+}   \refenvsym{,}  \gamma_{{\mathrm{2}}} } \Gamma \vdash \gamma_{{\mathrm{3}}} \subseteq \gamma_{{\mathrm{4}}} $.
    \item \label{item:promotion-open:typing}
          If\/ $ \Psi \mid^{  \overrightarrow{ \gamma_{{\mathrm{1}}} }^{+}  }   \blacktriangleright ^{ \gamma_{{\mathrm{2}}} }   \refenvsym{,}  \Gamma \vdash^{  \overrightarrow{ \gamma_{{\mathrm{3}}} }^{+}  }_{ R }  \refenvnt{e} : \refenvnt{A} $,
          then $ \Psi \mid^{  \overrightarrow{ \gamma_{{\mathrm{1}}} }^{+}   \refenvsym{,}  \gamma_{{\mathrm{2}}} }  \Gamma \vdash^{  \overrightarrow{ \gamma_{{\mathrm{3}}} }^{+}  }_{ R }  \refenvnt{e} : \refenvnt{A} $.
  \end{enumerate}
\end{lemma}

\begin{proof}
  By mutual induction on the given derivation.
\end{proof}

\begin{lemma}[Promotion for $ \blacktriangleleft $]\label{claim:promotion-shut}
  \begin{enumerate}
    \item \label{item:promotion-shut:ctxwf}
          If\/ $ \Psi \mid^{  \overrightarrow{ \gamma_{{\mathrm{1}}} }   \refenvsym{,}    \delta _{ 0 }  ,\dotsc,  \delta _{ \refenvnt{k} }   }  \blacktriangleleft _{ \refenvnt{k} }^{\binder{ \gamma_{{\mathrm{2}}} } }   \refenvsym{,}  \Gamma \vdash^{  \overrightarrow{ \gamma_{{\mathrm{3}}} }^{+}  }\token{wf} $,
          then $ \Psi  \refenvsym{,}   \binder{ \gamma_{{\mathrm{2}}} }( \mathbin{:\succeq} \;  \delta _{ 0 }   /  \mathbin{:\supseteq} \;  \delta _{ \refenvnt{k} }  )  \mid^{  \overrightarrow{ \gamma_{{\mathrm{1}}} }   \refenvsym{,}  \gamma_{{\mathrm{2}}} } \Gamma \vdash^{  \overrightarrow{ \gamma_{{\mathrm{3}}} }^{+}  }\token{wf} $.
    \item \label{item:promotion-shut:typwf}
          If\/ $ \Psi \mid^{  \overrightarrow{ \gamma_{{\mathrm{1}}} }   \refenvsym{,}    \delta _{ 0 }  ,\dotsc,  \delta _{ \refenvnt{k} }   }   \blacktriangleleft _{ \refenvnt{k} }^{\binder{ \gamma_{{\mathrm{2}}} } }   \refenvsym{,}  \Gamma \vdash ^{  \overrightarrow{ \gamma_{{\mathrm{3}}} }^{+}  } \refenvnt{A} \ \token{wf} $,
          then $ \Psi  \refenvsym{,}   \binder{ \gamma_{{\mathrm{2}}} }( \mathbin{:\succeq} \;  \delta _{ 0 }   /  \mathbin{:\supseteq} \;  \delta _{ \refenvnt{k} }  )  \mid^{  \overrightarrow{ \gamma_{{\mathrm{1}}} }   \refenvsym{,}  \gamma_{{\mathrm{2}}} }  \Gamma \vdash ^{  \overrightarrow{ \gamma_{{\mathrm{3}}} }^{+}  } \refenvnt{A} \ \token{wf} $.
    \item \label{item:promotion-shut:ltrans}
          If\/ $ \Psi \mid^{  \overrightarrow{ \gamma_{{\mathrm{1}}} }   \refenvsym{,}    \delta _{ 0 }  ,\dotsc,  \delta _{ \refenvnt{k} }   }  \blacktriangleleft _{ \refenvnt{k} }^{\binder{ \gamma_{{\mathrm{2}}} } }   \refenvsym{,}  \Gamma \vdash \gamma_{{\mathrm{3}}} \preceq \gamma_{{\mathrm{4}}} $,
          then $ \Psi  \refenvsym{,}   \binder{ \gamma_{{\mathrm{2}}} }( \mathbin{:\succeq} \;  \delta _{ 0 }   /  \mathbin{:\supseteq} \;  \delta _{ \refenvnt{k} }  )  \mid^{  \overrightarrow{ \gamma_{{\mathrm{1}}} }   \refenvsym{,}  \gamma_{{\mathrm{2}}} } \Gamma \vdash \gamma_{{\mathrm{3}}} \preceq \gamma_{{\mathrm{4}}} $.
    \item \label{item:promotion-shut:gtrans}
          If\/ $ \Psi \mid^{  \overrightarrow{ \gamma_{{\mathrm{1}}} }   \refenvsym{,}    \delta _{ 0 }  ,\dotsc,  \delta _{ \refenvnt{k} }   }  \blacktriangleleft _{ \refenvnt{k} }^{\binder{ \gamma_{{\mathrm{2}}} } }   \refenvsym{,}  \Gamma \vdash \gamma_{{\mathrm{3}}} \subseteq \gamma_{{\mathrm{4}}} $,
          then $ \Psi  \refenvsym{,}   \binder{ \gamma_{{\mathrm{2}}} }( \mathbin{:\succeq} \;  \delta _{ 0 }   /  \mathbin{:\supseteq} \;  \delta _{ \refenvnt{k} }  )  \mid^{  \overrightarrow{ \gamma_{{\mathrm{1}}} }   \refenvsym{,}  \gamma_{{\mathrm{2}}} } \Gamma \vdash \gamma_{{\mathrm{3}}} \subseteq \gamma_{{\mathrm{4}}} $.
    \item \label{item:promotion-shut:typing}
          If\/ $ \Psi \mid^{  \overrightarrow{ \gamma_{{\mathrm{1}}} }   \refenvsym{,}    \delta _{ 0 }  ,\dotsc,  \delta _{ \refenvnt{k} }   }   \blacktriangleleft _{ \refenvnt{k} }^{\binder{ \gamma_{{\mathrm{2}}} } }   \refenvsym{,}  \Gamma \vdash^{  \overrightarrow{ \gamma_{{\mathrm{3}}} }^{+}  }_{ R }  \refenvnt{e} : \refenvnt{A} $,
          then $ \Psi  \refenvsym{,}   \binder{ \gamma_{{\mathrm{2}}} }( \mathbin{:\succeq} \;  \delta _{ 0 }   /  \mathbin{:\supseteq} \;  \delta _{ \refenvnt{k} }  )  \mid^{  \overrightarrow{ \gamma_{{\mathrm{1}}} }   \refenvsym{,}  \gamma_{{\mathrm{2}}} }  \Gamma \vdash^{  \overrightarrow{ \gamma_{{\mathrm{3}}} }^{+}  }_{ R }  \refenvnt{e} : \refenvnt{A} $.
  \end{enumerate}
\end{lemma}

\begin{proof}
  By mutual induction on the given derivation.
\end{proof}

\begin{lemma}[Promotion for Variables]\label{claim:promotion-var}
  Suppose $\refenvmv{y} \, \not\in \,  \token{Dom}_{V}( \Psi ) $.
  \begin{enumerate}
    \item \label{item:promotion-var:ctxwf}
          If\/ $ \Psi \mid^{  \overrightarrow{ \gamma_{{\mathrm{1}}} }   \refenvsym{,}  \gamma_{{\mathrm{2}}} }  \binder{ \refenvmv{x} }\mathord{:^{\binder{ \gamma_{{\mathrm{3}}} } } } \refenvnt{A_{{\mathrm{1}}}}   \refenvsym{,}  \Gamma \vdash^{  \overrightarrow{ \gamma_{{\mathrm{4}}} }^{+}  }\token{wf} $,
          then $ \Psi  \refenvsym{,}   \binder{ \refenvmv{y} }: \refenvnt{A_{{\mathrm{1}}}} \mathrel{@}\binder{ \gamma_{{\mathrm{3}}} } \mathbin{:\succeq} \gamma_{{\mathrm{2}}}  \mid^{  \overrightarrow{ \gamma_{{\mathrm{1}}} }   \refenvsym{,}  \gamma_{{\mathrm{3}}} } \Gamma \vdash^{  \overrightarrow{ \gamma_{{\mathrm{4}}} }^{+}  }\token{wf} $.
    \item \label{item:promotion-var:typwf}
          If\/ $ \Psi \mid^{  \overrightarrow{ \gamma_{{\mathrm{1}}} }   \refenvsym{,}  \gamma_{{\mathrm{2}}} }   \binder{ \refenvmv{x} }\mathord{:^{\binder{ \gamma_{{\mathrm{3}}} } } } \refenvnt{A_{{\mathrm{1}}}}   \refenvsym{,}  \Gamma \vdash ^{  \overrightarrow{ \gamma_{{\mathrm{4}}} }^{+}  } \refenvnt{A_{{\mathrm{2}}}} \ \token{wf} $,
          then $ \Psi  \refenvsym{,}   \binder{ \refenvmv{y} }: \refenvnt{A_{{\mathrm{1}}}} \mathrel{@}\binder{ \gamma_{{\mathrm{3}}} } \mathbin{:\succeq} \gamma_{{\mathrm{2}}}  \mid^{  \overrightarrow{ \gamma_{{\mathrm{1}}} }   \refenvsym{,}  \gamma_{{\mathrm{3}}} }  \Gamma \vdash ^{  \overrightarrow{ \gamma_{{\mathrm{4}}} }^{+}  } \refenvnt{A_{{\mathrm{2}}}} \ \token{wf} $.
    \item \label{item:promotion-var:ltrans}
          If\/ $ \Psi \mid^{  \overrightarrow{ \gamma_{{\mathrm{1}}} }   \refenvsym{,}  \gamma_{{\mathrm{2}}} }  \binder{ \refenvmv{x} }\mathord{:^{\binder{ \gamma_{{\mathrm{3}}} } } } \refenvnt{A_{{\mathrm{1}}}}   \refenvsym{,}  \Gamma \vdash \gamma_{{\mathrm{4}}} \preceq \gamma_{{\mathrm{5}}} $,
          then $ \Psi  \refenvsym{,}   \binder{ \refenvmv{y} }: \refenvnt{A_{{\mathrm{1}}}} \mathrel{@}\binder{ \gamma_{{\mathrm{3}}} } \mathbin{:\succeq} \gamma_{{\mathrm{2}}}  \mid^{  \overrightarrow{ \gamma_{{\mathrm{1}}} }   \refenvsym{,}  \gamma_{{\mathrm{3}}} } \Gamma \vdash \gamma_{{\mathrm{4}}} \preceq \gamma_{{\mathrm{5}}} $.
    \item \label{item:promotion-var:gtrans}
          If\/ $ \Psi \mid^{  \overrightarrow{ \gamma_{{\mathrm{1}}} }   \refenvsym{,}  \gamma_{{\mathrm{2}}} }  \binder{ \refenvmv{x} }\mathord{:^{\binder{ \gamma_{{\mathrm{3}}} } } } \refenvnt{A_{{\mathrm{1}}}}   \refenvsym{,}  \Gamma \vdash \gamma_{{\mathrm{4}}} \subseteq \gamma_{{\mathrm{5}}} $,
          then $ \Psi  \refenvsym{,}   \binder{ \refenvmv{y} }: \refenvnt{A_{{\mathrm{1}}}} \mathrel{@}\binder{ \gamma_{{\mathrm{3}}} } \mathbin{:\succeq} \gamma_{{\mathrm{2}}}  \mid^{  \overrightarrow{ \gamma_{{\mathrm{1}}} }   \refenvsym{,}  \gamma_{{\mathrm{3}}} } \Gamma \vdash \gamma_{{\mathrm{4}}} \subseteq \gamma_{{\mathrm{5}}} $.
    \item \label{item:promotion-var:typing}
          If\/ $ \Psi \mid^{  \overrightarrow{ \gamma_{{\mathrm{1}}} }   \refenvsym{,}  \gamma_{{\mathrm{2}}} }   \binder{ \refenvmv{x} }\mathord{:^{\binder{ \gamma_{{\mathrm{3}}} } } } \refenvnt{A_{{\mathrm{1}}}}   \refenvsym{,}  \Gamma \vdash^{  \overrightarrow{ \gamma_{{\mathrm{4}}} }^{+}  }_{ R }  \refenvnt{e} : \refenvnt{A_{{\mathrm{2}}}} $,
          then $ \Psi  \refenvsym{,}   \binder{ \refenvmv{y} }: \refenvnt{A_{{\mathrm{1}}}} \mathrel{@}\binder{ \gamma_{{\mathrm{3}}} } \mathbin{:\succeq} \gamma_{{\mathrm{2}}}  \mid^{  \overrightarrow{ \gamma_{{\mathrm{1}}} }   \refenvsym{,}  \gamma_{{\mathrm{3}}} }  \Gamma \vdash^{  \overrightarrow{ \gamma_{{\mathrm{4}}} }^{+}  }_{ R  \refenvsym{,}  \refenvmv{x}  \coloneqq  \refenvmv{y} }  \refenvnt{e} : \refenvnt{A_{{\mathrm{2}}}} $.
  \end{enumerate}
\end{lemma}

\begin{proof}
  By mutual induction on the given derivation.
\end{proof}

\begin{lemma}[Promotion for Polymorphic Classifier Declarations]\label{claim:promotion-polyclsdecl}
  \begin{enumerate}
    \item \label{item:promotion-polyclsdecl:ctxwf}
          If
          $ \Psi \mid^{  \overrightarrow{ \delta_{{\mathrm{1}}} }   \refenvsym{,}   \gamma' _{ 0 }  }  [    \binder{  \gamma _{ 1 }  }  \mathbin{:\succeq}    \gamma' _{ 1 }  ,\dotsc,\binder{  \gamma _{ \refenvnt{k} }  }  \mathbin{:\succeq}   \gamma'  _{ \refenvnt{k} }   ]^{\binder{  \gamma _{ 0 }  } }   \refenvsym{,}  \Gamma \vdash^{  \overrightarrow{ \delta_{{\mathrm{2}}} }^{+}  }\token{wf} $,
          then
          $ \Psi  \refenvsym{,}   [    \binder{  \gamma _{ 0 }  }  \mathbin{:\succeq}    \gamma' _{ 0 }  ,\dotsc,\binder{  \gamma _{ \refenvnt{k} }  }  \mathbin{:\succeq}   \gamma'  _{ \refenvnt{k} }   ]  \mid^{  \overrightarrow{ \delta_{{\mathrm{1}}} }   \refenvsym{,}   \gamma _{ 0 }  } \Gamma \vdash^{  \overrightarrow{ \delta_{{\mathrm{2}}} }^{+}  }\token{wf} $.
    \item \label{item:promotion-polyclsdecl:typwf}
          If
          $ \Psi \mid^{  \overrightarrow{ \delta_{{\mathrm{1}}} }   \refenvsym{,}   \gamma' _{ 0 }  }   [    \binder{  \gamma _{ 1 }  }  \mathbin{:\succeq}    \gamma' _{ 1 }  ,\dotsc,\binder{  \gamma _{ \refenvnt{k} }  }  \mathbin{:\succeq}   \gamma'  _{ \refenvnt{k} }   ]^{\binder{  \gamma _{ 0 }  } }   \refenvsym{,}  \Gamma \vdash ^{  \overrightarrow{ \delta_{{\mathrm{2}}} }^{+}  } \refenvnt{A} \ \token{wf} $,
          then
          $ \Psi  \refenvsym{,}   [    \binder{  \gamma _{ 0 }  }  \mathbin{:\succeq}    \gamma' _{ 0 }  ,\dotsc,\binder{  \gamma _{ \refenvnt{k} }  }  \mathbin{:\succeq}   \gamma'  _{ \refenvnt{k} }   ]  \mid^{  \overrightarrow{ \delta_{{\mathrm{1}}} }   \refenvsym{,}   \gamma _{ 0 }  }  \Gamma \vdash ^{  \overrightarrow{ \delta_{{\mathrm{2}}} }^{+}  } \refenvnt{A} \ \token{wf} $.
    \item \label{item:promotion-polyclsdecl:ltrans}
          If
          $ \Psi \mid^{  \overrightarrow{ \delta_{{\mathrm{1}}} }   \refenvsym{,}   \gamma' _{ 0 }  }  [    \binder{  \gamma _{ 1 }  }  \mathbin{:\succeq}    \gamma' _{ 1 }  ,\dotsc,\binder{  \gamma _{ \refenvnt{k} }  }  \mathbin{:\succeq}   \gamma'  _{ \refenvnt{k} }   ]^{\binder{  \gamma _{ 0 }  } }   \refenvsym{,}  \Gamma \vdash \delta_{{\mathrm{3}}} \preceq \delta_{{\mathrm{4}}} $,
          then
          $ \Psi  \refenvsym{,}   [    \binder{  \gamma _{ 0 }  }  \mathbin{:\succeq}    \gamma' _{ 0 }  ,\dotsc,\binder{  \gamma _{ \refenvnt{k} }  }  \mathbin{:\succeq}   \gamma'  _{ \refenvnt{k} }   ]  \mid^{  \overrightarrow{ \delta_{{\mathrm{1}}} }   \refenvsym{,}   \gamma _{ 0 }  } \Gamma \vdash \delta_{{\mathrm{3}}} \preceq \delta_{{\mathrm{4}}} $.
    \item \label{item:promotion-polyclsdecl:gtrans}
          If
          $ \Psi \mid^{  \overrightarrow{ \delta_{{\mathrm{1}}} }   \refenvsym{,}   \gamma' _{ 0 }  }  [    \binder{  \gamma _{ 1 }  }  \mathbin{:\succeq}    \gamma' _{ 1 }  ,\dotsc,\binder{  \gamma _{ \refenvnt{k} }  }  \mathbin{:\succeq}   \gamma'  _{ \refenvnt{k} }   ]^{\binder{  \gamma _{ 0 }  } }   \refenvsym{,}  \Gamma \vdash \delta_{{\mathrm{3}}} \subseteq \delta_{{\mathrm{4}}} $,
          then
          $ \Psi  \refenvsym{,}   [    \binder{  \gamma _{ 0 }  }  \mathbin{:\succeq}    \gamma' _{ 0 }  ,\dotsc,\binder{  \gamma _{ \refenvnt{k} }  }  \mathbin{:\succeq}   \gamma'  _{ \refenvnt{k} }   ]  \mid^{  \overrightarrow{ \delta_{{\mathrm{1}}} }   \refenvsym{,}   \gamma _{ 0 }  } \Gamma \vdash \delta_{{\mathrm{3}}} \subseteq \delta_{{\mathrm{4}}} $.
    \item \label{item:promotion-polyclsdecl:typing}
          If
          $ \Psi \mid^{  \overrightarrow{ \delta_{{\mathrm{1}}} }   \refenvsym{,}   \gamma' _{ 0 }  }   [    \binder{  \gamma _{ 1 }  }  \mathbin{:\succeq}    \gamma' _{ 1 }  ,\dotsc,\binder{  \gamma _{ \refenvnt{k} }  }  \mathbin{:\succeq}   \gamma'  _{ \refenvnt{k} }   ]^{\binder{  \gamma _{ 0 }  } }   \refenvsym{,}  \Gamma \vdash^{  \overrightarrow{ \delta_{{\mathrm{2}}} }^{+}  }_{ R }  \refenvnt{e} : \refenvnt{A} $,
          then
          $ \Psi  \refenvsym{,}   [    \binder{  \gamma _{ 0 }  }  \mathbin{:\succeq}    \gamma' _{ 0 }  ,\dotsc,\binder{  \gamma _{ \refenvnt{k} }  }  \mathbin{:\succeq}   \gamma'  _{ \refenvnt{k} }   ]  \mid^{  \overrightarrow{ \delta_{{\mathrm{1}}} }   \refenvsym{,}   \gamma _{ 0 }  }  \Gamma \vdash^{  \overrightarrow{ \delta_{{\mathrm{2}}} }^{+}  }_{ R }  \refenvnt{e} : \refenvnt{A} $.
  \end{enumerate}
\end{lemma}

\begin{proof}
  By mutual induction on the given derivation.
\end{proof}

\begin{corollary}[Promotion]\label{claim:promotion}
  \begin{enumerate}
    \item If\/ $ \Psi \mid^{  \overrightarrow{ \gamma_{{\mathrm{1}}} }^{+}  }   \blacktriangleright ^{ \gamma_{{\mathrm{2}}} }  \vdash^{  \overrightarrow{ \gamma_{{\mathrm{1}}} }^{+}   \refenvsym{,}  \gamma_{{\mathrm{2}}} }_{ R }  \refenvnt{e} : \refenvnt{A} $,
          then
          $ \Psi \mid^{  \overrightarrow{ \gamma_{{\mathrm{1}}} }^{+}   \refenvsym{,}  \gamma_{{\mathrm{2}}} }  \varepsilon \vdash^{  \overrightarrow{ \gamma_{{\mathrm{1}}} }^{+}   \refenvsym{,}  \gamma_{{\mathrm{2}}} }_{ R }  \refenvnt{e} : \refenvnt{A} $.
    \item If
          $ \Psi \mid^{  \overrightarrow{ \gamma_{{\mathrm{1}}} }   \refenvsym{,}    \delta _{ 0 }  ,\dotsc,  \delta _{ \refenvnt{k} }   }   \blacktriangleleft _{ \refenvnt{k} }^{\binder{ \gamma_{{\mathrm{2}}} } }  \vdash^{  \overrightarrow{ \gamma_{{\mathrm{1}}} }   \refenvsym{,}  \gamma_{{\mathrm{2}}} }_{ R }  \refenvnt{e} : \refenvnt{A} $,
          then
          $ \Psi  \refenvsym{,}   \binder{ \gamma_{{\mathrm{2}}} }( \mathbin{:\succeq} \;  \delta _{ 0 }   /  \mathbin{:\supseteq} \;  \delta _{ \refenvnt{k} }  )  \mid^{  \overrightarrow{ \gamma_{{\mathrm{1}}} }   \refenvsym{,}  \gamma_{{\mathrm{2}}} }  \varepsilon \vdash^{  \overrightarrow{ \gamma_{{\mathrm{1}}} }   \refenvsym{,}  \gamma_{{\mathrm{2}}} }_{ R }  \refenvnt{e} : \refenvnt{A} $.
    \item If
          $ \Psi \mid^{  \overrightarrow{ \gamma_{{\mathrm{1}}} }   \refenvsym{,}  \gamma_{{\mathrm{2}}} }   \binder{ \refenvmv{x} }\mathord{:^{\binder{ \gamma_{{\mathrm{3}}} } } } \refenvnt{A_{{\mathrm{1}}}}  \vdash^{  \overrightarrow{ \gamma_{{\mathrm{1}}} }   \refenvsym{,}  \gamma_{{\mathrm{3}}} }_{ R }  \refenvnt{e} : \refenvnt{A_{{\mathrm{2}}}} $
          and $\refenvmv{y} \, \not\in \,  \token{Dom}_{V}( \Psi ) $,
          then
          $ \Psi  \refenvsym{,}   \binder{ \refenvmv{y} }: \refenvnt{A_{{\mathrm{1}}}} \mathrel{@}\binder{ \gamma_{{\mathrm{3}}} } \mathbin{:\succeq} \gamma_{{\mathrm{2}}}  \mid^{  \overrightarrow{ \gamma_{{\mathrm{1}}} }   \refenvsym{,}  \gamma_{{\mathrm{3}}} }  \varepsilon \vdash^{  \overrightarrow{ \gamma_{{\mathrm{1}}} }   \refenvsym{,}  \gamma_{{\mathrm{3}}} }_{ R  \refenvsym{,}  \refenvmv{x}  \coloneqq  \refenvmv{y} }  \refenvnt{e} : \refenvnt{A_{{\mathrm{2}}}} $.
    \item If
          $ \Psi \mid^{  \overrightarrow{ \delta_{{\mathrm{1}}} }   \refenvsym{,}   \gamma' _{ 0 }  }   [    \binder{  \gamma _{ 1 }  }  \mathbin{:\succeq}    \gamma' _{ 1 }  ,\dotsc,\binder{  \gamma _{ \refenvnt{k} }  }  \mathbin{:\succeq}   \gamma'  _{ \refenvnt{k} }   ]^{\binder{  \gamma _{ 0 }  } }  \vdash^{  \overrightarrow{ \delta_{{\mathrm{1}}} }   \refenvsym{,}   \gamma _{ 0 }  }_{ R }  \refenvnt{e} : \refenvnt{A} $,
          then
          $ \Psi  \refenvsym{,}   [    \binder{  \gamma _{ 0 }  }  \mathbin{:\succeq}    \gamma' _{ 0 }  ,\dotsc,\binder{  \gamma _{ \refenvnt{k} }  }  \mathbin{:\succeq}   \gamma'  _{ \refenvnt{k} }   ]  \mid^{  \overrightarrow{ \delta_{{\mathrm{1}}} }   \refenvsym{,}   \gamma _{ 0 }  }  \varepsilon \vdash^{  \overrightarrow{ \delta_{{\mathrm{1}}} }   \refenvsym{,}   \gamma _{ 0 }  }_{ R }  \refenvnt{e} : \refenvnt{A} $.
  \end{enumerate}
\end{corollary}

\subsection{Demotion Lemma}
\begin{definition}[Disjointness of Classifiers]
  We write $ \Psi \vdash  \overrightarrow{ \gamma_{{\mathrm{1}}} }  \mathrel{\#}  \overrightarrow{ \gamma_{{\mathrm{2}}} }  $ if\/ $\Psi  \vdash  \gamma'_{{\mathrm{2}}}  \subseteq  \gamma'_{{\mathrm{1}}}$ does not hold
  for any $\gamma'_{{\mathrm{1}}} \, \in \, \refenvsym{\{}   \overrightarrow{ \gamma_{{\mathrm{1}}} }   \refenvsym{\}}$ and $\gamma'_{{\mathrm{2}}} \, \in \, \refenvsym{\{}   \overrightarrow{ \gamma_{{\mathrm{2}}} }   \refenvsym{\}}$.
\end{definition}


\begin{lemma}[Demotion for Variables]\label{claim:demotion-var}
  Suppose
  $ \binder{ \refenvmv{x} }: \refenvnt{A_{{\mathrm{1}}}} \mathrel{@}\binder{ \gamma_{{\mathrm{2}}} } \mathbin{:\succeq} \gamma_{{\mathrm{4}}}  \, \in \, \Psi$,
  $ \Psi \vdash  \overrightarrow{ \gamma_{{\mathrm{1}}} }  \mathrel{\#} \gamma_{{\mathrm{2}}} $,
  and $\gamma_{{\mathrm{5}}} \, \not\in \,  \token{Dom}_{C}( \Psi )  \, \cup \,  \token{Dom}_{C}( \Gamma ) $.
  \begin{enumerate}
    \item \label{item:demotion-var:ctxwf}
          If\/ $ \Psi \mid^{  \overrightarrow{ \gamma_{{\mathrm{1}}} }   \refenvsym{,}  \gamma_{{\mathrm{2}}} } \Gamma \vdash^{  \overrightarrow{ \gamma_{{\mathrm{3}}} }^{+}  }\token{wf} $,
          then
          $ \Psi \mid^{  \overrightarrow{ \gamma_{{\mathrm{1}}} }   \refenvsym{,}  \gamma_{{\mathrm{4}}} }  \binder{ \refenvmv{x} }\mathord{:^{\binder{ \gamma_{{\mathrm{5}}} } } } \refenvnt{A_{{\mathrm{1}}}}   \refenvsym{,}  \Gamma  \refenvsym{[}  \gamma_{{\mathrm{2}}}  \coloneqq  \gamma_{{\mathrm{5}}}  \refenvsym{]} \vdash^{   \overrightarrow{ \gamma_{{\mathrm{3}}} }^{+}    \refenvsym{[}  \gamma_{{\mathrm{2}}}  \coloneqq  \gamma_{{\mathrm{5}}}  \refenvsym{]} }\token{wf} $.
    \item \label{item:demotion-var:typwf}
          If\/ $ \Psi \mid^{  \overrightarrow{ \gamma_{{\mathrm{1}}} }   \refenvsym{,}  \gamma_{{\mathrm{2}}} }  \Gamma \vdash ^{  \overrightarrow{ \gamma_{{\mathrm{3}}} }^{+}  } \refenvnt{A_{{\mathrm{2}}}} \ \token{wf} $,
          then
          $ \Psi \mid^{  \overrightarrow{ \gamma_{{\mathrm{1}}} }   \refenvsym{,}  \gamma_{{\mathrm{4}}} }   \binder{ \refenvmv{x} }\mathord{:^{\binder{ \gamma_{{\mathrm{5}}} } } } \refenvnt{A_{{\mathrm{1}}}}   \refenvsym{,}  \Gamma  \refenvsym{[}  \gamma_{{\mathrm{2}}}  \coloneqq  \gamma_{{\mathrm{5}}}  \refenvsym{]} \vdash ^{   \overrightarrow{ \gamma_{{\mathrm{3}}} }^{+}    \refenvsym{[}  \gamma_{{\mathrm{2}}}  \coloneqq  \gamma_{{\mathrm{5}}}  \refenvsym{]} } \refenvnt{A_{{\mathrm{2}}}}  \refenvsym{[}  \gamma_{{\mathrm{2}}}  \coloneqq  \gamma_{{\mathrm{5}}}  \refenvsym{]} \ \token{wf} $.
    \item \label{item:demotion-var:ltrans}
          If\/ $ \Psi \mid^{  \overrightarrow{ \gamma_{{\mathrm{1}}} }   \refenvsym{,}  \gamma_{{\mathrm{2}}} } \Gamma \vdash \gamma_{{\mathrm{6}}} \preceq \gamma_{{\mathrm{7}}} $
          and either $\gamma_{{\mathrm{7}}} \, \in \,  \token{Dom}_{C}( \Gamma ) $ or there exists $\gamma_{{\mathrm{8}}} \, \in \, \refenvsym{\{}   \overrightarrow{ \gamma_{{\mathrm{1}}} }   \refenvsym{,}  \gamma_{{\mathrm{2}}}  \refenvsym{\}}$ such that $ \Psi \mid^{  \overrightarrow{ \gamma_{{\mathrm{1}}} }   \refenvsym{,}  \gamma_{{\mathrm{2}}} } \Gamma \vdash \gamma_{{\mathrm{7}}} \subseteq \gamma_{{\mathrm{8}}} $,
          then
          $ \Psi \mid^{  \overrightarrow{ \gamma_{{\mathrm{1}}} }   \refenvsym{,}  \gamma_{{\mathrm{4}}} }  \binder{ \refenvmv{x} }\mathord{:^{\binder{ \gamma_{{\mathrm{5}}} } } } \refenvnt{A_{{\mathrm{1}}}}   \refenvsym{,}  \Gamma  \refenvsym{[}  \gamma_{{\mathrm{2}}}  \coloneqq  \gamma_{{\mathrm{5}}}  \refenvsym{]} \vdash \gamma_{{\mathrm{6}}}  \refenvsym{[}  \gamma_{{\mathrm{2}}}  \coloneqq  \gamma_{{\mathrm{5}}}  \refenvsym{]} \preceq \gamma_{{\mathrm{7}}}  \refenvsym{[}  \gamma_{{\mathrm{2}}}  \coloneqq  \gamma_{{\mathrm{5}}}  \refenvsym{]} $.
    \item \label{item:demotion-var:gtrans}
          If\/ $ \Psi \mid^{  \overrightarrow{ \gamma_{{\mathrm{1}}} }   \refenvsym{,}  \gamma_{{\mathrm{2}}} } \Gamma \vdash \gamma_{{\mathrm{6}}} \subseteq \gamma_{{\mathrm{7}}} $
          and either $\gamma_{{\mathrm{7}}} \, \in \,  \token{Dom}_{C}( \Gamma ) $ or there exists $\gamma_{{\mathrm{8}}} \, \in \, \refenvsym{\{}   \overrightarrow{ \gamma_{{\mathrm{1}}} }   \refenvsym{,}  \gamma_{{\mathrm{2}}}  \refenvsym{\}}$ such that $ \Psi \mid^{  \overrightarrow{ \gamma_{{\mathrm{1}}} }   \refenvsym{,}  \gamma_{{\mathrm{2}}} } \Gamma \vdash \gamma_{{\mathrm{7}}} \subseteq \gamma_{{\mathrm{8}}} $,
          then
          $ \Psi \mid^{  \overrightarrow{ \gamma_{{\mathrm{1}}} }   \refenvsym{,}  \gamma_{{\mathrm{4}}} }  \binder{ \refenvmv{x} }\mathord{:^{\binder{ \gamma_{{\mathrm{5}}} } } } \refenvnt{A_{{\mathrm{1}}}}   \refenvsym{,}  \Gamma  \refenvsym{[}  \gamma_{{\mathrm{2}}}  \coloneqq  \gamma_{{\mathrm{5}}}  \refenvsym{]} \vdash \gamma_{{\mathrm{6}}}  \refenvsym{[}  \gamma_{{\mathrm{2}}}  \coloneqq  \gamma_{{\mathrm{5}}}  \refenvsym{]} \subseteq \gamma_{{\mathrm{7}}}  \refenvsym{[}  \gamma_{{\mathrm{2}}}  \coloneqq  \gamma_{{\mathrm{5}}}  \refenvsym{]} $.
    \item \label{item:demotion-var:typing}
          If\/ $ \Psi \mid^{  \overrightarrow{ \gamma_{{\mathrm{1}}} }   \refenvsym{,}  \gamma_{{\mathrm{2}}} }  \Gamma \vdash^{  \overrightarrow{ \gamma_{{\mathrm{3}}} }^{+}  }_{  \token{id}  }  \refenvnt{e} : \refenvnt{A_{{\mathrm{2}}}} $,
          then
          $ \Psi \mid^{  \overrightarrow{ \gamma_{{\mathrm{1}}} }   \refenvsym{,}  \gamma_{{\mathrm{4}}} }   \binder{ \refenvmv{x} }\mathord{:^{\binder{ \gamma_{{\mathrm{5}}} } } } \refenvnt{A_{{\mathrm{1}}}}   \refenvsym{,}  \Gamma  \refenvsym{[}  \gamma_{{\mathrm{2}}}  \coloneqq  \gamma_{{\mathrm{5}}}  \refenvsym{]} \vdash^{   \overrightarrow{ \gamma_{{\mathrm{3}}} }^{+}    \refenvsym{[}  \gamma_{{\mathrm{2}}}  \coloneqq  \gamma_{{\mathrm{5}}}  \refenvsym{]} }_{  \token{id}  }  \refenvnt{e} : \refenvnt{A_{{\mathrm{2}}}}  \refenvsym{[}  \gamma_{{\mathrm{2}}}  \coloneqq  \gamma_{{\mathrm{5}}}  \refenvsym{]} $.
  \end{enumerate}
\end{lemma}

\begin{proof}
  We proceed by mutual induction on the given derivation.
  We only discuss the cases for visibility judgments and expression typing.
  \begin{description}
    \item[Case \textmd{\zcref{item:demotion-var:ctxwf}}:]
      By induction on the context well-formedness derivation.  We spell out
      the case for \ref{rule:runtime-wf-ctx-open}; the other cases are
      immediate by the induction hypothesis and reapplication of the same
      well-formedness rule.

      Suppose the last rule is \ref{rule:runtime-wf-ctx-open}.  By inversion,
      $\Gamma = \Gamma_{{\mathrm{1}}}  \refenvsym{,}   \blacktriangleright ^{ \delta_{{\mathrm{1}}} } $ and
      $ \overrightarrow{ \gamma_{{\mathrm{3}}} }^{+}  =  \overrightarrow{ \delta_{{\mathrm{2}}} }   \refenvsym{,}  \delta_{{\mathrm{3}}}  \refenvsym{,}  \delta_{{\mathrm{1}}}$, with premises
      \[
         \Psi \mid^{  \overrightarrow{ \gamma_{{\mathrm{1}}} }   \refenvsym{,}  \gamma_{{\mathrm{2}}} } \Gamma_{{\mathrm{1}}} \vdash^{  \overrightarrow{ \delta_{{\mathrm{2}}} }   \refenvsym{,}  \delta_{{\mathrm{3}}} }\token{wf} 
        \quad\text{and}\quad
         \Psi \mid^{  \overrightarrow{ \gamma_{{\mathrm{1}}} }   \refenvsym{,}  \gamma_{{\mathrm{2}}} } \Gamma_{{\mathrm{1}}} \vdash \delta_{{\mathrm{1}}} \subseteq \delta_{{\mathrm{3}}} .
      \]
      The induction hypothesis gives the demoted well-formedness of
      $\Gamma_{{\mathrm{1}}}$.  Moreover, by
      \zcref{claim:ctx-output-classifier-origin},
      $\delta_{{\mathrm{3}}} \, \in \, \refenvsym{\{}   \overrightarrow{ \gamma_{{\mathrm{1}}} }   \refenvsym{,}  \gamma_{{\mathrm{2}}}  \refenvsym{\}} \, \cup \,  \token{Dom}_{C}( \Gamma_{{\mathrm{1}}} )  \, \cup \,  \token{FC}( \Gamma_{{\mathrm{1}}} ) $, and hence the
      side condition of \zcref{item:demotion-var:gtrans} holds for the
      visibility premise.  Thus
      \[
         \Psi \mid^{  \overrightarrow{ \gamma_{{\mathrm{1}}} }   \refenvsym{,}  \gamma_{{\mathrm{4}}} }  \binder{ \refenvmv{x} }\mathord{:^{\binder{ \gamma_{{\mathrm{5}}} } } } \refenvnt{A_{{\mathrm{1}}}}  \refenvsym{[}  \gamma_{{\mathrm{2}}}  \coloneqq  \gamma_{{\mathrm{5}}}  \refenvsym{]}   \refenvsym{,}  \Gamma_{{\mathrm{1}}}  \refenvsym{[}  \gamma_{{\mathrm{2}}}  \coloneqq  \gamma_{{\mathrm{5}}}  \refenvsym{]} \vdash \delta_{{\mathrm{1}}}  \refenvsym{[}  \gamma_{{\mathrm{2}}}  \coloneqq  \gamma_{{\mathrm{5}}}  \refenvsym{]} \subseteq \delta_{{\mathrm{3}}}  \refenvsym{[}  \gamma_{{\mathrm{2}}}  \coloneqq  \gamma_{{\mathrm{5}}}  \refenvsym{]} .
      \]
      Reapplying \ref{rule:runtime-wf-ctx-open} yields the desired
      well-formedness judgment.

    \item[Case \textmd{\zcref{item:demotion-var:typwf}}:]
      By induction on the type well-formedness derivation.

    \item[Case \textmd{\zcref{item:demotion-var:ltrans}}:]
      This case is analogous to \zcref{item:demotion-var:gtrans}, using the
      inversion lemma and rules for $ \preceq $ in place of those for
      $ \subseteq $.

    \item[Case \textmd{\zcref{item:demotion-var:gtrans}}:]
      By induction with respect to $ \token{deg} ( \Psi , \Gamma , \gamma_{{\mathrm{7}}} ) $.

      By the side condition of the lemma, either
      there exists $\gamma_{{\mathrm{8}}} \, \in \, \refenvsym{\{}   \overrightarrow{ \gamma_{{\mathrm{1}}} }   \refenvsym{,}  \gamma_{{\mathrm{2}}}  \refenvsym{\}}$ such that $ \Psi \mid^{  \overrightarrow{ \gamma_{{\mathrm{1}}} }   \refenvsym{,}  \gamma_{{\mathrm{2}}} } \Gamma \vdash \gamma_{{\mathrm{7}}} \subseteq \gamma_{{\mathrm{8}}} $, or
      $\gamma_{{\mathrm{7}}} \, \in \,  \token{Dom}_{C}( \Gamma ) $.  We first consider the case where $\gamma_{{\mathrm{7}}} \, \not\in \,  \token{Dom}_{C}( \Gamma ) $.
      Then, we have $\gamma_{{\mathrm{8}}} \, \in \, \refenvsym{\{}   \overrightarrow{ \gamma_{{\mathrm{1}}} }   \refenvsym{,}  \gamma_{{\mathrm{2}}}  \refenvsym{\}}$ such that $ \Psi \mid^{  \overrightarrow{ \gamma_{{\mathrm{1}}} }   \refenvsym{,}  \gamma_{{\mathrm{2}}} } \Gamma \vdash \gamma_{{\mathrm{7}}} \subseteq \gamma_{{\mathrm{8}}} $.
      By disjointness of $ \token{Dom}_{C}( \Gamma ) $ and $ \token{Dom}_{C}( \Psi ) $, we have $\gamma_{{\mathrm{7}}} \, \in \,  \token{Dom}_{C}( \Psi ) $.
      Therefore $\Psi  \vdash  \gamma_{{\mathrm{6}}}  \subseteq  \gamma_{{\mathrm{7}}}$ by \zcref{claim:local-to-global-trans}.
      Moreover, \zcref{claim:regularity-runtime-judgments} and
      \zcref{item:demotion-var:ctxwf} give
      \[
         \Psi \mid^{  \overrightarrow{ \gamma_{{\mathrm{1}}} }   \refenvsym{,}  \gamma_{{\mathrm{4}}} }  \binder{ \refenvmv{x} }\mathord{:^{\binder{ \gamma_{{\mathrm{5}}} } } } \refenvnt{A_{{\mathrm{1}}}}  \refenvsym{[}  \gamma_{{\mathrm{2}}}  \coloneqq  \gamma_{{\mathrm{5}}}  \refenvsym{]}   \refenvsym{,}  \Gamma  \refenvsym{[}  \gamma_{{\mathrm{2}}}  \coloneqq  \gamma_{{\mathrm{5}}}  \refenvsym{]} \vdash^{  \dotsc  }\token{wf} .
      \]
      Therefore, by \zcref{claim:global-to-local-trans},
      \[
         \Psi \mid^{  \overrightarrow{ \gamma_{{\mathrm{1}}} }   \refenvsym{,}  \gamma_{{\mathrm{4}}} }  \binder{ \refenvmv{x} }\mathord{:^{\binder{ \gamma_{{\mathrm{5}}} } } } \refenvnt{A_{{\mathrm{1}}}}  \refenvsym{[}  \gamma_{{\mathrm{2}}}  \coloneqq  \gamma_{{\mathrm{5}}}  \refenvsym{]}   \refenvsym{,}  \Gamma  \refenvsym{[}  \gamma_{{\mathrm{2}}}  \coloneqq  \gamma_{{\mathrm{5}}}  \refenvsym{]} \vdash \gamma_{{\mathrm{6}}} \subseteq \gamma_{{\mathrm{7}}} .
      \]
      We conclude by cases on whether the substitution $\gamma_{{\mathrm{2}}}  \coloneqq  \gamma_{{\mathrm{5}}}$ affects $\gamma_{{\mathrm{6}}}$ or
      $\gamma_{{\mathrm{7}}}$.
      \begin{description}
        \item[Case \textmd{$\gamma_{{\mathrm{2}}} \neq \gamma_{{\mathrm{6}}}$ and $\gamma_{{\mathrm{2}}} \neq \gamma_{{\mathrm{7}}}$}:]
          The substitution leaves both endpoints unchanged, so the required
          judgment follows immediately.

        \item[Case \textmd{$\gamma_{{\mathrm{2}}} \neq \gamma_{{\mathrm{6}}}$ and $\gamma_{{\mathrm{2}}} = \gamma_{{\mathrm{7}}}$}:]
          By \zcref{claim:inversion-runtime-gtrans-nht} and
          $ \binder{ \refenvmv{x} }: \refenvnt{A_{{\mathrm{1}}}} \mathrel{@}\binder{ \gamma_{{\mathrm{2}}} } \mathbin{:\succeq} \gamma_{{\mathrm{4}}}  \, \in \, \Psi$, we have $\Psi  \vdash  \gamma_{{\mathrm{6}}}  \subseteq  \gamma_{{\mathrm{4}}}$.
          By \zcref{claim:global-to-local-trans},
          \[
             \Psi \mid^{  \overrightarrow{ \gamma_{{\mathrm{1}}} }   \refenvsym{,}  \gamma_{{\mathrm{4}}} }  \binder{ \refenvmv{x} }\mathord{:^{\binder{ \gamma_{{\mathrm{5}}} } } } \refenvnt{A_{{\mathrm{1}}}}  \refenvsym{[}  \gamma_{{\mathrm{2}}}  \coloneqq  \gamma_{{\mathrm{5}}}  \refenvsym{]}   \refenvsym{,}  \Gamma  \refenvsym{[}  \gamma_{{\mathrm{2}}}  \coloneqq  \gamma_{{\mathrm{5}}}  \refenvsym{]} \vdash \gamma_{{\mathrm{6}}}  \refenvsym{[}  \gamma_{{\mathrm{2}}}  \coloneqq  \gamma_{{\mathrm{5}}}  \refenvsym{]} \subseteq \gamma_{{\mathrm{4}}} .
          \]
          Reapplying \ref{rule:runtime-ltrans-var} in the demoted context and
          then \ref{rule:runtime-gtrans-lift} gives
          \[
             \Psi \mid^{  \overrightarrow{ \gamma_{{\mathrm{1}}} }   \refenvsym{,}  \gamma_{{\mathrm{4}}} }  \binder{ \refenvmv{x} }\mathord{:^{\binder{ \gamma_{{\mathrm{5}}} } } } \refenvnt{A_{{\mathrm{1}}}}  \refenvsym{[}  \gamma_{{\mathrm{2}}}  \coloneqq  \gamma_{{\mathrm{5}}}  \refenvsym{]}   \refenvsym{,}  \Gamma  \refenvsym{[}  \gamma_{{\mathrm{2}}}  \coloneqq  \gamma_{{\mathrm{5}}}  \refenvsym{]} \vdash \gamma_{{\mathrm{4}}} \subseteq \gamma_{{\mathrm{5}}} .
          \]
          The conclusion follows by
          \ref{rule:runtime-gtrans-trans}.

        \item[Case \textmd{$\gamma_{{\mathrm{2}}} = \gamma_{{\mathrm{6}}} = \gamma_{{\mathrm{7}}}$}:]
          Then
          $\gamma_{{\mathrm{6}}}  \refenvsym{[}  \gamma_{{\mathrm{2}}}  \coloneqq  \gamma_{{\mathrm{5}}}  \refenvsym{]} = \gamma_{{\mathrm{7}}}  \refenvsym{[}  \gamma_{{\mathrm{2}}}  \coloneqq  \gamma_{{\mathrm{5}}}  \refenvsym{]} = \gamma_{{\mathrm{5}}}$.
          The required judgment follows from
          \ref{rule:runtime-ltrans-refl} and \ref{rule:runtime-gtrans-lift}.

        \item[Case \textmd{$\gamma_{{\mathrm{2}}} = \gamma_{{\mathrm{6}}}$ and $\gamma_{{\mathrm{2}}} \neq \gamma_{{\mathrm{7}}}$}:]
          Since $\gamma_{{\mathrm{6}}} = \gamma_{{\mathrm{2}}}$, we have
          $\Psi  \vdash  \gamma_{{\mathrm{2}}}  \subseteq  \gamma_{{\mathrm{7}}}$.
          Moreover, for some $\gamma_{{\mathrm{8}}} \, \in \, \refenvsym{\{}   \overrightarrow{ \gamma_{{\mathrm{1}}} }   \refenvsym{,}  \gamma_{{\mathrm{2}}}  \refenvsym{\}}$ we have
          $ \Psi \mid^{  \overrightarrow{ \gamma_{{\mathrm{1}}} }   \refenvsym{,}  \gamma_{{\mathrm{2}}} } \Gamma \vdash \gamma_{{\mathrm{7}}} \subseteq \gamma_{{\mathrm{8}}} $.
          By \zcref{claim:local-to-global-trans}, this gives
          $\Psi  \vdash  \gamma_{{\mathrm{7}}}  \subseteq  \gamma_{{\mathrm{8}}}$; together with
          $\Psi  \vdash  \gamma_{{\mathrm{2}}}  \subseteq  \gamma_{{\mathrm{7}}}$ and \ref{rule:runtime-gtrans-trans}, we get
          $\Psi  \vdash  \gamma_{{\mathrm{2}}}  \subseteq  \gamma_{{\mathrm{8}}}$.
          Since $ \Psi \vdash  \overrightarrow{ \gamma_{{\mathrm{1}}} }  \mathrel{\#} \gamma_{{\mathrm{2}}} $, the only possible such
          $\gamma_{{\mathrm{8}}}$ is $\gamma_{{\mathrm{2}}}$.  Hence
          $\Psi  \vdash  \gamma_{{\mathrm{7}}}  \subseteq  \gamma_{{\mathrm{2}}}$.
          Applying \zcref{claim:trans-antisymmetry} to
          $\Psi  \vdash  \gamma_{{\mathrm{2}}}  \subseteq  \gamma_{{\mathrm{7}}}$ and $\Psi  \vdash  \gamma_{{\mathrm{7}}}  \subseteq  \gamma_{{\mathrm{2}}}$ yields
          $\gamma_{{\mathrm{2}}} = \gamma_{{\mathrm{7}}}$, contradicting the case assumption.  Thus
          this case is impossible.
      \end{description}

      It remains to consider the case $\gamma_{{\mathrm{7}}} \, \in \,  \token{Dom}_{C}( \Gamma ) $.  If
      $\gamma_{{\mathrm{6}}} = \gamma_{{\mathrm{7}}}$, then $\gamma_{{\mathrm{7}}}  \refenvsym{[}  \gamma_{{\mathrm{2}}}  \coloneqq  \gamma_{{\mathrm{5}}}  \refenvsym{]}$ is declared in the
      demoted context by \zcref{item:demotion-var:ctxwf}.  Hence the desired
      judgment follows from \ref{rule:runtime-ltrans-refl} and
      \ref{rule:runtime-gtrans-lift}.  Thus assume $\gamma_{{\mathrm{6}}} \neq \gamma_{{\mathrm{7}}}$.
      We perform case analysis using
      \zcref{claim:inversion-runtime-gtrans-ctx}.  In each case, the inversion
      gives a derivation
      $ \Psi \mid^{  \overrightarrow{ \gamma_{{\mathrm{1}}} }   \refenvsym{,}  \gamma_{{\mathrm{2}}} } \Gamma \vdash \gamma_{{\mathrm{6}}} \subseteq \delta_{{\mathrm{3}}} $
      where $ \token{deg} ( \Psi , \Gamma , \delta_{{\mathrm{3}}} )  <  \token{deg} ( \Psi , \Gamma , \gamma_{{\mathrm{7}}} ) $
      and $\delta_{{\mathrm{3}}} \, \in \, \refenvsym{\{}   \overrightarrow{ \gamma_{{\mathrm{1}}} }   \refenvsym{,}  \gamma_{{\mathrm{2}}}  \refenvsym{\}} \, \cup \,  \token{Dom}_{C}( \Gamma )  \, \cup \,  \token{FC}( \Gamma ) $.
      The membership condition follows from
      \zcref{claim:ctx-output-classifier-origin} when $\delta_{{\mathrm{3}}}$ comes from
      the output stack of the corresponding context prefix.  In the remaining
      polymorphic-classifier declaration cases, $\delta_{{\mathrm{3}}}$ appears as the
      right-hand side of a declaration $ \binder{ \gamma_{{\mathrm{7}}} }  \mathbin{:\succeq}   \delta_{{\mathrm{3}}} $, so the condition
      follows from the definitions of $ \token{Dom}_{C}( \Gamma ) $ and $ \token{FC}( \Gamma ) $.
      Hence, the induction hypothesis gives
      \[
         \Psi \mid^{  \overrightarrow{ \gamma_{{\mathrm{1}}} }   \refenvsym{,}  \gamma_{{\mathrm{4}}} }  \binder{ \refenvmv{x} }\mathord{:^{\binder{ \gamma_{{\mathrm{5}}} } } } \refenvnt{A_{{\mathrm{1}}}}  \refenvsym{[}  \gamma_{{\mathrm{2}}}  \coloneqq  \gamma_{{\mathrm{5}}}  \refenvsym{]}   \refenvsym{,}  \Gamma  \refenvsym{[}  \gamma_{{\mathrm{2}}}  \coloneqq  \gamma_{{\mathrm{5}}}  \refenvsym{]} \vdash \gamma_{{\mathrm{6}}}  \refenvsym{[}  \gamma_{{\mathrm{2}}}  \coloneqq  \gamma_{{\mathrm{5}}}  \refenvsym{]} \subseteq \delta_{{\mathrm{3}}}  \refenvsym{[}  \gamma_{{\mathrm{2}}}  \coloneqq  \gamma_{{\mathrm{5}}}  \refenvsym{]} .
      \]
      Reapplying the corresponding context rule gives
      \[
         \Psi \mid^{  \overrightarrow{ \gamma_{{\mathrm{1}}} }   \refenvsym{,}  \gamma_{{\mathrm{4}}} }  \binder{ \refenvmv{x} }\mathord{:^{\binder{ \gamma_{{\mathrm{5}}} } } } \refenvnt{A_{{\mathrm{1}}}}  \refenvsym{[}  \gamma_{{\mathrm{2}}}  \coloneqq  \gamma_{{\mathrm{5}}}  \refenvsym{]}   \refenvsym{,}  \Gamma  \refenvsym{[}  \gamma_{{\mathrm{2}}}  \coloneqq  \gamma_{{\mathrm{5}}}  \refenvsym{]} \vdash \delta_{{\mathrm{3}}}  \refenvsym{[}  \gamma_{{\mathrm{2}}}  \coloneqq  \gamma_{{\mathrm{5}}}  \refenvsym{]} \subseteq \gamma_{{\mathrm{7}}}  \refenvsym{[}  \gamma_{{\mathrm{2}}}  \coloneqq  \gamma_{{\mathrm{5}}}  \refenvsym{]} .
      \]
      The desired judgment follows by \ref{rule:runtime-gtrans-trans}.

    \item[Case \textmd{\zcref{item:demotion-var:typing}}:]
      By induction on the typing derivation.  We spell out
      \ref{rule:runtime-type-var}, \ref{rule:runtime-type-reserved-var}, and
      \ref{rule:runtime-type-splice}; the remaining cases are immediate or
      analogous by the induction hypothesis.

      \begin{description}
        \item[Case \textmd{\ref{rule:runtime-type-var}}:]
          By inversion, the expression is a variable $\refenvmv{z}$ and the
          derivation gives
          $\token{lookup} \, \refenvsym{(}  \Gamma  \refenvsym{,}  \refenvmv{z}  \refenvsym{)} = \token{Done} \, \refenvsym{(}  \refenvnt{A_{{\mathrm{2}}}}  \refenvsym{,}  \delta_{{\mathrm{1}}}  \refenvsym{)}$,
          \[
             \Psi \mid^{  \overrightarrow{ \gamma_{{\mathrm{1}}} }   \refenvsym{,}  \gamma_{{\mathrm{2}}} } \Gamma \vdash^{  \overrightarrow{ \delta_{{\mathrm{2}}} }   \refenvsym{,}  \delta_{{\mathrm{3}}} }\token{wf} 
            \quad\text{and}\quad
             \Psi \mid^{  \overrightarrow{ \gamma_{{\mathrm{1}}} }   \refenvsym{,}  \gamma_{{\mathrm{2}}} } \Gamma \vdash \delta_{{\mathrm{1}}} \preceq \delta_{{\mathrm{3}}} .
          \]
          By \zcref{item:demotion-var:ctxwf}, the well-formed context premise
          is preserved by demotion.  It remains to check the side condition
          needed to apply \zcref{item:demotion-var:ltrans} to the reachability
          premise.  By \zcref{claim:ctx-output-classifier-origin},
          \[
            \delta_{{\mathrm{3}}} \, \in \, \refenvsym{\{}   \overrightarrow{ \gamma_{{\mathrm{1}}} }   \refenvsym{,}  \gamma_{{\mathrm{2}}}  \refenvsym{\}} \, \cup \,  \token{Dom}_{C}( \Gamma )  \, \cup \,  \token{FC}( \Gamma ) .
          \]
          If $\delta_{{\mathrm{3}}} \, \in \,  \token{Dom}_{C}( \Gamma ) $, the side condition is immediate.  If
          $\delta_{{\mathrm{3}}} \, \in \, \refenvsym{\{}   \overrightarrow{ \gamma_{{\mathrm{1}}} }   \refenvsym{,}  \gamma_{{\mathrm{2}}}  \refenvsym{\}}$, it is also immediate by taking
          $\gamma_{{\mathrm{3}}} = \delta_{{\mathrm{3}}}$ and using reflexivity.  Finally, if
          $\delta_{{\mathrm{3}}} \, \in \,  \token{FC}( \Gamma ) $, then
          \zcref{claim:cls-upper-bound-wrt-gtrans-2} gives some
          $\gamma_{{\mathrm{3}}} \, \in \, \refenvsym{\{}   \overrightarrow{ \gamma_{{\mathrm{1}}} }   \refenvsym{,}  \gamma_{{\mathrm{2}}}  \refenvsym{\}}$ such that
          $ \Psi \mid^{  \overrightarrow{ \gamma_{{\mathrm{1}}} }   \refenvsym{,}  \gamma_{{\mathrm{2}}} } \Gamma \vdash \delta_{{\mathrm{3}}} \subseteq \gamma_{{\mathrm{3}}} $.
          Thus the side condition holds in all cases, and
          \zcref{item:demotion-var:ltrans} gives the demoted reachability
          premise.  The lookup premise is preserved by classifier
          substitution.  Reapplying \ref{rule:runtime-type-var} gives the
          required typing judgment.

        \item[Case \textmd{\ref{rule:runtime-type-reserved-var}}:]
          By inversion, the expression is a variable $\refenvmv{z}$,
          $\token{lookup} \, \refenvsym{(}  \Gamma  \refenvsym{,}  \refenvmv{z}  \refenvsym{)} =  \token{Fail} $, and since the renaming environment
          is $ \token{id} $, the reserved-name premise is
          $ \binder{ \refenvmv{z} }: \refenvnt{A_{{\mathrm{2}}}} \mathrel{@}\binder{ \delta_{{\mathrm{1}}} } \mathbin{:\succeq} \delta_{{\mathrm{2}}}  \, \in \, \Psi$. 
          If\/ $\refenvmv{z} = \refenvmv{x}$, then this premise is the distinguished
          declaration $ \binder{ \refenvmv{x} }: \refenvnt{A_{{\mathrm{1}}}} \mathrel{@}\binder{ \gamma_{{\mathrm{2}}} } \mathbin{:\succeq} \gamma_{{\mathrm{4}}}  \, \in \, \Psi$. Then we have
          \[
             \Psi \mid^{  \overrightarrow{ \gamma_{{\mathrm{1}}} }   \refenvsym{,}  \gamma_{{\mathrm{2}}} } \Gamma \vdash^{  \overrightarrow{ \delta_{{\mathrm{2}}} }   \refenvsym{,}  \delta_{{\mathrm{3}}} }\token{wf} 
            \quad\text{and}\quad
             \Psi \mid^{  \overrightarrow{ \gamma_{{\mathrm{1}}} }   \refenvsym{,}  \gamma_{{\mathrm{2}}} } \Gamma \vdash \gamma_{{\mathrm{2}}} \preceq \delta_{{\mathrm{3}}} .
          \]
          We first check the side condition needed to apply
          \zcref{item:demotion-var:ltrans}.  By
          \zcref{claim:ctx-output-classifier-origin},
          \[
            \delta_{{\mathrm{3}}} \, \in \, \refenvsym{\{}   \overrightarrow{ \gamma_{{\mathrm{1}}} }   \refenvsym{,}  \gamma_{{\mathrm{2}}}  \refenvsym{\}} \, \cup \,  \token{Dom}_{C}( \Gamma )  \, \cup \,  \token{FC}( \Gamma ) .
          \]
          If $\delta_{{\mathrm{3}}} \, \in \,  \token{Dom}_{C}( \Gamma ) $, the side condition is immediate.  If
          $\delta_{{\mathrm{3}}} \, \in \, \refenvsym{\{}   \overrightarrow{ \gamma_{{\mathrm{1}}} }   \refenvsym{,}  \gamma_{{\mathrm{2}}}  \refenvsym{\}}$, it is also immediate by taking
          $\gamma_{{\mathrm{3}}} = \delta_{{\mathrm{3}}}$ and using reflexivity.  Finally, if
          $\delta_{{\mathrm{3}}} \, \in \,  \token{FC}( \Gamma ) $, then
          \zcref{claim:cls-upper-bound-wrt-gtrans-2} gives some
          $\gamma_{{\mathrm{3}}} \, \in \, \refenvsym{\{}   \overrightarrow{ \gamma_{{\mathrm{1}}} }   \refenvsym{,}  \gamma_{{\mathrm{2}}}  \refenvsym{\}}$ such that
          $ \Psi \mid^{  \overrightarrow{ \gamma_{{\mathrm{1}}} }   \refenvsym{,}  \gamma_{{\mathrm{2}}} } \Gamma \vdash \delta_{{\mathrm{3}}} \subseteq \gamma_{{\mathrm{3}}} $.
          Thus the side condition holds in all cases, and
          \zcref{item:demotion-var:ltrans} gives
          \[
             \Psi \mid^{  \overrightarrow{ \gamma_{{\mathrm{1}}} }   \refenvsym{,}  \gamma_{{\mathrm{4}}} }  \binder{ \refenvmv{x} }\mathord{:^{\binder{ \gamma_{{\mathrm{5}}} } } } \refenvnt{A_{{\mathrm{1}}}}  \refenvsym{[}  \gamma_{{\mathrm{2}}}  \coloneqq  \gamma_{{\mathrm{5}}}  \refenvsym{]}   \refenvsym{,}  \Gamma  \refenvsym{[}  \gamma_{{\mathrm{2}}}  \coloneqq  \gamma_{{\mathrm{5}}}  \refenvsym{]} \vdash \gamma_{{\mathrm{5}}} \preceq \delta_{{\mathrm{3}}}  \refenvsym{[}  \gamma_{{\mathrm{2}}}  \coloneqq  \gamma_{{\mathrm{5}}}  \refenvsym{]} .
          \]
          Moreover, \zcref{item:demotion-var:ctxwf} gives the demoted context
          well-formedness premise, and the demoted context contains the
          ordinary binding $ \binder{ \refenvmv{x} }\mathord{:^{\binder{ \gamma_{{\mathrm{5}}} } } } \refenvnt{A_{{\mathrm{1}}}}  \refenvsym{[}  \gamma_{{\mathrm{2}}}  \coloneqq  \gamma_{{\mathrm{5}}}  \refenvsym{]} $.  Reapplying
          \ref{rule:runtime-type-var} yields the desired judgment.

          If\/ $\refenvmv{z} \neq \refenvmv{x}$, the same reserved-name declaration remains
          available in $\Psi$.  The context well-formedness premise is
          preserved by \zcref{item:demotion-var:ctxwf}.  The reachability premise
          is preserved by \zcref{item:demotion-var:ltrans}, using
          \zcref{claim:ctx-output-classifier-origin} for the side condition on
          the output classifier.  Reapplying
          \ref{rule:runtime-type-reserved-var} yields the desired judgment.

        \item[Case \textmd{\ref{rule:runtime-type-splice}}:]
          By inversion, the derivation gives premises
          \[
             \Psi \mid^{  \overrightarrow{ \gamma_{{\mathrm{1}}} }   \refenvsym{,}  \gamma_{{\mathrm{2}}} } \Gamma \vdash^{  \overrightarrow{ \delta_{{\mathrm{1}}} }   \refenvsym{,}    \delta _{ 0 }  ,\dotsc,  \delta _{ \refenvnt{k} }   }\token{wf} ,
          \]
          \[
             \Psi \mid^{  \overrightarrow{ \gamma_{{\mathrm{1}}} }   \refenvsym{,}  \gamma_{{\mathrm{2}}} }  \Gamma  \refenvsym{,}   \blacktriangleleft _{ \refenvnt{k} }^{\binder{ \delta_{{\mathrm{4}}} } }  \vdash^{  \overrightarrow{ \delta_{{\mathrm{1}}} }   \refenvsym{,}  \delta_{{\mathrm{4}}} }_{  \token{id}  }  \refenvnt{e} :  \langle \refenvnt{A_{{\mathrm{3}}}} \rangle^{ \delta_{{\mathrm{5}}} }  
          \]
          and
          $ \Psi \mid^{  \overrightarrow{ \gamma_{{\mathrm{1}}} }   \refenvsym{,}  \gamma_{{\mathrm{2}}} } \Gamma \vdash \delta_{{\mathrm{5}}} \preceq  \delta _{ \refenvnt{k} }  $.
          By \zcref{item:demotion-var:ctxwf}, the context well-formedness
          premise is preserved.  Applying the induction hypothesis to the body
          typing premise gives the demoted body typing judgment under
          $\Gamma  \refenvsym{[}  \gamma_{{\mathrm{2}}}  \coloneqq  \gamma_{{\mathrm{5}}}  \refenvsym{]}  \refenvsym{,}   \blacktriangleleft _{ \refenvnt{k} }^{\binder{ \delta_{{\mathrm{4}}} } } $.
          Finally, we check the side condition needed to demote the
          reachability premise $ \delta_{{\mathrm{5}}} \preceq  \delta _{ \refenvnt{k} }  $.  By
          \zcref{claim:ctx-output-classifier-origin},
          \[
             \delta _{ \refenvnt{k} }  \, \in \, \refenvsym{\{}   \overrightarrow{ \gamma_{{\mathrm{1}}} }   \refenvsym{,}  \gamma_{{\mathrm{2}}}  \refenvsym{\}} \, \cup \,  \token{Dom}_{C}( \Gamma )  \, \cup \,  \token{FC}( \Gamma ) .
          \]
          If $ \delta _{ \refenvnt{k} }  \, \in \,  \token{Dom}_{C}( \Gamma ) $, the side condition is immediate.  If
          $ \delta _{ \refenvnt{k} }  \, \in \, \refenvsym{\{}   \overrightarrow{ \gamma_{{\mathrm{1}}} }   \refenvsym{,}  \gamma_{{\mathrm{2}}}  \refenvsym{\}}$, it is also immediate by taking
          $\gamma_{{\mathrm{3}}} =  \delta _{ \refenvnt{k} } $ and using reflexivity.  Finally, if
          $ \delta _{ \refenvnt{k} }  \, \in \,  \token{FC}( \Gamma ) $, then
          \zcref{claim:cls-upper-bound-wrt-gtrans-2} gives some
          $\gamma_{{\mathrm{3}}} \, \in \, \refenvsym{\{}   \overrightarrow{ \gamma_{{\mathrm{1}}} }   \refenvsym{,}  \gamma_{{\mathrm{2}}}  \refenvsym{\}}$ such that
          $ \Psi \mid^{  \overrightarrow{ \gamma_{{\mathrm{1}}} }   \refenvsym{,}  \gamma_{{\mathrm{2}}} } \Gamma \vdash  \delta _{ \refenvnt{k} }  \subseteq \gamma_{{\mathrm{3}}} $.
          Thus the side condition holds in all cases, and
          \zcref{item:demotion-var:ltrans} preserves the reachability premise
          $ \delta_{{\mathrm{5}}} \preceq  \delta _{ \refenvnt{k} }  $.  Reapplying
          \ref{rule:runtime-type-splice} gives the desired typing judgment.
      \end{description}
  \end{description}
\end{proof}

\begin{lemma}[Demotion for $ \blacktriangleright $]\label{claim:demotion-open}
  Suppose $\Psi  \vdash  \gamma_{{\mathrm{3}}}  \subseteq  \gamma_{{\mathrm{2}}}$.
  \begin{enumerate}
    \item \label{item:demotion-open:ctxwf}
          If\/ $ \Psi \mid^{  \overrightarrow{ \gamma_{{\mathrm{1}}} }^{+}   \refenvsym{,}  \gamma_{{\mathrm{2}}}  \refenvsym{,}  \gamma_{{\mathrm{3}}} } \Gamma \vdash^{  \overrightarrow{ \gamma_{{\mathrm{4}}} }^{+}  }\token{wf} $,
          then $ \Psi \mid^{  \overrightarrow{ \gamma_{{\mathrm{1}}} }^{+}   \refenvsym{,}  \gamma_{{\mathrm{2}}} }  \blacktriangleright ^{ \gamma_{{\mathrm{3}}} }   \refenvsym{,}  \Gamma \vdash^{  \overrightarrow{ \gamma_{{\mathrm{4}}} }^{+}  }\token{wf} $.
    \item \label{item:demotion-open:typwf}
          If\/ $ \Psi \mid^{  \overrightarrow{ \gamma_{{\mathrm{1}}} }^{+}   \refenvsym{,}  \gamma_{{\mathrm{2}}}  \refenvsym{,}  \gamma_{{\mathrm{3}}} }  \Gamma \vdash ^{  \overrightarrow{ \gamma_{{\mathrm{4}}} }^{+}  } \refenvnt{A} \ \token{wf} $,
          then $ \Psi \mid^{  \overrightarrow{ \gamma_{{\mathrm{1}}} }^{+}   \refenvsym{,}  \gamma_{{\mathrm{2}}} }   \blacktriangleright ^{ \gamma_{{\mathrm{3}}} }   \refenvsym{,}  \Gamma \vdash ^{  \overrightarrow{ \gamma_{{\mathrm{4}}} }^{+}  } \refenvnt{A} \ \token{wf} $.
    \item \label{item:demotion-open:ltrans}
          If\/ $ \Psi \mid^{  \overrightarrow{ \gamma_{{\mathrm{1}}} }^{+}   \refenvsym{,}  \gamma_{{\mathrm{2}}}  \refenvsym{,}  \gamma_{{\mathrm{3}}} } \Gamma \vdash \gamma_{{\mathrm{4}}} \preceq \gamma_{{\mathrm{5}}} $
          and either $\gamma_{{\mathrm{5}}} \, \in \,  \token{Dom}_{C}( \Gamma ) $ or $\Psi  \vdash  \gamma_{{\mathrm{5}}}  \subseteq  \gamma_{{\mathrm{3}}}$,
          then $ \Psi \mid^{  \overrightarrow{ \gamma_{{\mathrm{1}}} }^{+}   \refenvsym{,}  \gamma_{{\mathrm{2}}} }  \blacktriangleright ^{ \gamma_{{\mathrm{3}}} }   \refenvsym{,}  \Gamma \vdash \gamma_{{\mathrm{4}}} \preceq \gamma_{{\mathrm{5}}} $.
    \item \label{item:demotion-open:gtrans}
          If\/ $ \Psi \mid^{  \overrightarrow{ \gamma_{{\mathrm{1}}} }^{+}   \refenvsym{,}  \gamma_{{\mathrm{2}}}  \refenvsym{,}  \gamma_{{\mathrm{3}}} } \Gamma \vdash \gamma_{{\mathrm{4}}} \subseteq \gamma_{{\mathrm{5}}} $
          and either $\gamma_{{\mathrm{5}}} \, \in \,  \token{Dom}_{C}( \Gamma ) $ or $\Psi  \vdash  \gamma_{{\mathrm{5}}}  \subseteq  \gamma_{{\mathrm{3}}}$,
          then $ \Psi \mid^{  \overrightarrow{ \gamma_{{\mathrm{1}}} }^{+}   \refenvsym{,}  \gamma_{{\mathrm{2}}} }  \blacktriangleright ^{ \gamma_{{\mathrm{3}}} }   \refenvsym{,}  \Gamma \vdash \gamma_{{\mathrm{4}}} \subseteq \gamma_{{\mathrm{5}}} $.
    \item \label{item:demotion-open:typing}
          If\/ $ \Psi \mid^{  \overrightarrow{ \gamma_{{\mathrm{1}}} }^{+}   \refenvsym{,}  \gamma_{{\mathrm{2}}}  \refenvsym{,}  \gamma_{{\mathrm{3}}} }  \Gamma \vdash^{  \overrightarrow{ \gamma_{{\mathrm{4}}} }^{+}  }_{  \token{id}  }  \refenvnt{e} : \refenvnt{A} $,
          then $ \Psi \mid^{  \overrightarrow{ \gamma_{{\mathrm{1}}} }^{+}   \refenvsym{,}  \gamma_{{\mathrm{2}}} }   \blacktriangleright ^{ \gamma_{{\mathrm{3}}} }   \refenvsym{,}  \Gamma \vdash^{  \overrightarrow{ \gamma_{{\mathrm{4}}} }^{+}  }_{  \token{id}  }  \refenvnt{e} : \refenvnt{A} $.
  \end{enumerate}
\end{lemma}

\begin{proof}
  By mutual induction on the given derivation.
\end{proof}

\begin{lemma}[Demotion for $ \blacktriangleleft $]\label{claim:demotion-shut}
  Suppose
  $ \binder{ \gamma_{{\mathrm{2}}} }( \mathbin{:\succeq} \;  \delta _{ 0 }   /  \mathbin{:\supseteq} \;  \delta _{ \refenvnt{k} }  )  \, \in \, \Psi$,
  $ \Psi \vdash  \overrightarrow{ \gamma_{{\mathrm{1}}} }  \mathrel{\#} \gamma_{{\mathrm{2}}} $,
  and $\gamma_{{\mathrm{4}}} \, \not\in \,  \token{Dom}_{C}( \Psi )  \, \cup \,  \token{Dom}_{C}( \Gamma ) $.
  \begin{enumerate}
    \item \label{item:demotion-shut:ctxwf}
          If\/ $ \Psi \mid^{  \overrightarrow{ \gamma_{{\mathrm{1}}} }   \refenvsym{,}  \gamma_{{\mathrm{2}}} } \Gamma \vdash^{  \overrightarrow{ \gamma_{{\mathrm{3}}} }^{+}  }\token{wf} $,
          then
          $ \Psi \mid^{  \overrightarrow{ \gamma_{{\mathrm{1}}} }   \refenvsym{,}    \delta _{ 0 }  ,\dotsc,  \delta _{ \refenvnt{k} }   }  \blacktriangleleft _{ \refenvnt{k} }^{\binder{ \gamma_{{\mathrm{4}}} } }   \refenvsym{,}  \Gamma  \refenvsym{[}  \gamma_{{\mathrm{2}}}  \coloneqq  \gamma_{{\mathrm{4}}}  \refenvsym{]} \vdash^{   \overrightarrow{ \gamma_{{\mathrm{3}}} }^{+}    \refenvsym{[}  \gamma_{{\mathrm{2}}}  \coloneqq  \gamma_{{\mathrm{4}}}  \refenvsym{]} }\token{wf} $.
    \item \label{item:demotion-shut:typwf}
          If\/ $ \Psi \mid^{  \overrightarrow{ \gamma_{{\mathrm{1}}} }   \refenvsym{,}  \gamma_{{\mathrm{2}}} }  \Gamma \vdash ^{  \overrightarrow{ \gamma_{{\mathrm{3}}} }^{+}  } \refenvnt{A} \ \token{wf} $,
          then
          $ \Psi \mid^{  \overrightarrow{ \gamma_{{\mathrm{1}}} }   \refenvsym{,}    \delta _{ 0 }  ,\dotsc,  \delta _{ \refenvnt{k} }   }   \blacktriangleleft _{ \refenvnt{k} }^{\binder{ \gamma_{{\mathrm{4}}} } }   \refenvsym{,}  \Gamma  \refenvsym{[}  \gamma_{{\mathrm{2}}}  \coloneqq  \gamma_{{\mathrm{4}}}  \refenvsym{]} \vdash ^{   \overrightarrow{ \gamma_{{\mathrm{3}}} }^{+}    \refenvsym{[}  \gamma_{{\mathrm{2}}}  \coloneqq  \gamma_{{\mathrm{4}}}  \refenvsym{]} } \refenvnt{A}  \refenvsym{[}  \gamma_{{\mathrm{2}}}  \coloneqq  \gamma_{{\mathrm{4}}}  \refenvsym{]} \ \token{wf} $.
    \item \label{item:demotion-shut:ltrans}
          If\/ $ \Psi \mid^{  \overrightarrow{ \gamma_{{\mathrm{1}}} }   \refenvsym{,}  \gamma_{{\mathrm{2}}} } \Gamma \vdash \gamma_{{\mathrm{5}}} \preceq \gamma_{{\mathrm{6}}} $
          and either $\gamma_{{\mathrm{6}}} \, \in \,  \token{Dom}_{C}( \Gamma ) $ or there exists $\gamma_{{\mathrm{7}}} \, \in \, \refenvsym{\{}   \overrightarrow{ \gamma_{{\mathrm{1}}} }   \refenvsym{,}  \gamma_{{\mathrm{2}}}  \refenvsym{\}}$ such that $ \Psi \mid^{  \overrightarrow{ \gamma_{{\mathrm{1}}} }   \refenvsym{,}  \gamma_{{\mathrm{2}}} } \Gamma \vdash \gamma_{{\mathrm{6}}} \subseteq \gamma_{{\mathrm{7}}} $,
          then
          $ \Psi \mid^{  \overrightarrow{ \gamma_{{\mathrm{1}}} }   \refenvsym{,}    \delta _{ 0 }  ,\dotsc,  \delta _{ \refenvnt{k} }   }  \blacktriangleleft _{ \refenvnt{k} }^{\binder{ \gamma_{{\mathrm{4}}} } }   \refenvsym{,}  \Gamma  \refenvsym{[}  \gamma_{{\mathrm{2}}}  \coloneqq  \gamma_{{\mathrm{4}}}  \refenvsym{]} \vdash \gamma_{{\mathrm{5}}}  \refenvsym{[}  \gamma_{{\mathrm{2}}}  \coloneqq  \gamma_{{\mathrm{4}}}  \refenvsym{]} \preceq \gamma_{{\mathrm{6}}}  \refenvsym{[}  \gamma_{{\mathrm{2}}}  \coloneqq  \gamma_{{\mathrm{4}}}  \refenvsym{]} $.
    \item \label{item:demotion-shut:gtrans}
          If\/ $ \Psi \mid^{  \overrightarrow{ \gamma_{{\mathrm{1}}} }   \refenvsym{,}  \gamma_{{\mathrm{2}}} } \Gamma \vdash \gamma_{{\mathrm{5}}} \subseteq \gamma_{{\mathrm{6}}} $
          and either $\gamma_{{\mathrm{6}}} \, \in \,  \token{Dom}_{C}( \Gamma ) $ or there exists $\gamma_{{\mathrm{7}}} \, \in \, \refenvsym{\{}   \overrightarrow{ \gamma_{{\mathrm{1}}} }   \refenvsym{,}  \gamma_{{\mathrm{2}}}  \refenvsym{\}}$ such that $ \Psi \mid^{  \overrightarrow{ \gamma_{{\mathrm{1}}} }   \refenvsym{,}  \gamma_{{\mathrm{2}}} } \Gamma \vdash \gamma_{{\mathrm{6}}} \subseteq \gamma_{{\mathrm{7}}} $,
          then
          $ \Psi \mid^{  \overrightarrow{ \gamma_{{\mathrm{1}}} }   \refenvsym{,}    \delta _{ 0 }  ,\dotsc,  \delta _{ \refenvnt{k} }   }  \blacktriangleleft _{ \refenvnt{k} }^{\binder{ \gamma_{{\mathrm{4}}} } }   \refenvsym{,}  \Gamma  \refenvsym{[}  \gamma_{{\mathrm{2}}}  \coloneqq  \gamma_{{\mathrm{4}}}  \refenvsym{]} \vdash \gamma_{{\mathrm{5}}}  \refenvsym{[}  \gamma_{{\mathrm{2}}}  \coloneqq  \gamma_{{\mathrm{4}}}  \refenvsym{]} \subseteq \gamma_{{\mathrm{6}}}  \refenvsym{[}  \gamma_{{\mathrm{2}}}  \coloneqq  \gamma_{{\mathrm{4}}}  \refenvsym{]} $.
    \item \label{item:demotion-shut:typing}
          If\/ $ \Psi \mid^{  \overrightarrow{ \gamma_{{\mathrm{1}}} }   \refenvsym{,}  \gamma_{{\mathrm{2}}} }  \Gamma \vdash^{  \overrightarrow{ \gamma_{{\mathrm{3}}} }^{+}  }_{  \token{id}  }  \refenvnt{e} : \refenvnt{A} $,
          then
          $ \Psi \mid^{  \overrightarrow{ \gamma_{{\mathrm{1}}} }   \refenvsym{,}    \delta _{ 0 }  ,\dotsc,  \delta _{ \refenvnt{k} }   }   \blacktriangleleft _{ \refenvnt{k} }^{\binder{ \gamma_{{\mathrm{4}}} } }   \refenvsym{,}  \Gamma  \refenvsym{[}  \gamma_{{\mathrm{2}}}  \coloneqq  \gamma_{{\mathrm{4}}}  \refenvsym{]} \vdash^{   \overrightarrow{ \gamma_{{\mathrm{3}}} }^{+}    \refenvsym{[}  \gamma_{{\mathrm{2}}}  \coloneqq  \gamma_{{\mathrm{4}}}  \refenvsym{]} }_{  \token{id}  }  \refenvnt{e} : \refenvnt{A}  \refenvsym{[}  \gamma_{{\mathrm{2}}}  \coloneqq  \gamma_{{\mathrm{4}}}  \refenvsym{]} $.
  \end{enumerate}
\end{lemma}

\begin{proof}
  We proceed by mutual induction on the given derivation.  The proof follows
  the same pattern as \zcref{claim:demotion-var}; we record the points where
  the $ \blacktriangleleft $ entry is used.
  \begin{description}
    \item[Case \textmd{\zcref{item:demotion-shut:ctxwf}}:]
      By induction on the context well-formedness derivation.  The case for
      \ref{rule:runtime-wf-ctx-open} is the only one that uses a visibility
      premise.  By inversion, the last rule gives premises
      \[
         \Psi \mid^{  \overrightarrow{ \gamma_{{\mathrm{1}}} }   \refenvsym{,}  \gamma_{{\mathrm{2}}} } \Gamma_{{\mathrm{1}}} \vdash^{  \overrightarrow{ \delta'_{{\mathrm{1}}} }   \refenvsym{,}  \delta'_{{\mathrm{2}}} }\token{wf} 
        \quad\text{and}\quad
         \Psi \mid^{  \overrightarrow{ \gamma_{{\mathrm{1}}} }   \refenvsym{,}  \gamma_{{\mathrm{2}}} } \Gamma_{{\mathrm{1}}} \vdash \delta'_{{\mathrm{3}}} \subseteq \delta'_{{\mathrm{2}}} .
      \]
      The induction hypothesis gives the demoted well-formedness of
      $\Gamma_{{\mathrm{1}}}$.  By \zcref{claim:ctx-output-classifier-origin},
      $\delta'_{{\mathrm{2}}} \, \in \, \refenvsym{\{}   \overrightarrow{ \gamma_{{\mathrm{1}}} }   \refenvsym{,}  \gamma_{{\mathrm{2}}}  \refenvsym{\}} \, \cup \,  \token{Dom}_{C}( \Gamma_{{\mathrm{1}}} )  \, \cup \,  \token{FC}( \Gamma_{{\mathrm{1}}} ) $, so
      \zcref{item:demotion-shut:gtrans}
      gives the demoted visibility premise.
      Reapplying \ref{rule:runtime-wf-ctx-open} completes the case.

    \item[Case \textmd{\zcref{item:demotion-shut:typwf}}:]
      By induction on the type well-formedness derivation.

    \item[Case \textmd{\zcref{item:demotion-shut:ltrans}}:]
      This case is analogous to \zcref{item:demotion-shut:gtrans}, using the
      rules and inversion principles for $ \preceq $ in place of those for
      $ \subseteq $.

    \item[Case \textmd{\zcref{item:demotion-shut:gtrans}}:]
      By induction with respect to $ \token{deg} ( \Psi , \Gamma , \gamma_{{\mathrm{6}}} ) $.
      By the side condition of the lemma, either
      $\gamma_{{\mathrm{6}}} \, \in \,  \token{Dom}_{C}( \Gamma ) $ or
      there exists $\gamma_{{\mathrm{7}}} \, \in \, \refenvsym{\{}   \overrightarrow{ \gamma_{{\mathrm{1}}} }   \refenvsym{,}  \gamma_{{\mathrm{2}}}  \refenvsym{\}}$ such that
      $ \Psi \mid^{  \overrightarrow{ \gamma_{{\mathrm{1}}} }   \refenvsym{,}  \gamma_{{\mathrm{2}}} } \Gamma \vdash \gamma_{{\mathrm{6}}} \subseteq \gamma_{{\mathrm{7}}} $.

      We first handle the case
      $\gamma_{{\mathrm{6}}} \, \not\in \,  \token{Dom}_{C}( \Gamma ) $.
      Then  there exists $\gamma_{{\mathrm{7}}} \, \in \, \refenvsym{\{}   \overrightarrow{ \gamma_{{\mathrm{1}}} }   \refenvsym{,}  \gamma_{{\mathrm{2}}}  \refenvsym{\}}$ such that
      $ \Psi \mid^{  \overrightarrow{ \gamma_{{\mathrm{1}}} }   \refenvsym{,}  \gamma_{{\mathrm{2}}} } \Gamma \vdash \gamma_{{\mathrm{6}}} \subseteq \gamma_{{\mathrm{7}}} $.
      We have $\gamma_{{\mathrm{6}}} \, \in \,  \token{Dom}_{C}( \Psi ) $ by regularity; hence
      $\Psi  \vdash  \gamma_{{\mathrm{5}}}  \subseteq  \gamma_{{\mathrm{6}}}$ by \zcref{claim:local-to-global-trans}.
      Moreover, regularity and \zcref{item:demotion-shut:ctxwf} give
      \[
         \Psi \mid^{  \overrightarrow{ \gamma_{{\mathrm{1}}} }   \refenvsym{,}    \delta _{ 0 }  ,\dotsc,  \delta _{ \refenvnt{k} }   }  \blacktriangleleft _{ \refenvnt{k} }^{\binder{ \gamma_{{\mathrm{4}}} } }   \refenvsym{,}  \Gamma  \refenvsym{[}  \gamma_{{\mathrm{2}}}  \coloneqq  \gamma_{{\mathrm{4}}}  \refenvsym{]} \vdash^{  \dotsc  }\token{wf} .
      \]
      Therefore, by \zcref{claim:global-to-local-trans},
      \[
         \Psi \mid^{  \overrightarrow{ \gamma_{{\mathrm{1}}} }   \refenvsym{,}    \delta _{ 0 }  ,\dotsc,  \delta _{ \refenvnt{k} }   }  \blacktriangleleft _{ \refenvnt{k} }^{\binder{ \gamma_{{\mathrm{4}}} } }   \refenvsym{,}  \Gamma  \refenvsym{[}  \gamma_{{\mathrm{2}}}  \coloneqq  \gamma_{{\mathrm{4}}}  \refenvsym{]} \vdash \gamma_{{\mathrm{5}}} \subseteq \gamma_{{\mathrm{6}}} .
      \]
      We conclude by cases on whether the substitution $\gamma_{{\mathrm{2}}}  \coloneqq  \gamma_{{\mathrm{4}}}$ affects
      $\gamma_{{\mathrm{5}}}$ or $\gamma_{{\mathrm{6}}}$.
      \begin{description}
        \item[Case \textmd{$\gamma_{{\mathrm{2}}} \neq \gamma_{{\mathrm{5}}}$ and $\gamma_{{\mathrm{2}}} \neq \gamma_{{\mathrm{6}}}$}:]
          The substitution leaves both endpoints unchanged, so the required
          judgment follows immediately.

        \item[Case \textmd{$\gamma_{{\mathrm{2}}} \neq \gamma_{{\mathrm{5}}}$ and $\gamma_{{\mathrm{2}}} = \gamma_{{\mathrm{6}}}$}:]
          By \zcref{claim:inversion-runtime-gtrans-nht} and
          $ \binder{ \gamma_{{\mathrm{2}}} }( \mathbin{:\succeq} \;  \delta _{ 0 }   /  \mathbin{:\supseteq} \;  \delta _{ \refenvnt{k} }  )  \, \in \, \Psi$, we have
          $\Psi  \vdash  \gamma_{{\mathrm{5}}}  \subseteq   \delta _{ 0 } $ or $\Psi  \vdash  \gamma_{{\mathrm{5}}}  \subseteq   \delta _{ \refenvnt{k} } $.
          By \zcref{claim:global-to-local-trans}, the corresponding judgment
          holds in the demoted context.  If the intermediate classifier is
          $ \delta _{ 0 } $, then \ref{rule:runtime-ltrans-shut} followed by
          \ref{rule:runtime-gtrans-lift} gives
          \[
             \Psi \mid^{  \overrightarrow{ \gamma_{{\mathrm{1}}} }   \refenvsym{,}    \delta _{ 0 }  ,\dotsc,  \delta _{ \refenvnt{k} }   }  \blacktriangleleft _{ \refenvnt{k} }^{\binder{ \gamma_{{\mathrm{4}}} } }   \refenvsym{,}  \Gamma  \refenvsym{[}  \gamma_{{\mathrm{2}}}  \coloneqq  \gamma_{{\mathrm{4}}}  \refenvsym{]} \vdash  \delta _{ 0 }  \subseteq \gamma_{{\mathrm{4}}} .
          \]
          If the intermediate classifier is $ \delta _{ \refenvnt{k} } $, then
          \ref{rule:runtime-gtrans-shut-ctx} gives
          \[
             \Psi \mid^{  \overrightarrow{ \gamma_{{\mathrm{1}}} }   \refenvsym{,}    \delta _{ 0 }  ,\dotsc,  \delta _{ \refenvnt{k} }   }  \blacktriangleleft _{ \refenvnt{k} }^{\binder{ \gamma_{{\mathrm{4}}} } }   \refenvsym{,}  \Gamma  \refenvsym{[}  \gamma_{{\mathrm{2}}}  \coloneqq  \gamma_{{\mathrm{4}}}  \refenvsym{]} \vdash  \delta _{ \refenvnt{k} }  \subseteq \gamma_{{\mathrm{4}}} .
          \]
          In either subcase, the conclusion follows by
          \ref{rule:runtime-gtrans-trans}.

        \item[Case \textmd{$\gamma_{{\mathrm{2}}} = \gamma_{{\mathrm{5}}} = \gamma_{{\mathrm{6}}}$}:]
          Then
          $\gamma_{{\mathrm{5}}}  \refenvsym{[}  \gamma_{{\mathrm{2}}}  \coloneqq  \gamma_{{\mathrm{4}}}  \refenvsym{]} = \gamma_{{\mathrm{6}}}  \refenvsym{[}  \gamma_{{\mathrm{2}}}  \coloneqq  \gamma_{{\mathrm{4}}}  \refenvsym{]} = \gamma_{{\mathrm{4}}}$.
          The required judgment follows from
          \ref{rule:runtime-ltrans-refl} and \ref{rule:runtime-gtrans-lift}.

        \item[Case \textmd{$\gamma_{{\mathrm{2}}} = \gamma_{{\mathrm{5}}}$ and $\gamma_{{\mathrm{2}}} \neq \gamma_{{\mathrm{6}}}$}:]
          Since $\gamma_{{\mathrm{5}}} = \gamma_{{\mathrm{2}}}$, we have
          $\Psi  \vdash  \gamma_{{\mathrm{2}}}  \subseteq  \gamma_{{\mathrm{6}}}$.
          Moreover, for some $\gamma_{{\mathrm{7}}} \, \in \, \refenvsym{\{}   \overrightarrow{ \gamma_{{\mathrm{1}}} }   \refenvsym{,}  \gamma_{{\mathrm{2}}}  \refenvsym{\}}$ we have
          $ \Psi \mid^{  \overrightarrow{ \gamma_{{\mathrm{1}}} }   \refenvsym{,}  \gamma_{{\mathrm{2}}} } \Gamma \vdash \gamma_{{\mathrm{6}}} \subseteq \gamma_{{\mathrm{7}}} $.
          By \zcref{claim:local-to-global-trans}, this gives
          $\Psi  \vdash  \gamma_{{\mathrm{6}}}  \subseteq  \gamma_{{\mathrm{7}}}$; together with
          $\Psi  \vdash  \gamma_{{\mathrm{2}}}  \subseteq  \gamma_{{\mathrm{6}}}$ and \ref{rule:runtime-gtrans-trans}, we get
          $\Psi  \vdash  \gamma_{{\mathrm{2}}}  \subseteq  \gamma_{{\mathrm{7}}}$.
          Since $ \Psi \vdash  \overrightarrow{ \gamma_{{\mathrm{1}}} }  \mathrel{\#} \gamma_{{\mathrm{2}}} $, the only possible such
          $\gamma_{{\mathrm{7}}}$ is $\gamma_{{\mathrm{2}}}$.  Hence
          $\Psi  \vdash  \gamma_{{\mathrm{6}}}  \subseteq  \gamma_{{\mathrm{2}}}$.
          Applying \zcref{claim:trans-antisymmetry} to
          $\Psi  \vdash  \gamma_{{\mathrm{2}}}  \subseteq  \gamma_{{\mathrm{6}}}$ and $\Psi  \vdash  \gamma_{{\mathrm{6}}}  \subseteq  \gamma_{{\mathrm{2}}}$ yields
          $\gamma_{{\mathrm{2}}} = \gamma_{{\mathrm{6}}}$, contradicting the case assumption.  Thus
          this case is impossible.
      \end{description}

      It remains to consider the case $\gamma_{{\mathrm{6}}} \, \in \,  \token{Dom}_{C}( \Gamma ) $.  If
      $\gamma_{{\mathrm{5}}} = \gamma_{{\mathrm{6}}}$, then $\gamma_{{\mathrm{6}}}  \refenvsym{[}  \gamma_{{\mathrm{2}}}  \coloneqq  \gamma_{{\mathrm{4}}}  \refenvsym{]}$ is declared in the
      demoted context by \zcref{item:demotion-shut:ctxwf}.  Hence the desired
      judgment follows from \ref{rule:runtime-ltrans-refl} and
      \ref{rule:runtime-gtrans-lift}.  Thus assume $\gamma_{{\mathrm{5}}} \neq \gamma_{{\mathrm{6}}}$.
      We perform case analysis using
      \zcref{claim:inversion-runtime-gtrans-ctx}.  In each case, the inversion
      gives a derivation
      $ \Psi \mid^{  \overrightarrow{ \gamma_{{\mathrm{1}}} }   \refenvsym{,}  \gamma_{{\mathrm{2}}} } \Gamma \vdash \gamma_{{\mathrm{5}}} \subseteq \delta'_{{\mathrm{3}}} $
      where $ \token{deg} ( \Psi , \Gamma , \delta'_{{\mathrm{3}}} )  <  \token{deg} ( \Psi , \Gamma , \gamma_{{\mathrm{6}}} ) $
      and $\delta'_{{\mathrm{3}}} \, \in \, \refenvsym{\{}   \overrightarrow{ \gamma_{{\mathrm{1}}} }   \refenvsym{,}  \gamma_{{\mathrm{2}}}  \refenvsym{\}} \, \cup \,  \token{Dom}_{C}( \Gamma )  \, \cup \,  \token{FC}( \Gamma ) $.
      The membership condition follows from
      \zcref{claim:ctx-output-classifier-origin} when $\delta'_{{\mathrm{3}}}$ comes from
      the output stack of the corresponding context prefix.  In the remaining
      polymorphic-classifier declaration cases, $\delta'_{{\mathrm{3}}}$ appears as the
      right-hand side of a declaration $ \binder{ \gamma_{{\mathrm{6}}} }  \mathbin{:\succeq}   \delta'_{{\mathrm{3}}} $, so the condition
      follows from the definitions of $ \token{Dom}_{C}( \Gamma ) $ and $ \token{FC}( \Gamma ) $.
      Hence, the induction hypothesis gives
      \[
         \Psi \mid^{  \overrightarrow{ \gamma_{{\mathrm{1}}} }   \refenvsym{,}    \delta _{ 0 }  ,\dotsc,  \delta _{ \refenvnt{k} }   }  \blacktriangleleft _{ \refenvnt{k} }^{\binder{ \gamma_{{\mathrm{4}}} } }   \refenvsym{,}  \Gamma  \refenvsym{[}  \gamma_{{\mathrm{2}}}  \coloneqq  \gamma_{{\mathrm{4}}}  \refenvsym{]} \vdash \gamma_{{\mathrm{5}}}  \refenvsym{[}  \gamma_{{\mathrm{2}}}  \coloneqq  \gamma_{{\mathrm{4}}}  \refenvsym{]} \subseteq \delta'_{{\mathrm{3}}}  \refenvsym{[}  \gamma_{{\mathrm{2}}}  \coloneqq  \gamma_{{\mathrm{4}}}  \refenvsym{]} .
      \]
      Reapplying the corresponding context rule gives
      \[
         \Psi \mid^{  \overrightarrow{ \gamma_{{\mathrm{1}}} }   \refenvsym{,}    \delta _{ 0 }  ,\dotsc,  \delta _{ \refenvnt{k} }   }  \blacktriangleleft _{ \refenvnt{k} }^{\binder{ \gamma_{{\mathrm{4}}} } }   \refenvsym{,}  \Gamma  \refenvsym{[}  \gamma_{{\mathrm{2}}}  \coloneqq  \gamma_{{\mathrm{4}}}  \refenvsym{]} \vdash \delta'_{{\mathrm{3}}}  \refenvsym{[}  \gamma_{{\mathrm{2}}}  \coloneqq  \gamma_{{\mathrm{4}}}  \refenvsym{]} \subseteq \gamma_{{\mathrm{6}}}  \refenvsym{[}  \gamma_{{\mathrm{2}}}  \coloneqq  \gamma_{{\mathrm{4}}}  \refenvsym{]} .
      \]
      The desired judgment follows by \ref{rule:runtime-gtrans-trans}.

    \item[Case \textmd{\zcref{item:demotion-shut:typing}}:]
      By induction on the typing derivation.  The cases
      \ref{rule:runtime-type-var}, \ref{rule:runtime-type-reserved-var}, and
      \ref{rule:runtime-type-splice} are analogous to the corresponding cases
      in \zcref{claim:demotion-var}, using
      \zcref{item:demotion-shut:ctxwf} for
      context well-formedness and \zcref{item:demotion-shut:ltrans} for reachability premises.
  \end{description}
\end{proof}

\begin{lemma}[Demotion for Polymorphic Classifier Declarations]\label{claim:demotion-polyclsdecl}
  Let $\sigma =   \gamma _{ 0 }  \coloneqq  \delta' _{ 0 }  ,\dotsc,  \gamma _{ \refenvnt{k} }  \coloneqq  \delta' _{ \refenvnt{k} }  $.
  Suppose
  $ [    \binder{  \gamma _{ 0 }  }  \mathbin{:\succeq}    \gamma' _{ 0 }  ,\dotsc,\binder{  \gamma _{ \refenvnt{k} }  }  \mathbin{:\succeq}   \gamma'  _{ \refenvnt{k} }   ]  \, \in \, \Psi$,
  $ \Psi \vdash  \overrightarrow{ \delta_{{\mathrm{1}}} }^{+}  \mathrel{\#}   \gamma _{ 0 }  ,\dotsc,  \gamma _{ \refenvnt{k} }   $,
  and $ \delta' _{ \refenvnt{i} }  \, \not\in \,  \token{Dom}_{C}( \Psi )  \, \cup \,  \token{Dom}_{C}( \Gamma ) $ for $0 \le \refenvnt{i} \le \refenvnt{k}$.
  \begin{enumerate}
    \item \label{item:demotion-polyclsdecl:ctxwf}
          If\/ $ \Psi \mid^{  \overrightarrow{ \delta_{{\mathrm{1}}} }^{+}   \refenvsym{,}   \gamma _{ 0 }  } \Gamma \vdash^{  \overrightarrow{ \delta_{{\mathrm{2}}} }^{+}  }\token{wf} $,
          then
          $ \Psi \mid^{  \overrightarrow{ \delta_{{\mathrm{1}}} }^{+}   \refenvsym{,}   \gamma' _{ 0 }  }  [    \binder{  \delta' _{ 1 }  }  \mathbin{:\succeq}    \gamma' _{ 1 }  ,\dotsc,\binder{  \delta' _{ \refenvnt{k} }  }  \mathbin{:\succeq}   \gamma'  _{ \refenvnt{k} }   ]^{\binder{  \delta' _{ 0 }  } }   \refenvsym{,}  \Gamma  \refenvsym{[}  \sigma  \refenvsym{]} \vdash^{   \overrightarrow{ \delta_{{\mathrm{2}}} }^{+}    \refenvsym{[}  \sigma  \refenvsym{]} }\token{wf} $.
    \item \label{item:demotion-polyclsdecl:typwf}
          If\/ $ \Psi \mid^{  \overrightarrow{ \delta_{{\mathrm{1}}} }^{+}   \refenvsym{,}   \gamma _{ 0 }  }  \Gamma \vdash ^{  \overrightarrow{ \delta_{{\mathrm{2}}} }^{+}  } \refenvnt{A} \ \token{wf} $,
          then
          $ \Psi \mid^{  \overrightarrow{ \delta_{{\mathrm{1}}} }^{+}   \refenvsym{,}   \gamma' _{ 0 }  }   [    \binder{  \delta' _{ 1 }  }  \mathbin{:\succeq}    \gamma' _{ 1 }  ,\dotsc,\binder{  \delta' _{ \refenvnt{k} }  }  \mathbin{:\succeq}   \gamma'  _{ \refenvnt{k} }   ]^{\binder{  \delta' _{ 0 }  } }   \refenvsym{,}  \Gamma  \refenvsym{[}  \sigma  \refenvsym{]} \vdash ^{   \overrightarrow{ \delta_{{\mathrm{2}}} }^{+}    \refenvsym{[}  \sigma  \refenvsym{]} } \refenvnt{A}  \refenvsym{[}  \sigma  \refenvsym{]} \ \token{wf} $.
    \item \label{item:demotion-polyclsdecl:ltrans}
          If\/ $ \Psi \mid^{  \overrightarrow{ \delta_{{\mathrm{1}}} }^{+}   \refenvsym{,}   \gamma _{ 0 }  } \Gamma \vdash \delta_{{\mathrm{2}}} \preceq \delta_{{\mathrm{3}}} $
          and either $\delta_{{\mathrm{3}}} \, \in \,  \token{Dom}_{C}( \Gamma ) $ or there exists $\delta_{{\mathrm{4}}} \, \in \, \refenvsym{\{}   \overrightarrow{ \delta_{{\mathrm{1}}} }^{+}   \refenvsym{,}   \gamma _{ 0 }   \refenvsym{\}}$ such that $ \Psi \mid^{  \overrightarrow{ \delta_{{\mathrm{1}}} }^{+}   \refenvsym{,}   \gamma _{ 0 }  } \Gamma \vdash \delta_{{\mathrm{3}}} \preceq \delta_{{\mathrm{4}}} $,
          then
          $ \Psi \mid^{  \overrightarrow{ \delta_{{\mathrm{1}}} }^{+}   \refenvsym{,}   \gamma' _{ 0 }  }  [    \binder{  \delta' _{ 1 }  }  \mathbin{:\succeq}    \gamma' _{ 1 }  ,\dotsc,\binder{  \delta' _{ \refenvnt{k} }  }  \mathbin{:\succeq}   \gamma'  _{ \refenvnt{k} }   ]^{\binder{  \delta' _{ 0 }  } }   \refenvsym{,}  \Gamma  \refenvsym{[}  \sigma  \refenvsym{]} \vdash \delta_{{\mathrm{2}}}  \refenvsym{[}  \sigma  \refenvsym{]} \preceq \delta_{{\mathrm{3}}}  \refenvsym{[}  \sigma  \refenvsym{]} $.
    \item \label{item:demotion-polyclsdecl:gtrans}
          If\/ $ \Psi \mid^{  \overrightarrow{ \delta_{{\mathrm{1}}} }^{+}   \refenvsym{,}   \gamma _{ 0 }  } \Gamma \vdash \delta_{{\mathrm{2}}} \subseteq \delta_{{\mathrm{3}}} $
          and either $\delta_{{\mathrm{3}}} \, \in \,  \token{Dom}_{C}( \Gamma ) $ or there exists $\delta_{{\mathrm{4}}} \, \in \, \refenvsym{\{}   \overrightarrow{ \delta_{{\mathrm{1}}} }^{+}   \refenvsym{,}   \gamma _{ 0 }   \refenvsym{\}}$ such that $ \Psi \mid^{  \overrightarrow{ \delta_{{\mathrm{1}}} }^{+}   \refenvsym{,}   \gamma _{ 0 }  } \Gamma \vdash \delta_{{\mathrm{3}}} \subseteq \delta_{{\mathrm{4}}} $,
          then
          $ \Psi \mid^{  \overrightarrow{ \delta_{{\mathrm{1}}} }^{+}   \refenvsym{,}   \gamma' _{ 0 }  }  [    \binder{  \delta' _{ 1 }  }  \mathbin{:\succeq}    \gamma' _{ 1 }  ,\dotsc,\binder{  \delta' _{ \refenvnt{k} }  }  \mathbin{:\succeq}   \gamma'  _{ \refenvnt{k} }   ]^{\binder{  \delta' _{ 0 }  } }   \refenvsym{,}  \Gamma  \refenvsym{[}  \sigma  \refenvsym{]} \vdash \delta_{{\mathrm{2}}}  \refenvsym{[}  \sigma  \refenvsym{]} \subseteq \delta_{{\mathrm{3}}}  \refenvsym{[}  \sigma  \refenvsym{]} $.
    \item \label{item:demotion-polyclsdecl:typing}
          If\/ $ \Psi \mid^{  \overrightarrow{ \delta_{{\mathrm{1}}} }^{+}   \refenvsym{,}   \gamma _{ 0 }  }  \Gamma \vdash^{  \overrightarrow{ \delta_{{\mathrm{2}}} }^{+}  }_{  \token{id}  }  \refenvnt{e} : \refenvnt{A} $,
          then
          $ \Psi \mid^{  \overrightarrow{ \delta_{{\mathrm{1}}} }^{+}   \refenvsym{,}   \gamma' _{ 0 }  }   [    \binder{  \delta' _{ 1 }  }  \mathbin{:\succeq}    \gamma' _{ 1 }  ,\dotsc,\binder{  \delta' _{ \refenvnt{k} }  }  \mathbin{:\succeq}   \gamma'  _{ \refenvnt{k} }   ]^{\binder{  \delta' _{ 0 }  } }   \refenvsym{,}  \Gamma  \refenvsym{[}  \sigma  \refenvsym{]} \vdash^{   \overrightarrow{ \delta_{{\mathrm{2}}} }^{+}    \refenvsym{[}  \sigma  \refenvsym{]} }_{  \token{id}  }  \refenvnt{e} : \refenvnt{A}  \refenvsym{[}  \sigma  \refenvsym{]} $.
  \end{enumerate}
\end{lemma}

\begin{proof}
  We proceed by mutual induction on the given derivation.  The proof follows
  the same pattern as \zcref{claim:demotion-var}; the main difference is that
  the demotion substitutes the whole sequence of classifiers in
  $\sigma$ and introduces the polymorphic-classifier declaration
  $ [    \binder{  \delta' _{ 1 }  }  \mathbin{:\succeq}    \gamma' _{ 1 }  ,\dotsc,\binder{  \delta' _{ \refenvnt{k} }  }  \mathbin{:\succeq}   \gamma'  _{ \refenvnt{k} }   ]^{\binder{  \delta' _{ 0 }  } } $ in the local context.
  \begin{description}
    \item[Case \textmd{\zcref{item:demotion-polyclsdecl:ctxwf}}:]
      This case is analogous to \zcref{item:demotion-var:ctxwf} of
      \zcref{claim:demotion-var}.

    \item[Case \textmd{\zcref{item:demotion-polyclsdecl:typwf}}:]
      By induction on the type well-formedness derivation.

    \item[Case \textmd{\zcref{item:demotion-polyclsdecl:ltrans}}:]
      This case is analogous to \zcref{item:demotion-polyclsdecl:gtrans},
      using the rules and inversion principles for $ \preceq $ in place of
      those for $ \subseteq $.

    \item[Case \textmd{\zcref{item:demotion-polyclsdecl:gtrans}}:]
      By induction with respect to $ \token{deg} ( \Psi , \Gamma , \delta_{{\mathrm{3}}} ) $.
      By the side condition of the lemma, either
      $\delta_{{\mathrm{3}}} \, \in \,  \token{Dom}_{C}( \Gamma ) $ or
      there exists $\delta_{{\mathrm{4}}} \, \in \, \refenvsym{\{}   \overrightarrow{ \delta_{{\mathrm{1}}} }^{+}   \refenvsym{,}   \gamma _{ 0 }   \refenvsym{\}}$ such that
      $ \Psi \mid^{  \overrightarrow{ \delta_{{\mathrm{1}}} }^{+}   \refenvsym{,}   \gamma _{ 0 }  } \Gamma \vdash \delta_{{\mathrm{3}}} \subseteq \delta_{{\mathrm{4}}} $.

      We first handle the case $\delta_{{\mathrm{3}}} \, \not\in \,  \token{Dom}_{C}( \Gamma ) $.
      Then there exists $\delta_{{\mathrm{4}}} \, \in \, \refenvsym{\{}   \overrightarrow{ \delta_{{\mathrm{1}}} }^{+}   \refenvsym{,}   \gamma _{ 0 }   \refenvsym{\}}$ such that
      $ \Psi \mid^{  \overrightarrow{ \delta_{{\mathrm{1}}} }^{+}   \refenvsym{,}   \gamma _{ 0 }  } \Gamma \vdash \delta_{{\mathrm{3}}} \subseteq \delta_{{\mathrm{4}}} $.
      From disjointness of $ \token{Dom}_{C}( \Gamma ) $ and $ \token{Dom}_{C}( \Psi ) $, we have $\delta_{{\mathrm{3}}} \, \in \,  \token{Dom}_{C}( \Psi ) $.
      Hence, by \zcref{claim:local-to-global-trans}, we have
      $\Psi  \vdash  \delta_{{\mathrm{2}}}  \subseteq  \delta_{{\mathrm{3}}}$.  Moreover, regularity and
      \zcref{item:demotion-polyclsdecl:ctxwf} give
      \[
         \Psi \mid^{  \overrightarrow{ \delta_{{\mathrm{1}}} }^{+}   \refenvsym{,}   \gamma' _{ 0 }  }  [    \binder{  \delta' _{ 1 }  }  \mathbin{:\succeq}    \gamma' _{ 1 }  ,\dotsc,\binder{  \delta' _{ \refenvnt{k} }  }  \mathbin{:\succeq}   \gamma'  _{ \refenvnt{k} }   ]^{\binder{  \delta' _{ 0 }  } }   \refenvsym{,}  \Gamma  \refenvsym{[}  \sigma  \refenvsym{]} \vdash^{  \dotsc  }\token{wf} .
      \]
      Therefore, by \zcref{claim:global-to-local-trans}, we obtain
      \[
         \Psi \mid^{  \overrightarrow{ \delta_{{\mathrm{1}}} }^{+}   \refenvsym{,}   \gamma' _{ 0 }  }  [    \binder{  \delta' _{ 1 }  }  \mathbin{:\succeq}    \gamma' _{ 1 }  ,\dotsc,\binder{  \delta' _{ \refenvnt{k} }  }  \mathbin{:\succeq}   \gamma'  _{ \refenvnt{k} }   ]^{\binder{  \delta' _{ 0 }  } }   \refenvsym{,}  \Gamma  \refenvsym{[}  \sigma  \refenvsym{]} \vdash \delta_{{\mathrm{2}}} \subseteq \delta_{{\mathrm{3}}} .
      \]
      We conclude by cases on whether $\sigma$ affects $\delta_{{\mathrm{2}}}$ or
      $\delta_{{\mathrm{3}}}$.
      \begin{description}
        \item[Case \textmd{$\delta_{{\mathrm{2}}} \not\in \refenvsym{\{}    \gamma _{ 0 }  ,\dotsc,  \gamma _{ \refenvnt{k} }    \refenvsym{\}}$ and
              $\delta_{{\mathrm{3}}} \not\in \refenvsym{\{}    \gamma _{ 0 }  ,\dotsc,  \gamma _{ \refenvnt{k} }    \refenvsym{\}}$}:]
          The substitution leaves both endpoints unchanged, so the required
          judgment follows immediately.

        \item[Case \textmd{$\delta_{{\mathrm{2}}} \not\in \refenvsym{\{}    \gamma _{ 0 }  ,\dotsc,  \gamma _{ \refenvnt{k} }    \refenvsym{\}}$ and
              $\delta_{{\mathrm{3}}} \in \refenvsym{\{}    \gamma _{ 0 }  ,\dotsc,  \gamma _{ \refenvnt{k} }    \refenvsym{\}}$}:]
          Let $\delta_{{\mathrm{3}}} =  \gamma _{ \refenvnt{i} } $.  If $\delta_{{\mathrm{2}}} =  \gamma _{ \refenvnt{i} } $, this
          contradicts the assumption $\delta_{{\mathrm{2}}} \not\in \refenvsym{\{}    \gamma _{ 0 }  ,\dotsc,  \gamma _{ \refenvnt{k} }    \refenvsym{\}}$.
          Thus $\delta_{{\mathrm{2}}} \neq  \gamma _{ \refenvnt{i} } $.  By
          \zcref{claim:inversion-runtime-gtrans-nht}, the derivation
          $\Psi  \vdash  \delta_{{\mathrm{2}}}  \subseteq   \gamma _{ \refenvnt{i} } $ factors through either $ \gamma' _{ \refenvnt{i} } $ or,
          when $\refenvnt{i} < \refenvnt{k}$, $ \gamma _{ \refenvnt{i}  \refenvsym{+}  1 } $.
          In the former subcase, \zcref{claim:global-to-local-trans} gives the
          demoted-context derivation ending in $ \gamma' _{ \refenvnt{i} } $, and the
          polymorphic-classifier declaration introduced in the context gives
          $  \gamma' _{ \refenvnt{i} }  \subseteq  \delta' _{ \refenvnt{i} }  $.  In the latter subcase, the induction
          hypothesis applies to the smaller derivation ending in
          $ \gamma _{ \refenvnt{i}  \refenvsym{+}  1 } $; the same context declaration gives
          $  \delta' _{ \refenvnt{i}  \refenvsym{+}  1 }  \subseteq  \delta' _{ \refenvnt{i} }  $.  Hence in either subcase we obtain
          \[
             \Psi \mid^{  \overrightarrow{ \delta_{{\mathrm{1}}} }^{+}   \refenvsym{,}   \gamma' _{ 0 }  }  [    \binder{  \delta' _{ 1 }  }  \mathbin{:\succeq}    \gamma' _{ 1 }  ,\dotsc,\binder{  \delta' _{ \refenvnt{k} }  }  \mathbin{:\succeq}   \gamma'  _{ \refenvnt{k} }   ]^{\binder{  \delta' _{ 0 }  } }   \refenvsym{,}  \Gamma  \refenvsym{[}  \sigma  \refenvsym{]} \vdash \delta_{{\mathrm{2}}}  \refenvsym{[}  \sigma  \refenvsym{]} \subseteq  \delta' _{ \refenvnt{i} }  ,
          \]
          which is the required judgment because
          $ \gamma _{ \refenvnt{i} }   \refenvsym{[}  \sigma  \refenvsym{]} =  \delta' _{ \refenvnt{i} } $.

        \item[Case \textmd{$\delta_{{\mathrm{2}}} \in \refenvsym{\{}    \gamma _{ 0 }  ,\dotsc,  \gamma _{ \refenvnt{k} }    \refenvsym{\}}$ and
              $\delta_{{\mathrm{3}}} \in \refenvsym{\{}    \gamma _{ 0 }  ,\dotsc,  \gamma _{ \refenvnt{k} }    \refenvsym{\}}$}:]
          Let $\delta_{{\mathrm{2}}} =  \gamma _{ \refenvnt{i} } $ and $\delta_{{\mathrm{3}}} =  \gamma _{ \refenvnt{j} } $.  Since
          $\Psi  \vdash   \gamma _{ \refenvnt{i} }   \subseteq   \gamma _{ \refenvnt{j} } $, the order of the polymorphic
          classifier declaration gives $\refenvnt{i} \ge \refenvnt{j}$.  If
          $\refenvnt{i} = \refenvnt{j}$, the result follows by reflexivity and lifting
          after substitution.  If $\refenvnt{i} > \refenvnt{j}$, reapplying the
          corresponding polymorphic-classifier context rule along the sequence
          from $ \delta' _{ \refenvnt{i} } $ to $ \delta' _{ \refenvnt{j} } $ gives
          \[
             \Psi \mid^{  \overrightarrow{ \delta_{{\mathrm{1}}} }^{+}   \refenvsym{,}   \gamma' _{ 0 }  }  [    \binder{  \delta' _{ 1 }  }  \mathbin{:\succeq}    \gamma' _{ 1 }  ,\dotsc,\binder{  \delta' _{ \refenvnt{k} }  }  \mathbin{:\succeq}   \gamma'  _{ \refenvnt{k} }   ]^{\binder{  \delta' _{ 0 }  } }   \refenvsym{,}  \Gamma  \refenvsym{[}  \sigma  \refenvsym{]} \vdash  \delta' _{ \refenvnt{i} }  \subseteq  \delta' _{ \refenvnt{j} }  .
          \]
          This is exactly the required judgment.

        \item[Case \textmd{$\delta_{{\mathrm{2}}} \in \refenvsym{\{}    \gamma _{ 0 }  ,\dotsc,  \gamma _{ \refenvnt{k} }    \refenvsym{\}}$ and
              $\delta_{{\mathrm{3}}} \not\in \refenvsym{\{}    \gamma _{ 0 }  ,\dotsc,  \gamma _{ \refenvnt{k} }    \refenvsym{\}}$}:]
          Let $\delta_{{\mathrm{2}}} =  \gamma _{ \refenvnt{i} } $.  Then
          $\Psi  \vdash   \gamma _{ \refenvnt{i} }   \subseteq  \delta_{{\mathrm{3}}}$.
          Moreover, for some $\delta_{{\mathrm{4}}} \, \in \, \refenvsym{\{}   \overrightarrow{ \delta_{{\mathrm{1}}} }^{+}   \refenvsym{,}   \gamma _{ 0 }   \refenvsym{\}}$ we have
          $ \Psi \mid^{  \overrightarrow{ \delta_{{\mathrm{1}}} }^{+}   \refenvsym{,}   \gamma _{ 0 }  } \Gamma \vdash \delta_{{\mathrm{3}}} \subseteq \delta_{{\mathrm{4}}} $.
          By \zcref{claim:local-to-global-trans}, this gives
          $\Psi  \vdash  \delta_{{\mathrm{3}}}  \subseteq  \delta_{{\mathrm{4}}}$; together with
          $\Psi  \vdash   \gamma _{ \refenvnt{i} }   \subseteq  \delta_{{\mathrm{3}}}$ and \ref{rule:runtime-gtrans-trans}, we get
          $\Psi  \vdash   \gamma _{ \refenvnt{i} }   \subseteq  \delta_{{\mathrm{4}}}$.
          If $\delta_{{\mathrm{4}}} \, \in \, \refenvsym{\{}   \overrightarrow{ \delta_{{\mathrm{1}}} }^{+}   \refenvsym{\}}$, this contradicts
          $ \Psi \vdash  \overrightarrow{ \delta_{{\mathrm{1}}} }^{+}  \mathrel{\#}   \gamma _{ 0 }  ,\dotsc,  \gamma _{ \refenvnt{k} }   $.  Hence
          $\delta_{{\mathrm{4}}} =  \gamma _{ 0 } $, and so
          $\Psi  \vdash  \delta_{{\mathrm{3}}}  \subseteq   \gamma _{ 0 } $.
          Now $\Psi  \vdash   \gamma _{ \refenvnt{i} }   \subseteq  \delta_{{\mathrm{3}}}$ and
          $\Psi  \vdash  \delta_{{\mathrm{3}}}  \subseteq   \gamma _{ 0 } $ place $\delta_{{\mathrm{3}}}$ between
          $ \gamma _{ \refenvnt{i} } $ and $ \gamma _{ 0 } $ in the same polymorphic-classifier
          declaration.  By \zcref{claim:deg-preserves-trans-order}, this
          forces $\delta_{{\mathrm{3}}} =  \gamma _{ \refenvnt{j} } $ for some $\refenvnt{j}$, contradicting
          $\delta_{{\mathrm{3}}} \not\in \refenvsym{\{}    \gamma _{ 0 }  ,\dotsc,  \gamma _{ \refenvnt{k} }    \refenvsym{\}}$.  Thus this case is
          impossible.
      \end{description}

      It remains to consider the case $\delta_{{\mathrm{3}}} \, \in \,  \token{Dom}_{C}( \Gamma ) $.  If
      $\delta_{{\mathrm{2}}} = \delta_{{\mathrm{3}}}$, then $\delta_{{\mathrm{3}}}  \refenvsym{[}  \sigma  \refenvsym{]}$ is declared in the
      demoted context by \zcref{item:demotion-polyclsdecl:ctxwf}.  Hence the desired
      judgment follows from \ref{rule:runtime-ltrans-refl} and
      \ref{rule:runtime-gtrans-lift}.  Thus assume $\delta_{{\mathrm{2}}} \neq \delta_{{\mathrm{3}}}$.
      We perform case analysis using
      \zcref{claim:inversion-runtime-gtrans-ctx}.  In each case, the inversion
      gives a derivation
      $ \Psi \mid^{  \overrightarrow{ \delta_{{\mathrm{1}}} }^{+}   \refenvsym{,}   \gamma _{ 0 }  } \Gamma \vdash \delta_{{\mathrm{2}}} \subseteq \delta_{{\mathrm{4}}} $
      where $ \token{deg} ( \Psi , \Gamma , \delta_{{\mathrm{4}}} )  <  \token{deg} ( \Psi , \Gamma , \delta_{{\mathrm{3}}} ) $
      and $\delta_{{\mathrm{4}}} \, \in \, \refenvsym{\{}   \overrightarrow{ \delta_{{\mathrm{1}}} }^{+}   \refenvsym{,}   \gamma _{ 0 }   \refenvsym{\}} \, \cup \,  \token{Dom}_{C}( \Gamma )  \, \cup \,  \token{FC}( \Gamma ) $.
      The membership condition follows from
      \zcref{claim:ctx-output-classifier-origin} when $\delta_{{\mathrm{4}}}$ comes from
      the output stack of the corresponding context prefix.  In the remaining
      polymorphic-classifier declaration cases, $\delta_{{\mathrm{4}}}$ appears as the
      right-hand side of a declaration $ \binder{ \delta_{{\mathrm{3}}} }  \mathbin{:\succeq}   \delta_{{\mathrm{4}}} $, so the condition
      follows from the definitions of $ \token{Dom}_{C}( \Gamma ) $ and $ \token{FC}( \Gamma ) $.
      Hence, the induction hypothesis gives
      \[
         \Psi \mid^{  \overrightarrow{ \delta_{{\mathrm{1}}} }^{+}   \refenvsym{,}   \gamma' _{ 0 }  }  [    \binder{  \delta' _{ 1 }  }  \mathbin{:\succeq}    \gamma' _{ 1 }  ,\dotsc,\binder{  \delta' _{ \refenvnt{k} }  }  \mathbin{:\succeq}   \gamma'  _{ \refenvnt{k} }   ]^{\binder{  \delta' _{ 0 }  } }   \refenvsym{,}  \Gamma  \refenvsym{[}  \sigma  \refenvsym{]} \vdash \delta_{{\mathrm{2}}}  \refenvsym{[}  \sigma  \refenvsym{]} \subseteq \delta_{{\mathrm{4}}}  \refenvsym{[}  \sigma  \refenvsym{]} .
      \]
      Reapplying the corresponding context rule gives
      \[
         \Psi \mid^{  \overrightarrow{ \delta_{{\mathrm{1}}} }^{+}   \refenvsym{,}   \gamma' _{ 0 }  }  [    \binder{  \delta' _{ 1 }  }  \mathbin{:\succeq}    \gamma' _{ 1 }  ,\dotsc,\binder{  \delta' _{ \refenvnt{k} }  }  \mathbin{:\succeq}   \gamma'  _{ \refenvnt{k} }   ]^{\binder{  \delta' _{ 0 }  } }   \refenvsym{,}  \Gamma  \refenvsym{[}  \sigma  \refenvsym{]} \vdash \delta_{{\mathrm{4}}}  \refenvsym{[}  \sigma  \refenvsym{]} \subseteq \delta_{{\mathrm{3}}}  \refenvsym{[}  \sigma  \refenvsym{]} .
      \]
      The desired judgment follows by \ref{rule:runtime-gtrans-trans}.

    \item[Case \textmd{\zcref{item:demotion-polyclsdecl:typing}}:]
      By induction on the typing derivation.  The cases
      \ref{rule:runtime-type-var}, \ref{rule:runtime-type-reserved-var}, and
      \ref{rule:runtime-type-splice} are analogous to the corresponding cases
      in \zcref{claim:demotion-var}, using
      \zcref{item:demotion-polyclsdecl:ctxwf} for context well-formedness and
      \zcref{item:demotion-polyclsdecl:ltrans} for reachability premises.
      The cases for \ref{rule:runtime-type-polycls} and
      \ref{rule:runtime-type-appcls} additionally use
      \zcref{claim:polyclsdecl-substitution} to commute the classifier
      substitution through polymorphic classifier declarations.
  \end{description}
\end{proof}

\begin{corollary}[Demotion]\label{claim:demotion}
  \begin{enumerate}
    \item Suppose
          $ \Psi \mid^{  \overrightarrow{ \gamma_{{\mathrm{1}}} }^{+}   \refenvsym{,}  \gamma_{{\mathrm{2}}}  \refenvsym{,}  \gamma_{{\mathrm{3}}} }  \varepsilon \vdash^{  \overrightarrow{ \gamma_{{\mathrm{1}}} }^{+}   \refenvsym{,}  \gamma_{{\mathrm{2}}}  \refenvsym{,}  \gamma_{{\mathrm{3}}} }_{  \token{id}  }  \refenvnt{e} : \refenvnt{A} $.
          If\/ $\Psi  \vdash  \gamma_{{\mathrm{3}}}  \subseteq  \gamma_{{\mathrm{2}}}$, then
          $ \Psi \mid^{  \overrightarrow{ \gamma_{{\mathrm{1}}} }^{+}   \refenvsym{,}  \gamma_{{\mathrm{2}}} }   \blacktriangleright ^{ \gamma_{{\mathrm{3}}} }  \vdash^{  \overrightarrow{ \gamma_{{\mathrm{1}}} }^{+}   \refenvsym{,}  \gamma_{{\mathrm{2}}}  \refenvsym{,}  \gamma_{{\mathrm{3}}} }_{  \token{id}  }  \refenvnt{e} : \refenvnt{A} $.
    \item Suppose
          $ \Psi \mid^{  \overrightarrow{ \gamma_{{\mathrm{1}}} }   \refenvsym{,}  \gamma_{{\mathrm{2}}} }  \varepsilon \vdash^{  \overrightarrow{ \gamma_{{\mathrm{1}}} }   \refenvsym{,}  \gamma_{{\mathrm{2}}} }_{  \token{id}  }  \refenvnt{e} : \refenvnt{A} $
          and $ \binder{ \gamma_{{\mathrm{2}}} }( \mathbin{:\succeq} \;  \delta _{ 0 }   /  \mathbin{:\supseteq} \;  \delta _{ \refenvnt{k} }  )  \, \in \, \Psi$
          and $ \Psi \vdash  \overrightarrow{ \gamma_{{\mathrm{1}}} }  \mathrel{\#} \gamma_{{\mathrm{2}}} $.
          If\/ $\gamma_{{\mathrm{4}}} \, \not\in \,  \token{Dom}_{C}( \Psi ) $, then
          $ \Psi \mid^{  \overrightarrow{ \gamma_{{\mathrm{1}}} }   \refenvsym{,}    \delta _{ 0 }  ,\dotsc,  \delta _{ \refenvnt{k} }   }   \blacktriangleleft _{ \refenvnt{k} }^{\binder{ \gamma_{{\mathrm{4}}} } }  \vdash^{  \overrightarrow{ \gamma_{{\mathrm{1}}} }   \refenvsym{,}  \gamma_{{\mathrm{4}}} }_{  \token{id}  }  \refenvnt{e} : \refenvnt{A}  \refenvsym{[}  \gamma_{{\mathrm{2}}}  \coloneqq  \gamma_{{\mathrm{4}}}  \refenvsym{]} $.
    \item Suppose
          $ \Psi \mid^{  \overrightarrow{ \gamma_{{\mathrm{1}}} }   \refenvsym{,}  \gamma_{{\mathrm{2}}} }  \varepsilon \vdash^{  \overrightarrow{ \gamma_{{\mathrm{1}}} }   \refenvsym{,}  \gamma_{{\mathrm{2}}} }_{  \token{id}  }  \refenvnt{e} : \refenvnt{A_{{\mathrm{2}}}} $
          and $ \binder{ \refenvmv{x} }: \refenvnt{A_{{\mathrm{1}}}} \mathrel{@}\binder{ \gamma_{{\mathrm{2}}} } \mathbin{:\succeq} \gamma_{{\mathrm{4}}}  \, \in \, \Psi$
          and $ \Psi \vdash  \overrightarrow{ \gamma_{{\mathrm{1}}} }  \mathrel{\#} \gamma_{{\mathrm{2}}} $.
          If\/ $\gamma_{{\mathrm{5}}} \, \not\in \,  \token{Dom}_{C}( \Psi ) $, then
          $ \Psi \mid^{  \overrightarrow{ \gamma_{{\mathrm{1}}} }   \refenvsym{,}  \gamma_{{\mathrm{4}}} }   \binder{ \refenvmv{x} }\mathord{:^{\binder{ \gamma_{{\mathrm{5}}} } } } \refenvnt{A_{{\mathrm{1}}}}  \refenvsym{[}  \gamma_{{\mathrm{2}}}  \coloneqq  \gamma_{{\mathrm{5}}}  \refenvsym{]}  \vdash^{  \overrightarrow{ \gamma_{{\mathrm{1}}} }   \refenvsym{,}  \gamma_{{\mathrm{5}}} }_{  \token{id}  }  \refenvnt{e} : \refenvnt{A_{{\mathrm{2}}}}  \refenvsym{[}  \gamma_{{\mathrm{2}}}  \coloneqq  \gamma_{{\mathrm{5}}}  \refenvsym{]} $.
    \item Let $\sigma =   \gamma _{ 0 }  \coloneqq  \delta' _{ 0 }  ,\dotsc,  \gamma _{ \refenvnt{k} }  \coloneqq  \delta' _{ \refenvnt{k} }  $.
          Suppose
          $ \Psi \mid^{  \overrightarrow{ \delta_{{\mathrm{1}}} }^{+}   \refenvsym{,}   \gamma _{ 0 }  }  \varepsilon \vdash^{  \overrightarrow{ \delta_{{\mathrm{1}}} }^{+}   \refenvsym{,}   \gamma _{ 0 }  }_{  \token{id}  }  \refenvnt{e} : \refenvnt{A} $,
          and $ [    \binder{  \gamma _{ 0 }  }  \mathbin{:\succeq}    \gamma' _{ 0 }  ,\dotsc,\binder{  \gamma _{ \refenvnt{k} }  }  \mathbin{:\succeq}   \gamma'  _{ \refenvnt{k} }   ]  \, \in \, \Psi$
          and $ \Psi \vdash  \overrightarrow{ \delta_{{\mathrm{1}}} }^{+}  \mathrel{\#}   \gamma _{ 0 }  ,\dotsc,  \gamma _{ \refenvnt{k} }   $.
          If\/ $ \delta' _{ \refenvnt{i} }  \, \not\in \,  \token{Dom}_{C}( \Psi ) $ for $0 \le \refenvnt{i} \le \refenvnt{k}$,
          then
          $ \Psi \mid^{  \overrightarrow{ \delta_{{\mathrm{1}}} }^{+}   \refenvsym{,}   \gamma' _{ 0 }  }   [    \binder{  \delta' _{ 1 }  }  \mathbin{:\succeq}    \gamma' _{ 1 }  ,\dotsc,\binder{  \delta' _{ \refenvnt{k} }  }  \mathbin{:\succeq}   \gamma'  _{ \refenvnt{k} }   ]^{\binder{  \delta' _{ 0 }  } }  \vdash^{  \overrightarrow{ \delta_{{\mathrm{1}}} }^{+}   \refenvsym{,}   \delta' _{ 0 }  }_{  \token{id}  }  \refenvnt{e} : \refenvnt{A}  \refenvsym{[}  \sigma  \refenvsym{]} $.
  \end{enumerate}
\end{corollary}

\subsection{Type Soundness}

\begin{lemma}[Inversion for Runtime Expression Typing]\label{claim:inversion-runtime-typing}
  Suppose $ \Psi \mid^{  \overrightarrow{ \gamma_{{\mathrm{1}}} }^{+}  }  \Gamma \vdash^{  \overrightarrow{ \gamma_{{\mathrm{2}}} }^{+}  }_{ R }  \refenvnt{e} : \refenvnt{A} $.
  \begin{enumerate}
    \item\label{item:inversion-runtime-typing:int} If\/ $\refenvnt{e} = \refenvnt{n}$,
          then the derivation ends with \ref{rule:runtime-type-int}.
    \item\label{item:inversion-runtime-typing:var} If\/ $\refenvnt{e} =\refenvmv{x}$,
          then the derivation ends with
          \ref{rule:runtime-type-appcls},
          \ref{rule:runtime-type-var} or
          \ref{rule:runtime-type-reserved-var}.
    \item\label{item:inversion-runtime-typing:func-base}
          If\/ $\refenvnt{e} =  \lambda \binder{ \refenvmv{x} }.\  \refenvnt{e'} $
          and $\refenvnt{A} = \refenvnt{A_{{\mathrm{1}}}}  \rightarrow  \refenvnt{A_{{\mathrm{2}}}}$,
          then the derivation ends with \ref{rule:runtime-type-func}.
    \item\label{item:inversion-runtime-typing:func-polycls}
          If\/ $\refenvnt{e} =  \lambda \binder{ \refenvmv{x} }.\  \refenvnt{e'} $
          and $\refenvnt{A} =  \forall  \varrho . \refenvnt{A'} $,
          then the derivation ends with \ref{rule:runtime-type-polycls}.
    \item\label{item:inversion-runtime-typing:rec-base}
          If\/ $\refenvnt{e} =  \token{rec}\ \binder{ \refenvmv{f} }(\binder{ \refenvmv{x} }).\  \refenvnt{e'} $
          and $\refenvnt{A} = \refenvnt{A_{{\mathrm{1}}}}  \rightarrow  \refenvnt{A_{{\mathrm{2}}}}$,
          then the derivation ends with \ref{rule:runtime-type-rec}.
    \item\label{item:inversion-runtime-typing:rec-polycls}
          If\/ $\refenvnt{e} =  \token{rec}\ \binder{ \refenvmv{f} }(\binder{ \refenvmv{x} }).\  \refenvnt{e'} $
          and $\refenvnt{A} =  \forall  \varrho . \refenvnt{A'} $,
          then the derivation ends with \ref{rule:runtime-type-polycls}.
    \item\label{item:inversion-runtime-typing:quote-base}
          If\/ $\refenvnt{e} = \langle  \refenvnt{e'}  \rangle $
          and $\refenvnt{A} =  \langle \refenvnt{A'} \rangle^{ \gamma_{{\mathrm{3}}} } $,
          then the derivation ends with \ref{rule:runtime-type-quote}.
    \item\label{item:inversion-runtime-typing:quote-polycls}
          If\/ $\refenvnt{e} = \langle  \refenvnt{e'}  \rangle $
          and $\refenvnt{A} =  \forall  \varrho . \refenvnt{A'} $,
          then the derivation ends with \ref{rule:runtime-type-polycls}.
    \item\label{item:inversion-runtime-typing:app}
          If\/ $\refenvnt{e} =  \refenvnt{e_{{\mathrm{1}}}} \refenvnt{e_{{\mathrm{2}}}} $,
          then the derivation ends with \ref{rule:runtime-type-appcls} or \ref{rule:runtime-type-app}.
    \item\label{item:inversion-runtime-typing:splice}
          If\/ $\refenvnt{e} =  { \mathdollar }_{ \refenvnt{k} }\lbrace \refenvnt{e'} \rbrace $,
          then the derivation ends with \ref{rule:runtime-type-appcls} or \ref{rule:runtime-type-splice}.
    \item\label{item:inversion-runtime-typing:ref}
          If\/ $\refenvnt{e} = \token{ref} \, \refenvsym{(}  \refenvnt{e'}  \refenvsym{)}$,
          then the derivation ends with \ref{rule:runtime-type-ref}.
    \item\label{item:inversion-runtime-typing:get}
          If\/ $\refenvnt{e} =  \token{deref}( \refenvnt{e'} ) $,
          then the derivation ends with  \ref{rule:runtime-type-appcls} or \ref{rule:runtime-type-get}.
    \item\label{item:inversion-runtime-typing:set}
          If\/ $\refenvnt{e} =  \refenvnt{e_{{\mathrm{1}}}} \coloneqq \refenvnt{e_{{\mathrm{2}}}} $,
          then the derivation ends with  \ref{rule:runtime-type-appcls} or  \ref{rule:runtime-type-set}.
  \end{enumerate}
\end{lemma}

\begin{proof}
  This follows directly from \zcref{claim:runtime-typing-normal-form}.
\end{proof}

\begin{lemma}[Safety of $ \token{lookup} $]\label{claim:safety-lookup}
  If\/ $ \Psi \mid^{ \gamma }  \varepsilon \vdash^{ \gamma }_{ R }  \refenvmv{x} : \refenvnt{A} $, which is derived by \ref{rule:runtime-type-reserved-var},
  and\/ $ \Psi \mid \Theta \vdash^{ \gamma } E \ \token{wf} $,
  then there exists\/ $\refenvnt{v}$ such that
  $\token{lookup} \, \refenvsym{(}  E  \refenvsym{,}  \token{rename} \, \refenvsym{(}  R  \refenvsym{,}  \refenvmv{x}  \refenvsym{)}  \refenvsym{)} = \token{Done} \, \refenvsym{(}  \refenvnt{v}  \refenvsym{)}$
  and\/ $ \Psi \mid \Theta \vdash^{ \gamma } \refenvnt{v} : \refenvnt{A} \ \token{val} $.
\end{lemma}

\begin{proof}
  By induction on the derivation of $ \Psi \mid \Theta \vdash^{ \gamma } E \ \token{wf} $. For the base case where $E = \refenvsym{(}  E_{{\mathrm{1}}}  \refenvsym{,}  \refenvmv{x}  \coloneqq  \refenvnt{v}  \refenvsym{)}$, we use \zcref{claim:value-portability} to conclude.
\end{proof}

\begin{lemma}[Safety of $ \token{lookupStore} $]\label{claim:safety-lookup-store}
  If\/ $ \Psi \mid \Theta \vdash^{ \gamma } \refenvmv{l} :  \refenvnt{A} \/\ \token{ref}  \ \token{val} $ and\/ $\Psi  \vdash  S  \colon  \Theta$, then there exists\/ $\refenvnt{v}$ such that\/ $\token{lookupStore}  \refenvsym{(}  S  \refenvsym{,}  \refenvmv{l}  \refenvsym{)} = \token{Done} \, \refenvsym{(}  \refenvnt{v}  \refenvsym{)}$ and\/ $ \Psi \mid \Theta \vdash^{ \gamma } \refenvnt{v} : \refenvnt{A} \ \token{val} $.
\end{lemma}

\begin{proof}
  Straightforward by inverting \ref{rule:value-type-loc} and \ref{rule:type-store}. We also use \zcref{claim:value-portability} to conclude.
\end{proof}

\begin{lemma}[Safety of $ \token{updateStore} $]\label{claim:safety-assignment}
  If\/ $ \Psi \mid \Theta \vdash^{ \gamma } \refenvnt{v} : \refenvnt{A} \ \token{val} $, $\Psi  \vdash  S  \colon  \Theta$ and\/ $ \refenvmv{l} : \refenvnt{A}  \, \in \, \Theta$, then\/ $\token{updateStore} \, \refenvsym{(}  S  \refenvsym{,}  \refenvmv{l}  \refenvsym{,}  \refenvnt{v}  \refenvsym{)} = \token{Done} \, \refenvsym{(}  S_{{\mathrm{1}}}  \refenvsym{)}$ for some\/ $S_{{\mathrm{1}}}$ where\/ $\Psi  \vdash  S_{{\mathrm{1}}}  \colon  \Theta$.
\end{lemma}

\begin{proof}
  Straightforward by inverting \ref{rule:type-store}.
\end{proof}

\begin{theorem}[Soundness of Runtime Typing]\label{claim:type-soundness}\leavevmode\samepage
  \begin{enumerate}
    \item\label{item:type-soundness:runtime} If\/ $ \Psi_{{\mathrm{1}}} \mid^{ \gamma_{{\mathrm{1}}} }  \varepsilon \vdash^{ \gamma_{{\mathrm{1}}} }_{ R }   \refenvnt{e} ^{ 0  }  : \refenvnt{A} $,
          $ \Psi_{{\mathrm{1}}} \mid \Theta_{{\mathrm{1}}} \vdash^{ \gamma_{{\mathrm{1}}} } E \ \token{wf} $, and
          $\Psi_{{\mathrm{1}}}  \vdash  S_{{\mathrm{1}}}  \colon  \Theta_{{\mathrm{1}}}$, then either of the following holds.
          \begin{itemize}
            \item $\mathcal{V}^{\mathrm{rt} }  \refenvsym{(}   \refenvnt{e} ^{ 0  }   \refenvsym{,}  E  \refenvsym{,}  R  \refenvsym{,}   \token{Dom}_{V}( \Psi_{{\mathrm{1}}} )   \refenvsym{,}  S_{{\mathrm{1}}}  \refenvsym{,}  \refenvnt{k_{{\mathrm{2}}}}  \refenvsym{)} =  \token{Timeout} $
            \item There exist $\refenvnt{v}$, $\Psi_{{\mathrm{2}}}$, $\Theta_{{\mathrm{2}}}$, and
                  $S_{{\mathrm{2}}}$ such that
                  \begin{itemize}
                    \item $\mathcal{V}^{\mathrm{rt} }  \refenvsym{(}   \refenvnt{e} ^{ 0  }   \refenvsym{,}  E  \refenvsym{,}  R  \refenvsym{,}   \token{Dom}_{V}( \Psi_{{\mathrm{1}}} )   \refenvsym{,}  S_{{\mathrm{1}}}  \refenvsym{,}  \refenvnt{k_{{\mathrm{2}}}}  \refenvsym{)} =
                          \token{Done} \, \refenvsym{(}  \refenvnt{v}  \refenvsym{,}   \token{Dom}_{V}( \Psi_{{\mathrm{2}}} )   \refenvsym{,}  S_{{\mathrm{2}}}  \refenvsym{)}$,
                    \item $ \Psi_{{\mathrm{2}}} \mid \Theta_{{\mathrm{2}}} \vdash^{ \gamma_{{\mathrm{1}}} } \refenvnt{v} : \refenvnt{A} \ \token{val} $,
                    \item $\Psi_{{\mathrm{2}}}  \vdash  S_{{\mathrm{2}}}  \colon  \Theta_{{\mathrm{2}}}$, and
                    \item $ \Psi_{{\mathrm{1}}} \subseteq \Psi_{{\mathrm{2}}} $ and $ \Theta_{{\mathrm{1}}} \subseteq \Theta_{{\mathrm{2}}} $.
                  \end{itemize}
          \end{itemize}

    \item\label{item:type-soundness:future} If\/
          $ \Psi_{{\mathrm{1}}} \mid^{   \gamma _{ 0 }  ,\dotsc,  \gamma _{  \refenvnt{k_{{\mathrm{1}}}} ^{+}  }   }  \varepsilon \vdash^{   \gamma _{ 0 }  ,\dotsc,  \gamma _{  \refenvnt{k_{{\mathrm{1}}}} ^{+}  }   }_{ R }   \refenvnt{e_{{\mathrm{1}}}} ^{  \refenvnt{k_{{\mathrm{1}}}} ^{+}   }  : \refenvnt{A} $,
          $ \Psi_{{\mathrm{1}}} \mid \Theta_{{\mathrm{1}}} \vdash^{  \gamma _{ 0 }  } E \ \token{wf} $, and
          $\Psi_{{\mathrm{1}}}  \vdash  S_{{\mathrm{1}}}  \colon  \Theta_{{\mathrm{1}}}$, then either of the following holds.
          \begin{itemize}
            \item $\mathcal{V}^{\mathrm{fut} }  \refenvsym{(}  \refenvnt{k_{{\mathrm{1}}}}  \refenvsym{,}   \refenvnt{e_{{\mathrm{1}}}} ^{  \refenvnt{k_{{\mathrm{1}}}} ^{+}   }   \refenvsym{,}  E  \refenvsym{,}  R  \refenvsym{,}   \token{Dom}_{V}( \Psi_{{\mathrm{1}}} )   \refenvsym{,}  S_{{\mathrm{1}}}  \refenvsym{,}  \refenvnt{k_{{\mathrm{2}}}}  \refenvsym{)} =  \token{Timeout} $
            \item There exist $ \refenvnt{e_{{\mathrm{2}}}} ^{ \refenvnt{k_{{\mathrm{1}}}}  } $, $\Psi_{{\mathrm{2}}}$, $\Theta_{{\mathrm{2}}}$, and
                  $S_{{\mathrm{2}}}$ such that
                  \begin{itemize}
                    \item $\mathcal{V}^{\mathrm{fut} }  \refenvsym{(}  \refenvnt{k_{{\mathrm{1}}}}  \refenvsym{,}   \refenvnt{e_{{\mathrm{1}}}} ^{  \refenvnt{k_{{\mathrm{1}}}} ^{+}   }   \refenvsym{,}  E  \refenvsym{,}  R  \refenvsym{,}   \token{Dom}_{V}( \Psi_{{\mathrm{1}}} )   \refenvsym{,}  S_{{\mathrm{1}}}  \refenvsym{,}  \refenvnt{k_{{\mathrm{2}}}}  \refenvsym{)} =
                          \token{Done} \, \refenvsym{(}   \refenvnt{e_{{\mathrm{2}}}} ^{ \refenvnt{k_{{\mathrm{1}}}}  }   \refenvsym{,}   \token{Dom}_{V}( \Psi_{{\mathrm{2}}} )   \refenvsym{,}  S_{{\mathrm{2}}}  \refenvsym{)}$,
                    \item $ \Psi_{{\mathrm{2}}} \mid^{   \gamma _{ 1 }  ,\dotsc,  \gamma _{  \refenvnt{k_{{\mathrm{1}}}} ^{+}  }   }  \varepsilon \vdash^{   \gamma _{ 1 }  ,\dotsc,  \gamma _{  \refenvnt{k_{{\mathrm{1}}}} ^{+}  }   }_{  \token{id}  }   \refenvnt{e_{{\mathrm{2}}}} ^{ \refenvnt{k_{{\mathrm{1}}}}  }  : \refenvnt{A} $,
                    \item $\Psi_{{\mathrm{2}}}  \vdash  S_{{\mathrm{2}}}  \colon  \Theta_{{\mathrm{2}}}$, and
                    \item $ \Psi_{{\mathrm{1}}} \subseteq \Psi_{{\mathrm{2}}} $ and $ \Theta_{{\mathrm{1}}} \subseteq \Theta_{{\mathrm{2}}} $.
                  \end{itemize}
          \end{itemize}
  \end{enumerate}
\end{theorem}

\begin{proof}
  By mutual induction with respect to $\refenvnt{k_{{\mathrm{2}}}}$ and the given derivation.

  \begin{description}
    \item[\zcref{item:type-soundness:runtime}:]
          The case where $\refenvnt{k_{{\mathrm{2}}}} = 0$ is trivial. We consider the case where $\refenvnt{k_{{\mathrm{2}}}} > 0$.
          We perform case analysis on $\refenvnt{e}$.

          \begin{description}
            \item[Case \textmd{Last derivation is \ref{rule:runtime-type-appcls}}:]
                  Let $\varrho =  \binder{  \delta _{ 1 }  }  \mathbin{:\succeq}    \delta' _{ 1 }  ,\dotsc,\binder{  \delta _{ \refenvnt{k} }  }  \mathbin{:\succeq}    \delta' _{ \refenvnt{k} }  $ and
                  $\sigma =   \delta _{ 1 }  \coloneqq  \delta'' _{ 1 }  ,\dotsc,  \delta _{ \refenvnt{k} }  \coloneqq  \delta'' _{ \refenvnt{k} }  $.
                  We are given
                  \begin{mathpar}
                    \inferrule*[left={\ref{rule:runtime-type-appcls}}]{
                       \Psi_{{\mathrm{1}}} \mid^{ \gamma_{{\mathrm{1}}} }  \varepsilon \vdash^{ \gamma_{{\mathrm{1}}} }_{ R }   \refenvnt{e} ^{ 0  }  :  \forall  \varrho . \refenvnt{A'}   \\
                       \Psi_{{\mathrm{1}}} \mid^{ \gamma_{{\mathrm{1}}} } \varepsilon \vdash  \delta' _{ \refenvnt{i} }  \preceq  \delta'' _{ \refenvnt{i} }   \text{\ for\ } 1 \le \refenvnt{i} \le \refenvnt{k} \\
                       \Psi_{{\mathrm{1}}} \mid^{ \gamma_{{\mathrm{1}}} } \varepsilon \vdash  \delta'' _{ \refenvnt{i}  \refenvsym{+}  1 }  \subseteq  \delta'' _{ \refenvnt{i} }   \text{\ for\ } 0 \le \refenvnt{i} < \refenvnt{k}
                    }{
                       \Psi_{{\mathrm{1}}} \mid^{ \gamma_{{\mathrm{1}}} }  \varepsilon \vdash^{ \gamma_{{\mathrm{1}}} }_{ R }   \refenvnt{e} ^{ 0  }  : \refenvnt{A'}  \refenvsym{[}  \sigma  \refenvsym{]} 
                    }
                  \end{mathpar}
                  where $ \delta'' _{ 0 }  = \gamma_{{\mathrm{1}}}$ and $\refenvnt{A} = \refenvnt{A'}  \refenvsym{[}  \sigma  \refenvsym{]}$.

                  By the induction hypothesis applied to the premise typing
                  derivation, either of the following holds:
                  \begin{itemize}
                    \item $\mathcal{V}^{\mathrm{rt} }  \refenvsym{(}   \refenvnt{e} ^{ 0  }   \refenvsym{,}  E  \refenvsym{,}  R  \refenvsym{,}   \token{Dom}_{V}( \Psi_{{\mathrm{1}}} )   \refenvsym{,}  S_{{\mathrm{1}}}  \refenvsym{,}  \refenvnt{k_{{\mathrm{2}}}}  \refenvsym{)} =  \token{Timeout} $
                    \item We have $\refenvnt{v_{{\mathrm{1}}}}$, $\Psi_{{\mathrm{2}}}$, $S_{{\mathrm{2}}}$ and $\Theta_{{\mathrm{2}}}$ such that
                          \begin{itemize}
                            \item $\mathcal{V}^{\mathrm{rt} }  \refenvsym{(}   \refenvnt{e} ^{ 0  }   \refenvsym{,}  E  \refenvsym{,}  R  \refenvsym{,}   \token{Dom}_{V}( \Psi_{{\mathrm{1}}} )   \refenvsym{,}  S_{{\mathrm{1}}}  \refenvsym{,}  \refenvnt{k_{{\mathrm{2}}}}  \refenvsym{)} = \token{Done} \, \refenvsym{(}  \refenvnt{v_{{\mathrm{1}}}}  \refenvsym{,}   \token{Dom}_{V}( \Psi_{{\mathrm{2}}} )   \refenvsym{,}  S_{{\mathrm{2}}}  \refenvsym{)}$
                            \item $ \Psi_{{\mathrm{2}}} \mid \Theta_{{\mathrm{2}}} \vdash^{ \gamma_{{\mathrm{1}}} } \refenvnt{v_{{\mathrm{1}}}} :  \forall  \varrho . \refenvnt{A'}  \ \token{val} $
                            \item $\Psi_{{\mathrm{2}}}  \vdash  S_{{\mathrm{2}}}  \colon  \Theta_{{\mathrm{2}}}$
                            \item $ \Psi_{{\mathrm{1}}} \subseteq \Psi_{{\mathrm{2}}} $
                            \item $ \Theta_{{\mathrm{1}}} \subseteq \Theta_{{\mathrm{2}}} $
                          \end{itemize}
                  \end{itemize}
                  The first case is trivial, and we consider the second case.
                  By weakening along $ \Psi_{{\mathrm{1}}} \subseteq \Psi_{{\mathrm{2}}} $, we have
                  \begin{itemize}
                    \item $ \Psi_{{\mathrm{2}}} \mid^{ \gamma_{{\mathrm{1}}} } \varepsilon \vdash  \delta' _{ \refenvnt{i} }  \preceq  \delta'' _{ \refenvnt{i} }  $
                          for each $\refenvnt{i}$ with $1 \le \refenvnt{i} \le \refenvnt{k}$,
                    \item $ \Psi_{{\mathrm{2}}} \mid^{ \gamma_{{\mathrm{1}}} } \varepsilon \vdash  \delta'' _{ \refenvnt{i}  \refenvsym{+}  1 }  \subseteq  \delta'' _{ \refenvnt{i} }  $
                          for each $\refenvnt{i}$ with $0 \le \refenvnt{i} < \refenvnt{k}$.
                  \end{itemize}
                  By \zcref{claim:local-to-global-trans}, these give the
                  global premises required by \zcref{claim:value-appcls}.
                  Hence, by \zcref{claim:value-appcls}, there exists
                  $\Psi_{{\mathrm{3}}}$ such that $ \Psi_{{\mathrm{2}}} \subseteq \Psi_{{\mathrm{3}}} $,
                  $ \token{Dom}_{V}( \Psi_{{\mathrm{3}}} )  =  \token{Dom}_{V}( \Psi_{{\mathrm{2}}} ) $, and
                  \[
                     \Psi_{{\mathrm{3}}} \mid \Theta_{{\mathrm{2}}} \vdash^{ \gamma_{{\mathrm{1}}} } \refenvnt{v_{{\mathrm{1}}}} : \refenvnt{A'}  \refenvsym{[}  \sigma  \refenvsym{]} \ \token{val} .
                  \]
                  Moreover, $\Psi_{{\mathrm{3}}}  \vdash  S_{{\mathrm{2}}}  \colon  \Theta_{{\mathrm{2}}}$ follows by weakening
                  along $ \Psi_{{\mathrm{2}}} \subseteq \Psi_{{\mathrm{3}}} $.  Thus the desired result follows by
                  taking the final value to be $\refenvnt{v_{{\mathrm{1}}}}$, the final
                  reserved-name context to be $\Psi_{{\mathrm{3}}}$, and the final
                  store typing context to be $\Theta_{{\mathrm{2}}}$.

            \item[Case \textmd{$ \refenvnt{e} ^{ 0  }  = \refenvmv{x}$}:]
                  By \zcref{claim:inversion-runtime-typing}, the typing derivation ends with
                  \ref{rule:runtime-type-var}, \ref{rule:runtime-type-reserved-var}, or
                  \ref{rule:runtime-type-appcls}.

                  The case of \ref{rule:runtime-type-var} is impossible because
                  $\Gamma =  \varepsilon $. The case of \ref{rule:runtime-type-appcls}
                  has already been discussed. The remaining case,
                  \ref{rule:runtime-type-reserved-var}, follows from
                  \zcref{claim:safety-lookup}.

            \item[Case \textmd{$ \refenvnt{e} ^{ 0  }  =   \lambda \binder{ \refenvmv{x} }.\  \refenvnt{e}  ^{ 0  } $}:]
                  By \ref{rule:value-type-clos-func}.

            \item[Case \textmd{$ \refenvnt{e} ^{ 0  }  =   \token{rec}\ \binder{ \refenvmv{f} }(\binder{ \refenvmv{x} }).\  \refenvnt{e}  ^{ 0  } $}:]
                  By \ref{rule:value-type-clos-rec}.

            \item[Case \textmd{$ \refenvnt{e} ^{ 0  }  =    \refenvnt{e_{{\mathrm{1}}}} ^{ 0  }  \refenvnt{e_{{\mathrm{2}}}}  ^{ 0  } $}:]
                  By \zcref{claim:inversion-runtime-typing}, it is derived by \ref{rule:runtime-type-appcls} or \ref{rule:runtime-type-app}.
                  As the former case is already discussed, we consider the latter.
                  In this case, we are given
                  \begin{mathpar}
                    \inferrule*[left={\ref{rule:runtime-type-app}}]{
                       \Psi_{{\mathrm{1}}} \mid^{ \gamma_{{\mathrm{1}}} }  \varepsilon \vdash^{ \gamma_{{\mathrm{1}}} }_{ R }   \refenvnt{e_{{\mathrm{1}}}} ^{ 0  }  : \refenvnt{B}  \rightarrow  \refenvnt{A}  \\
                       \Psi_{{\mathrm{1}}} \mid^{ \gamma_{{\mathrm{1}}} }  \varepsilon \vdash^{ \gamma_{{\mathrm{1}}} }_{ R }   \refenvnt{e_{{\mathrm{2}}}} ^{ 0  }  : \refenvnt{B} 
                    }{
                       \Psi_{{\mathrm{1}}} \mid^{ \gamma_{{\mathrm{1}}} }  \varepsilon \vdash^{ \gamma_{{\mathrm{1}}} }_{ R }     \refenvnt{e_{{\mathrm{1}}}} ^{ 0  }  \refenvnt{e_{{\mathrm{2}}}}  ^{ 0  }  : \refenvnt{A} 
                    }
                  \end{mathpar}
                  for some $\refenvnt{B}$.
                  By IH on $ \refenvnt{e_{{\mathrm{1}}}} ^{ 0  } $, either of the following holds:
                  \begin{itemize}
                    \item $\mathcal{V}^{\mathrm{rt} }  \refenvsym{(}   \refenvnt{e_{{\mathrm{1}}}} ^{ 0  }   \refenvsym{,}  E  \refenvsym{,}  R  \refenvsym{,}   \token{Dom}_{V}( \Psi_{{\mathrm{1}}} )   \refenvsym{,}  S_{{\mathrm{1}}}  \refenvsym{,}  \refenvnt{k_{{\mathrm{2}}}}  \refenvsym{-}  1  \refenvsym{)} =  \token{Timeout} $
                    \item We have $\refenvnt{v_{{\mathrm{1}}}}$, $\Psi_{{\mathrm{2}}}$, $S_{{\mathrm{2}}}$ and $\Theta_{{\mathrm{2}}}$ such that
                          \begin{itemize}
                            \item $\mathcal{V}^{\mathrm{rt} }  \refenvsym{(}   \refenvnt{e_{{\mathrm{1}}}} ^{ 0  }   \refenvsym{,}  E  \refenvsym{,}  R  \refenvsym{,}   \token{Dom}_{V}( \Psi_{{\mathrm{1}}} )   \refenvsym{,}  S_{{\mathrm{1}}}  \refenvsym{,}  \refenvnt{k_{{\mathrm{2}}}}  \refenvsym{-}  1  \refenvsym{)} = \token{Done} \, \refenvsym{(}  \refenvnt{v_{{\mathrm{1}}}}  \refenvsym{,}   \token{Dom}_{V}( \Psi_{{\mathrm{2}}} )   \refenvsym{,}  S_{{\mathrm{2}}}  \refenvsym{)}$
                            \item $ \Psi_{{\mathrm{2}}} \mid \Theta_{{\mathrm{2}}} \vdash^{ \gamma_{{\mathrm{1}}} } \refenvnt{v_{{\mathrm{1}}}} : \refenvnt{B}  \rightarrow  \refenvnt{A} \ \token{val} $
                            \item $\Psi_{{\mathrm{2}}}  \vdash  S_{{\mathrm{2}}}  \colon  \Theta_{{\mathrm{2}}}$
                            \item $ \Psi_{{\mathrm{1}}} \subseteq \Psi_{{\mathrm{2}}} $
                            \item $ \Theta_{{\mathrm{1}}} \subseteq \Theta_{{\mathrm{2}}} $
                          \end{itemize}
                  \end{itemize}
                  The first case is trivial, and we consider the second case.
                  We have $ \Psi_{{\mathrm{2}}} \mid^{ \gamma_{{\mathrm{1}}} }  \varepsilon \vdash^{ \gamma_{{\mathrm{1}}} }_{ R }   \refenvnt{e_{{\mathrm{2}}}} ^{ 0  }  : \refenvnt{B} $
                  by \zcref{claim:nht-weakening}.  Moreover,
                  $ \Psi_{{\mathrm{2}}} \mid \Theta_{{\mathrm{2}}} \vdash^{ \gamma_{{\mathrm{1}}} } E \ \token{wf} $ follows by
                  weakening along $ \Psi_{{\mathrm{1}}} \subseteq \Psi_{{\mathrm{2}}} $ and $ \Theta_{{\mathrm{1}}} \subseteq \Theta_{{\mathrm{2}}} $.
                  Thus, we can apply the IH and get either of the following.

                  \begin{itemize}
                    \item $\mathcal{V}^{\mathrm{rt} }  \refenvsym{(}   \refenvnt{e_{{\mathrm{2}}}} ^{ 0  }   \refenvsym{,}  E  \refenvsym{,}  R  \refenvsym{,}   \token{Dom}_{V}( \Psi_{{\mathrm{2}}} )   \refenvsym{,}  S_{{\mathrm{2}}}  \refenvsym{,}  \refenvnt{k_{{\mathrm{2}}}}  \refenvsym{-}  1  \refenvsym{)} =  \token{Timeout} $
                    \item We have $\refenvnt{v_{{\mathrm{2}}}}$, $\Psi_{{\mathrm{3}}}$, $S_{{\mathrm{3}}}$ and $\Theta_{{\mathrm{3}}}$ such that
                          \begin{itemize}
                            \item $\mathcal{V}^{\mathrm{rt} }  \refenvsym{(}   \refenvnt{e_{{\mathrm{2}}}} ^{ 0  }   \refenvsym{,}  E  \refenvsym{,}  R  \refenvsym{,}   \token{Dom}_{V}( \Psi_{{\mathrm{2}}} )   \refenvsym{,}  S_{{\mathrm{2}}}  \refenvsym{,}  \refenvnt{k_{{\mathrm{2}}}}  \refenvsym{-}  1  \refenvsym{)} = \token{Done} \, \refenvsym{(}  \refenvnt{v_{{\mathrm{2}}}}  \refenvsym{,}   \token{Dom}_{V}( \Psi_{{\mathrm{3}}} )   \refenvsym{,}  S_{{\mathrm{3}}}  \refenvsym{)}$
                            \item $ \Psi_{{\mathrm{3}}} \mid \Theta_{{\mathrm{3}}} \vdash^{ \gamma_{{\mathrm{1}}} } \refenvnt{v_{{\mathrm{2}}}} : \refenvnt{B} \ \token{val} $
                            \item $\Psi_{{\mathrm{3}}}  \vdash  S_{{\mathrm{3}}}  \colon  \Theta_{{\mathrm{3}}}$
                            \item $ \Psi_{{\mathrm{2}}} \subseteq \Psi_{{\mathrm{3}}} $
                            \item $ \Theta_{{\mathrm{2}}} \subseteq \Theta_{{\mathrm{3}}} $
                          \end{itemize}
                  \end{itemize}
                  The first case is trivial, and we consider the second case.
                  $\refenvnt{v_{{\mathrm{1}}}}$ is typed by either of \ref{rule:value-type-clos-func} or \ref{rule:value-type-clos-rec}. We consider the case where $\refenvnt{v_{{\mathrm{1}}}}$ is typed by \ref{rule:value-type-clos-rec}, and the other case is similar.
                  By inverting the typing of $\refenvnt{v_{{\mathrm{1}}}}$, we have
                  $\refenvnt{v_{{\mathrm{1}}}} = \token{clos} \, \refenvsym{(}  E_{{\mathrm{1}}}  \refenvsym{,}  R_{{\mathrm{1}}}  \refenvsym{,}    \token{rec}\ \binder{ \refenvmv{f} }(\binder{ \refenvmv{x} }).\  \refenvnt{e_{{\mathrm{3}}}}  ^{ 0  }   \refenvsym{)}$
                  for some $E_{{\mathrm{1}}}$, $R_{{\mathrm{1}}}$, $\refenvmv{f}$, $\refenvmv{x}$ and $ \refenvnt{e_{{\mathrm{3}}}} ^{ 0  } $ such that
                  \begin{itemize}
                    \item $ \Psi_{{\mathrm{3}}} \mid^{ \gamma_{{\mathrm{2}}} }  \varepsilon \vdash^{ \gamma_{{\mathrm{2}}} }_{ R_{{\mathrm{1}}} }    \token{rec}\ \binder{ \refenvmv{f} }(\binder{ \refenvmv{x} }).\  \refenvnt{e_{{\mathrm{3}}}}  ^{ 0  }  : \refenvnt{B}  \rightarrow  \refenvnt{A} $
                    \item $ \Psi_{{\mathrm{3}}} \mid \Theta_{{\mathrm{3}}} \vdash^{ \gamma_{{\mathrm{2}}} } E_{{\mathrm{1}}} \ \token{wf} $
                    \item $ \Psi_{{\mathrm{3}}}  \vdash^{ \gamma_{{\mathrm{1}}} }  \refenvnt{B}  \rightarrow  \refenvnt{A} \ \token{wf} $
                  \end{itemize}
                  for some $\gamma_{{\mathrm{2}}}$.
                  By inverting the typing of $  \token{rec}\ \binder{ \refenvmv{f} }(\binder{ \refenvmv{x} }).\  \refenvnt{e_{{\mathrm{3}}}}  ^{ 0  } $,
                  we have $ \Psi_{{\mathrm{3}}} \mid^{ \gamma_{{\mathrm{2}}} }   \binder{ \refenvmv{f} }\mathord{:^{\binder{ \gamma_{{\mathrm{3}}} } } } \refenvnt{B}  \rightarrow  \refenvnt{A}   \refenvsym{,}   \binder{ \refenvmv{x} }\mathord{:^{\binder{ \gamma_{{\mathrm{4}}} } } } \refenvnt{B}  \vdash^{ \gamma_{{\mathrm{4}}} }_{ R_{{\mathrm{1}}} }   \refenvnt{e_{{\mathrm{3}}}} ^{ 0  }  : \refenvnt{A} $
                  for some $\gamma_{{\mathrm{3}}}$ and $\gamma_{{\mathrm{4}}}$.
                  We take $g = \token{gensym} \, \refenvsym{(}   \token{Dom}_{V}( \Psi_{{\mathrm{3}}} )   \refenvsym{)}$ and
                  $\refenvmv{y} = \token{gensym} \, \refenvsym{(}   \token{Dom}_{V}( \Psi_{{\mathrm{3}}} )   \refenvsym{,}  g  \refenvsym{)}$.
                  Let $R_{{\mathrm{2}}} = R_{{\mathrm{1}}}  \refenvsym{,}  \refenvmv{f}  \coloneqq  g  \refenvsym{,}  \refenvmv{x}  \coloneqq  \refenvmv{y}$.
                  As $g \, \not\in \,  \token{Dom}_{V}( \Psi_{{\mathrm{3}}} ) $ and $\refenvmv{y} \, \not\in \,  \token{Dom}_{V}( \Psi_{{\mathrm{3}}} ) $,
                  we apply \zcref{claim:promotion} to get
                  $ \Psi_{{\mathrm{3}}}  \refenvsym{,}   \binder{ g }: \refenvnt{B}  \rightarrow  \refenvnt{A} \mathrel{@}\binder{ \gamma_{{\mathrm{3}}} } \mathbin{:\succeq} \gamma_{{\mathrm{2}}}   \refenvsym{,}   \binder{ \refenvmv{y} }: \refenvnt{B} \mathrel{@}\binder{ \gamma_{{\mathrm{4}}} } \mathbin{:\succeq} \gamma_{{\mathrm{3}}}  \mid^{ \gamma_{{\mathrm{4}}} }  \varepsilon \vdash^{ \gamma_{{\mathrm{4}}} }_{ R_{{\mathrm{2}}} }   \refenvnt{e_{{\mathrm{3}}}} ^{ 0  }  : \refenvnt{A} $.
                  Let $\Psi_{{\mathrm{4}}} =
                  \Psi_{{\mathrm{3}}}  \refenvsym{,}   \binder{ g }: \refenvnt{B}  \rightarrow  \refenvnt{A} \mathrel{@}\binder{ \gamma_{{\mathrm{3}}} } \mathbin{:\succeq} \gamma_{{\mathrm{2}}}   \refenvsym{,}   \binder{ \refenvmv{y} }: \refenvnt{B} \mathrel{@}\binder{ \gamma_{{\mathrm{4}}} } \mathbin{:\succeq} \gamma_{{\mathrm{3}}} $.
                  From $ \Psi_{{\mathrm{3}}} \mid \Theta_{{\mathrm{3}}} \vdash^{ \gamma_{{\mathrm{2}}} } E_{{\mathrm{1}}} \ \token{wf} $ and
                  $ \Psi_{{\mathrm{2}}} \mid \Theta_{{\mathrm{2}}} \vdash^{ \gamma_{{\mathrm{1}}} } \refenvnt{v_{{\mathrm{1}}}} : \refenvnt{B}  \rightarrow  \refenvnt{A} \ \token{val} $,
                  we have $ \Psi_{{\mathrm{4}}} \mid \Theta_{{\mathrm{3}}} \vdash^{ \gamma_{{\mathrm{3}}} } E_{{\mathrm{1}}}  \refenvsym{,}  g  \coloneqq  \refenvnt{v_{{\mathrm{1}}}} \ \token{wf} $
                  by \ref{rule:runtime-wf-venv-var},
                  weakening along $ \Psi_{{\mathrm{2}}} \subseteq \Psi_{{\mathrm{3}}} $, $ \Psi_{{\mathrm{3}}} \subseteq \Psi_{{\mathrm{4}}} $, and
                  $ \Theta_{{\mathrm{2}}} \subseteq \Theta_{{\mathrm{3}}} $,
                  and \zcref{claim:value-portability}.
                  Then, as we have $ \Psi_{{\mathrm{3}}} \mid \Theta_{{\mathrm{3}}} \vdash^{ \gamma_{{\mathrm{1}}} } \refenvnt{v_{{\mathrm{2}}}} : \refenvnt{B} \ \token{val} $,
                  we have $ \Psi_{{\mathrm{4}}} \mid \Theta_{{\mathrm{3}}} \vdash^{ \gamma_{{\mathrm{4}}} } E_{{\mathrm{1}}}  \refenvsym{,}  g  \coloneqq  \refenvnt{v_{{\mathrm{1}}}}  \refenvsym{,}  \refenvmv{y}  \coloneqq  \refenvnt{v_{{\mathrm{2}}}} \ \token{wf} $
                  by \ref{rule:runtime-wf-venv-var},
                  weakening along $ \Psi_{{\mathrm{3}}} \subseteq \Psi_{{\mathrm{4}}} $, and
                  \zcref{claim:value-portability}.
                  We also have $\Psi_{{\mathrm{4}}}  \vdash  S_{{\mathrm{3}}}  \colon  \Theta_{{\mathrm{3}}}$ by
                  weakening along $ \Psi_{{\mathrm{3}}} \subseteq \Psi_{{\mathrm{4}}} $.
                  Let $E_{{\mathrm{2}}} = E_{{\mathrm{1}}}  \refenvsym{,}  g  \coloneqq  \refenvnt{v_{{\mathrm{1}}}}  \refenvsym{,}  \refenvmv{y}  \coloneqq  \refenvnt{v_{{\mathrm{2}}}}$.
                  Hence, we can apply IH on $ \refenvnt{e_{{\mathrm{3}}}} ^{ 0  } $ to get either of the following.
                  \begin{itemize}
                    \item $\mathcal{V}^{\mathrm{rt} }  \refenvsym{(}   \refenvnt{e_{{\mathrm{3}}}} ^{ 0  }   \refenvsym{,}  E_{{\mathrm{2}}}  \refenvsym{,}  R_{{\mathrm{2}}}  \refenvsym{,}   \token{Dom}_{V}( \Psi_{{\mathrm{4}}} )   \refenvsym{,}  S_{{\mathrm{3}}}  \refenvsym{,}  \refenvnt{k_{{\mathrm{2}}}}  \refenvsym{-}  1  \refenvsym{)} =  \token{Timeout} $
                    \item We have $\refenvnt{v_{{\mathrm{3}}}}$, $\Psi_{{\mathrm{5}}}$, $S_{{\mathrm{4}}}$ and $\Theta_{{\mathrm{4}}}$ such that
                          \begin{itemize}
                            \item $\mathcal{V}^{\mathrm{rt} }  \refenvsym{(}   \refenvnt{e_{{\mathrm{3}}}} ^{ 0  }   \refenvsym{,}  E_{{\mathrm{2}}}  \refenvsym{,}  R_{{\mathrm{2}}}  \refenvsym{,}   \token{Dom}_{V}( \Psi_{{\mathrm{4}}} )   \refenvsym{,}  S_{{\mathrm{3}}}  \refenvsym{,}  \refenvnt{k_{{\mathrm{2}}}}  \refenvsym{-}  1  \refenvsym{)} = \token{Done} \, \refenvsym{(}  \refenvnt{v_{{\mathrm{3}}}}  \refenvsym{,}   \token{Dom}_{V}( \Psi_{{\mathrm{5}}} )   \refenvsym{,}  S_{{\mathrm{4}}}  \refenvsym{)}$
                            \item $ \Psi_{{\mathrm{5}}} \mid \Theta_{{\mathrm{4}}} \vdash^{ \gamma_{{\mathrm{4}}} } \refenvnt{v_{{\mathrm{3}}}} : \refenvnt{A} \ \token{val} $
                            \item $\Psi_{{\mathrm{5}}}  \vdash  S_{{\mathrm{4}}}  \colon  \Theta_{{\mathrm{4}}}$
                            \item $ \Psi_{{\mathrm{4}}} \subseteq \Psi_{{\mathrm{5}}} $
                            \item $ \Theta_{{\mathrm{3}}} \subseteq \Theta_{{\mathrm{4}}} $
                          \end{itemize}
                  \end{itemize}
                  Here, $\mathcal{V}^{\mathrm{rt} }  \refenvsym{(}   \refenvnt{e} ^{ 0  }   \refenvsym{,}  E  \refenvsym{,}  R  \refenvsym{,}   \token{Dom}_{V}( \Psi_{{\mathrm{1}}} )   \refenvsym{,}  S_{{\mathrm{1}}}  \refenvsym{,}  \refenvnt{k_{{\mathrm{2}}}}  \refenvsym{)} = \token{Done} \, \refenvsym{(}  \refenvnt{v_{{\mathrm{3}}}}  \refenvsym{,}   \token{Dom}_{V}( \Psi_{{\mathrm{5}}} )   \refenvsym{,}  S_{{\mathrm{4}}}  \refenvsym{)}$
                  from the definition of $ \mathcal{V}^{\mathrm{rt} } $.
                  Hence, it suffices to show that $ \Psi_{{\mathrm{5}}} \mid \Theta_{{\mathrm{4}}} \vdash^{ \gamma_{{\mathrm{1}}} } \refenvnt{v_{{\mathrm{3}}}} : \refenvnt{A} \ \token{val} $,
                  which can be shown by \zcref{claim:value-portability}.

            \item[Case \textmd{$ \refenvnt{e} ^{ 0  }  =  \langle   \refenvnt{e_{{\mathrm{1}}}} ^{ 1  }   \rangle $}:]
                  By \zcref{claim:inversion-runtime-typing}, it is derived by \ref{rule:runtime-type-quote} or \ref{rule:runtime-type-polycls}.
                  After repeating the inversion, we have
                  \[
                     \Psi_{{\mathrm{1}}} \mid^{  \delta _{ 0 }  }    [   \varrho _{ 1 }   ]^{\binder{  \delta _{ 1 }  } }  ,\dotsc,  [   \varrho _{ \refenvnt{k} }   ]^{\binder{  \delta _{ \refenvnt{k} }  } }    \refenvsym{,}   \blacktriangleright ^{ \gamma_{{\mathrm{2}}} }  \vdash^{  \delta _{ \refenvnt{k} }   \refenvsym{,}  \gamma_{{\mathrm{2}}} }_{ R }   \refenvnt{e_{{\mathrm{1}}}} ^{ 1  }  : \refenvnt{A_{{\mathrm{1}}}} .
                  \]
                  for some $\refenvnt{k}$, $  \delta _{ 1 }  ,\dotsc,  \delta _{ \refenvnt{k} }  $, $ \varrho _{ 1 } ,\dotsc, \varrho _{ \refenvnt{k} } $, $\refenvnt{A_{{\mathrm{1}}}}$ and $\gamma_{{\mathrm{2}}}$
                  such that $\refenvnt{k} \ge 0$, $ \delta _{ 0 }  = \gamma_{{\mathrm{1}}}$,
                  and $\refenvnt{A} =  \forall   \varrho _{ 1 }  \dotsc\forall  \varrho _{ \refenvnt{k} }  .  \langle \refenvnt{A_{{\mathrm{1}}}} \rangle^{ \gamma_{{\mathrm{2}}} }  $.

                  By repeating \zcref{claim:promotion}, we have
                  \[
                     \Psi_{{\mathrm{1}}}  \refenvsym{,}   [     \binder{  \delta _{ 1 }  }  \mathbin{:\succeq}   \delta  _{ 0 }   \refenvsym{,}  \varrho _{ 1 }   ],\dotsc,[     \binder{  \delta _{ \refenvnt{k} }  }  \mathbin{:\succeq}   \delta  _{ \refenvnt{k}  \refenvsym{-}  1 }   \refenvsym{,}  \varrho _{ \refenvnt{k} }   ]  \mid^{  \delta _{ \refenvnt{k} }   \refenvsym{,}  \gamma_{{\mathrm{2}}} }  \varepsilon \vdash^{  \delta _{ \refenvnt{k} }   \refenvsym{,}  \gamma_{{\mathrm{2}}} }_{ R }   \refenvnt{e_{{\mathrm{1}}}} ^{ 1  }  : \refenvnt{A_{{\mathrm{1}}}} .
                  \]
                  Let $\Psi_{{\mathrm{2}}} = \Psi_{{\mathrm{1}}}  \refenvsym{,}   [     \binder{  \delta _{ 1 }  }  \mathbin{:\succeq}   \delta  _{ 0 }   \refenvsym{,}  \varrho _{ 1 }   ],\dotsc,[     \binder{  \delta _{ \refenvnt{k} }  }  \mathbin{:\succeq}   \delta  _{ \refenvnt{k}  \refenvsym{-}  1 }   \refenvsym{,}  \varrho _{ \refenvnt{k} }   ] $.
                  We have $ \token{Dom}_{V}( \Psi_{{\mathrm{2}}} )  =  \token{Dom}_{V}( \Psi_{{\mathrm{1}}} ) $ and
                  $ \Psi_{{\mathrm{2}}} \mid \Theta_{{\mathrm{1}}} \vdash^{  \delta _{ \refenvnt{k} }  } E \ \token{wf} $ by weakening and
                  repeated application of \ref{rule:runtime-wf-venv-polycls}.
                  Also, $\Psi_{{\mathrm{2}}}  \vdash  S_{{\mathrm{1}}}  \colon  \Theta_{{\mathrm{1}}}$ follows by weakening.
                  Hence, we apply the induction hypothesis on $ \refenvnt{e_{{\mathrm{1}}}} ^{ 1  } $ and get either of the following.
                  \begin{itemize}
                    \item $\mathcal{V}^{\mathrm{fut} }  \refenvsym{(}  0  \refenvsym{,}   \refenvnt{e_{{\mathrm{1}}}} ^{ 1  }   \refenvsym{,}  E  \refenvsym{,}  R  \refenvsym{,}   \token{Dom}_{V}( \Psi_{{\mathrm{2}}} )   \refenvsym{,}  S_{{\mathrm{1}}}  \refenvsym{,}  \refenvnt{k_{{\mathrm{2}}}}  \refenvsym{-}  1  \refenvsym{)} =  \token{Timeout} $
                    \item We have $ \refenvnt{e_{{\mathrm{2}}}} ^{ 0  } $, $\Psi_{{\mathrm{3}}}$, $S_{{\mathrm{2}}}$ and $\Theta_{{\mathrm{2}}}$ such that
                          \begin{itemize}
                            \item $\mathcal{V}^{\mathrm{fut} }  \refenvsym{(}  0  \refenvsym{,}   \refenvnt{e_{{\mathrm{1}}}} ^{ 1  }   \refenvsym{,}  E  \refenvsym{,}  R  \refenvsym{,}   \token{Dom}_{V}( \Psi_{{\mathrm{2}}} )   \refenvsym{,}  S_{{\mathrm{1}}}  \refenvsym{,}  \refenvnt{k_{{\mathrm{2}}}}  \refenvsym{-}  1  \refenvsym{)} = \token{Done} \, \refenvsym{(}   \refenvnt{e_{{\mathrm{2}}}} ^{ 0  }   \refenvsym{,}   \token{Dom}_{V}( \Psi_{{\mathrm{3}}} )   \refenvsym{,}  S_{{\mathrm{2}}}  \refenvsym{)}$
                            \item $ \Psi_{{\mathrm{3}}} \mid^{ \gamma_{{\mathrm{2}}} }  \varepsilon \vdash^{ \gamma_{{\mathrm{2}}} }_{  \token{id}  }   \refenvnt{e_{{\mathrm{2}}}} ^{ 0  }  : \refenvnt{A_{{\mathrm{1}}}} $
                            \item $\Psi_{{\mathrm{3}}}  \vdash  S_{{\mathrm{2}}}  \colon  \Theta_{{\mathrm{2}}}$
                            \item $ \Psi_{{\mathrm{2}}} \subseteq \Psi_{{\mathrm{3}}} $
                            \item $ \Theta_{{\mathrm{1}}} \subseteq \Theta_{{\mathrm{2}}} $
                          \end{itemize}
                  \end{itemize}
                  The first case is trivial, and we consider the second case.

                  Since $ \token{Dom}_{V}( \Psi_{{\mathrm{2}}} )  =  \token{Dom}_{V}( \Psi_{{\mathrm{1}}} ) $,
                  the definition of $ \mathcal{V}^{\mathrm{rt} } $ gives
                  \[
                    \mathcal{V}^{\mathrm{rt} }  \refenvsym{(}   \langle   \refenvnt{e_{{\mathrm{1}}}} ^{ 1  }   \rangle   \refenvsym{,}  E  \refenvsym{,}  R  \refenvsym{,}   \token{Dom}_{V}( \Psi_{{\mathrm{1}}} )   \refenvsym{,}  S_{{\mathrm{1}}}  \refenvsym{,}  \refenvnt{k_{{\mathrm{2}}}}  \refenvsym{)}
                    = \token{Done} \, \refenvsym{(}   \langle   \refenvnt{e_{{\mathrm{2}}}} ^{ 0  }   \rangle   \refenvsym{,}   \token{Dom}_{V}( \Psi_{{\mathrm{3}}} )   \refenvsym{,}  S_{{\mathrm{2}}}  \refenvsym{)}.
                  \]
                  It remains to show
                  $ \Psi_{{\mathrm{3}}} \mid \Theta_{{\mathrm{2}}} \vdash^{ \gamma_{{\mathrm{1}}} }  \langle   \refenvnt{e_{{\mathrm{2}}}} ^{ 0  }   \rangle  : \refenvnt{A} \ \token{val} $.
                  By repeated demotion, using $ \Psi_{{\mathrm{2}}} \subseteq \Psi_{{\mathrm{3}}} $, we have
                  \[
                     \Psi_{{\mathrm{3}}} \mid^{  \delta _{ 0 }  }    [   \varrho _{ 1 }   ]^{\binder{  \delta _{ 1 }  } }  ,\dotsc,  [   \varrho _{ \refenvnt{k} }   ]^{\binder{  \delta _{ \refenvnt{k} }  } }    \refenvsym{,}   \blacktriangleright ^{ \gamma_{{\mathrm{2}}} }  \vdash^{  \delta _{ \refenvnt{k} }   \refenvsym{,}  \gamma_{{\mathrm{2}}} }_{  \token{id}  }   \refenvnt{e_{{\mathrm{2}}}} ^{ 0  }  : \refenvnt{A_{{\mathrm{1}}}} .
                  \]
                  Then applying \ref{rule:runtime-type-quote} and
                  \ref{rule:runtime-type-polycls} repeatedly, we have
                  \[
                     \Psi_{{\mathrm{3}}} \mid^{  \delta _{ 0 }  }  \varepsilon \vdash^{ \gamma_{{\mathrm{1}}} }_{  \token{id}  }   \langle   \refenvnt{e_{{\mathrm{2}}}} ^{ 0  }   \rangle  : \refenvnt{A} .
                  \]
                  Hence, we can apply \ref{rule:value-type-code} to get the desired value typing judgment.

            \item[Case \textmd{$ \refenvnt{e} ^{ 0  }  =  { \mathdollar }_{ 0 }\lbrace  \refenvnt{e_{{\mathrm{1}}}} ^{ 0  }  \rbrace $}:]
                  By \zcref{claim:inversion-runtime-typing}, it is derived by
                  \ref{rule:runtime-type-appcls} or \ref{rule:runtime-type-splice}.
                  The former case is already discussed, and we consider the latter case.
                  We are given
                  \begin{mathpar}
                    \inferrule*[left={\ref{rule:runtime-type-splice}}]{
                       \Psi_{{\mathrm{1}}} \mid^{ \gamma_{{\mathrm{1}}} }   \blacktriangleleft _{ 0 }^{\binder{ \gamma_{{\mathrm{2}}} } }  \vdash^{ \gamma_{{\mathrm{2}}} }_{ R }   \refenvnt{e_{{\mathrm{1}}}} ^{ 0  }  :  \langle \refenvnt{A} \rangle^{ \gamma_{{\mathrm{3}}} }   \\
                       \Psi_{{\mathrm{1}}} \mid^{ \gamma_{{\mathrm{1}}} } \varepsilon \vdash \gamma_{{\mathrm{3}}} \preceq \gamma_{{\mathrm{1}}} 
                    }{
                       \Psi_{{\mathrm{1}}} \mid^{ \gamma_{{\mathrm{1}}} }  \varepsilon \vdash^{ \gamma_{{\mathrm{1}}} }_{ R }   { \mathdollar }_{ 0 }\lbrace  \refenvnt{e_{{\mathrm{1}}}} ^{ 0  }  \rbrace  : \refenvnt{A} 
                    }
                  \end{mathpar}
                  for some $\gamma_{{\mathrm{2}}}$ and $\gamma_{{\mathrm{3}}}$.

                  Let $\Psi_{{\mathrm{2}}} = \Psi_{{\mathrm{1}}}  \refenvsym{,}   \binder{ \gamma_{{\mathrm{2}}} }( \mathbin{:\succeq} \; \gamma_{{\mathrm{1}}}  /  \mathbin{:\supseteq} \; \gamma_{{\mathrm{1}}} ) $.
                  By \zcref{claim:promotion}, we have
                  $ \Psi_{{\mathrm{2}}} \mid^{ \gamma_{{\mathrm{2}}} }  \varepsilon \vdash^{ \gamma_{{\mathrm{2}}} }_{ R }   \refenvnt{e_{{\mathrm{1}}}} ^{ 0  }  :  \langle \refenvnt{A} \rangle^{ \gamma_{{\mathrm{3}}} }  $.
                  We have $ \token{Dom}_{V}( \Psi_{{\mathrm{2}}} )  =  \token{Dom}_{V}( \Psi_{{\mathrm{1}}} ) $, and
                  $ \Psi_{{\mathrm{2}}} \mid \Theta_{{\mathrm{1}}} \vdash^{ \gamma_{{\mathrm{2}}} } E \ \token{wf} $ by
                  \ref{rule:runtime-wf-venv-name-cls}.  Also,
                  $\Psi_{{\mathrm{2}}}  \vdash  S_{{\mathrm{1}}}  \colon  \Theta_{{\mathrm{1}}}$ follows by weakening.
                  Hence, by the induction hypothesis on $ \refenvnt{e_{{\mathrm{1}}}} ^{ 0  } $, we have
                  either of the following.
                  \begin{itemize}
                    \item $\mathcal{V}^{\mathrm{rt} }  \refenvsym{(}   \refenvnt{e_{{\mathrm{1}}}} ^{ 0  }   \refenvsym{,}  E  \refenvsym{,}  R  \refenvsym{,}   \token{Dom}_{V}( \Psi_{{\mathrm{2}}} )   \refenvsym{,}  S_{{\mathrm{1}}}  \refenvsym{,}  \refenvnt{k_{{\mathrm{2}}}}  \refenvsym{-}  1  \refenvsym{)} =  \token{Timeout} $
                    \item We have $\refenvnt{v_{{\mathrm{1}}}}$, $\Psi_{{\mathrm{3}}}$, $S_{{\mathrm{2}}}$ and $\Theta_{{\mathrm{2}}}$ such that
                          \begin{itemize}
                            \item $\mathcal{V}^{\mathrm{rt} }  \refenvsym{(}   \refenvnt{e_{{\mathrm{1}}}} ^{ 0  }   \refenvsym{,}  E  \refenvsym{,}  R  \refenvsym{,}   \token{Dom}_{V}( \Psi_{{\mathrm{2}}} )   \refenvsym{,}  S_{{\mathrm{1}}}  \refenvsym{,}  \refenvnt{k_{{\mathrm{2}}}}  \refenvsym{-}  1  \refenvsym{)} = \token{Done} \, \refenvsym{(}  \refenvnt{v_{{\mathrm{1}}}}  \refenvsym{,}   \token{Dom}_{V}( \Psi_{{\mathrm{3}}} )   \refenvsym{,}  S_{{\mathrm{2}}}  \refenvsym{)}$
                            \item $ \Psi_{{\mathrm{3}}} \mid \Theta_{{\mathrm{2}}} \vdash^{ \gamma_{{\mathrm{2}}} } \refenvnt{v_{{\mathrm{1}}}} :  \langle \refenvnt{A} \rangle^{ \gamma_{{\mathrm{3}}} }  \ \token{val} $
                            \item $\Psi_{{\mathrm{3}}}  \vdash  S_{{\mathrm{2}}}  \colon  \Theta_{{\mathrm{2}}}$
                            \item $ \Psi_{{\mathrm{2}}} \subseteq \Psi_{{\mathrm{3}}} $
                            \item $ \Theta_{{\mathrm{1}}} \subseteq \Theta_{{\mathrm{2}}} $
                          \end{itemize}
                  \end{itemize}
                  The first case is trivial, and we consider the second case.
                  By inverting the typing of $\refenvnt{v_{{\mathrm{1}}}}$, we have
                  $ \Psi_{{\mathrm{3}}} \mid^{ \gamma_{{\mathrm{2}}} }  \varepsilon \vdash^{ \gamma_{{\mathrm{2}}} }_{  \token{id}  }   \langle   \refenvnt{e_{{\mathrm{2}}}} ^{ 0  }   \rangle  :  \langle \refenvnt{A} \rangle^{ \gamma_{{\mathrm{3}}} }  $
                  for some $ \refenvnt{e_{{\mathrm{2}}}} ^{ 0  } $ such that $\refenvnt{v_{{\mathrm{1}}}} =  \langle   \refenvnt{e_{{\mathrm{2}}}} ^{ 0  }   \rangle $.
                  By inversion of \ref{rule:runtime-type-quote}, we obtain
                  $ \Psi_{{\mathrm{3}}} \mid^{ \gamma_{{\mathrm{2}}} }   \blacktriangleright ^{ \gamma_{{\mathrm{3}}} }  \vdash^{ \gamma_{{\mathrm{2}}}  \refenvsym{,}  \gamma_{{\mathrm{3}}} }_{  \token{id}  }   \refenvnt{e_{{\mathrm{2}}}} ^{ 0  }  : \refenvnt{A} $.
                  Hence \zcref{claim:unlift-quote-body} gives
                  $ \Psi_{{\mathrm{3}}} \mid^{ \gamma_{{\mathrm{3}}} }  \varepsilon \vdash^{ \gamma_{{\mathrm{3}}} }_{  \token{id}  }   \refenvnt{e_{{\mathrm{2}}}} ^{ 0  }  : \refenvnt{A} $.
                  By weakening the premise $ \Psi_{{\mathrm{1}}} \mid^{ \gamma_{{\mathrm{1}}} } \varepsilon \vdash \gamma_{{\mathrm{3}}} \preceq \gamma_{{\mathrm{1}}} $
                  along $ \Psi_{{\mathrm{1}}} \subseteq \Psi_{{\mathrm{2}}} $ and $ \Psi_{{\mathrm{2}}} \subseteq \Psi_{{\mathrm{3}}} $, and then
                  applying \zcref{claim:local-to-global-trans}, we obtain
                  $\Psi_{{\mathrm{3}}}  \vdash  \gamma_{{\mathrm{3}}}  \preceq  \gamma_{{\mathrm{1}}}$.  Hence
                  \zcref{claim:nht-monotonicity} gives
                  $ \Psi_{{\mathrm{3}}} \mid^{ \gamma_{{\mathrm{1}}} }  \varepsilon \vdash^{ \gamma_{{\mathrm{1}}} }_{  \token{id}  }   \refenvnt{e_{{\mathrm{2}}}} ^{ 0  }  : \refenvnt{A} $.
                  Moreover, $ \Psi_{{\mathrm{3}}} \mid \Theta_{{\mathrm{2}}} \vdash^{ \gamma_{{\mathrm{1}}} } E \ \token{wf} $ follows by
                  weakening, since $ \Psi_{{\mathrm{1}}} \subseteq \Psi_{{\mathrm{2}}} $, $ \Psi_{{\mathrm{2}}} \subseteq \Psi_{{\mathrm{3}}} $, and
                  $ \Theta_{{\mathrm{1}}} \subseteq \Theta_{{\mathrm{2}}} $.  Thus, by the induction hypothesis on
                  $ \refenvnt{e_{{\mathrm{2}}}} ^{ 0  } $, we have the following.
                  \begin{itemize}
                    \item $\mathcal{V}^{\mathrm{rt} }  \refenvsym{(}   \refenvnt{e_{{\mathrm{2}}}} ^{ 0  }   \refenvsym{,}  E  \refenvsym{,}   \token{id}   \refenvsym{,}   \token{Dom}_{V}( \Psi_{{\mathrm{3}}} )   \refenvsym{,}  S_{{\mathrm{2}}}  \refenvsym{,}  \refenvnt{k_{{\mathrm{2}}}}  \refenvsym{-}  1  \refenvsym{)} =  \token{Timeout} $
                    \item We have $\refenvnt{v_{{\mathrm{2}}}}$, $\Psi_{{\mathrm{4}}}$, $S_{{\mathrm{3}}}$ and $\Theta_{{\mathrm{3}}}$ such that
                          \begin{itemize}
                            \item $\mathcal{V}^{\mathrm{rt} }  \refenvsym{(}   \refenvnt{e_{{\mathrm{2}}}} ^{ 0  }   \refenvsym{,}  E  \refenvsym{,}   \token{id}   \refenvsym{,}   \token{Dom}_{V}( \Psi_{{\mathrm{3}}} )   \refenvsym{,}  S_{{\mathrm{2}}}  \refenvsym{,}  \refenvnt{k_{{\mathrm{2}}}}  \refenvsym{-}  1  \refenvsym{)} = \token{Done} \, \refenvsym{(}  \refenvnt{v_{{\mathrm{2}}}}  \refenvsym{,}   \token{Dom}_{V}( \Psi_{{\mathrm{4}}} )   \refenvsym{,}  S_{{\mathrm{3}}}  \refenvsym{)}$
                            \item $ \Psi_{{\mathrm{4}}} \mid \Theta_{{\mathrm{3}}} \vdash^{ \gamma_{{\mathrm{1}}} } \refenvnt{v_{{\mathrm{2}}}} : \refenvnt{A} \ \token{val} $
                            \item $\Psi_{{\mathrm{4}}}  \vdash  S_{{\mathrm{3}}}  \colon  \Theta_{{\mathrm{3}}}$
                            \item $ \Psi_{{\mathrm{3}}} \subseteq \Psi_{{\mathrm{4}}} $
                            \item $ \Theta_{{\mathrm{2}}} \subseteq \Theta_{{\mathrm{3}}} $
                          \end{itemize}
                  \end{itemize}
                  The first case is trivial, and we consider the second case.
                  Since $ \token{Dom}_{V}( \Psi_{{\mathrm{2}}} )  =  \token{Dom}_{V}( \Psi_{{\mathrm{1}}} ) $, the definition of
                  $ \mathcal{V}^{\mathrm{rt} } $ gives
                  $\mathcal{V}^{\mathrm{rt} }  \refenvsym{(}   { \mathdollar }_{ 0 }\lbrace  \refenvnt{e_{{\mathrm{1}}}} ^{ 0  }  \rbrace   \refenvsym{,}  E  \refenvsym{,}  R  \refenvsym{,}   \token{Dom}_{V}( \Psi_{{\mathrm{1}}} )   \refenvsym{,}  S_{{\mathrm{1}}}  \refenvsym{,}  \refenvnt{k_{{\mathrm{2}}}}  \refenvsym{)} = \token{Done} \, \refenvsym{(}  \refenvnt{v_{{\mathrm{2}}}}  \refenvsym{,}   \token{Dom}_{V}( \Psi_{{\mathrm{4}}} )   \refenvsym{,}  S_{{\mathrm{3}}}  \refenvsym{)}$.
                  Therefore we are done.

            \item[Case \textmd{$ \refenvnt{e} ^{ 0  }  = \token{ref} \, \refenvsym{(}   \refenvnt{e_{{\mathrm{1}}}} ^{ 0  }   \refenvsym{)}$}:]
                  We are given
                  \begin{mathpar}
                    \inferrule*[left={\ref{rule:runtime-type-ref}}]{
                       \Psi_{{\mathrm{1}}} \mid^{ \gamma_{{\mathrm{1}}} }  \varepsilon \vdash^{ \gamma_{{\mathrm{1}}} }_{ R }   \refenvnt{e_{{\mathrm{1}}}} ^{ 0  }  : \refenvnt{A_{{\mathrm{1}}}} 
                    }{
                       \Psi_{{\mathrm{1}}} \mid^{ \gamma_{{\mathrm{1}}} }  \varepsilon \vdash^{ \gamma_{{\mathrm{1}}} }_{ R }  \token{ref} \, \refenvsym{(}   \refenvnt{e_{{\mathrm{1}}}} ^{ 0  }   \refenvsym{)} :  \refenvnt{A_{{\mathrm{1}}}} \/\ \token{ref}  
                    }
                  \end{mathpar}
                  for some $\refenvnt{A_{{\mathrm{1}}}}$ where $\refenvnt{A} =  \refenvnt{A_{{\mathrm{1}}}} \/\ \token{ref} $.
                  By the induction hypothesis on $ \refenvnt{e_{{\mathrm{1}}}} ^{ 0  } $, we have
                  either of the following.
                  \begin{itemize}
                    \item $\mathcal{V}^{\mathrm{rt} }  \refenvsym{(}   \refenvnt{e_{{\mathrm{1}}}} ^{ 0  }   \refenvsym{,}  E  \refenvsym{,}  R  \refenvsym{,}   \token{Dom}_{V}( \Psi_{{\mathrm{1}}} )   \refenvsym{,}  S_{{\mathrm{1}}}  \refenvsym{,}  \refenvnt{k_{{\mathrm{2}}}}  \refenvsym{-}  1  \refenvsym{)} =  \token{Timeout} $
                    \item We have $\refenvnt{v_{{\mathrm{1}}}}$, $\Psi_{{\mathrm{2}}}$, $S_{{\mathrm{2}}}$ and $\Theta_{{\mathrm{2}}}$ such that
                          \begin{itemize}
                            \item $\mathcal{V}^{\mathrm{rt} }  \refenvsym{(}   \refenvnt{e_{{\mathrm{1}}}} ^{ 0  }   \refenvsym{,}  E  \refenvsym{,}  R  \refenvsym{,}   \token{Dom}_{V}( \Psi_{{\mathrm{1}}} )   \refenvsym{,}  S_{{\mathrm{1}}}  \refenvsym{,}  \refenvnt{k_{{\mathrm{2}}}}  \refenvsym{-}  1  \refenvsym{)} = \token{Done} \, \refenvsym{(}  \refenvnt{v_{{\mathrm{1}}}}  \refenvsym{,}   \token{Dom}_{V}( \Psi_{{\mathrm{2}}} )   \refenvsym{,}  S_{{\mathrm{2}}}  \refenvsym{)}$
                            \item $ \Psi_{{\mathrm{2}}} \mid \Theta_{{\mathrm{2}}} \vdash^{ \gamma_{{\mathrm{1}}} } \refenvnt{v_{{\mathrm{1}}}} : \refenvnt{A_{{\mathrm{1}}}} \ \token{val} $
                            \item $\Psi_{{\mathrm{2}}}  \vdash  S_{{\mathrm{2}}}  \colon  \Theta_{{\mathrm{2}}}$
                            \item $ \Psi_{{\mathrm{1}}} \subseteq \Psi_{{\mathrm{2}}} $
                            \item $ \Theta_{{\mathrm{1}}} \subseteq \Theta_{{\mathrm{2}}} $
                          \end{itemize}
                  \end{itemize}
                  The first case is trivial, and we consider the second case.
                  Let $\refenvmv{l}$ be a location such that $\token{alloc} \, \refenvsym{(}  S_{{\mathrm{2}}}  \refenvsym{)} = \token{Done} \, \refenvsym{(}  \refenvmv{l}  \refenvsym{)}$.  Since
                  $\refenvmv{l} \, \not\in \,  \token{Dom}_{L}( S_{{\mathrm{2}}} ) $, define
                  $S_{{\mathrm{3}}} = S_{{\mathrm{2}}}  \refenvsym{,}  \refenvmv{l}  \coloneqq  \refenvnt{v_{{\mathrm{1}}}}$ and
                  $\Theta_{{\mathrm{3}}} = \Theta_{{\mathrm{2}}}  \refenvsym{,}   \refenvmv{l} : \refenvnt{A_{{\mathrm{1}}}} $.
                  By the definition of $ \mathcal{V}^{\mathrm{rt} } $,
                  \[
                    \mathcal{V}^{\mathrm{rt} }  \refenvsym{(}  \token{ref} \, \refenvsym{(}   \refenvnt{e_{{\mathrm{1}}}} ^{ 0  }   \refenvsym{)}  \refenvsym{,}  E  \refenvsym{,}  R  \refenvsym{,}   \token{Dom}_{V}( \Psi_{{\mathrm{1}}} )   \refenvsym{,}  S_{{\mathrm{1}}}  \refenvsym{,}  \refenvnt{k_{{\mathrm{2}}}}  \refenvsym{)}
                    =
                    \token{Done} \, \refenvsym{(}  \refenvmv{l}  \refenvsym{,}   \token{Dom}_{V}( \Psi_{{\mathrm{2}}} )   \refenvsym{,}  S_{{\mathrm{3}}}  \refenvsym{)}.
                  \]
                  It remains to show
                  $ \Psi_{{\mathrm{2}}} \mid \Theta_{{\mathrm{3}}} \vdash^{ \gamma_{{\mathrm{1}}} } \refenvmv{l} :  \refenvnt{A_{{\mathrm{1}}}} \/\ \token{ref}  \ \token{val} $ and
                  $\Psi_{{\mathrm{2}}}  \vdash  S_{{\mathrm{3}}}  \colon  \Theta_{{\mathrm{3}}}$.  The former follows from
                  \ref{rule:value-type-loc}.  The latter follows from
                  \ref{rule:type-store}, using the store typing of
                  $S_{{\mathrm{2}}}$ and the value typing of $\refenvnt{v_{{\mathrm{1}}}}$.

            \item[Case \textmd{$ \refenvnt{e} ^{ 0  }  =   \refenvnt{e_{{\mathrm{1}}}} ^{ 0  }  \coloneqq  \refenvnt{e_{{\mathrm{2}}}} ^{ 0  }  $}:]
                  By \zcref{claim:safety-assignment}.

            \item[Case \textmd{$ \refenvnt{e} ^{ 0  }  =  \token{deref}(  \refenvnt{e_{{\mathrm{1}}}} ^{ 0  }  ) $}:]
                  By \zcref{claim:safety-lookup-store}.

          \end{description}


    \item[\zcref{item:type-soundness:future}]: The case where $\refenvnt{k_{{\mathrm{2}}}} = 0$ is trivial. We consider the case where $\refenvnt{k_{{\mathrm{2}}}} > 0$.
          We perform case analysis on $\refenvnt{e}$ and its last derivation.

          \begin{description}
            \item[Case \textmd{Last derivation is \ref{rule:runtime-type-appcls}}:]
                  Let $\varrho =  \binder{  \delta _{ 1 }  }  \mathbin{:\succeq}    \delta' _{ 1 }  ,\dotsc,\binder{  \delta _{ \refenvnt{k} }  }  \mathbin{:\succeq}    \delta' _{ \refenvnt{k} }  $ and
                  $\sigma =   \delta _{ 1 }  \coloneqq  \delta'' _{ 1 }  ,\dotsc,  \delta _{ \refenvnt{k} }  \coloneqq  \delta'' _{ \refenvnt{k} }  $.
                  We are given
                  \begin{mathpar}
                    \inferrule*[left={\ref{rule:runtime-type-appcls}}]{
                       \Psi_{{\mathrm{1}}} \mid^{   \gamma _{ 0 }  ,\dotsc,  \gamma _{  \refenvnt{k_{{\mathrm{1}}}} ^{+}  }   }  \varepsilon \vdash^{   \gamma _{ 0 }  ,\dotsc,  \gamma _{  \refenvnt{k_{{\mathrm{1}}}} ^{+}  }   }_{ R }   \refenvnt{e_{{\mathrm{1}}}} ^{  \refenvnt{k_{{\mathrm{1}}}} ^{+}   }  :  \forall  \varrho . \refenvnt{A'}   \\
                       \Psi_{{\mathrm{1}}} \mid^{   \gamma _{ 0 }  ,\dotsc,  \gamma _{  \refenvnt{k_{{\mathrm{1}}}} ^{+}  }   } \varepsilon \vdash  \delta' _{ \refenvnt{i} }  \preceq  \delta'' _{ \refenvnt{i} }  
                        \text{\ for\ } 1 \le \refenvnt{i} \le \refenvnt{k} \\
                       \Psi_{{\mathrm{1}}} \mid^{   \gamma _{ 0 }  ,\dotsc,  \gamma _{  \refenvnt{k_{{\mathrm{1}}}} ^{+}  }   } \varepsilon \vdash  \delta'' _{ \refenvnt{i}  \refenvsym{+}  1 }  \subseteq  \delta'' _{ \refenvnt{i} }  
                        \text{\ for\ } 0 \le \refenvnt{i} < \refenvnt{k}
                    }{
                       \Psi_{{\mathrm{1}}} \mid^{   \gamma _{ 0 }  ,\dotsc,  \gamma _{  \refenvnt{k_{{\mathrm{1}}}} ^{+}  }   }  \varepsilon \vdash^{   \gamma _{ 0 }  ,\dotsc,  \gamma _{  \refenvnt{k_{{\mathrm{1}}}} ^{+}  }   }_{ R }   \refenvnt{e_{{\mathrm{1}}}} ^{  \refenvnt{k_{{\mathrm{1}}}} ^{+}   }  : \refenvnt{A'}  \refenvsym{[}  \sigma  \refenvsym{]} 
                    }
                  \end{mathpar}
                  where $ \delta'' _{ 0 }  =  \gamma _{  \refenvnt{k_{{\mathrm{1}}}} ^{+}  } $ and
                  $\refenvnt{A} = \refenvnt{A'}  \refenvsym{[}  \sigma  \refenvsym{]}$.

                  By the induction hypothesis applied to the premise typing
                  derivation, either of the following holds:
                  \begin{itemize}
                    \item $\mathcal{V}^{\mathrm{fut} }  \refenvsym{(}  \refenvnt{k_{{\mathrm{1}}}}  \refenvsym{,}   \refenvnt{e_{{\mathrm{1}}}} ^{  \refenvnt{k_{{\mathrm{1}}}} ^{+}   }   \refenvsym{,}  E  \refenvsym{,}  R  \refenvsym{,}   \token{Dom}_{V}( \Psi_{{\mathrm{1}}} )   \refenvsym{,}  S_{{\mathrm{1}}}  \refenvsym{,}  \refenvnt{k_{{\mathrm{2}}}}  \refenvsym{)} =  \token{Timeout} $
                    \item We have $ \refenvnt{e_{{\mathrm{2}}}} ^{ \refenvnt{k_{{\mathrm{1}}}}  } $, $\Psi_{{\mathrm{2}}}$, $S_{{\mathrm{2}}}$ and
                          $\Theta_{{\mathrm{2}}}$ such that
                          \begin{itemize}
                            \item $\mathcal{V}^{\mathrm{fut} }  \refenvsym{(}  \refenvnt{k_{{\mathrm{1}}}}  \refenvsym{,}   \refenvnt{e_{{\mathrm{1}}}} ^{  \refenvnt{k_{{\mathrm{1}}}} ^{+}   }   \refenvsym{,}  E  \refenvsym{,}  R  \refenvsym{,}   \token{Dom}_{V}( \Psi_{{\mathrm{1}}} )   \refenvsym{,}  S_{{\mathrm{1}}}  \refenvsym{,}  \refenvnt{k_{{\mathrm{2}}}}  \refenvsym{)}
                                  = \token{Done} \, \refenvsym{(}   \refenvnt{e_{{\mathrm{2}}}} ^{ \refenvnt{k_{{\mathrm{1}}}}  }   \refenvsym{,}   \token{Dom}_{V}( \Psi_{{\mathrm{2}}} )   \refenvsym{,}  S_{{\mathrm{2}}}  \refenvsym{)}$
                            \item $ \Psi_{{\mathrm{2}}} \mid^{   \gamma _{ 1 }  ,\dotsc,  \gamma _{ \refenvnt{k_{{\mathrm{1}}}} }   }  \varepsilon \vdash^{   \gamma _{ 1 }  ,\dotsc,  \gamma _{ \refenvnt{k_{{\mathrm{1}}}} }   }_{  \token{id}  }   \refenvnt{e_{{\mathrm{2}}}} ^{ \refenvnt{k_{{\mathrm{1}}}}  }  :  \forall  \varrho . \refenvnt{A'}  $
                            \item $\Psi_{{\mathrm{2}}}  \vdash  S_{{\mathrm{2}}}  \colon  \Theta_{{\mathrm{2}}}$
                            \item $ \Psi_{{\mathrm{1}}} \subseteq \Psi_{{\mathrm{2}}} $
                            \item $ \Theta_{{\mathrm{1}}} \subseteq \Theta_{{\mathrm{2}}} $
                          \end{itemize}
                  \end{itemize}
                  The first case is trivial, and we consider the second case.
                  By weakening along $ \Psi_{{\mathrm{1}}} \subseteq \Psi_{{\mathrm{2}}} $ and then applying
                  \zcref{claim:local-to-global-trans}, the reachability/visibility premises
                  become global judgments over $\Psi_{{\mathrm{2}}}$. Applying
                  \zcref{claim:global-to-local-trans} to the residual stack $  \gamma _{ 1 }  ,\dotsc,  \gamma _{ \refenvnt{k} }  $
                  gives
                  \begin{itemize}
                    \item $ \Psi_{{\mathrm{2}}} \mid^{   \gamma _{ 1 }  ,\dotsc,  \gamma _{ \refenvnt{k_{{\mathrm{1}}}} }   } \varepsilon \vdash  \delta' _{ \refenvnt{i} }  \preceq  \delta'' _{ \refenvnt{i} }  $
                          for each $\refenvnt{i}$ with $1 \le \refenvnt{i} \le \refenvnt{k}$,
                    \item $ \Psi_{{\mathrm{2}}} \mid^{   \gamma _{ 1 }  ,\dotsc,  \gamma _{ \refenvnt{k_{{\mathrm{1}}}} }   } \varepsilon \vdash  \delta'' _{ \refenvnt{i}  \refenvsym{+}  1 }  \subseteq  \delta'' _{ \refenvnt{i} }  $
                          for each $\refenvnt{i}$ with $0 \le \refenvnt{i} < \refenvnt{k}$.
                  \end{itemize}
                  Reapplying \ref{rule:runtime-type-appcls} gives
                  \[
                     \Psi_{{\mathrm{2}}} \mid^{   \gamma _{ 1 }  ,\dotsc,  \gamma _{ \refenvnt{k_{{\mathrm{1}}}} }   }  \varepsilon \vdash^{   \gamma _{ 1 }  ,\dotsc,  \gamma _{ \refenvnt{k_{{\mathrm{1}}}} }   }_{  \token{id}  }   \refenvnt{e_{{\mathrm{2}}}} ^{ \refenvnt{k_{{\mathrm{1}}}}  }  : \refenvnt{A'}  \refenvsym{[}  \sigma  \refenvsym{]} .
                  \]
                  This is what we want.

            %% koko made yatta
            \item[Case \textmd{$ \refenvnt{e} ^{  \refenvnt{k_{{\mathrm{1}}}} ^{+}   }  =   \lambda \binder{ \refenvmv{x} }.\  \refenvnt{e_{{\mathrm{1}}}}  ^{  \refenvnt{k_{{\mathrm{1}}}} ^{+}   } $}:]
                By \zcref{claim:inversion-runtime-typing},
                it is derived by \ref{rule:runtime-type-func} or
                \ref{rule:runtime-type-polycls}.

                In the former case, we are given
                \begin{mathpar}
                  \inferrule*[left={\ref{rule:runtime-type-func}}]{
                     \Psi_{{\mathrm{1}}} \mid^{   \gamma _{ 0 }  ,\dotsc,  \gamma _{  \refenvnt{k_{{\mathrm{1}}}} ^{+}  }   }   \binder{ \refenvmv{x} }\mathord{:^{\binder{ \gamma'_{{\mathrm{1}}} } } } \refenvnt{A_{{\mathrm{1}}}}  \vdash^{   \gamma _{ 0 }  ,\dotsc,  \gamma _{ \refenvnt{k_{{\mathrm{1}}}} }    \refenvsym{,}  \gamma'_{{\mathrm{1}}} }_{ R }   \refenvnt{e_{{\mathrm{1}}}} ^{  \refenvnt{k_{{\mathrm{1}}}} ^{+}   }  : \refenvnt{A_{{\mathrm{2}}}}  \\
                    \gamma'_{{\mathrm{1}}} \, \not\in \,  \token{FC}( \refenvnt{A_{{\mathrm{2}}}} )  \\
                     \Psi_{{\mathrm{1}}} \mid^{   \gamma _{ 0 }  ,\dotsc,  \gamma _{  \refenvnt{k_{{\mathrm{1}}}} ^{+}  }   } \varepsilon \vdash^{   \gamma _{ 0 }  ,\dotsc,  \gamma _{ \refenvnt{k_{{\mathrm{1}}}} }    \refenvsym{,}   \gamma _{  \refenvnt{k_{{\mathrm{1}}}} ^{+}  }  }\token{wf} 
                  }{
                     \Psi_{{\mathrm{1}}} \mid^{   \gamma _{ 0 }  ,\dotsc,  \gamma _{  \refenvnt{k_{{\mathrm{1}}}} ^{+}  }   }  \varepsilon \vdash^{   \gamma _{ 0 }  ,\dotsc,  \gamma _{  \refenvnt{k_{{\mathrm{1}}}} ^{+}  }   }_{ R }    \lambda \binder{ \refenvmv{x} }.\  \refenvnt{e_{{\mathrm{1}}}}  ^{  \refenvnt{k_{{\mathrm{1}}}} ^{+}   }  : \refenvnt{A_{{\mathrm{1}}}}  \rightarrow  \refenvnt{A_{{\mathrm{2}}}} 
                  }
                \end{mathpar}
                for some $\refenvnt{A_{{\mathrm{1}}}}$, $\refenvnt{A_{{\mathrm{2}}}}$ and $\gamma'_{{\mathrm{1}}}$.

                Let $\refenvmv{y} = \token{gensym} \, \refenvsym{(}   \token{Dom}_{V}( \Psi_{{\mathrm{1}}} )   \refenvsym{)}$ and
                $\Psi_{{\mathrm{2}}} = \Psi_{{\mathrm{1}}}  \refenvsym{,}   \binder{ \refenvmv{y} }: \refenvnt{A_{{\mathrm{1}}}} \mathrel{@}\binder{ \gamma'_{{\mathrm{1}}} } \mathbin{:\succeq}  \gamma _{  \refenvnt{k_{{\mathrm{1}}}} ^{+}  }  $.
                By \zcref{claim:promotion}, we have
                \[
                   \Psi_{{\mathrm{2}}} \mid^{   \gamma _{ 0 }  ,\dotsc,  \gamma _{ \refenvnt{k_{{\mathrm{1}}}} }    \refenvsym{,}  \gamma'_{{\mathrm{1}}} }  \varepsilon \vdash^{   \gamma _{ 0 }  ,\dotsc,  \gamma _{ \refenvnt{k_{{\mathrm{1}}}} }    \refenvsym{,}  \gamma'_{{\mathrm{1}}} }_{ R  \refenvsym{,}  \refenvmv{x}  \coloneqq  \refenvmv{y} }   \refenvnt{e_{{\mathrm{1}}}} ^{  \refenvnt{k_{{\mathrm{1}}}} ^{+}   }  : \refenvnt{A_{{\mathrm{2}}}} .
                \]
                Moreover, $ \token{Dom}_{V}( \Psi_{{\mathrm{2}}} )  =  \token{Dom}_{V}( \Psi_{{\mathrm{1}}} )   \refenvsym{,}  \refenvmv{y}$.
                By weakening along $ \Psi_{{\mathrm{1}}} \subseteq \Psi_{{\mathrm{2}}} $, we also have
                $ \Psi_{{\mathrm{2}}} \mid \Theta_{{\mathrm{1}}} \vdash^{  \gamma _{ 0 }  } E \ \token{wf} $ and
                $\Psi_{{\mathrm{2}}}  \vdash  S_{{\mathrm{1}}}  \colon  \Theta_{{\mathrm{1}}}$.
                Hence, by the induction hypothesis on $ \refenvnt{e_{{\mathrm{1}}}} ^{  \refenvnt{k_{{\mathrm{1}}}} ^{+}   } $, either
                of the following holds:
                \begin{itemize}
                  \item $\mathcal{V}^{\mathrm{fut} }  \refenvsym{(}  \refenvnt{k_{{\mathrm{1}}}}  \refenvsym{,}   \refenvnt{e_{{\mathrm{1}}}} ^{  \refenvnt{k_{{\mathrm{1}}}} ^{+}   }   \refenvsym{,}  E  \refenvsym{,}  \refenvsym{(}  R  \refenvsym{,}  \refenvmv{x}  \coloneqq  \refenvmv{y}  \refenvsym{)}  \refenvsym{,}   \token{Dom}_{V}( \Psi_{{\mathrm{2}}} )   \refenvsym{,}  S_{{\mathrm{1}}}  \refenvsym{,}  \refenvnt{k_{{\mathrm{2}}}}  \refenvsym{-}  1  \refenvsym{)} =  \token{Timeout} $
                  \item We have $ \refenvnt{e_{{\mathrm{2}}}} ^{ \refenvnt{k_{{\mathrm{1}}}}  } $, $\Psi_{{\mathrm{3}}}$, $S_{{\mathrm{2}}}$,
                        and $\Theta_{{\mathrm{2}}}$ such that
                        \begin{itemize}
                          \item $\mathcal{V}^{\mathrm{fut} }  \refenvsym{(}  \refenvnt{k_{{\mathrm{1}}}}  \refenvsym{,}   \refenvnt{e_{{\mathrm{1}}}} ^{  \refenvnt{k_{{\mathrm{1}}}} ^{+}   }   \refenvsym{,}  E  \refenvsym{,}  \refenvsym{(}  R  \refenvsym{,}  \refenvmv{x}  \coloneqq  \refenvmv{y}  \refenvsym{)}  \refenvsym{,}   \token{Dom}_{V}( \Psi_{{\mathrm{2}}} )   \refenvsym{,}  S_{{\mathrm{1}}}  \refenvsym{,}  \refenvnt{k_{{\mathrm{2}}}}  \refenvsym{-}  1  \refenvsym{)}
                                = \token{Done} \, \refenvsym{(}   \refenvnt{e_{{\mathrm{2}}}} ^{ \refenvnt{k_{{\mathrm{1}}}}  }   \refenvsym{,}   \token{Dom}_{V}( \Psi_{{\mathrm{3}}} )   \refenvsym{,}  S_{{\mathrm{2}}}  \refenvsym{)}$
                          \item $ \Psi_{{\mathrm{3}}} \mid^{   \gamma _{ 1 }  ,\dotsc,  \gamma _{ \refenvnt{k_{{\mathrm{1}}}} }    \refenvsym{,}  \gamma'_{{\mathrm{1}}} }  \varepsilon \vdash^{   \gamma _{ 1 }  ,\dotsc,  \gamma _{ \refenvnt{k_{{\mathrm{1}}}} }    \refenvsym{,}  \gamma'_{{\mathrm{1}}} }_{  \token{id}  }   \refenvnt{e_{{\mathrm{2}}}} ^{ \refenvnt{k_{{\mathrm{1}}}}  }  : \refenvnt{A_{{\mathrm{2}}}} $
                          \item $\Psi_{{\mathrm{3}}}  \vdash  S_{{\mathrm{2}}}  \colon  \Theta_{{\mathrm{2}}}$
                          \item $ \Psi_{{\mathrm{2}}} \subseteq \Psi_{{\mathrm{3}}} $
                          \item $ \Theta_{{\mathrm{1}}} \subseteq \Theta_{{\mathrm{2}}} $
                        \end{itemize}
                \end{itemize}
                The first case is trivial, and we consider the second case.
                Since $\gamma'_{{\mathrm{1}}} \, \not\in \,  \token{FC}( \refenvnt{A_{{\mathrm{2}}}} ) $, the demotion does not change
                the result type: $\refenvnt{A_{{\mathrm{2}}}}  \refenvsym{[}  \gamma'_{{\mathrm{1}}}  \coloneqq  \gamma'_{{\mathrm{2}}}  \refenvsym{]} = \refenvnt{A_{{\mathrm{2}}}}$.  Thus, by
                \zcref{claim:demotion}, using $ \Psi_{{\mathrm{2}}} \subseteq \Psi_{{\mathrm{3}}} $, we have
                \[
                   \Psi_{{\mathrm{3}}} \mid^{   \gamma _{ 1 }  ,\dotsc,  \gamma _{ \refenvnt{k_{{\mathrm{1}}}} }   }   \binder{ \refenvmv{y} }\mathord{:^{\binder{ \gamma'_{{\mathrm{2}}} } } } \refenvnt{A_{{\mathrm{1}}}}  \vdash^{   \gamma _{ 1 }  ,\dotsc,  \gamma _{ \refenvnt{k_{{\mathrm{1}}}} }    \refenvsym{,}  \gamma'_{{\mathrm{2}}} }_{  \token{id}  }   \refenvnt{e_{{\mathrm{2}}}} ^{ \refenvnt{k_{{\mathrm{1}}}}  }  : \refenvnt{A_{{\mathrm{2}}}} .
                \]
                for fresh $\gamma'_{{\mathrm{2}}}$.
                Reapplying \ref{rule:runtime-type-func} gives
                \[
                   \Psi_{{\mathrm{3}}} \mid^{   \gamma _{ 1 }  ,\dotsc,  \gamma _{ \refenvnt{k_{{\mathrm{1}}}} }   }  \varepsilon \vdash^{   \gamma _{ 1 }  ,\dotsc,  \gamma _{ \refenvnt{k_{{\mathrm{1}}}} }   }_{  \token{id}  }    \lambda \binder{ \refenvmv{y} }.\  \refenvnt{e_{{\mathrm{2}}}}  ^{ \refenvnt{k_{{\mathrm{1}}}}  }  : \refenvnt{A_{{\mathrm{1}}}}  \rightarrow  \refenvnt{A_{{\mathrm{2}}}} .
                \]
                Since $\mathcal{V}^{\mathrm{fut} }  \refenvsym{(}  \refenvnt{k_{{\mathrm{1}}}}  \refenvsym{,}    \lambda \binder{ \refenvmv{x} }.\  \refenvnt{e_{{\mathrm{1}}}}  ^{  \refenvnt{k_{{\mathrm{1}}}} ^{+}   }   \refenvsym{,}  E  \refenvsym{,}  R  \refenvsym{,}   \token{Dom}_{V}( \Psi_{{\mathrm{1}}} )   \refenvsym{,}  S_{{\mathrm{1}}}  \refenvsym{,}  \refenvnt{k_{{\mathrm{2}}}}  \refenvsym{)}
                =
                \token{Done} \, \refenvsym{(}    \lambda \binder{ \refenvmv{y} }.\  \refenvnt{e_{{\mathrm{2}}}}  ^{ \refenvnt{k_{{\mathrm{1}}}}  }   \refenvsym{,}   \token{Dom}_{V}( \Psi_{{\mathrm{3}}} )   \refenvsym{,}  S_{{\mathrm{2}}}  \refenvsym{)}$ by the
                definition of $ \mathcal{V}^{\mathrm{fut} } $, this is the desired result.

                We next consider the case where $ \refenvnt{e} ^{  \refenvnt{k_{{\mathrm{1}}}} ^{+}   } $ is derived by \ref{rule:runtime-type-polycls}.
                In this case, we are given
                \begin{mathpar}
                  \inferrule*[left={\ref{rule:runtime-type-polycls}}]{
                     \Psi_{{\mathrm{1}}} \mid^{   \gamma _{ 0 }  ,\dotsc,  \gamma _{  \refenvnt{k_{{\mathrm{1}}}} ^{+}  }   }   [    \binder{  \delta _{ 1 }  }  \mathbin{:\succeq}    \delta' _{ 1 }  ,\dotsc,\binder{  \delta _{ \refenvnt{k} }  }  \mathbin{:\succeq}   \delta'  _{ \refenvnt{k} }   ]^{\binder{  \delta _{ 0 }  } }  \vdash^{   \gamma _{ 0 }  ,\dotsc,  \gamma _{ \refenvnt{k_{{\mathrm{1}}}} }    \refenvsym{,}   \delta _{ 0 }  }_{ R }    \lambda \binder{ \refenvmv{x} }.\  \refenvnt{e_{{\mathrm{1}}}}  ^{  \refenvnt{k_{{\mathrm{1}}}} ^{+}   }  : \refenvnt{A'}  \\
                     \delta _{ 0 }  \, \not\in \,  \token{FC}( \refenvnt{A'} )  \\
                     \Psi_{{\mathrm{1}}} \mid^{   \gamma _{ 0 }  ,\dotsc,  \gamma _{  \refenvnt{k_{{\mathrm{1}}}} ^{+}  }   } \varepsilon \vdash^{   \gamma _{ 0 }  ,\dotsc,  \gamma _{ \refenvnt{k_{{\mathrm{1}}}} }    \refenvsym{,}   \delta' _{ 0 }  }\token{wf} 
                  }{
                     \Psi_{{\mathrm{1}}} \mid^{   \gamma _{ 0 }  ,\dotsc,  \gamma _{  \refenvnt{k_{{\mathrm{1}}}} ^{+}  }   }  \varepsilon \vdash^{   \gamma _{ 0 }  ,\dotsc,  \gamma _{ \refenvnt{k_{{\mathrm{1}}}} }    \refenvsym{,}   \delta' _{ 0 }  }_{ R }    \lambda \binder{ \refenvmv{x} }.\  \refenvnt{e_{{\mathrm{1}}}}  ^{  \refenvnt{k_{{\mathrm{1}}}} ^{+}   }  :  \forall    \binder{  \delta _{ 1 }  }  \mathbin{:\succeq}    \delta' _{ 1 }  ,\dotsc,\binder{  \delta _{ \refenvnt{k} }  }  \mathbin{:\succeq}   \delta'  _{ \refenvnt{k} }  . \refenvnt{A'}  
                  }
                \end{mathpar}
                for some $\refenvnt{k}$, $  \delta _{ 0 }  ,\dotsc,  \delta _{ \refenvnt{k} }  $, $  \delta' _{ 0 }  ,\dotsc,  \delta' _{ \refenvnt{k} }  $, and
                $\refenvnt{A'}$, where $ \delta' _{ 0 }  =  \gamma _{  \refenvnt{k_{{\mathrm{1}}}} ^{+}  } $ and
                $\refenvnt{A} =  \forall    \binder{  \delta _{ 1 }  }  \mathbin{:\succeq}    \delta' _{ 1 }  ,\dotsc,\binder{  \delta _{ \refenvnt{k} }  }  \mathbin{:\succeq}   \delta'  _{ \refenvnt{k} }  . \refenvnt{A'} $.

                By \zcref{claim:promotion}, the premise typing judgment can be
                promoted to the reserved-name context.  Let
                \[
                  \Psi_{{\mathrm{2}}} =
                  \Psi_{{\mathrm{1}}}  \refenvsym{,}   [    \binder{  \delta _{ 0 }  }  \mathbin{:\succeq}    \delta' _{ 0 }  ,\dotsc,\binder{  \delta _{ \refenvnt{k} }  }  \mathbin{:\succeq}   \delta'  _{ \refenvnt{k} }   ] .
                \]
                Then
                \[
                   \Psi_{{\mathrm{2}}} \mid^{   \gamma _{ 0 }  ,\dotsc,  \gamma _{ \refenvnt{k_{{\mathrm{1}}}} }    \refenvsym{,}   \delta _{ 0 }  }  \varepsilon \vdash^{   \gamma _{ 0 }  ,\dotsc,  \gamma _{ \refenvnt{k_{{\mathrm{1}}}} }    \refenvsym{,}   \delta _{ 0 }  }_{ R }    \lambda \binder{ \refenvmv{x} }.\  \refenvnt{e_{{\mathrm{1}}}}  ^{  \refenvnt{k_{{\mathrm{1}}}} ^{+}   }  : \refenvnt{A'} .
                \]
                Moreover, $ \token{Dom}_{V}( \Psi_{{\mathrm{2}}} )  =  \token{Dom}_{V}( \Psi_{{\mathrm{1}}} ) $, and the
                environment and store typing premises are preserved by
                weakening along $ \Psi_{{\mathrm{1}}} \subseteq \Psi_{{\mathrm{2}}} $.  Hence, by the induction
                hypothesis applied to this promoted derivation, either of the
                following holds:
                \begin{itemize}
                  \item $\mathcal{V}^{\mathrm{fut} }  \refenvsym{(}  \refenvnt{k_{{\mathrm{1}}}}  \refenvsym{,}    \lambda \binder{ \refenvmv{x} }.\  \refenvnt{e_{{\mathrm{1}}}}  ^{  \refenvnt{k_{{\mathrm{1}}}} ^{+}   }   \refenvsym{,}  E  \refenvsym{,}  R  \refenvsym{,}   \token{Dom}_{V}( \Psi_{{\mathrm{2}}} )   \refenvsym{,}  S_{{\mathrm{1}}}  \refenvsym{,}  \refenvnt{k_{{\mathrm{2}}}}  \refenvsym{)} =  \token{Timeout} $
                  \item We have $ \refenvnt{e_{{\mathrm{2}}}} ^{ \refenvnt{k_{{\mathrm{1}}}}  } $, $\Psi_{{\mathrm{3}}}$, $S_{{\mathrm{2}}}$,
                        and $\Theta_{{\mathrm{2}}}$ such that
                        \begin{itemize}
                          \item $\mathcal{V}^{\mathrm{fut} }  \refenvsym{(}  \refenvnt{k_{{\mathrm{1}}}}  \refenvsym{,}    \lambda \binder{ \refenvmv{x} }.\  \refenvnt{e_{{\mathrm{1}}}}  ^{  \refenvnt{k_{{\mathrm{1}}}} ^{+}   }   \refenvsym{,}  E  \refenvsym{,}  R  \refenvsym{,}   \token{Dom}_{V}( \Psi_{{\mathrm{2}}} )   \refenvsym{,}  S_{{\mathrm{1}}}  \refenvsym{,}  \refenvnt{k_{{\mathrm{2}}}}  \refenvsym{)}
                                = \token{Done} \, \refenvsym{(}   \refenvnt{e_{{\mathrm{2}}}} ^{ \refenvnt{k_{{\mathrm{1}}}}  }   \refenvsym{,}   \token{Dom}_{V}( \Psi_{{\mathrm{3}}} )   \refenvsym{,}  S_{{\mathrm{2}}}  \refenvsym{)}$
                          \item $ \Psi_{{\mathrm{3}}} \mid^{   \gamma _{ 1 }  ,\dotsc,  \gamma _{ \refenvnt{k_{{\mathrm{1}}}} }    \refenvsym{,}   \delta _{ 0 }  }  \varepsilon \vdash^{   \gamma _{ 1 }  ,\dotsc,  \gamma _{ \refenvnt{k_{{\mathrm{1}}}} }    \refenvsym{,}   \delta _{ 0 }  }_{  \token{id}  }   \refenvnt{e_{{\mathrm{2}}}} ^{ \refenvnt{k_{{\mathrm{1}}}}  }  : \refenvnt{A'} $
                          \item $\Psi_{{\mathrm{3}}}  \vdash  S_{{\mathrm{2}}}  \colon  \Theta_{{\mathrm{2}}}$
                          \item $ \Psi_{{\mathrm{2}}} \subseteq \Psi_{{\mathrm{3}}} $
                          \item $ \Theta_{{\mathrm{1}}} \subseteq \Theta_{{\mathrm{2}}} $
                        \end{itemize}
                \end{itemize}
	                The first case is trivial, and we consider the second case.
	                By the definition of $ \mathcal{V}^{\mathrm{fut} } $ for functions, there
	                are some $\refenvmv{y}$ and $ \refenvnt{e'_{{\mathrm{2}}}} ^{ \refenvnt{k_{{\mathrm{1}}}}  } $ such that
	                $ \refenvnt{e_{{\mathrm{2}}}} ^{ \refenvnt{k_{{\mathrm{1}}}}  }  =   \lambda \binder{ \refenvmv{y} }.\  \refenvnt{e'_{{\mathrm{2}}}}  ^{ \refenvnt{k_{{\mathrm{1}}}}  } $.  Hence
	                $ \refenvnt{e_{{\mathrm{2}}}} ^{ \refenvnt{k_{{\mathrm{1}}}}  } $ is an introduction form.
	                By applying the polymorphic-classifier case of
	                \zcref{claim:demotion}, using $ \Psi_{{\mathrm{2}}} \subseteq \Psi_{{\mathrm{3}}} $, we obtain
	                the local premise
                \[
                   \Psi_{{\mathrm{3}}} \mid^{   \gamma _{ 1 }  ,\dotsc,  \gamma _{ \refenvnt{k_{{\mathrm{1}}}} }    \refenvsym{,}   \delta' _{ 0 }  }   [    \binder{  \delta _{ 1 }  }  \mathbin{:\succeq}    \delta' _{ 1 }  ,\dotsc,\binder{  \delta _{ \refenvnt{k} }  }  \mathbin{:\succeq}   \delta'  _{ \refenvnt{k} }   ]^{\binder{  \delta _{ 0 }  } }  \vdash^{   \gamma _{ 1 }  ,\dotsc,  \gamma _{ \refenvnt{k_{{\mathrm{1}}}} }    \refenvsym{,}   \delta _{ 0 }  }_{  \token{id}  }   \refenvnt{e_{{\mathrm{2}}}} ^{ \refenvnt{k_{{\mathrm{1}}}}  }  : \refenvnt{A'} .
                \]
                Reapplying \ref{rule:runtime-type-polycls} gives
                \[
                   \Psi_{{\mathrm{3}}} \mid^{   \gamma _{ 1 }  ,\dotsc,  \gamma _{ \refenvnt{k_{{\mathrm{1}}}} }    \refenvsym{,}   \delta' _{ 0 }  }  \varepsilon \vdash^{   \gamma _{ 1 }  ,\dotsc,  \gamma _{ \refenvnt{k_{{\mathrm{1}}}} }    \refenvsym{,}   \delta' _{ 0 }  }_{  \token{id}  }   \refenvnt{e_{{\mathrm{2}}}} ^{ \refenvnt{k_{{\mathrm{1}}}}  }  :  \forall    \binder{  \delta _{ 1 }  }  \mathbin{:\succeq}    \delta' _{ 1 }  ,\dotsc,\binder{  \delta _{ \refenvnt{k} }  }  \mathbin{:\succeq}   \delta'  _{ \refenvnt{k} }  . \refenvnt{A'}  .
                \]
                Since $ \token{Dom}_{V}( \Psi_{{\mathrm{2}}} )  =  \token{Dom}_{V}( \Psi_{{\mathrm{1}}} ) $ and
                $ \delta' _{ 0 }  =  \gamma _{  \refenvnt{k_{{\mathrm{1}}}} ^{+}  } $, this is exactly the typing
                required for the result of the original
                $ \mathcal{V}^{\mathrm{fut} } $ computation.


            \item[Case \textmd{$ \refenvnt{e} ^{  \refenvnt{k_{{\mathrm{1}}}} ^{+}   }  =   \token{rec}\ \binder{ \refenvmv{f} }(\binder{ \refenvmv{x} }).\  \refenvnt{e_{{\mathrm{1}}}}  ^{  \refenvnt{k_{{\mathrm{1}}}} ^{+}   } $}:]
              Mostly the same as the previous case, but we need to use \ref{rule:runtime-type-rec} instead of \ref{rule:runtime-type-func}.

            \item[Case \textmd{$ \refenvnt{e} ^{  \refenvnt{k_{{\mathrm{1}}}} ^{+}   }  =  \langle   \refenvnt{e_{{\mathrm{1}}}} ^{  \refenvnt{k_{{\mathrm{1}}}}  \refenvsym{+}  2   }   \rangle $}:] By \zcref{claim:demotion}.

            \item[Case \textmd{$ \refenvnt{e} ^{  \refenvnt{k_{{\mathrm{1}}}} ^{+}   }  =  { \mathdollar }_{ \refenvnt{k_{{\mathrm{3}}}} }\lbrace  \refenvnt{e_{{\mathrm{1}}}} ^{   \refenvnt{k_{{\mathrm{1}}}} ^{+}   \refenvsym{-}  \refenvnt{k_{{\mathrm{3}}}}   }  \rbrace $ where $ \refenvnt{k_{{\mathrm{1}}}} ^{+}  > \refenvnt{k_{{\mathrm{3}}}}$}:] By \zcref{claim:demotion}.

            \item[Case \textmd{$ \refenvnt{e} ^{  \refenvnt{k_{{\mathrm{1}}}} ^{+}   }  =  { \mathdollar }_{  \refenvnt{k_{{\mathrm{1}}}} ^{+}  }\lbrace  \refenvnt{e_{{\mathrm{1}}}} ^{ 0  }  \rbrace $}:]
              By \zcref{claim:inversion-runtime-typing}, it is derived by \ref{rule:runtime-type-appcls} or \ref{rule:runtime-type-splice}.
              The former case is already discussed, and we consider the latter case.

              We are given
              \begin{mathpar}
                \inferrule*[left={\ref{rule:runtime-type-splice}}]{
                   \Psi_{{\mathrm{1}}} \mid^{   \gamma _{ 0 }  ,\dotsc,  \gamma _{  \refenvnt{k_{{\mathrm{1}}}} ^{+}  }   }   \blacktriangleleft _{  \refenvnt{k_{{\mathrm{1}}}} ^{+}  }^{\binder{ \delta_{{\mathrm{1}}} } }  \vdash^{ \delta_{{\mathrm{1}}} }_{ R }   \refenvnt{e_{{\mathrm{1}}}} ^{ 0  }  :  \langle \refenvnt{A} \rangle^{ \delta_{{\mathrm{2}}} }   \\
                   \Psi_{{\mathrm{1}}} \mid^{   \gamma _{ 0 }  ,\dotsc,  \gamma _{  \refenvnt{k_{{\mathrm{1}}}} ^{+}  }   } \varepsilon \vdash \delta_{{\mathrm{2}}} \preceq  \gamma _{  \refenvnt{k_{{\mathrm{1}}}} ^{+}  }   \\
                  \delta_{{\mathrm{1}}} \, \not\in \,  \token{FC}( \refenvnt{A} ) 
                }{
                   \Psi_{{\mathrm{1}}} \mid^{   \gamma _{ 0 }  ,\dotsc,  \gamma _{  \refenvnt{k_{{\mathrm{1}}}} ^{+}  }   }  \varepsilon \vdash^{   \gamma _{ 0 }  ,\dotsc,  \gamma _{  \refenvnt{k_{{\mathrm{1}}}} ^{+}  }   }_{ R }   { \mathdollar }_{  \refenvnt{k_{{\mathrm{1}}}} ^{+}  }\lbrace  \refenvnt{e_{{\mathrm{1}}}} ^{ 0  }  \rbrace  : \refenvnt{A} 
                }
              \end{mathpar}
              for some $\delta_{{\mathrm{1}}}$ and $\delta_{{\mathrm{2}}}$.
              Let $\Psi_{{\mathrm{2}}} = \Psi_{{\mathrm{1}}}  \refenvsym{,}   \binder{ \delta_{{\mathrm{1}}} }( \mathbin{:\succeq} \;  \gamma _{ 0 }   /  \mathbin{:\supseteq} \;  \gamma _{  \refenvnt{k_{{\mathrm{1}}}} ^{+}  }  ) $.
              By \zcref{claim:promotion}, we have
              \[
                 \Psi_{{\mathrm{2}}} \mid^{ \delta_{{\mathrm{1}}} }  \varepsilon \vdash^{ \delta_{{\mathrm{1}}} }_{ R }   \refenvnt{e_{{\mathrm{1}}}} ^{ 0  }  :  \langle \refenvnt{A} \rangle^{ \delta_{{\mathrm{2}}} }  .
              \]
              Moreover, $ \token{Dom}_{V}( \Psi_{{\mathrm{2}}} )  =  \token{Dom}_{V}( \Psi_{{\mathrm{1}}} ) $.
              By weakening along $ \Psi_{{\mathrm{1}}} \subseteq \Psi_{{\mathrm{2}}} $, we have
              $ \Psi_{{\mathrm{2}}} \mid \Theta_{{\mathrm{1}}} \vdash^{ \delta_{{\mathrm{1}}} } E \ \token{wf} $ by
              \ref{rule:runtime-wf-venv-name-cls}, and
              $\Psi_{{\mathrm{2}}}  \vdash  S_{{\mathrm{1}}}  \colon  \Theta_{{\mathrm{1}}}$.
              Hence, by the induction hypothesis on $ \refenvnt{e_{{\mathrm{1}}}} ^{ 0  } $, either
              of the following holds:
              \begin{itemize}
                \item $\mathcal{V}^{\mathrm{rt} }  \refenvsym{(}   \refenvnt{e_{{\mathrm{1}}}} ^{ 0  }   \refenvsym{,}  E  \refenvsym{,}  R  \refenvsym{,}   \token{Dom}_{V}( \Psi_{{\mathrm{2}}} )   \refenvsym{,}  S_{{\mathrm{1}}}  \refenvsym{,}  \refenvnt{k_{{\mathrm{2}}}}  \refenvsym{-}  1  \refenvsym{)} =  \token{Timeout} $
                \item We have $\refenvnt{v_{{\mathrm{1}}}}$, $\Psi_{{\mathrm{3}}}$, $S_{{\mathrm{2}}}$ and
                      $\Theta_{{\mathrm{2}}}$ such that
                      \begin{itemize}
                        \item $\mathcal{V}^{\mathrm{rt} }  \refenvsym{(}   \refenvnt{e_{{\mathrm{1}}}} ^{ 0  }   \refenvsym{,}  E  \refenvsym{,}  R  \refenvsym{,}   \token{Dom}_{V}( \Psi_{{\mathrm{2}}} )   \refenvsym{,}  S_{{\mathrm{1}}}  \refenvsym{,}  \refenvnt{k_{{\mathrm{2}}}}  \refenvsym{-}  1  \refenvsym{)}
                              = \token{Done} \, \refenvsym{(}  \refenvnt{v_{{\mathrm{1}}}}  \refenvsym{,}   \token{Dom}_{V}( \Psi_{{\mathrm{3}}} )   \refenvsym{,}  S_{{\mathrm{2}}}  \refenvsym{)}$
                        \item $ \Psi_{{\mathrm{3}}} \mid \Theta_{{\mathrm{2}}} \vdash^{ \delta_{{\mathrm{1}}} } \refenvnt{v_{{\mathrm{1}}}} :  \langle \refenvnt{A} \rangle^{ \delta_{{\mathrm{2}}} }  \ \token{val} $
                        \item $\Psi_{{\mathrm{3}}}  \vdash  S_{{\mathrm{2}}}  \colon  \Theta_{{\mathrm{2}}}$
                        \item $ \Psi_{{\mathrm{2}}} \subseteq \Psi_{{\mathrm{3}}} $
                        \item $ \Theta_{{\mathrm{1}}} \subseteq \Theta_{{\mathrm{2}}} $
                      \end{itemize}
              \end{itemize}
              The first case is trivial, and we consider the second case.
              By inverting the typing of $\refenvnt{v_{{\mathrm{1}}}}$ and applying
              \zcref{claim:unlift-quote-body}, we have
              $ \Psi_{{\mathrm{3}}} \mid^{ \delta_{{\mathrm{2}}} }  \varepsilon \vdash^{ \delta_{{\mathrm{2}}} }_{  \token{id}  }   \refenvnt{e_{{\mathrm{2}}}} ^{ 0  }  : \refenvnt{A} $
              for some $ \refenvnt{e_{{\mathrm{2}}}} ^{ 0  } $ such that $\refenvnt{v_{{\mathrm{1}}}} =  \langle   \refenvnt{e_{{\mathrm{2}}}} ^{ 0  }   \rangle $.
              By weakening the premise
              $ \Psi_{{\mathrm{1}}} \mid^{   \gamma _{ 0 }  ,\dotsc,  \gamma _{  \refenvnt{k_{{\mathrm{1}}}} ^{+}  }   } \varepsilon \vdash \delta_{{\mathrm{2}}} \preceq  \gamma _{  \refenvnt{k_{{\mathrm{1}}}} ^{+}  }  $
              along $ \Psi_{{\mathrm{1}}} \subseteq \Psi_{{\mathrm{2}}} $ and $ \Psi_{{\mathrm{2}}} \subseteq \Psi_{{\mathrm{3}}} $, and then
              applying \zcref{claim:local-to-global-trans}, we obtain
              $\Psi_{{\mathrm{3}}}  \vdash  \delta_{{\mathrm{2}}}  \preceq   \gamma _{  \refenvnt{k_{{\mathrm{1}}}} ^{+}  } $.  Hence
              \zcref{claim:nht-monotonicity} gives
              \[
                 \Psi_{{\mathrm{3}}} \mid^{   \gamma _{ 1 }  ,\dotsc,  \gamma _{ \refenvnt{k_{{\mathrm{1}}}} }   }  \varepsilon \vdash^{   \gamma _{ 1 }  ,\dotsc,  \gamma _{ \refenvnt{k_{{\mathrm{1}}}} }   }_{  \token{id}  }   \refenvnt{e_{{\mathrm{2}}}} ^{ 0  }  : \refenvnt{A} .
              \]
              Since $ \token{Dom}_{V}( \Psi_{{\mathrm{2}}} )  =  \token{Dom}_{V}( \Psi_{{\mathrm{1}}} ) $, the definition of
              $ \mathcal{V}^{\mathrm{fut} } $ gives the desired result.
	          \end{description}
  \end{description}
\end{proof}


\begin{corollary}[Soundness of Surface Typing]
  If\/ $ \varepsilon \vdash^{  \exclam  }  \refenvnt{e} ^{ 0  }  : \refenvnt{A} $, then either of the following holds.
  \begin{itemize}
    \item $\mathcal{V}^{\mathrm{rt} }  \refenvsym{(}   \refenvnt{e} ^{ 0  }   \refenvsym{,}  \varepsilon  \refenvsym{,}   \token{id}   \refenvsym{,}  \varepsilon  \refenvsym{,}  \varepsilon  \refenvsym{,}  \refenvnt{k_{{\mathrm{2}}}}  \refenvsym{)} =  \token{Timeout} $
    \item $\mathcal{V}^{\mathrm{rt} }  \refenvsym{(}   \refenvnt{e} ^{ 0  }   \refenvsym{,}  \varepsilon  \refenvsym{,}   \token{id}   \refenvsym{,}  \varepsilon  \refenvsym{,}  \varepsilon  \refenvsym{,}  \refenvnt{k_{{\mathrm{2}}}}  \refenvsym{)} = \token{Done} \, \refenvsym{(}  \refenvnt{v}  \refenvsym{,}  N  \refenvsym{,}  S  \refenvsym{)}$ where $ \Psi \mid \Theta \vdash^{  \exclam  } \refenvnt{v} : \refenvnt{A} \ \token{val} $, $ \token{Dom}_{V}( \Psi )  = N$ and $\Psi  \vdash  S  \colon  \Theta$ for some $\Psi$ and $\Theta$.
  \end{itemize}
\end{corollary}

\subsection{Safety of Offline Code Generation}
\begin{lemma}[Discarding Reserved Names]\label{claim:discard-reserved-names}
  If\/ $ \Psi \mid^{  \exclam  }  \varepsilon \vdash^{  \exclam  }_{  \token{id}  }   \refenvnt{e} ^{ 0  }  : \refenvnt{A} $, then $ \varepsilon \mid^{  \exclam  }  \varepsilon \vdash^{  \exclam  }_{  \token{id}  }   \refenvnt{e} ^{ 0  }  : \refenvnt{A} $.
\end{lemma}

\begin{proof}
  We prove the following generalized statements by mutual induction on the derivations.
  \begin{enumerate}
    \item If $ \Psi \mid^{  \exclam  } \Gamma \vdash^{  \overrightarrow{ \gamma }^{+}  }\token{wf} $, then $ \varepsilon \mid^{  \exclam  } \Gamma \vdash^{  \overrightarrow{ \gamma }^{+}  }\token{wf} $.
    \item If $ \Psi \mid^{  \exclam  }  \Gamma \vdash ^{  \overrightarrow{ \gamma }^{+}  } \refenvnt{A} \ \token{wf} $, then $ \varepsilon \mid^{  \exclam  }  \Gamma \vdash ^{  \overrightarrow{ \gamma }^{+}  } \refenvnt{A} \ \token{wf} $.
    \item If $ \Psi \mid^{  \exclam  } \Gamma \vdash \gamma_{{\mathrm{1}}} \preceq \gamma_{{\mathrm{2}}} $ where $\gamma_{{\mathrm{1}}} \, \in \,  \token{Dom}_{C}( \Gamma ) $ and $\gamma_{{\mathrm{2}}} \, \in \,  \token{Dom}_{C}( \Gamma ) $, then $ \varepsilon \mid^{  \exclam  } \Gamma \vdash \gamma_{{\mathrm{1}}} \preceq \gamma_{{\mathrm{2}}} $.
    \item If $ \Psi \mid^{  \exclam  } \Gamma \vdash \gamma_{{\mathrm{1}}} \subseteq \gamma_{{\mathrm{2}}} $ where $\gamma_{{\mathrm{1}}} \, \in \,  \token{Dom}_{C}( \Gamma ) $ and $\gamma_{{\mathrm{2}}} \, \in \,  \token{Dom}_{C}( \Gamma ) $, then $ \varepsilon \mid^{  \exclam  } \Gamma \vdash \gamma_{{\mathrm{1}}} \subseteq \gamma_{{\mathrm{2}}} $.
    \item\label{item:discard-reserved-names-generalized-expression} If $ \Psi \mid^{  \exclam  }  \Gamma \vdash^{  \overrightarrow{ \gamma_{{\mathrm{1}}} }^{+}  }_{  \token{id}  }  \refenvnt{e} : \refenvnt{A} $, then $ \varepsilon \mid^{  \exclam  }  \Gamma \vdash^{  \overrightarrow{ \gamma_{{\mathrm{1}}} }^{+}  }_{  \token{id}  }  \refenvnt{e} : \refenvnt{A} $.
  \end{enumerate}
  Then, the main statement is the special case of \zcref{item:discard-reserved-names-generalized-expression}, where $\Gamma =  \varepsilon $.
\end{proof}

\begin{theorem}[Safety of Offline Code Generation]
  \label{claim:safety-offline-code-gen}
  If\/ $ \varepsilon \vdash^{  \exclam  }  \refenvnt{e_{{\mathrm{1}}}} ^{ 0  }  :  \langle \refenvnt{A} \rangle^{  \exclam  }  $ and\/ $\mathcal{V}^{\mathrm{rt} }  \refenvsym{(}   \refenvnt{e_{{\mathrm{1}}}} ^{ 0  }   \refenvsym{,}  \varepsilon  \refenvsym{,}   \token{id}   \refenvsym{,}  \varepsilon  \refenvsym{,}  \varepsilon  \refenvsym{,}  \refenvnt{k_{{\mathrm{2}}}}  \refenvsym{)} = \token{Done} \, \refenvsym{(}  \refenvnt{v}  \refenvsym{,}  N  \refenvsym{,}  S  \refenvsym{)}$, then $\refenvnt{v} =  \langle   \refenvnt{e_{{\mathrm{2}}}} ^{ 0  }   \rangle $ and\/ $ \varepsilon \vdash^{  \exclam  }  \refenvnt{e_{{\mathrm{2}}}} ^{ 0  }  : \refenvnt{A} $ for some $ \refenvnt{e_{{\mathrm{2}}}} ^{ 0  } $.
\end{theorem}

\begin{proof}
  From \zcref{claim:type-soundness}, we have some $\Psi, \Theta$
  such that $ \Psi \mid \Theta \vdash^{  \exclam  } \refenvnt{v} :  \langle \refenvnt{A} \rangle^{  \exclam  }  \ \token{val} $
  where $ \token{Dom}_{V}( \Psi )  = N$ and $ \token{Dom}_{L}( \Theta )  =  \token{Dom}_{L}( S ) $.
  By inversion of \ref{rule:value-type-code}, there is some $\refenvnt{e_{{\mathrm{2}}}}$ such
  that $\refenvnt{v} =  \langle  \refenvnt{e_{{\mathrm{2}}}}  \rangle $ and
  \[
     \Psi \mid^{  \exclam  }  \varepsilon \vdash^{  \exclam  }_{  \token{id}  }   \langle  \refenvnt{e_{{\mathrm{2}}}}  \rangle  :  \langle \refenvnt{A} \rangle^{  \exclam  }  .
  \]
  By inversion of \ref{rule:runtime-type-quote}, we have
  \[
     \Psi \mid^{  \exclam  }   \blacktriangleright ^{  \exclam  }  \vdash^{  \exclam   \refenvsym{,}   \exclam  }_{  \token{id}  }  \refenvnt{e_{{\mathrm{2}}}} : \refenvnt{A} .
  \]
  Hence \zcref{claim:unlift-quote-body} gives
  $ \Psi \mid^{  \exclam  }  \varepsilon \vdash^{  \exclam  }_{  \token{id}  }  \refenvnt{e_{{\mathrm{2}}}} : \refenvnt{A} $.  Finally,
  \zcref{claim:discard-reserved-names} yields
  $ \varepsilon \mid^{  \exclam  }  \varepsilon \vdash^{  \exclam  }_{  \token{id}  }  \refenvnt{e_{{\mathrm{2}}}} : \refenvnt{A} $.
\end{proof}

\section{Counterexamples for Type Soundness of \lambra}\label{sec:lambra-counterexamples}
\newcommand{\ptint}{\texttt{int}\xspace}
\newcommand{\ptref}{\ \texttt{ref}}
\newcommand{\pref}[1]{\texttt{ref}_{\{#1\}}}
\newcommand{\pset}[1]{\texttt{set}_{\{#1\}}}
\newcommand{\pget}[1]{\texttt{get}_{\{#1\}}}
\newcommand{\prun}[1]{\texttt{run}_{\{#1\}}}
\newcommand{\plift}[1]{\texttt{lift}_{\{#1\}}}
\newcommand{\plet}{\texttt{let}\;}
\newcommand{\pin}{\;\texttt{in}\;}
\newcommand{\pseq}{\texttt{;}}
\newcommand{\peq}{\texttt{=}}
\lambra~\cite{conf/esop/Rhiger12} is an attempt to design a contextual-types-based type system for MetaML-style MSP with mutable state. The idea is to annotate code types with contexts, which is similar in spirit to our use of RECs. However, contextual types in \lambra account only for what we call reachability and cannot capture visibility. As a result, \lambra admits well-typed programs that nevertheless cause scope extrusion. In fact, the scope-extrusion example from Section 2.3 is typable in \lambra. Below, we present the corresponding program in \lambra.
\begin{align*}
  ;\vdash & \;\plet\;r^{[](\ptint)\ptref}\ \peq\ \pref{[](\ptint)}(\uparrow 1)\;\texttt{in}                                                                                                      \\
          & \uparrow\uparrow(\lambda x^{\ptint}.\downarrow\downarrow(\pset{[](\ptint)}(r, \uparrow(\plet y^{\ptint}\ \peq\ \uparrow(x)\;\texttt{in}\;1))\texttt{;}\uparrow\uparrow x))\texttt{;} \\
          & \; \pget{\ptint\to\ptint}(r)                                                                                                                                                         \\
  :       & \; \texttt{int} \to \texttt{int}
\end{align*}
The semantics of \lambra uses a local store, which does not allow code fragments to escape their defining scopes. Hence, $\pset{[](\ptint)}$ on the second line gets stuck, because the code fragment $\uparrow(\plet y^{\ptint}\ \peq\ \uparrow(x)\;\texttt{in}\;1)$ cannot escape the scope of $x$. This is a counterexample to progress for \lambra.

\bibliographystyle{plain}
\bibliography{mybib}

\end{document}
